# Supplementary material for: The CoCo-Beholder: Enabling Comprehensive Evaluation of Congestion Control Algorithms
Source: arXiv:1912.10531 source file (2019-12-22)
Supplement: Supplementary file 1 [file AppendixA.tex]

\section{The Help Message of CoCo-Beholder Testing Tool}

\bigbreak
\bigbreak

\begin{lstlisting}[frame=single]
$ ./run.py -h
usage: run.py [-h] [-d DIR] -p DIR [-l FILE] [-r MBITPS] [-t SEC] [-m USEC]
              [-s SEED] [-b MiB] [-q1 SIZE] [-q2 SIZE] [-q SIZE]
              base delta step [jitter]

The script tests congestion control schemes by running flows of different
schemes in the dumbbell topology for runtime seconds. Each flow has a host in
the left half and a host in the right half of the topology and the hosts                                                           
exchange a scheme's traffic with one host being the sender and one being the                                                       
receiver. There is the left router that interconnects all the hosts in the                                                         
left half and the right router that interconnects all the hosts in the right                                                       
half of the topology. All the flows share the common central link between the                                                      
two routers. User can define how many flows of which schemes should be run by                                                      
defining groups of flows. A group of flows is defined by a scheme name, number                                                     
of flows, a second of runtime at which the group of flows should be started,                                                       
direction of the flows: left-to-right or right-to-left, rate/delay/queue-size                                                      
of the links belonging to the flows in the left half of the topology,                                                              
rate/delay/queue-size of the links belonging to the flows in the right half of                                                     
the topology. For the central link, user can define its rate, constant or                                                          
VARIABLE DELAY with optional jitter, individual queue-size for each end of the                                                     
central link. Qdisc netem is applied to interfaces of links to set rates,                                                          
delays and queue-sizes of the links. For each link, the specified rate/delay                                                       
/queue-size parameters are always installed at both ends of the link.                                                              
             
  
          
                                                                                                                                     
positional arguments:                                                                                                              
  base                  Initial delay set at both ends of the central link in                                                      
                        the formats: N (milliseconds assumed), Nus, Nms, Ns                                                        
        
                        
  delta                 The delay at both ends of the central link is changed
                        each delta time, the formats for delta: N
                        (milliseconds assumed), Nus, Nms, Ns. If you do not
                        need variable delay and want the delay to be constant
                        just set delta to a value greater than that of
                        -t/--runtime.
                        
  step                  Step by which the delay at both ends of the central
                        link is changed each delta time in these formats: N
                        (milliseconds assumed), Nus, Nms, Ns. The delay will
                        always lie in range [0us, --max-delay us].
                        
  jitter                Jitter affecting the delay at both ends of the central
                        link in the formats: N (milliseconds assumed), Nus,
                        Nms, Ns. The argument is optional.
                        

optional arguments:
  -h, --help            show this help message and exit
                        
  -d DIR, --dir DIR     Output directory, default is "dumps". Service file
                        metadata.json containing parameters with which testing
                        is actually performed is written there. For each flow,
                        pcap-files, recorded at interfaces of the two hosts
                        between which the flow runs, are written there named
                        "<flow's starting #>-<scheme>-<sender/receiver>.pcap"
                        
  -p DIR, --pantheon DIR
                        Pantheon [pantheon.stanford.edu] directory where
                        congestion control schemes are searched
                        
  -l FILE, --layout FILE
                        Input yaml-file defining groups of flows run in the
                        dumbbell topology. Default is "layout.yml" and during
                        the first run of the script this file is created with
                        example settings.
                        
                            
                               
  -r MBITPS, --rate MBITPS
                        Rate of the central link in Mbit/s, type is float,
                        default value is 100.0. If you do not want to limit
                        the rate just set it to zero: for qdisc netem, setting
                        rate/delay of an interface to zero means the same as
                        you leave the parameter unset.
                        
  -t SEC, --runtime SEC
                        Runtime of testing in seconds (default 30)
                        
  -m USEC, --max-delay USEC
                        Max delay and jitter fed to netem in microseconds
                        (default is 100000000, i.e. 100 sec)
                        
  -s SEED, --seed SEED  Randomization seed to define if the delay at the
                        central link is increased or decreased by step after a
                        subsequent delta time, if not specified is set to
                        current Unix time. The parameter is useful if one
                        wants to reproduce results of testing in which delay
                        variability feature was used.
                        
  -b MiB, --buffer MiB  Set the operating system capture buffer size to chosen
                        number of MiB (1024 KiB), default is 2 MiB. The value
                        is set as -B option for tcpdump recordings on all
                        hosts.
                        
  -q1 SIZE, --first-queue SIZE
                        Size of transmit queue of the left router's interface
                        at the first end of the central link of the dumbbell
                        topology, default is 1000 packets
                        
  -q2 SIZE, --second-queue SIZE
                        Size of transmit queue of the right router's interface
                        at the second end of the central link of the dumbbell
                        topology, default is 1000 packets
                        
  -q SIZE, --queues SIZE
                        Common size of transmit queues of both the interfaces
                        at the ends of the central link of the dumbbell
                        topology, same as -q1 N -q2 N, default is 1000 packets

\end{lstlisting}

\section{The Help Message of CoCo-Beholder Analysis Tool}

\bigbreak
\bigbreak

\begin{lstlisting}[frame=single]
$ ./analyze.py -h
usage: analyze.py [-h] [-d DIR] [-o OUTPUT_DIR]

The script extracts data from pcap-files captured during testing.

optional arguments:
  -h, --help            show this help message and exit
                        
  -d DIR, --dir DIR     folder with input pcap-files, default is "dumps"
                        
  -o OUTPUT_DIR, --output-dir OUTPUT_DIR
                        folder with output files, default is "graphs/data"
\end{lstlisting}

\section{The Help Message of CoCo-Beholder Plotting Tool}

\bigbreak
\bigbreak

\begin{lstlisting}[frame=single]
$ ./plot.py -h
usage: plot.py [-h] [-d DIR] [-o OUTPUT_DIR] [-f] [-t] [-s "FIELD1 FIELD2..."]
               [-i SEC] [-c "COLOR1 COLOR2..."] [-j COLOR]

The script makes graphs and stats over data extracted from pcap-files.
Possible types of graphs and stats: per-flow (-f), total (-t), per-subset
(-s). For any type chosen, the following graphs and stats are generated:
average throughput, average Jain's index, average one-way delay, per-packet
one-way delay. The average graphs are averaged per chosen time interval (-i).
Average Jain's index graph always contains one curve, as it is computed over
the curves present in the corresponding average throughput graph.

optional arguments:
  -h, --help            show this help message and exit
                        
  -d DIR, --dir DIR     Folder with input data-files, default is "graphs/data"
                        
  -o OUTPUT_DIR, --output-dir OUTPUT_DIR
                        Folder with output graphs and stats, default is
                        "graphs"
                        
  -f, --per-flow        Graphs and stats are generated per flow, i.e. each
                        graph has a separate curve per flow
                        
  -t, --total           Total graphs and stats are generated for all flows
                        altogether, i.e. each graph has only one curve
                        
  -s "FIELD1 FIELD2...", --per-subset "FIELD1 FIELD2..."
                        Graphs and stats are generated per subset, i.e. each
                        graph has one curve per subset. Flows are in one
                        subset if they have the same values of the chosen
                        layout field(s). E.g. for -s "scheme direction", each
                        graph will have one curve per subset of flows having
                        both the same scheme name and direction. Currently
                        allowed layout fields: ['scheme', 'direction'].
                        
  -i SEC, --interval SEC
                        Interval per which average graphs are computed in
                        seconds, default is 0.5
                        
  -c "COLOR1 COLOR2...", --colors "COLOR1 COLOR2..."
                        Color cycle for curves with colors specified in any
                        format recognized by matplotlib
                        
  -j COLOR, --jains-index-color COLOR
                        Color for Jain's index curve, if not specified the
                        first color in -c/--colors is used
\end{lstlisting}

\section{The Help Message of CoCo-Beholder Cleaning Tool}

\bigbreak
\bigbreak

\begin{lstlisting}[frame=single]
$ ./clean.py -h
usage: clean.py [-h] [-a] [-p] [-d] [-g] [-s] [-r] [-m] [-f1 FOLDER1]
                [-f2 FOLDER2] [-f3 FOLDER3]

The script cleans three output directories. The script deletes only
pcap/json/png/log files and does not touch any subdirectories. If any of the
chosen directories gets completely empty the script also deletes the
directory.

optional arguments:
  -h, --help            show this help message and exit
                        
  -a, --all             delete all files in the three directories, same as
                        -pdg
                        
  -p, --pcap, --pcaps   delete all files in directory with pcap-files
                        
  -d, --data            delete all files in directory with data-files
                        
  -g, --graph, --graphs
                        delete all files in directory with graphs
                        
  -s, --senders, --sender
                        among chosen files, delete files belonging exclusively
                        to senders
                        
  -r, --receivers, --receiver
                        among chosen files, delete files belonging exclusively
                        to receivers
                        
  -m, --mutual          among chosen files, delete files common for senders
                        and receivers
                        
  -f1 FOLDER1, --folder1 FOLDER1
                        directory with pcap-files to clean, default is "dumps"
                        
  -f2 FOLDER2, --folder2 FOLDER2
                        directory with data-files to clean, default is
                        "graphs/data"
                        
  -f3 FOLDER3, --folder3 FOLDER3
                        directory with graphs to clean, default is "graphs"
\end{lstlisting}
