# Supplementary material for: The CoCo-Beholder: Enabling Comprehensive Evaluation of Congestion Control Algorithms
Source: arXiv:1912.10531 source file (2019-12-22)
Supplement: Supplementary file 2 [file AppendixB.tex]

\section{The Testing Setup}

\begin{lstlisting}[frame=single,caption=The command.,mathescape]
$\text{\textbf{\textcolor{teal}{\$} ./run.py \textcolor{darkblue}{-p} \(\sim\)/pantheon 0ms 500ms 10ms 5ms \textcolor{darkblue}{-t} 20 \textcolor{darkblue}{-r} 70 \textcolor{darkblue}{-s} 3}}$
\end{lstlisting}

\begin{lstlisting}[frame=single,language=yaml,caption=The layout file.]
# Delays/rates are optional: if lacking or null, they are set to 0us/0.0
# and for netem, to set delay/rate to zero is same as to leave it unset.
# Sizes of queues are optional: if lacking or null, they are set to 1000.
- direction: <-
  flows: 3
  left-delay: null
  left-queues: null
  left-rate: 20
  right-delay: 50ms
  right-queues: null
  right-rate: null
  scheme: bbr
  start: 0
- direction: ->
  flows: 3
  left-delay: 5ms
  left-queues: null
  left-rate: 20
  right-delay: 5ms
  right-queues: null
  right-rate: null
  scheme: bbr
  start: 0
- direction: <-
  flows: 2
  left-delay: 50ms
  left-queues: null
  left-rate: null
  right-delay: null
  right-queues: null
  right-rate: 10
  scheme: copa
  start: 10
- direction: ->
  flows: 2
  left-delay: 5ms
  left-queues: null
  left-rate: null
  right-delay: 5ms
  right-queues: null
  right-rate: 10
  scheme: copa
  start: 10
\end{lstlisting}

\section{Example Output of CoCo-Beholder Plotting Tool}

In Listing~\ref{list:plottingoutput}, there is an example output of CoCo-Beholder plotting tool generating per-scheme plots and statistics.\\

\begin{minipage}{\linewidth}
\begin{lstlisting}[caption=An example output of CoCo-Beholder plotting tool.,label=list:plottingoutput,mathescape] 
$\text{\textbf{\textcolor{teal}{\$} ./plot.py \textcolor{darkblue}{-s} "scheme"}}$
Loading data of the curves to make average plots and stats...
Plotting average throughput...
Plotting average one-way delay...
Plotting average Jain's index...
Saving average statistics...
Plotting per packet one-way delay...
Saving per-packet statistics...
SUCCESS
\end{lstlisting}
\end{minipage}

\newpage

\section{Per-Flow Plots and Statistics}

The default aggregation interval 0.5 s is indicated in all the average plots of this section. 

\begin{figure}[h!]
\centering
\includegraphics[width=\textwidth]{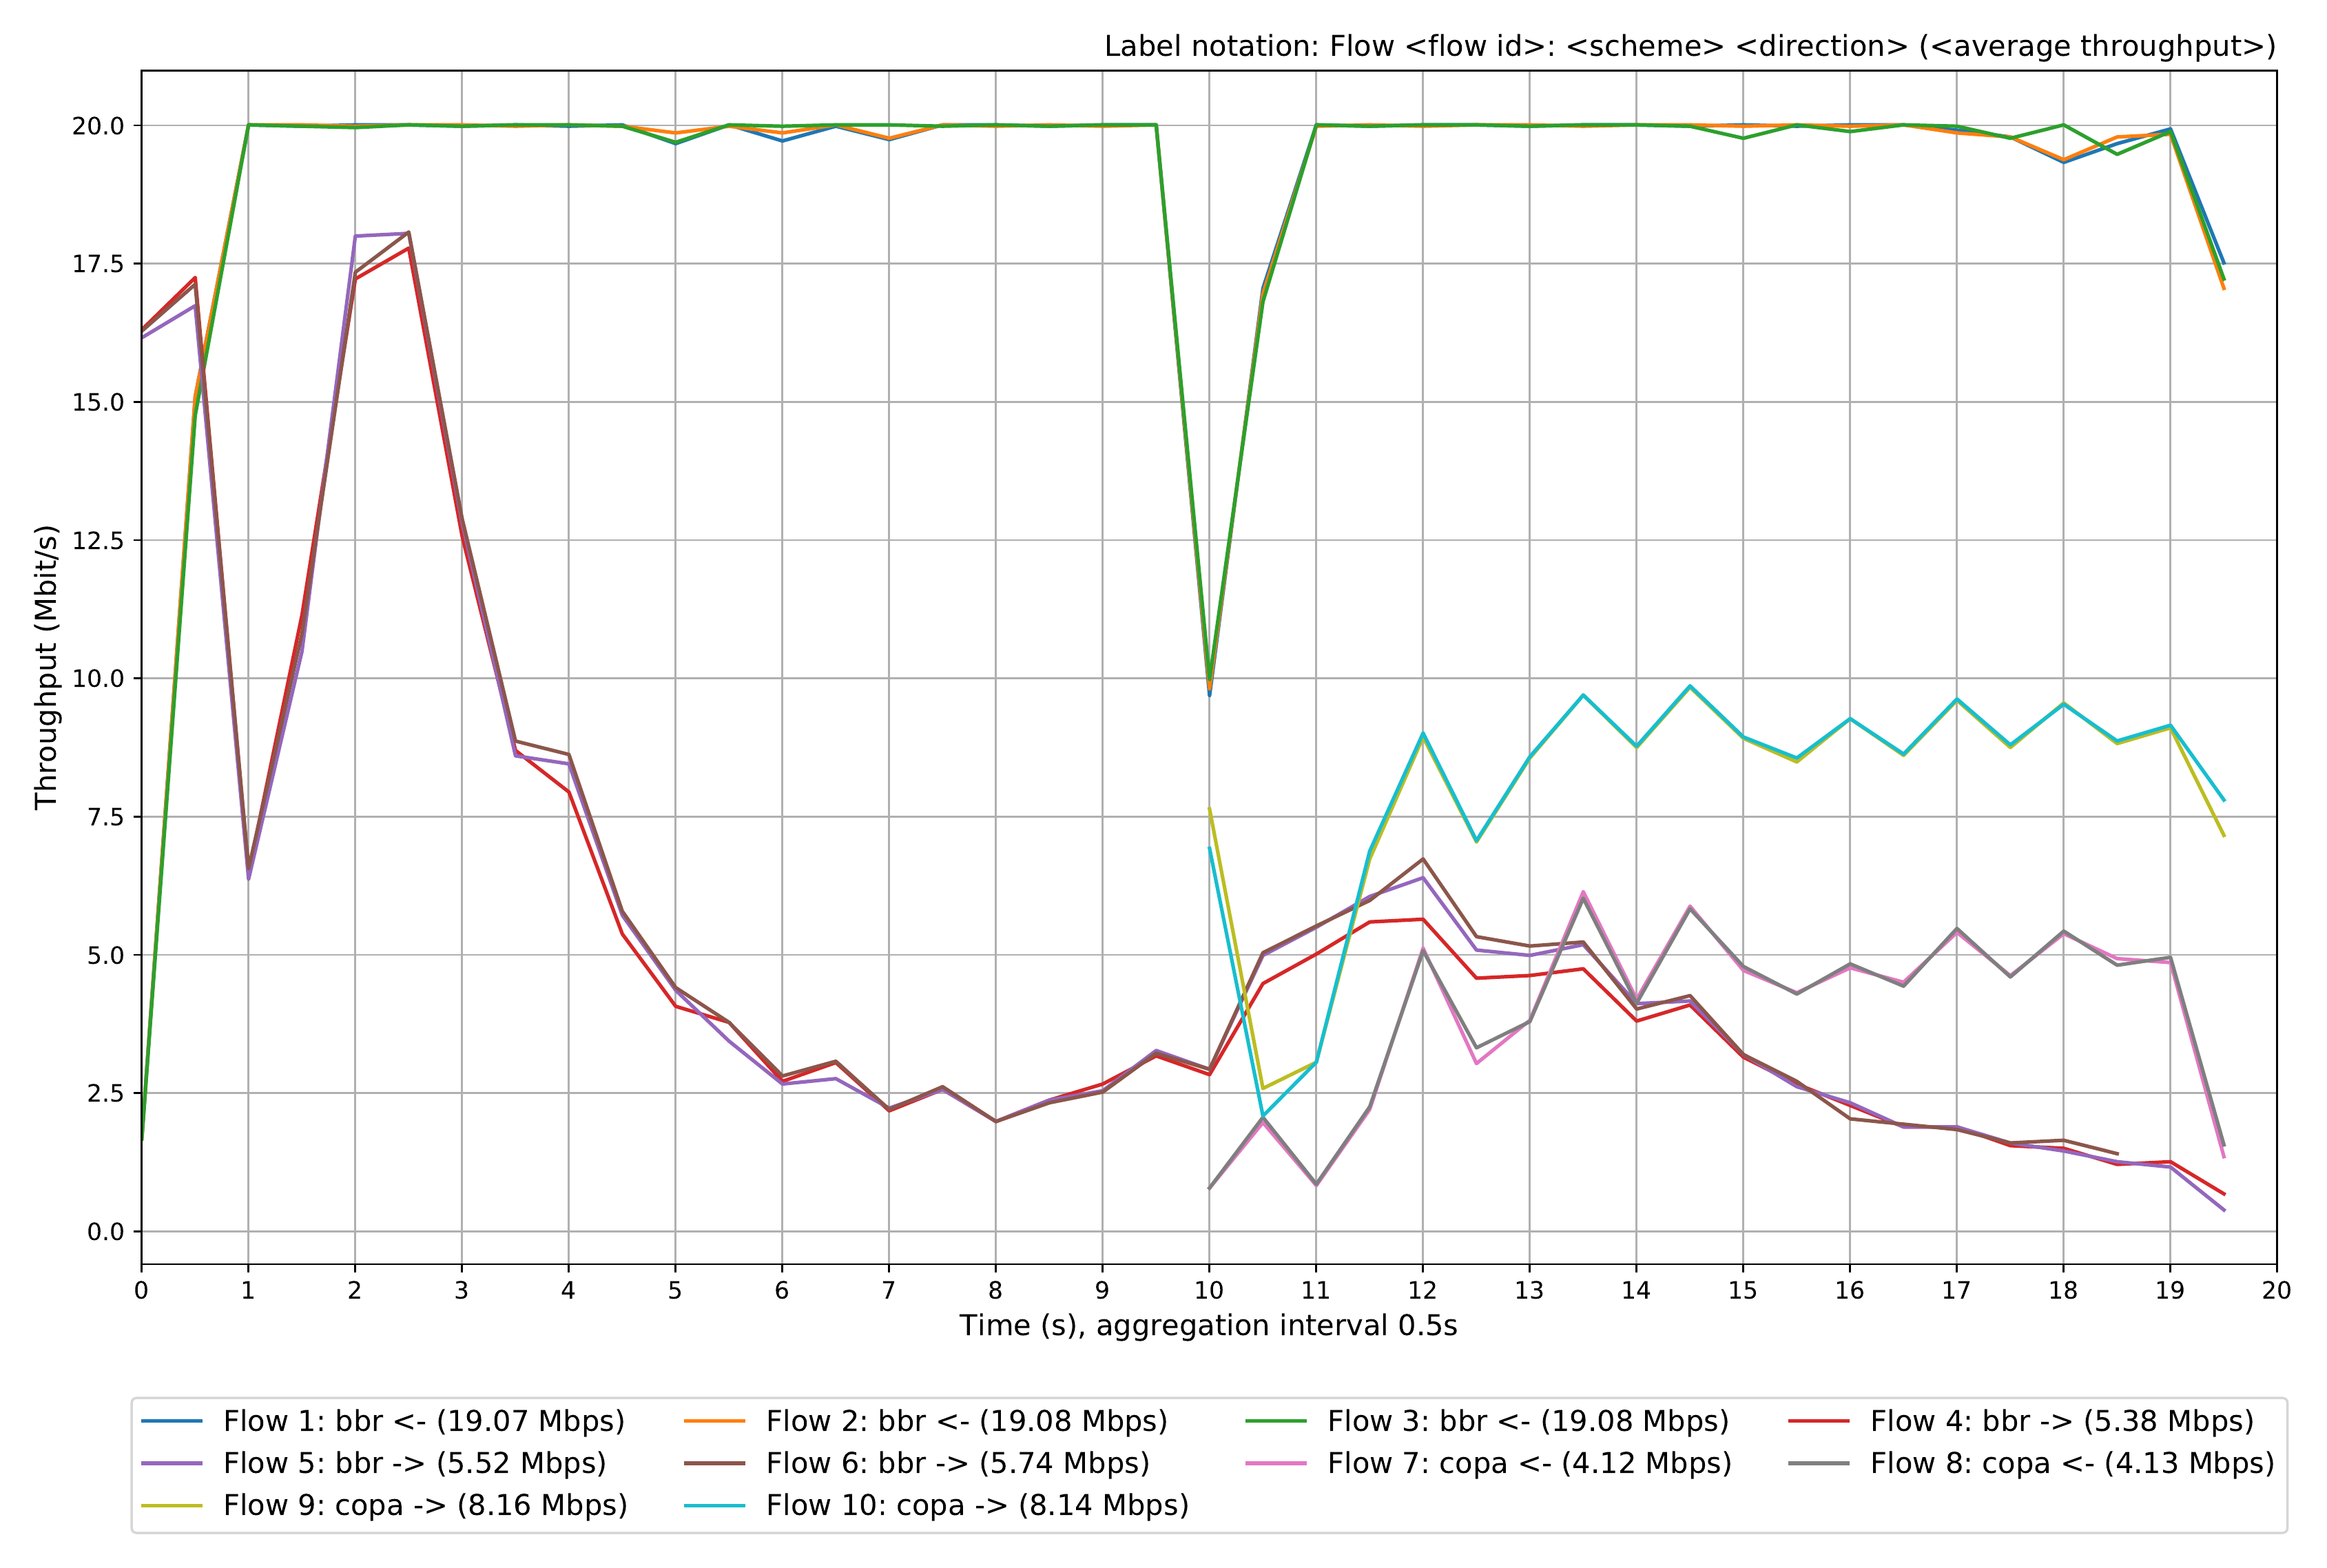}
\caption{Per-flow average throughput plot.}
\label{fig:pfrate}
\end{figure}

\begin{figure}[h!]
\centering
\includegraphics[width=\textwidth]{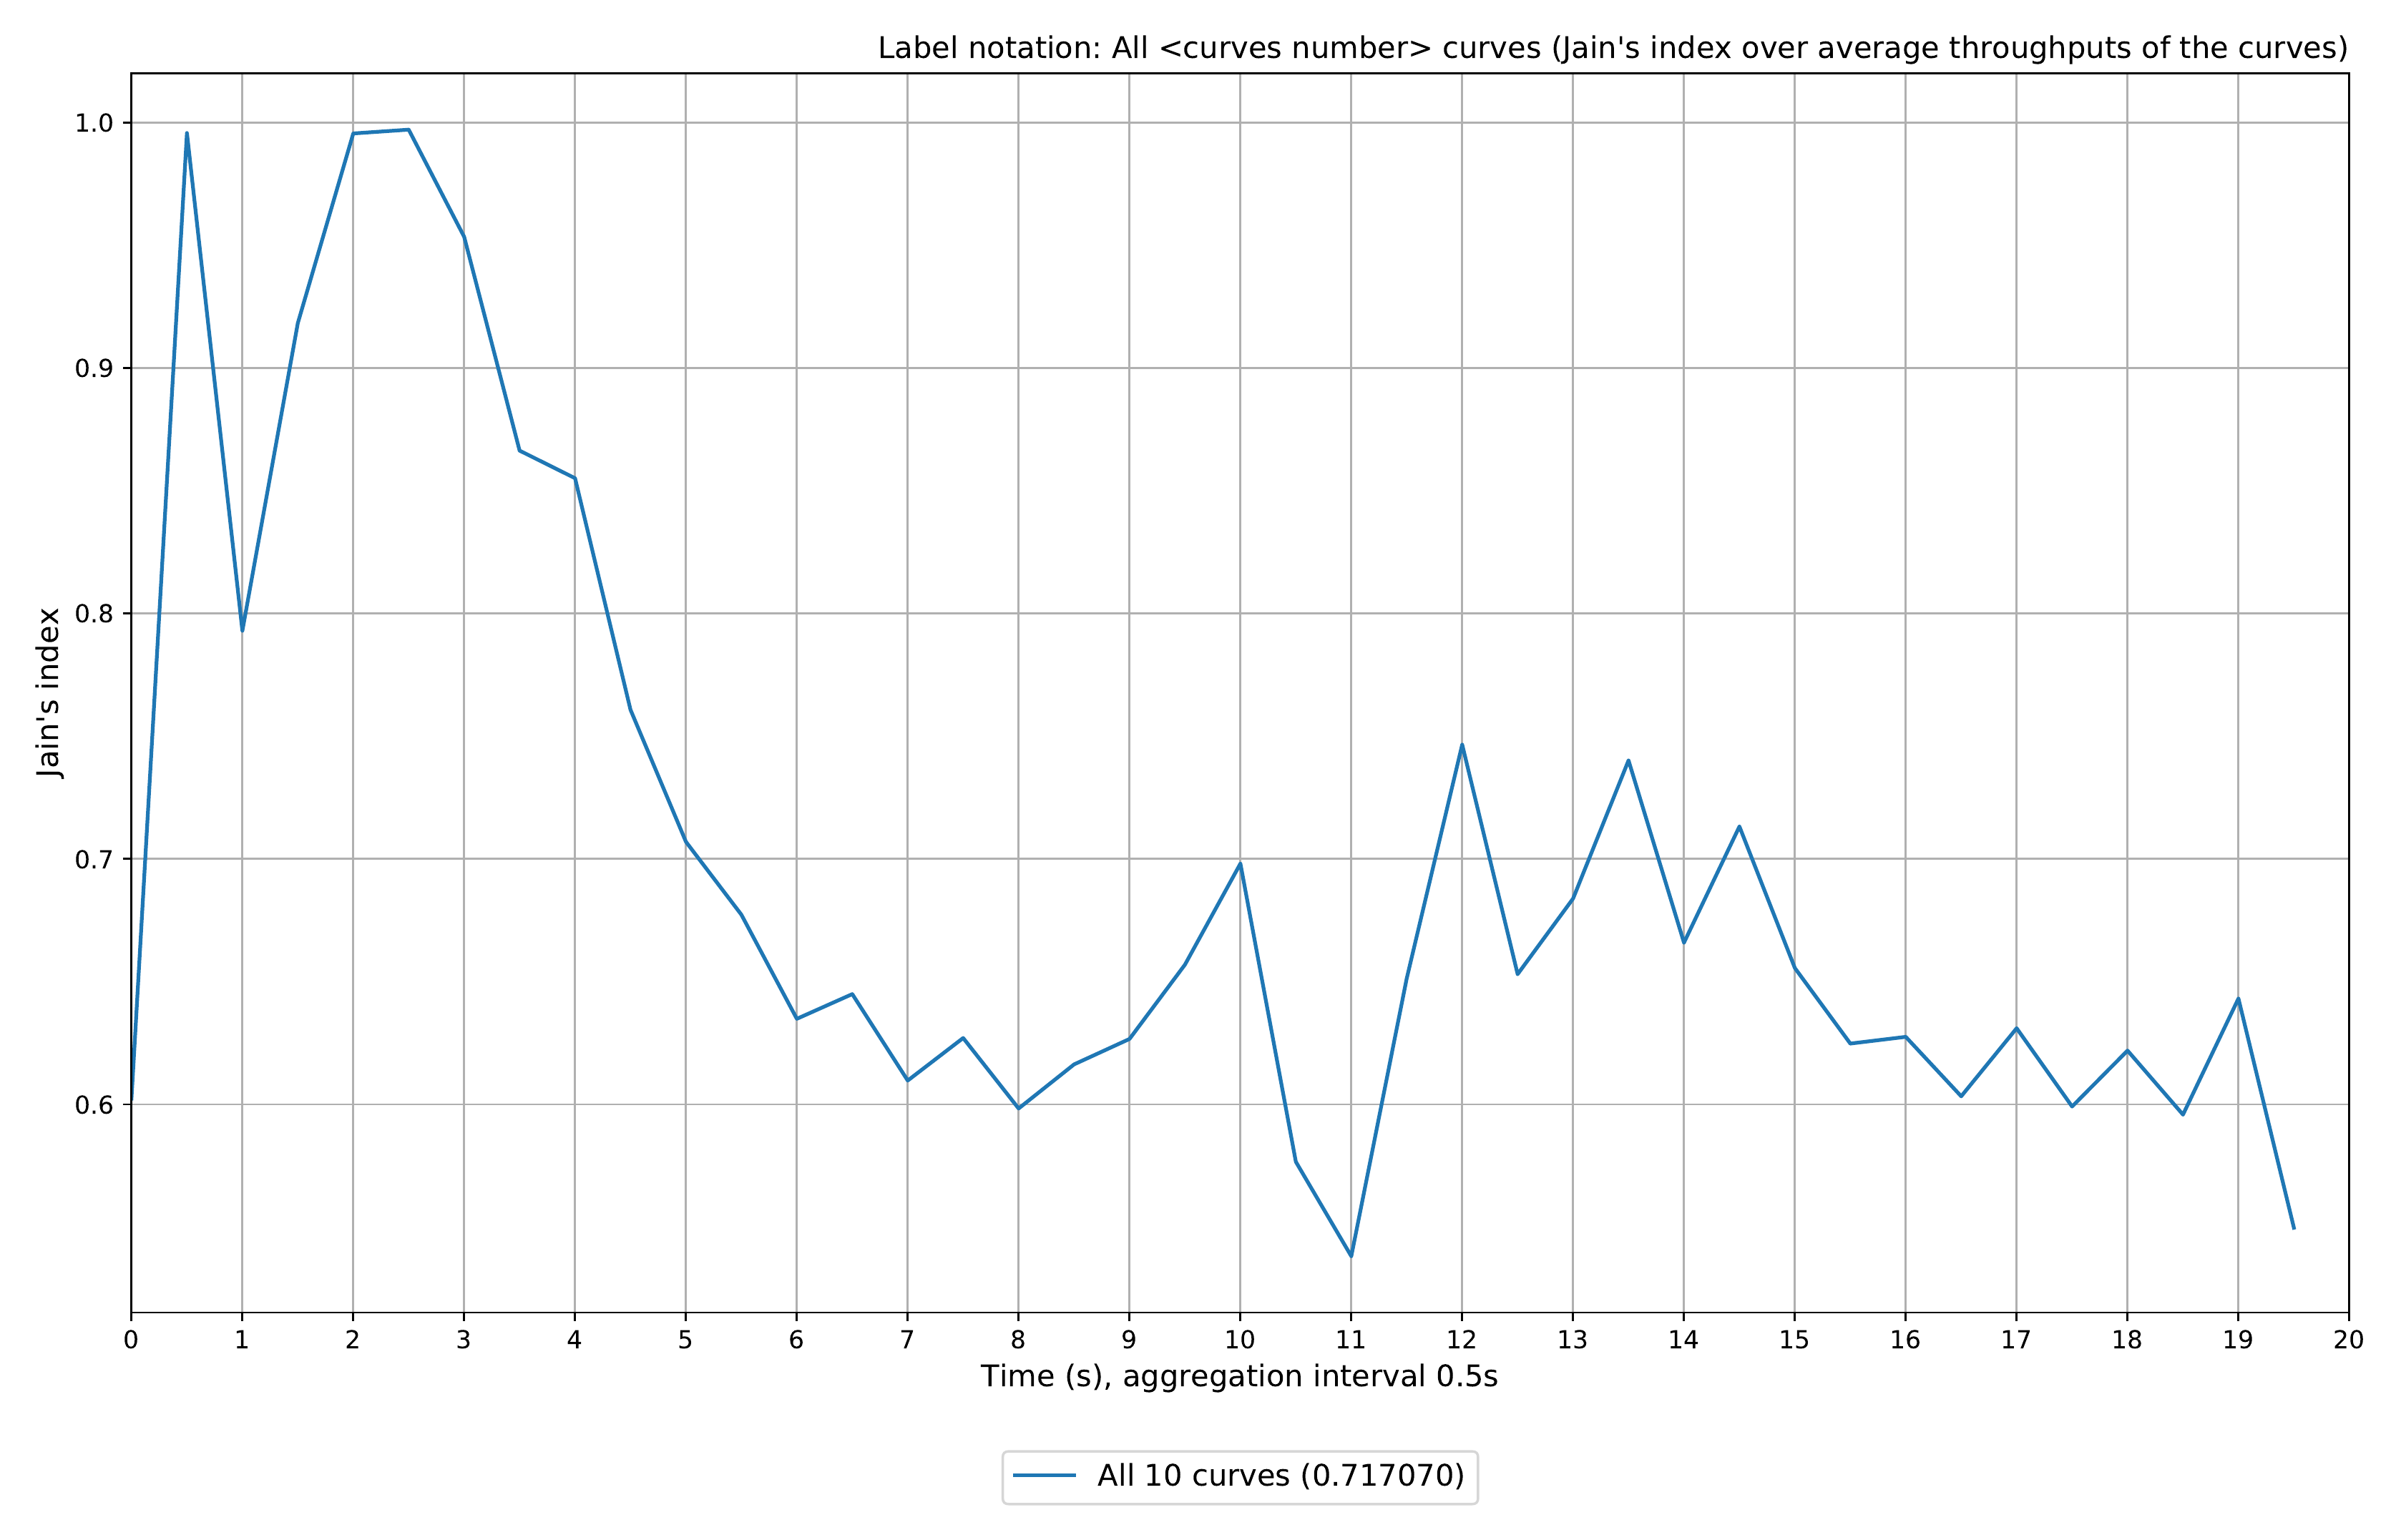}
\caption{Per-flow average Jain's index plot.}
\label{fig:pfjain}
\end{figure}

It can be seen that the average Jain's Index plot~\ref{fig:pfjain} indeed corresponds to the curves in the average rate plot~\ref{fig:pfrate}. In the meanwhile, the average one-way delay plot~\ref{fig:pfavgdelay} looks quite similar to the per-packet one-way delay plot~\ref{fig:pfpptdelay}.

\begin{figure}[h!]
\centering
\includegraphics[width=\textwidth]{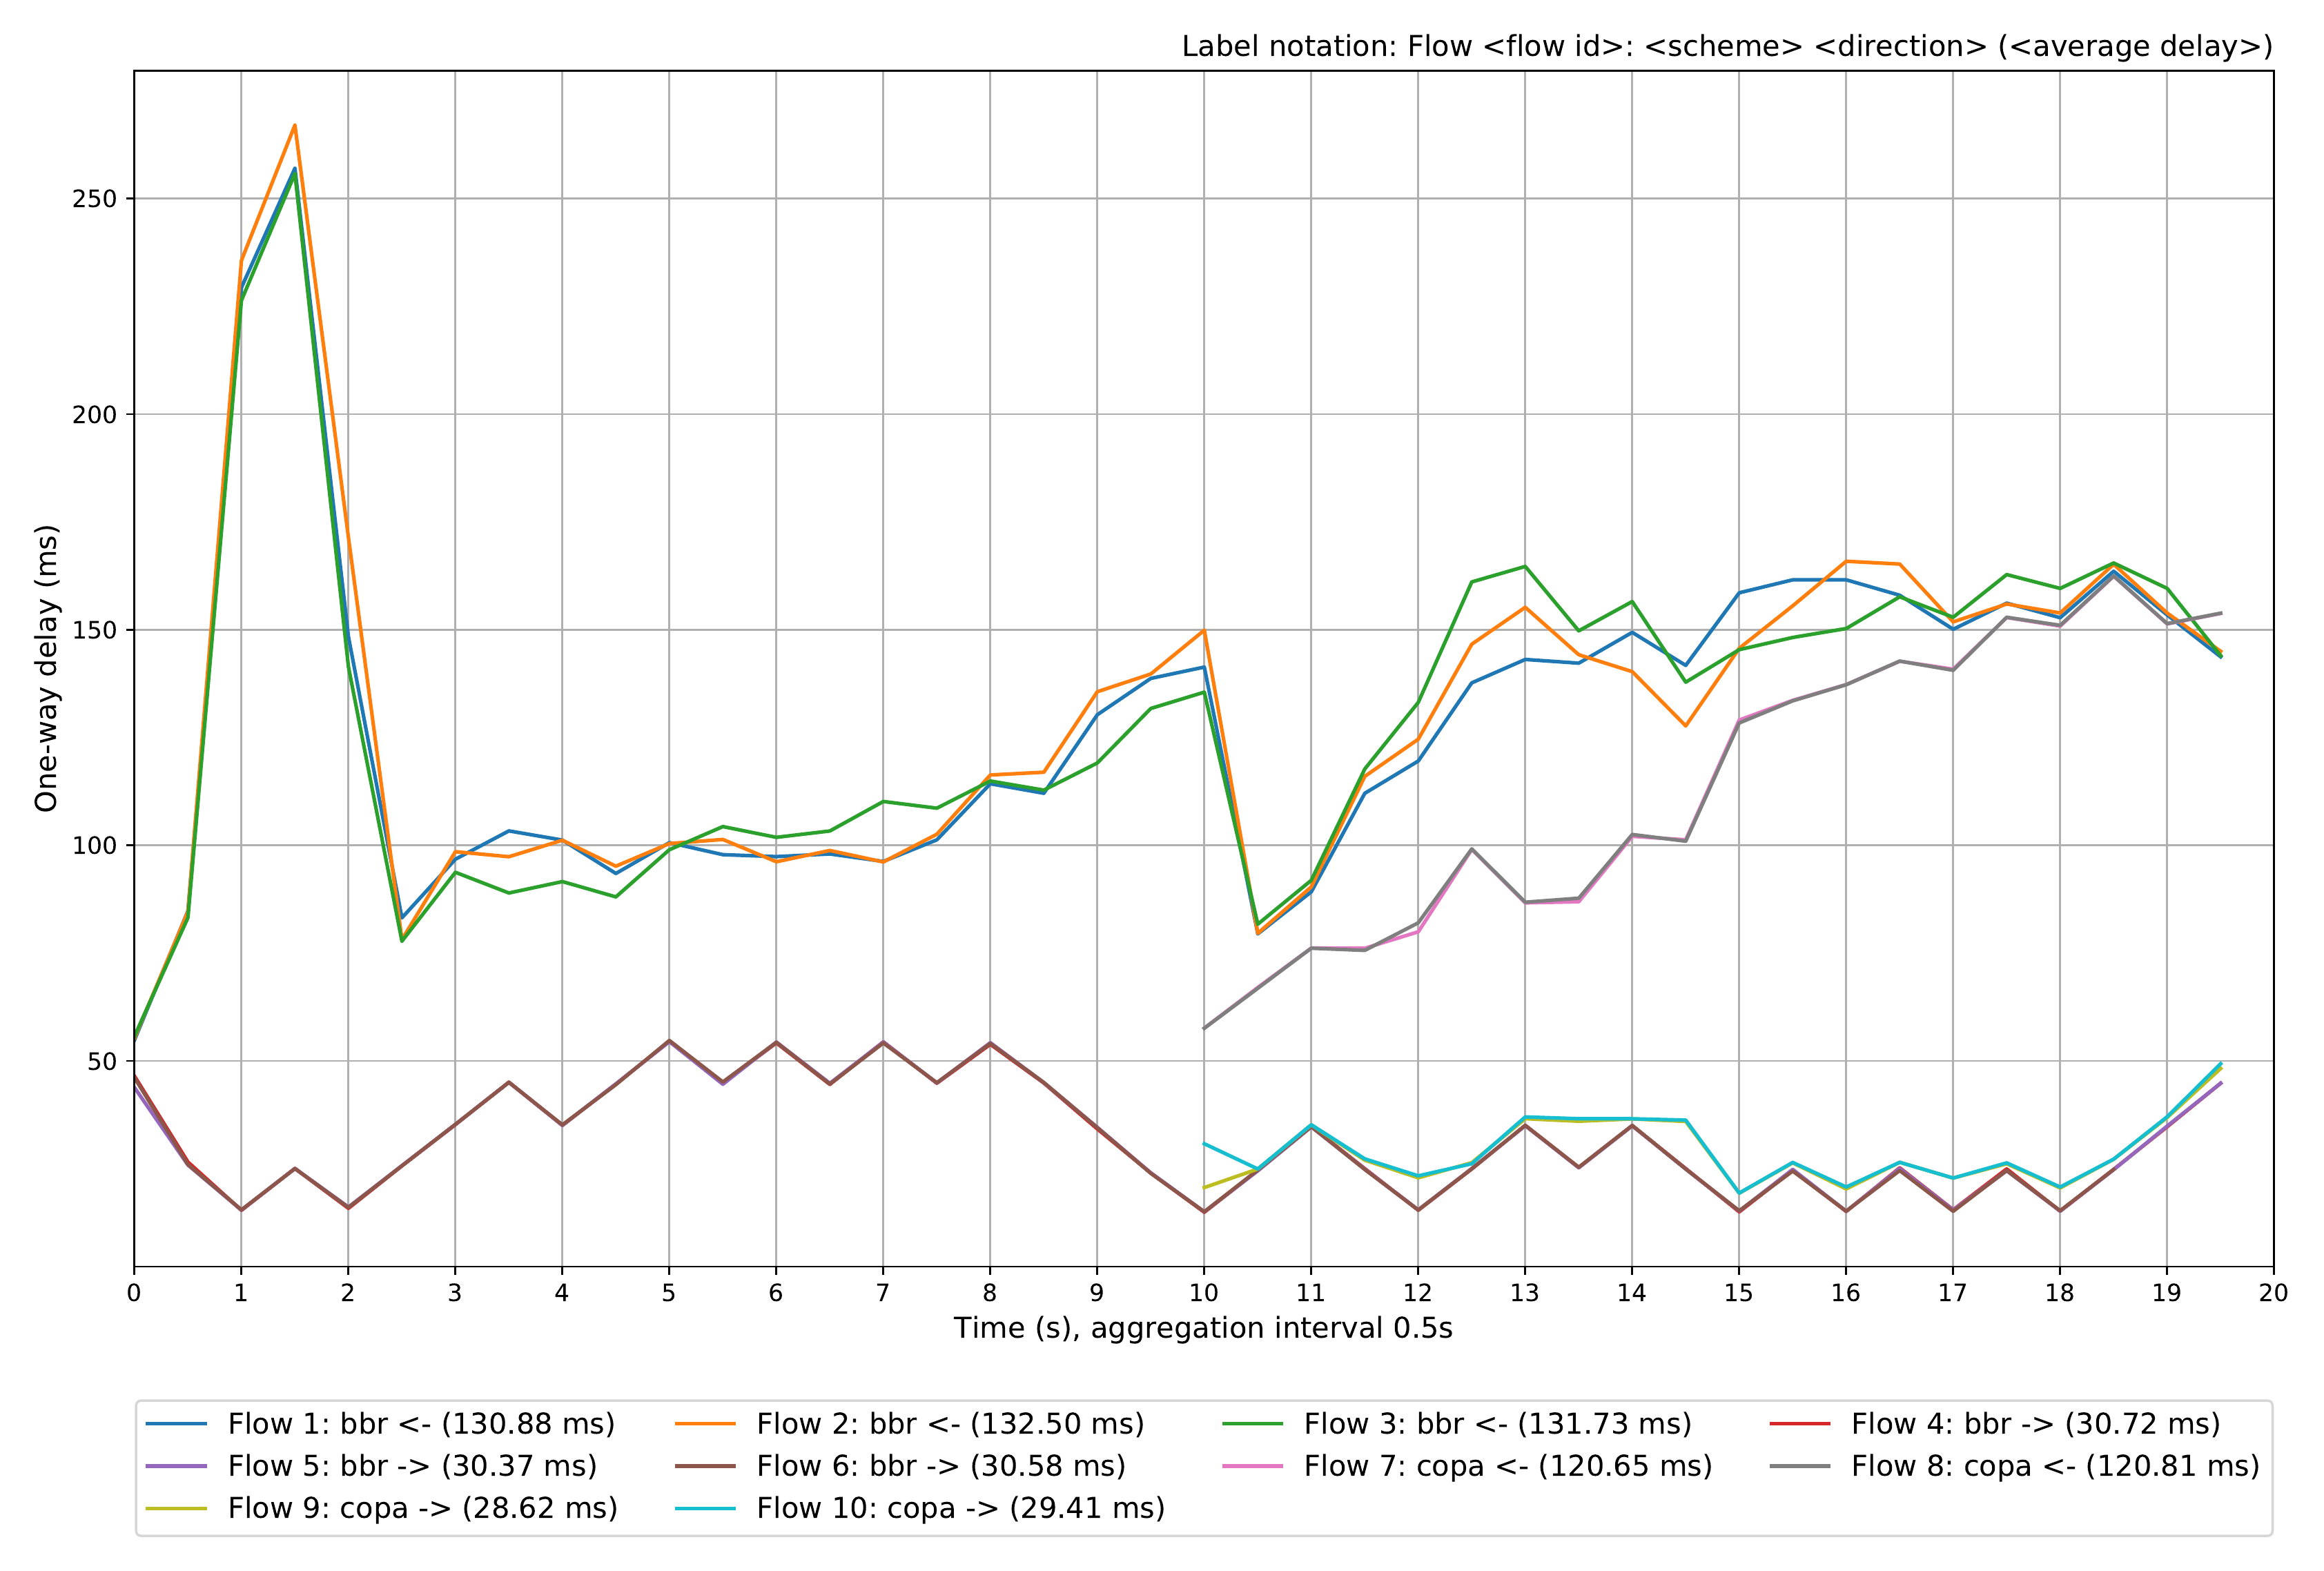}
\caption{Per-flow average one-way delay plot.}
\label{fig:pfavgdelay}
\end{figure}

\begin{figure}[h!]
\centering
\includegraphics[width=\textwidth]{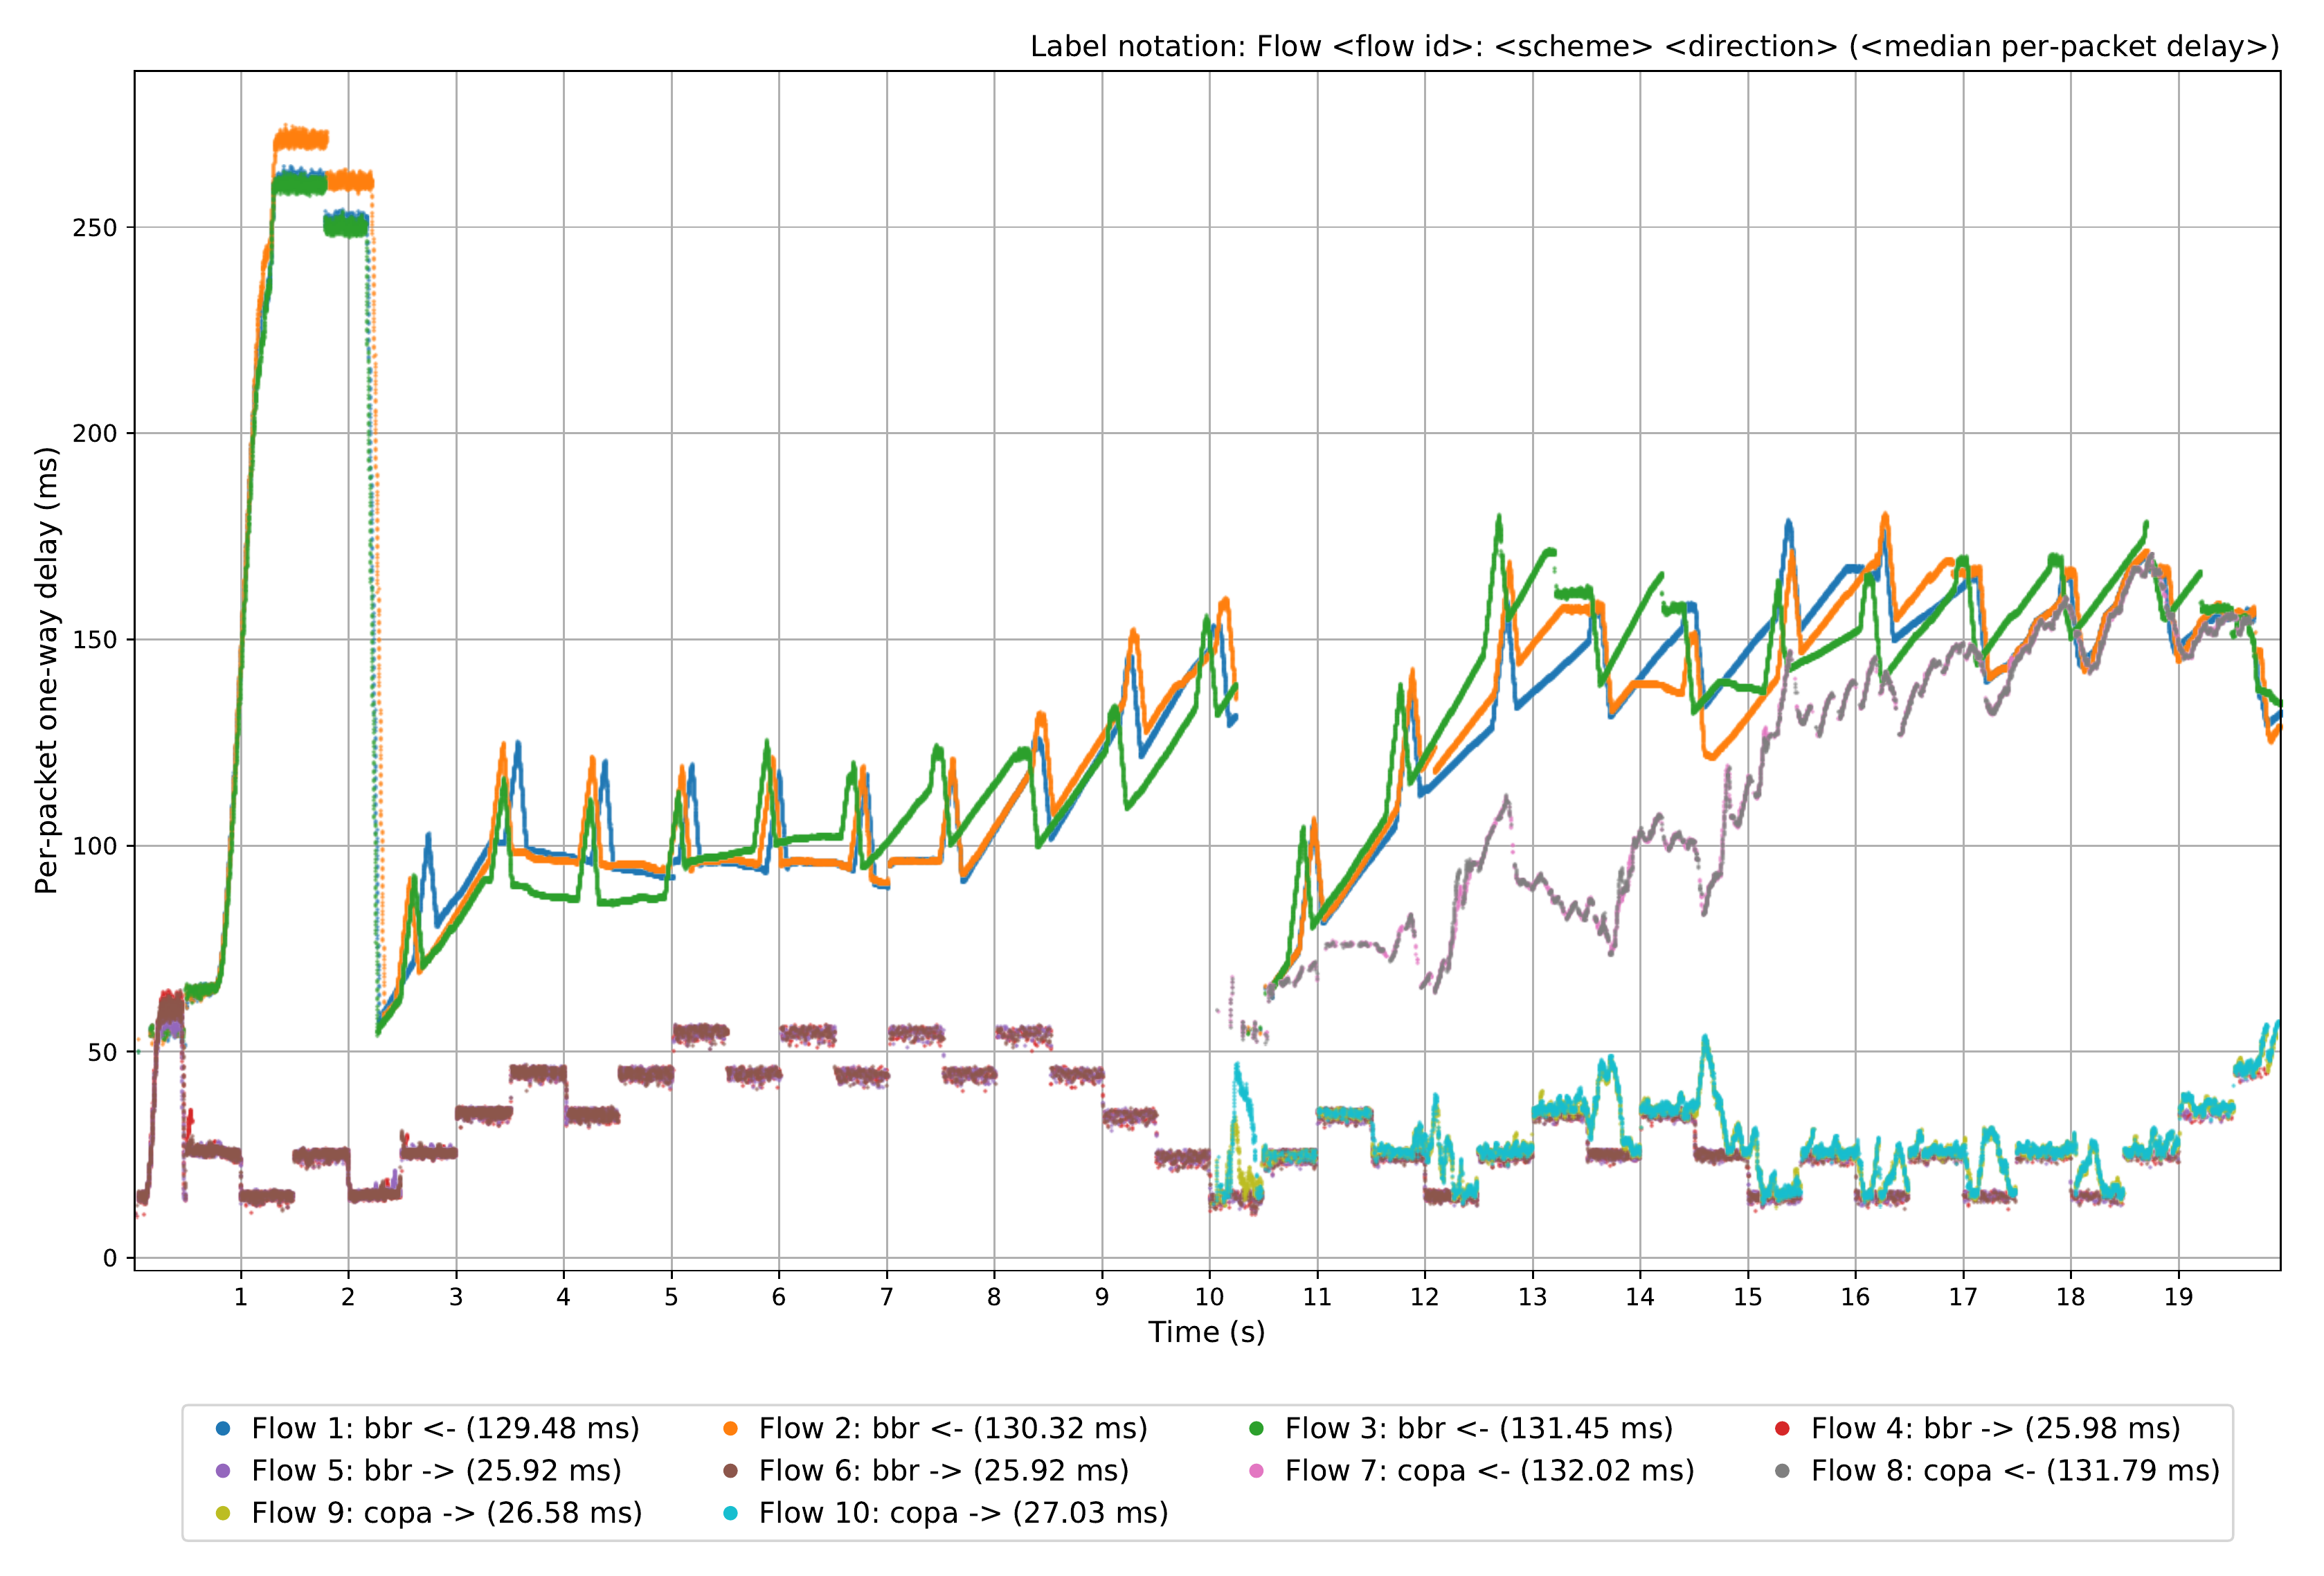}
\caption{Per-flow per-packet one-way delay plot.}
\label{fig:pfpptdelay}
\end{figure}

\newpage

\begin{lstlisting}[frame=single,basicstyle=\linespread{0.94}\ttfamily\normalsize,caption=Per-flow statistics.]
== Average and loss statistics ==

Average Jain's index  : 0.717070

-- Curve "Flow 1: bbr <-":
Average throughput    : 19.072241 Mbps
Average one-way delay : 130.876473 ms
Loss                  : 0.454414 %

-- Curve "Flow 2: bbr <-":
Average throughput    : 19.083428 Mbps
Average one-way delay : 132.495166 ms
Loss                  : 0.501920 %

-- Curve "Flow 3: bbr <-":
Average throughput    : 19.078041 Mbps
Average one-way delay : 131.729678 ms
Loss                  : 0.508129 %

-- Curve "Flow 4: bbr ->":
Average throughput    : 5.378910 Mbps
Average one-way delay : 30.715393 ms
Loss                  : 0.022758 %

-- Curve "Flow 5: bbr ->":
Average throughput    : 5.523644 Mbps
Average one-way delay : 30.366745 ms
Loss                  : 0.000000 %

-- Curve "Flow 6: bbr ->":
Average throughput    : 5.742734 Mbps
Average one-way delay : 30.576849 ms
Loss                  : 0.044449 %

-- Curve "Flow 7: copa <-":
Average throughput    : 4.121129 Mbps
Average one-way delay : 120.647484 ms
Loss                  : 5.027032 %

-- Curve "Flow 8: copa <-":
Average throughput    : 4.132335 Mbps
Average one-way delay : 120.812378 ms
Loss                  : 4.863382 %

-- Curve "Flow 9: copa ->":
Average throughput    : 8.163581 Mbps
Average one-way delay : 28.620982 ms
Loss                  : 0.278835 %

-- Curve "Flow 10: copa ->":
Average throughput    : 8.140077 Mbps
Average one-way delay : 29.411703 ms
Loss                  : 0.278835 %

===== Per-packet statistics =====

-- Curve "Flow 1: bbr <-":
Median per-packet one-way delay          : 129.477978 ms
Average per-packet one-way delay         : 130.876473 ms
95th percentile per-packet one-way delay : 232.173920 ms

-- Curve "Flow 2: bbr <-":
Median per-packet one-way delay          : 130.324125 ms
Average per-packet one-way delay         : 132.495166 ms
95th percentile per-packet one-way delay : 246.256113 ms

-- Curve "Flow 3: bbr <-":
Median per-packet one-way delay          : 131.448030 ms
Average per-packet one-way delay         : 131.729678 ms
95th percentile per-packet one-way delay : 228.887796 ms

-- Curve "Flow 4: bbr ->":
Median per-packet one-way delay          : 25.976896 ms
Average per-packet one-way delay         : 30.715393 ms
95th percentile per-packet one-way delay : 55.579901 ms

-- Curve "Flow 5: bbr ->":
Median per-packet one-way delay          : 25.920868 ms
Average per-packet one-way delay         : 30.366745 ms
95th percentile per-packet one-way delay : 55.373907 ms

-- Curve "Flow 6: bbr ->":
Median per-packet one-way delay          : 25.922060 ms
Average per-packet one-way delay         : 30.576849 ms
95th percentile per-packet one-way delay : 55.610895 ms

-- Curve "Flow 7: copa <-":
Median per-packet one-way delay          : 132.015944 ms
Average per-packet one-way delay         : 120.647484 ms
95th percentile per-packet one-way delay : 159.695148 ms

-- Curve "Flow 8: copa <-":
Median per-packet one-way delay          : 131.787062 ms
Average per-packet one-way delay         : 120.812378 ms
95th percentile per-packet one-way delay : 159.190893 ms

-- Curve "Flow 9: copa ->":
Median per-packet one-way delay          : 26.577950 ms
Average per-packet one-way delay         : 28.620982 ms
95th percentile per-packet one-way delay : 46.072006 ms

-- Curve "Flow 10: copa ->":
Median per-packet one-way delay          : 27.031898 ms
Average per-packet one-way delay         : 29.411703 ms
95th percentile per-packet one-way delay : 46.618938 ms
\end{lstlisting}

\section{Per-Scheme Plots and Statistics}

The commentary on the average rate plot~\ref{fig:psrate} can be found at the end of the section. The aggregation interval for all the  average plots in this section is 0.3 seconds.

\begin{figure}[h!]
\centering
\includegraphics[width=\textwidth]{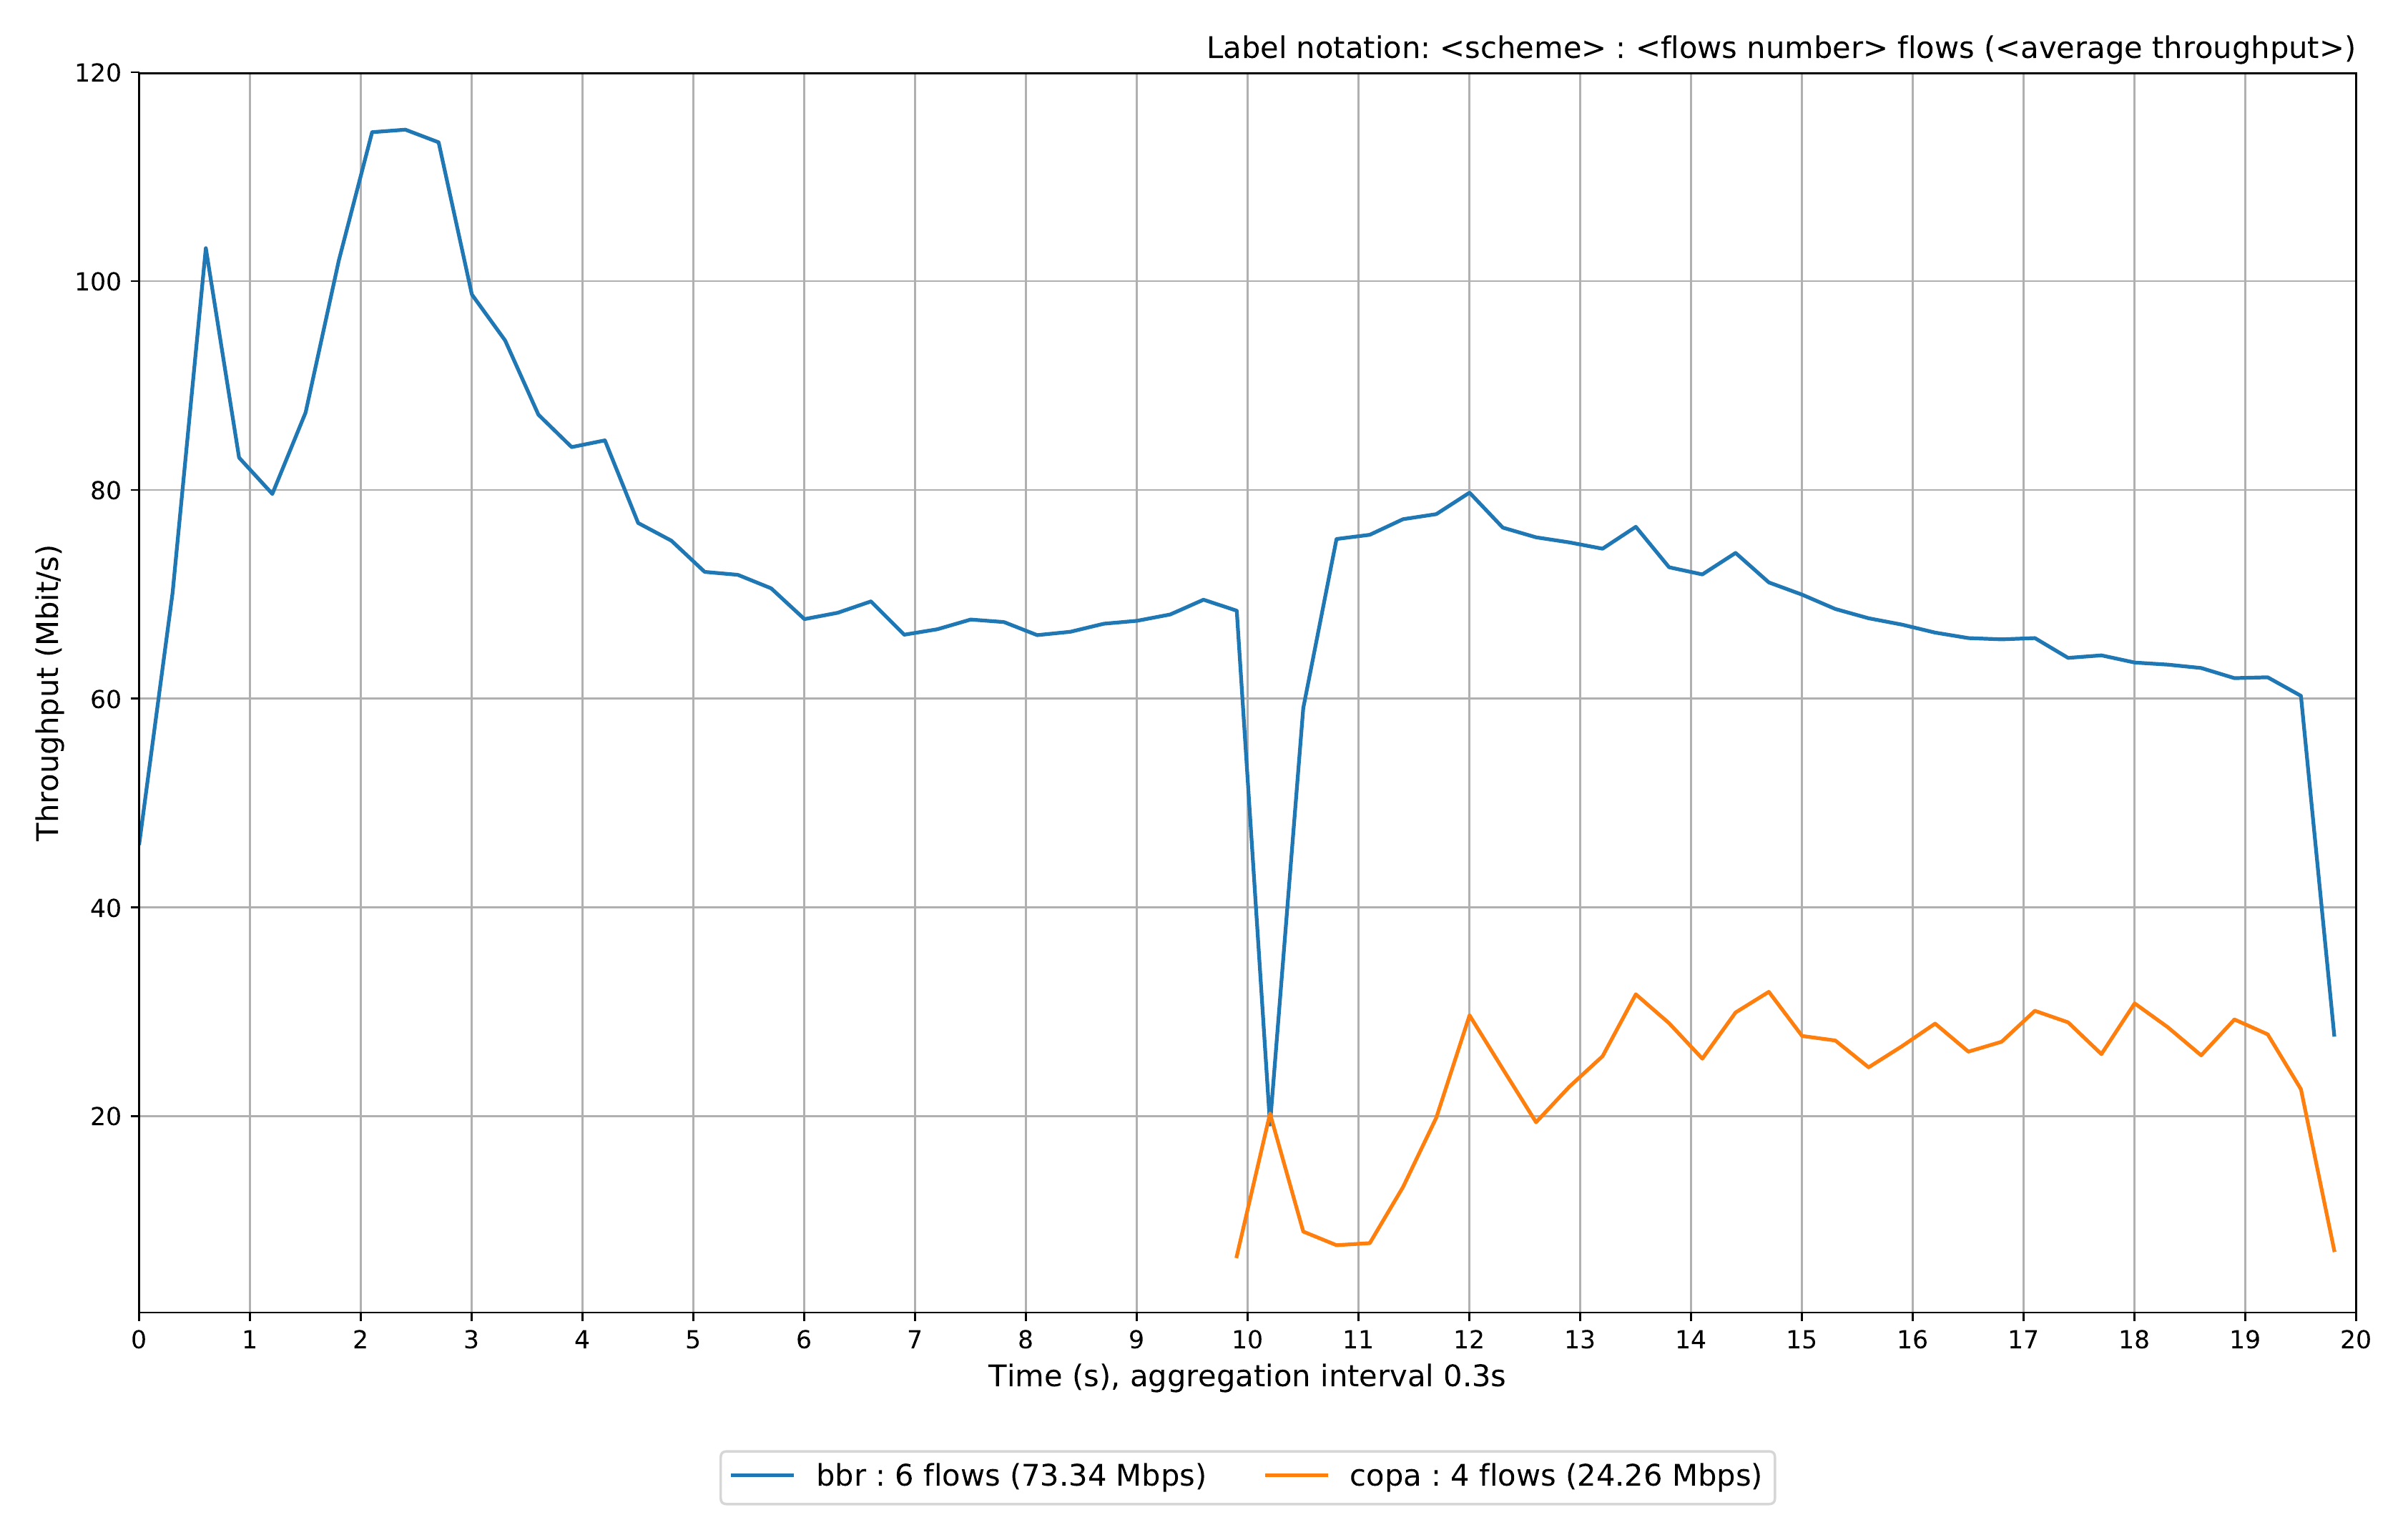}
\caption{Per-scheme average throughput plot.}
\label{fig:psrate}
\end{figure}

\vspace{0.4cm}

\begin{figure}[h!]
\centering
\includegraphics[width=\textwidth]{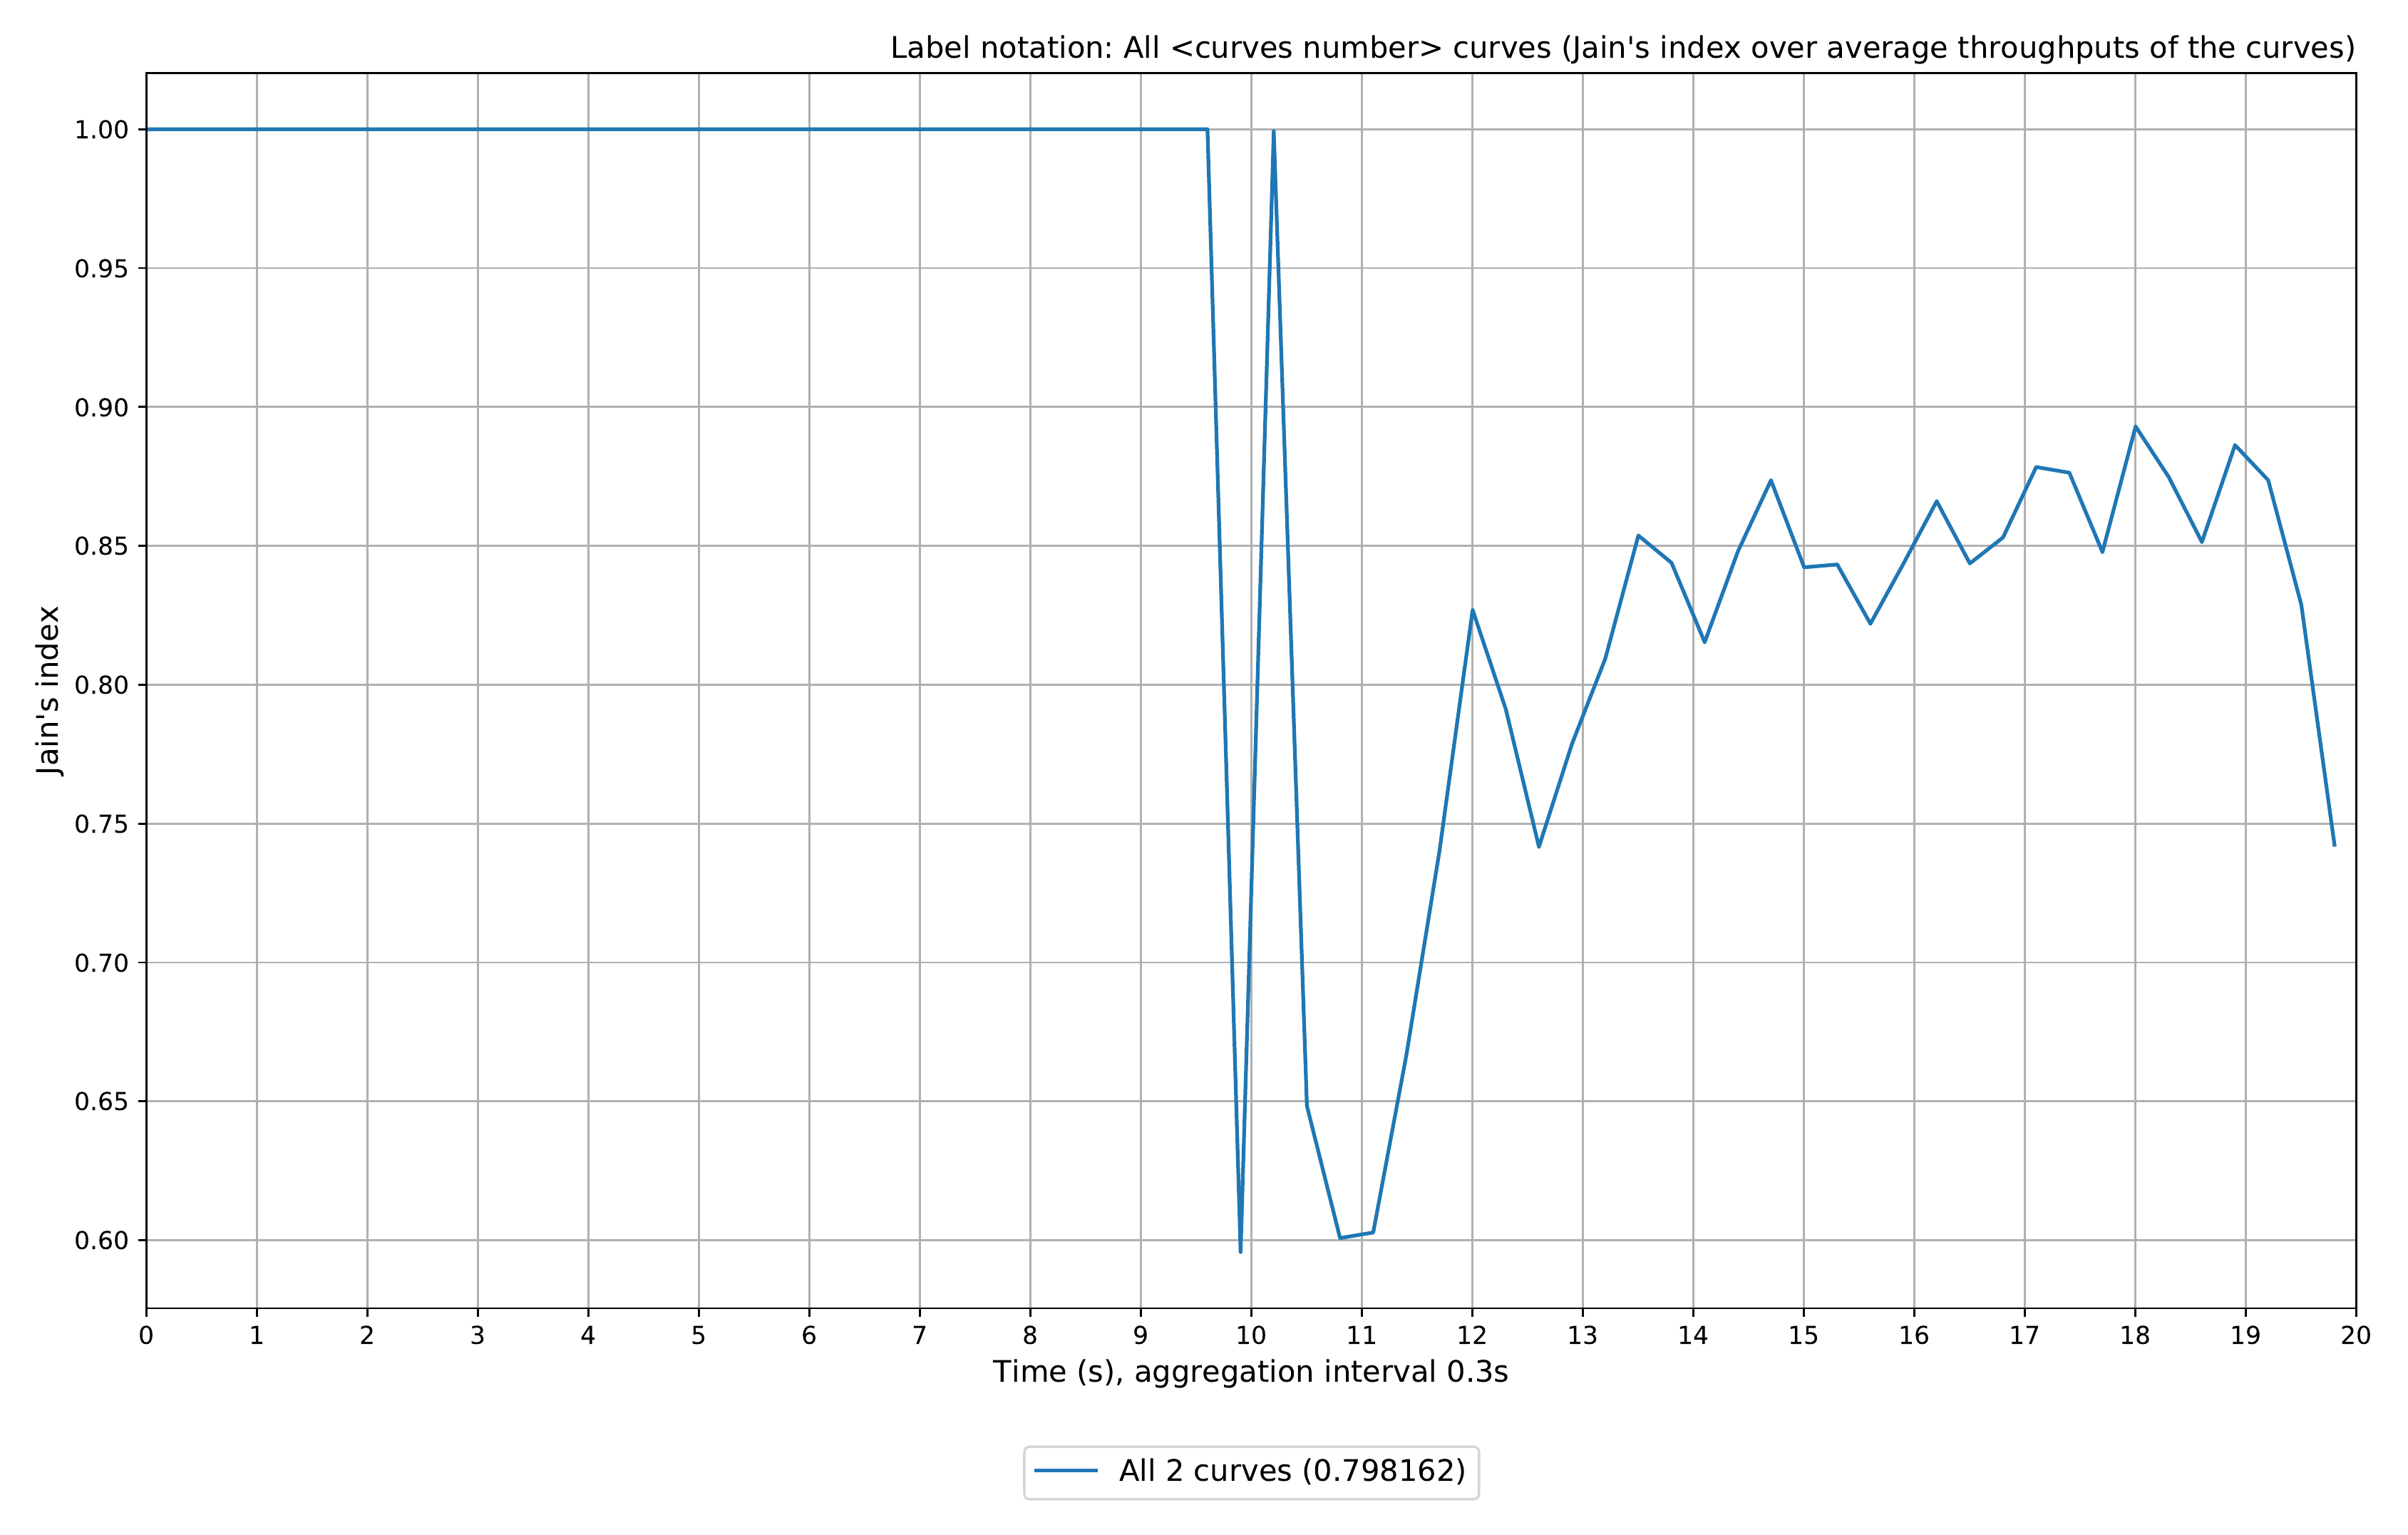}
\caption{Per-scheme average Jain's index plot.}
\end{figure}

\textcolor{white}{.}\\

\begin{figure}[h!]
\centering
\includegraphics[width=\textwidth]{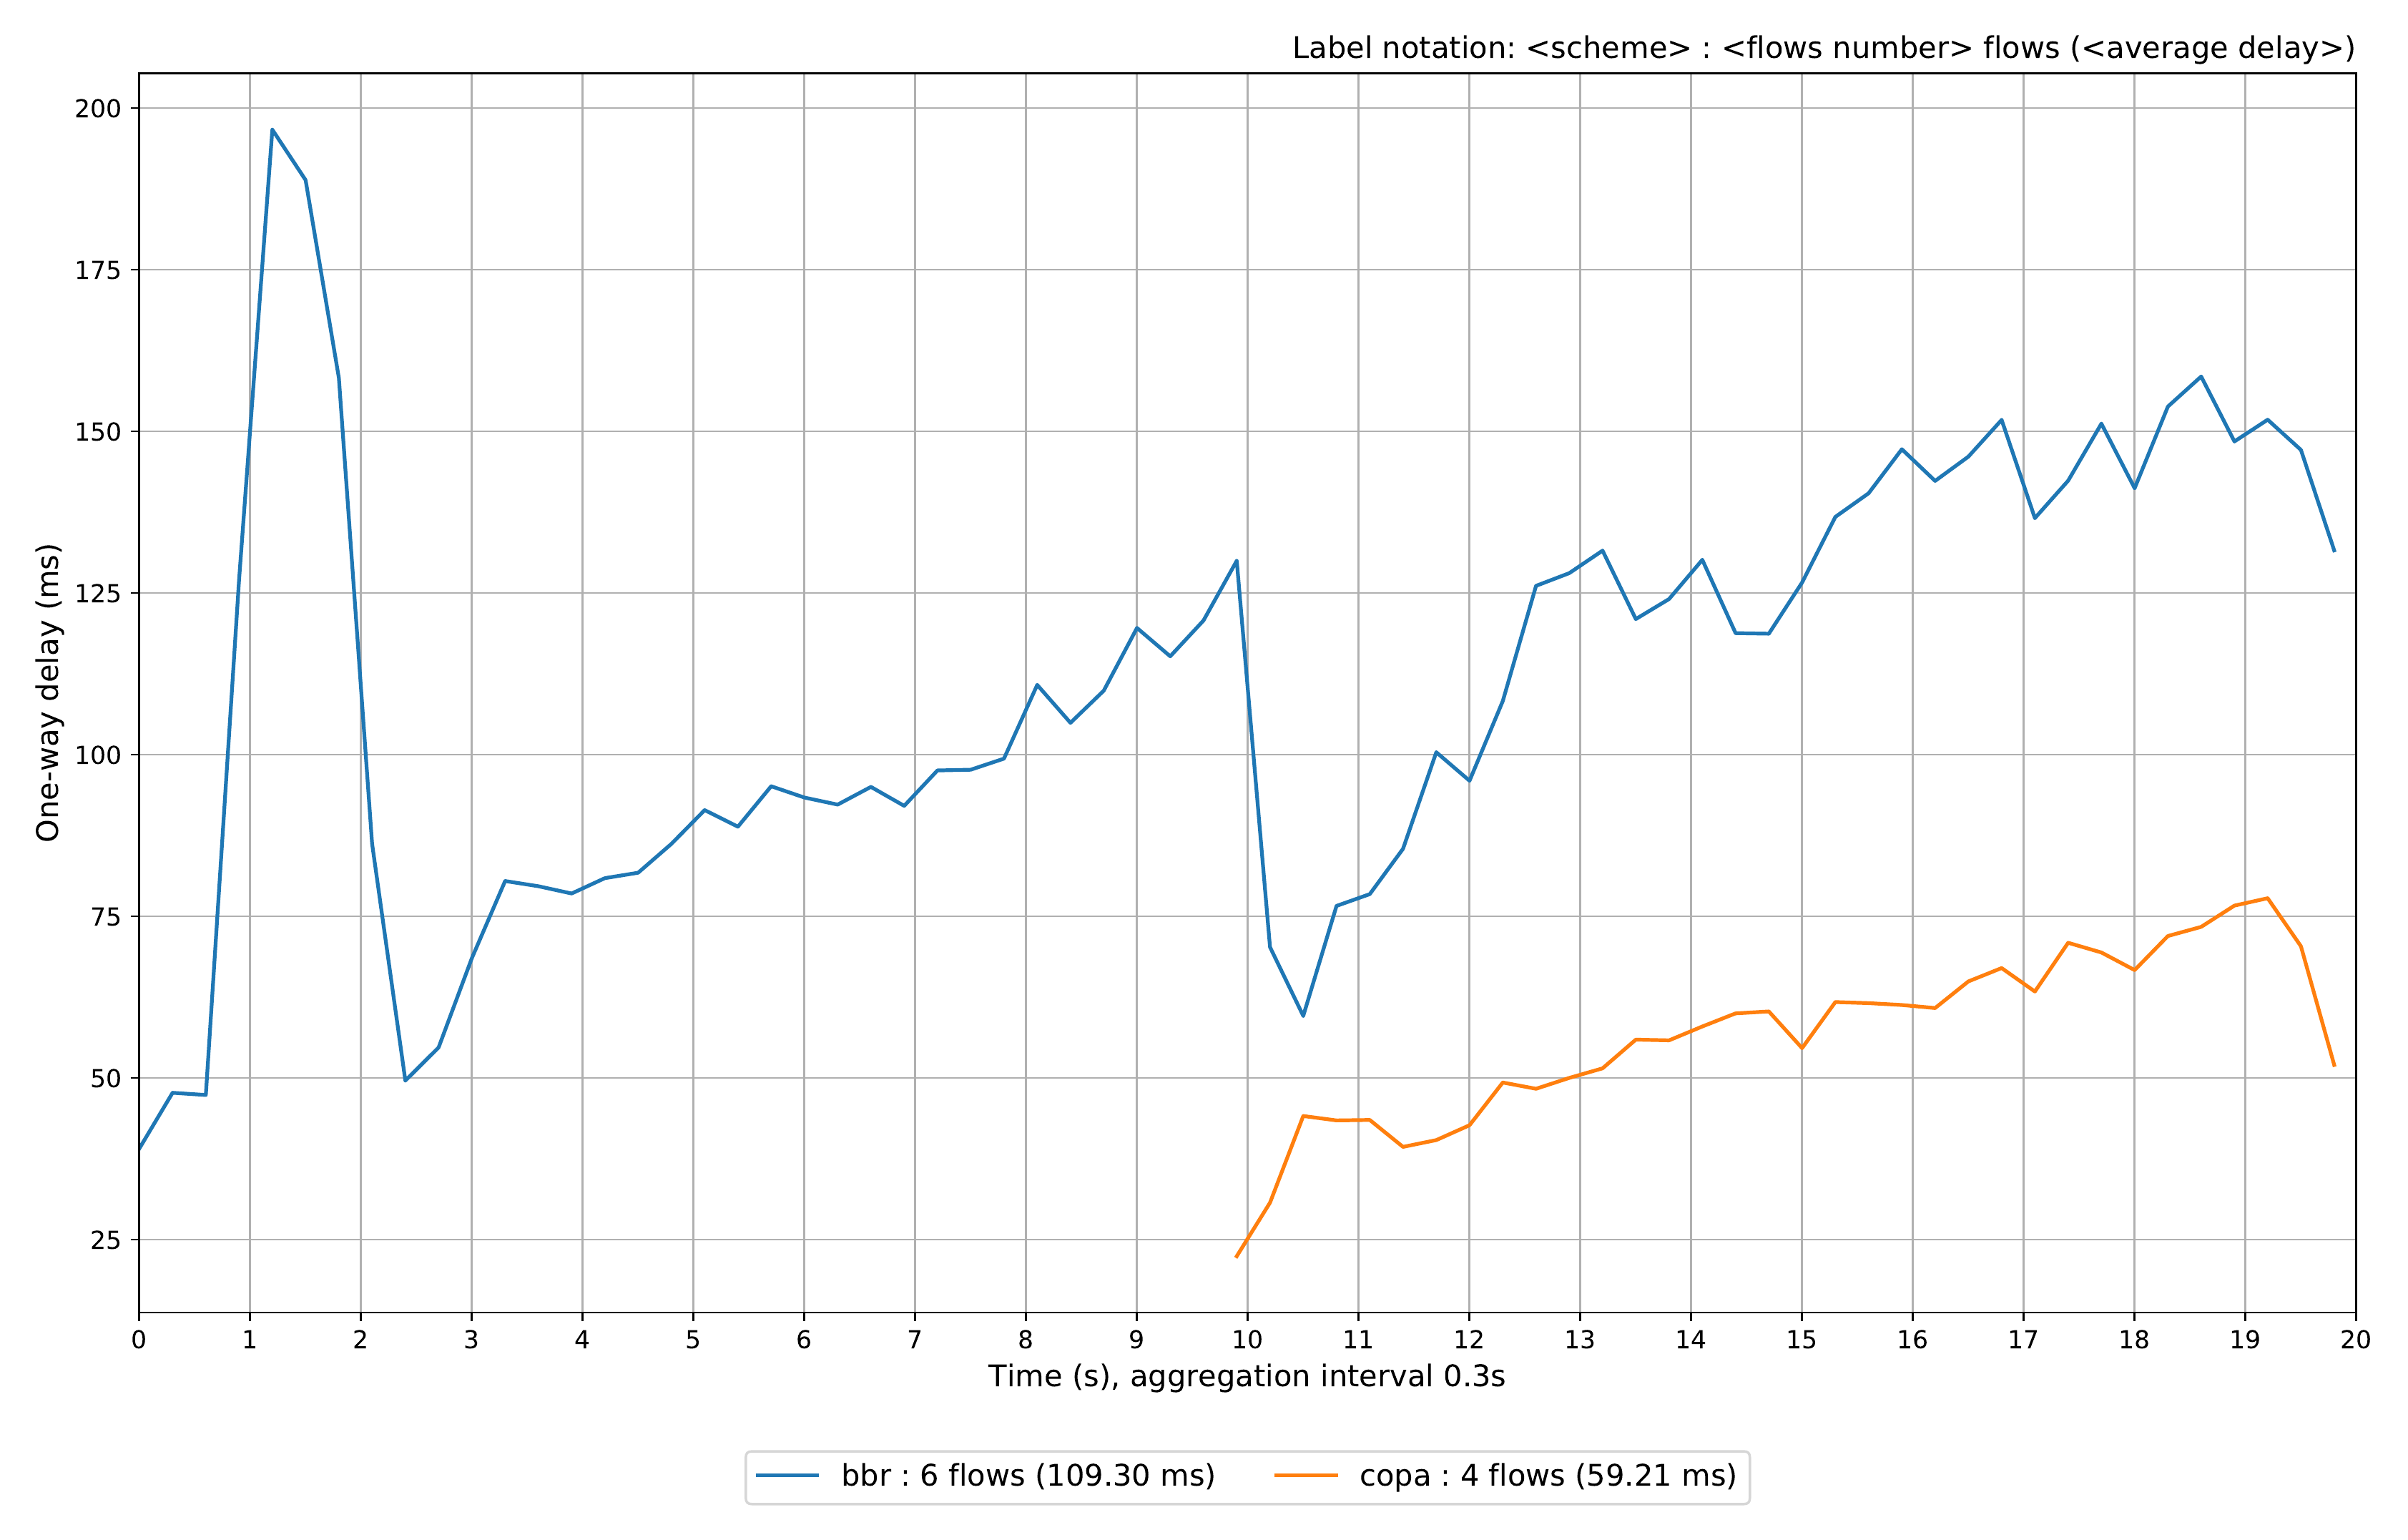}
\caption{Per-scheme average one-way delay plot.}
\end{figure}

\textcolor{white}{.}

\begin{figure}[h!]
\centering
\includegraphics[width=\textwidth]{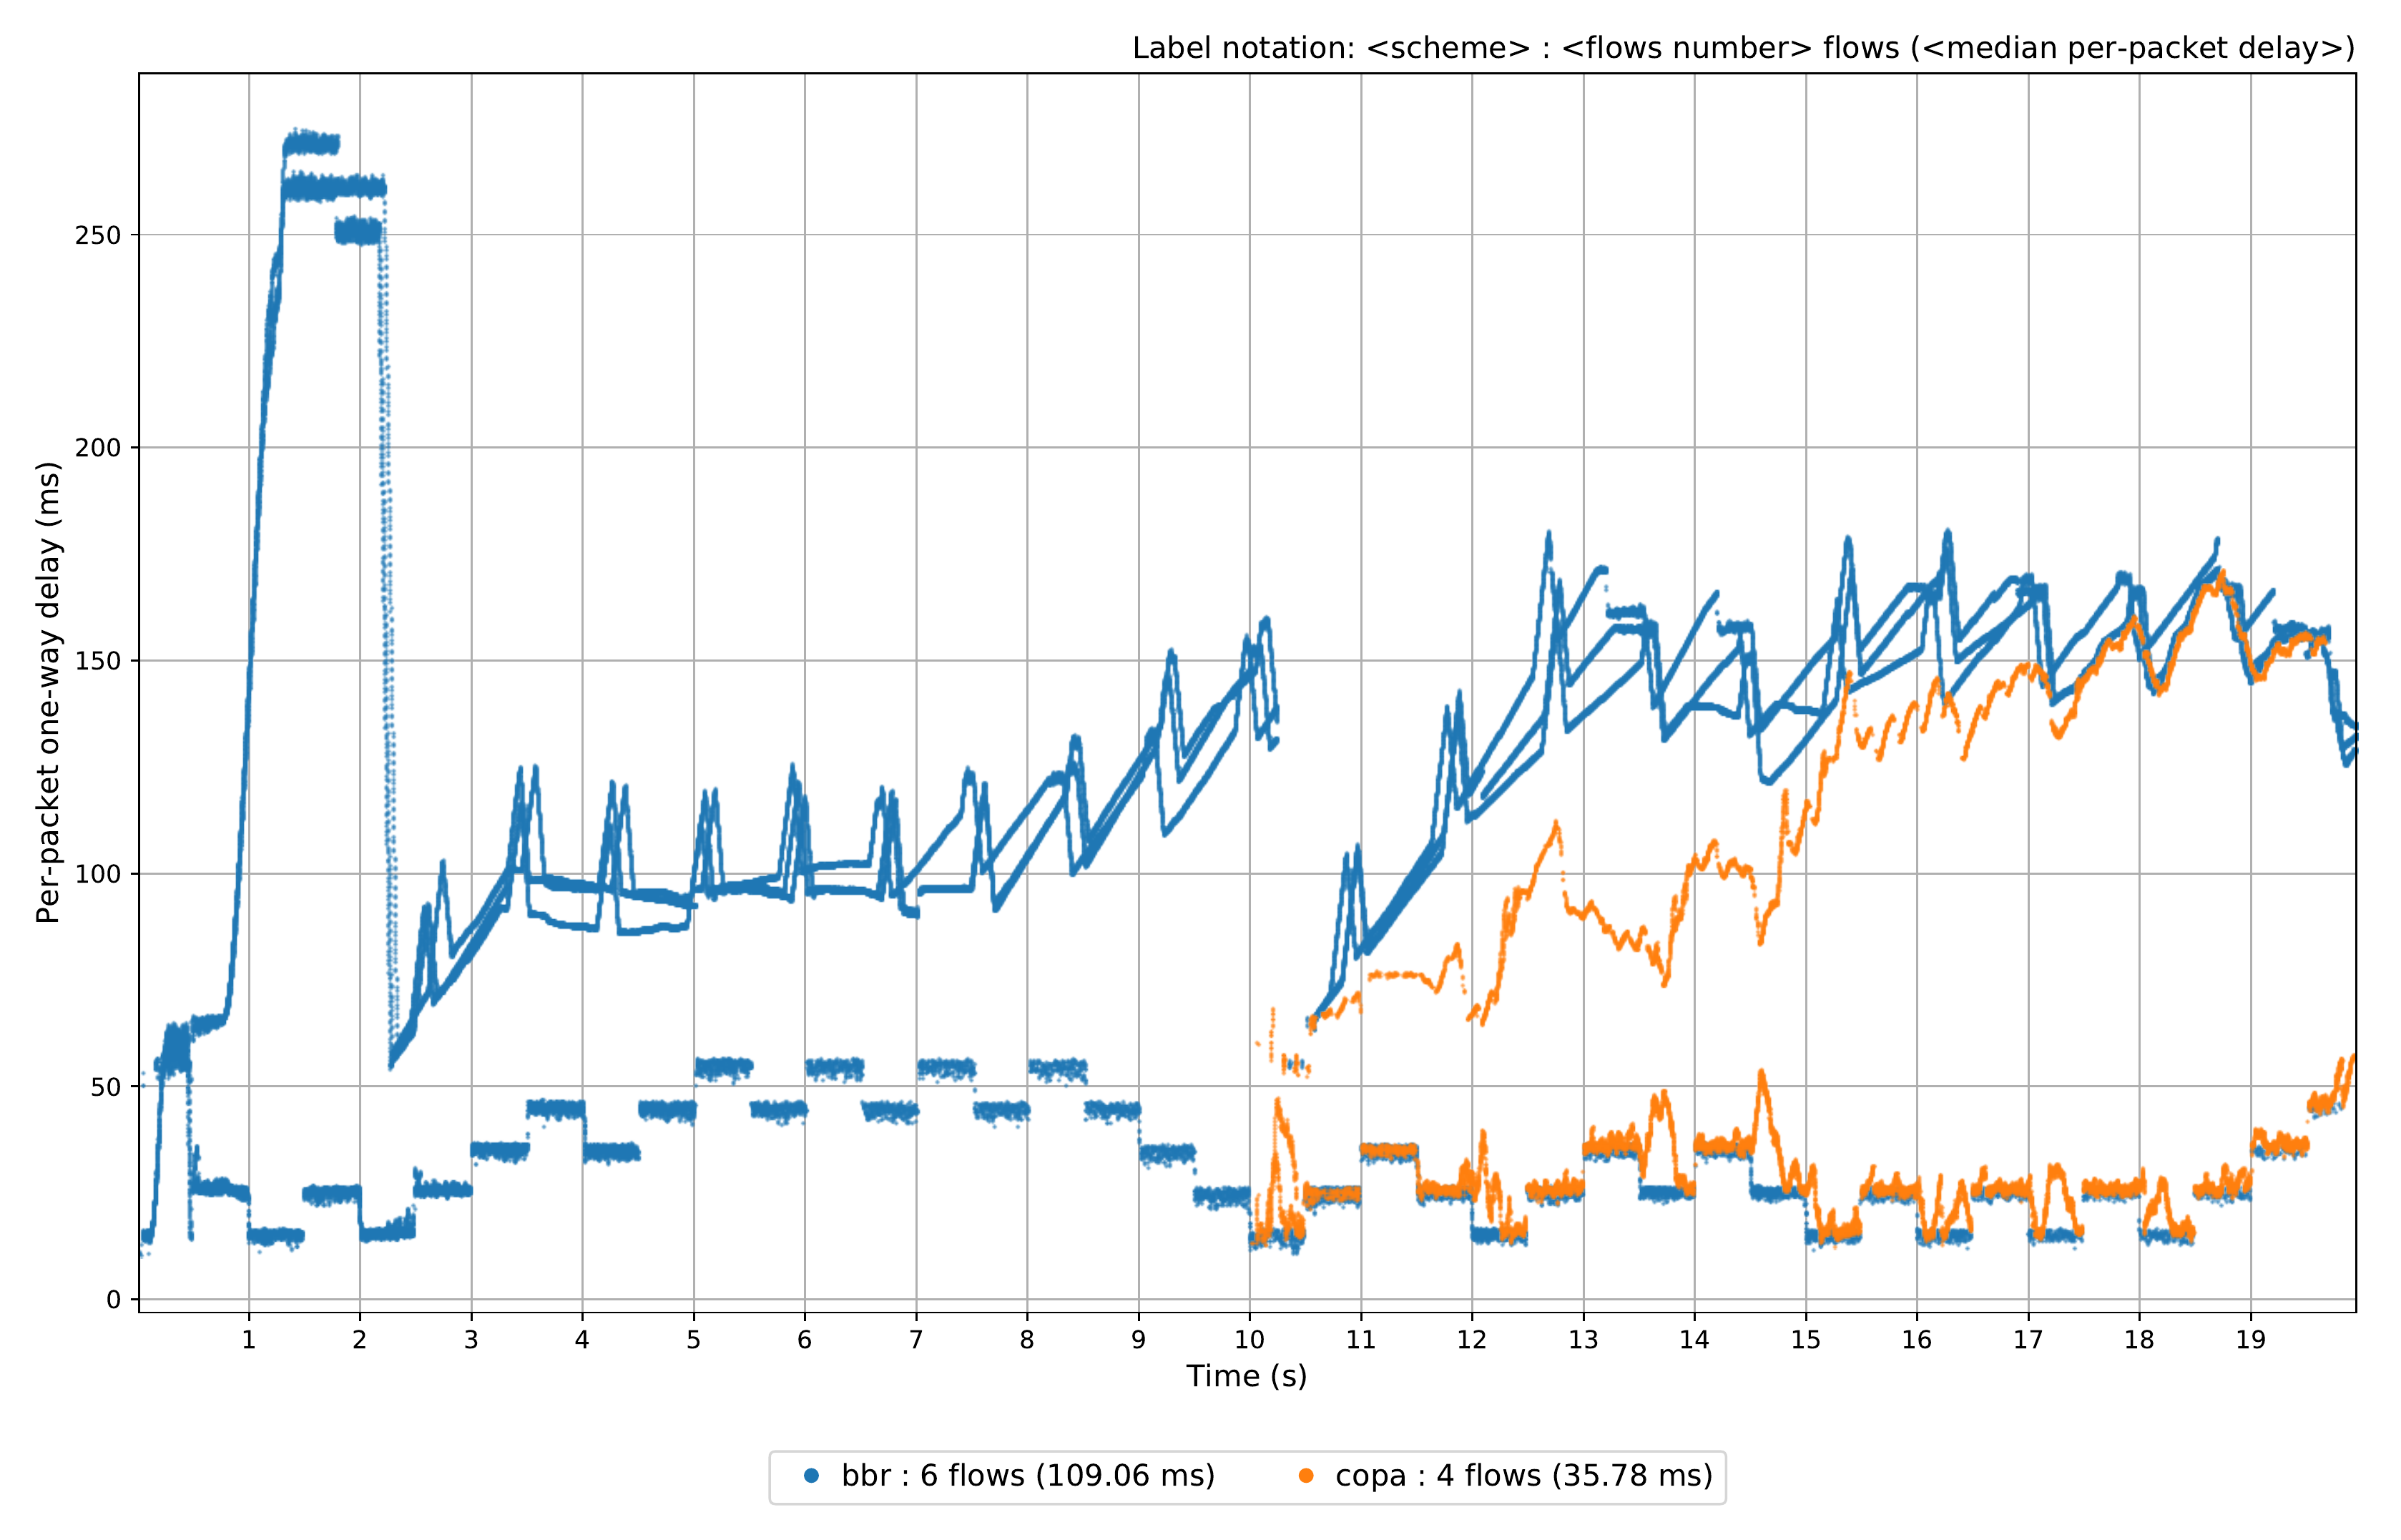}
\caption{Per-scheme per-packet one-way delay plot.}
\end{figure}

\newpage

\textcolor{white}{.}

\begin{lstlisting}[frame=single,basicstyle=\linespread{1}\ttfamily\normalsize,caption=Per-scheme statistics.]
== Average and loss statistics ==

Average Jain's index  : 0.798162

-- Curve "bbr : 6 flows":
Average throughput    : 73.340494 Mbps
Average one-way delay : 109.298397 ms
Loss                  : 0.385401 %

-- Curve "copa : 4 flows":
Average throughput    : 24.260061 Mbps
Average one-way delay : 59.213476 ms
Loss                  : 1.864832 %

===== Per-packet statistics =====

-- Curve "bbr : 6 flows":
Median per-packet one-way delay          : 109.058142 ms
Average per-packet one-way delay         : 109.298397 ms
95th percentile per-packet one-way delay : 176.163912 ms

-- Curve "copa : 4 flows":
Median per-packet one-way delay          : 35.775185 ms
Average per-packet one-way delay         : 59.213476 ms
95th percentile per-packet one-way delay : 152.766943 ms
\end{lstlisting}
\bigbreak
\bigbreak
The three leftward and the three rightward TCP BBR flows can have at maximum $6 \cdot 20=120$ Mbit/s rate together. This is the achievable rate because the bandwidth of the central link in both directions is $2 \cdot 70=140$ Mbit/s. Analogously, the two leftward and the two rightward Copa flows can have at maximum $4 \cdot 10=40$ Mbit/s rate. The conclusions are reflected in the average rate plot~\ref{fig:psrate}.

\newpage

\section{Per-Direction Plots and Statistics}

In this section, the aggregation interval of all the three average plots is 0.1 seconds.

\begin{figure}[h!]
\centering
\includegraphics[width=\textwidth]{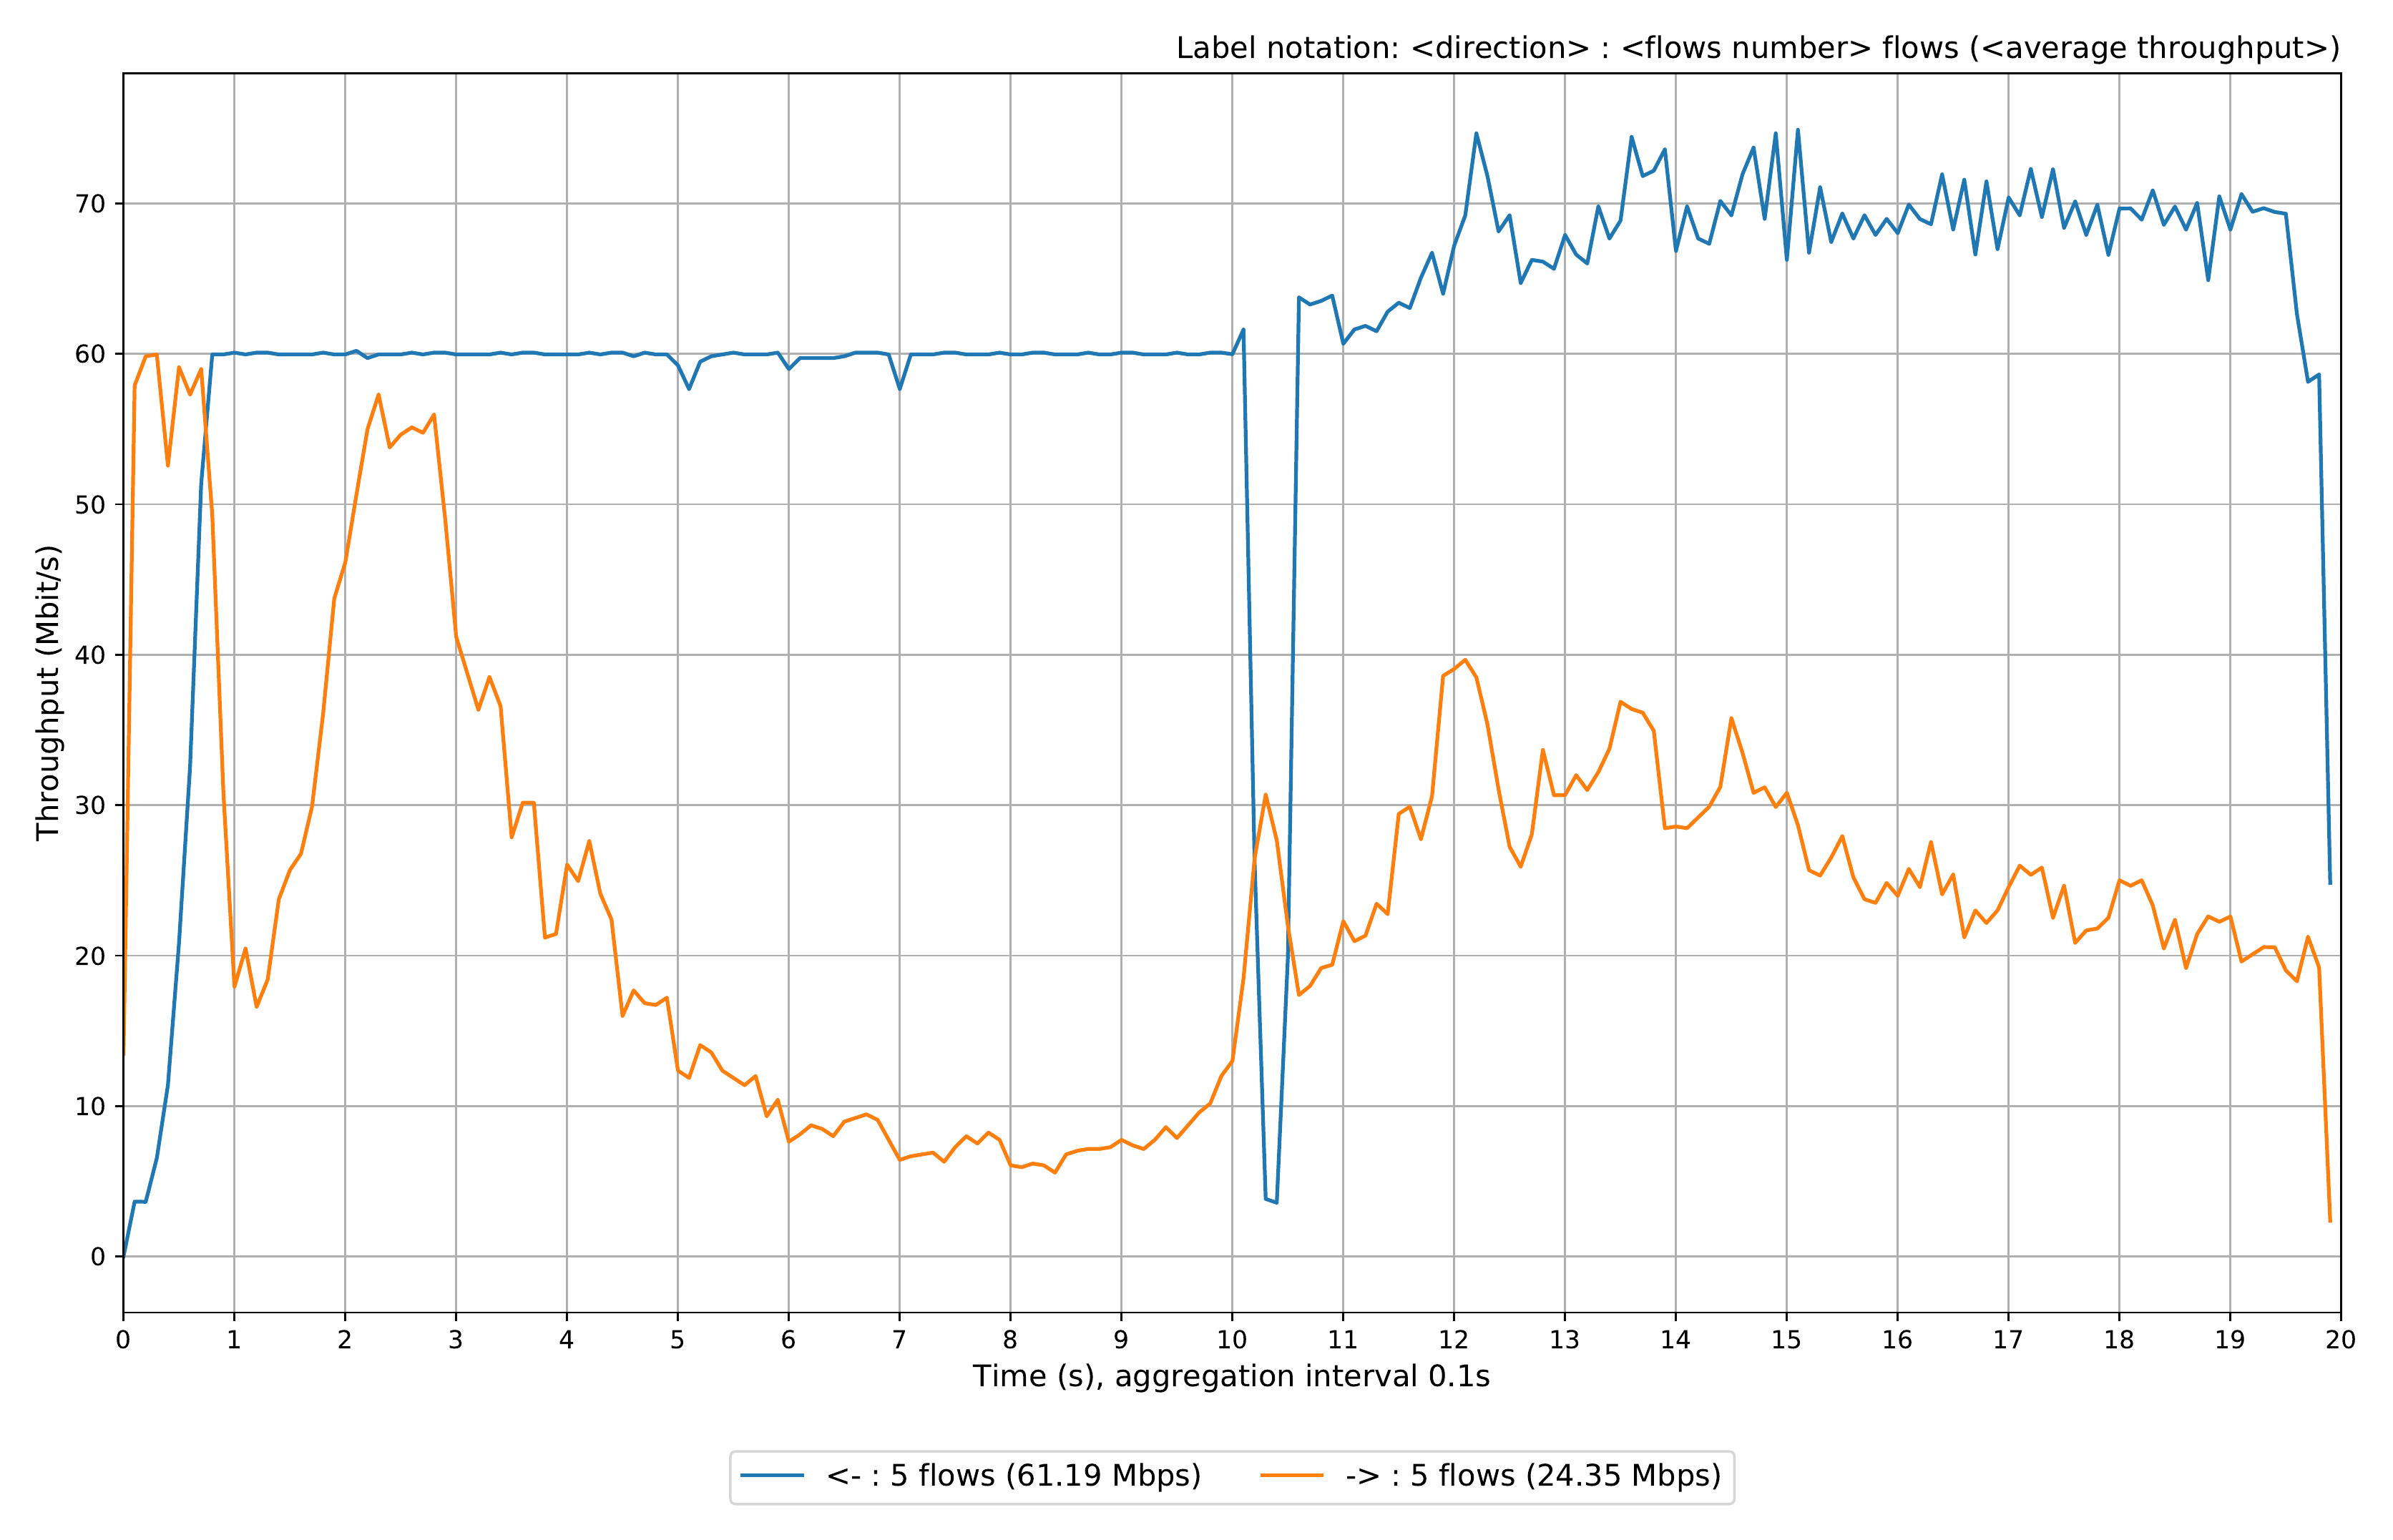}
\caption{Per-direction average throughput plot.}
\label{fig:pdrate}
\end{figure}

\vspace{0.5cm}

\begin{figure}[h!]
\centering
\includegraphics[width=\textwidth]{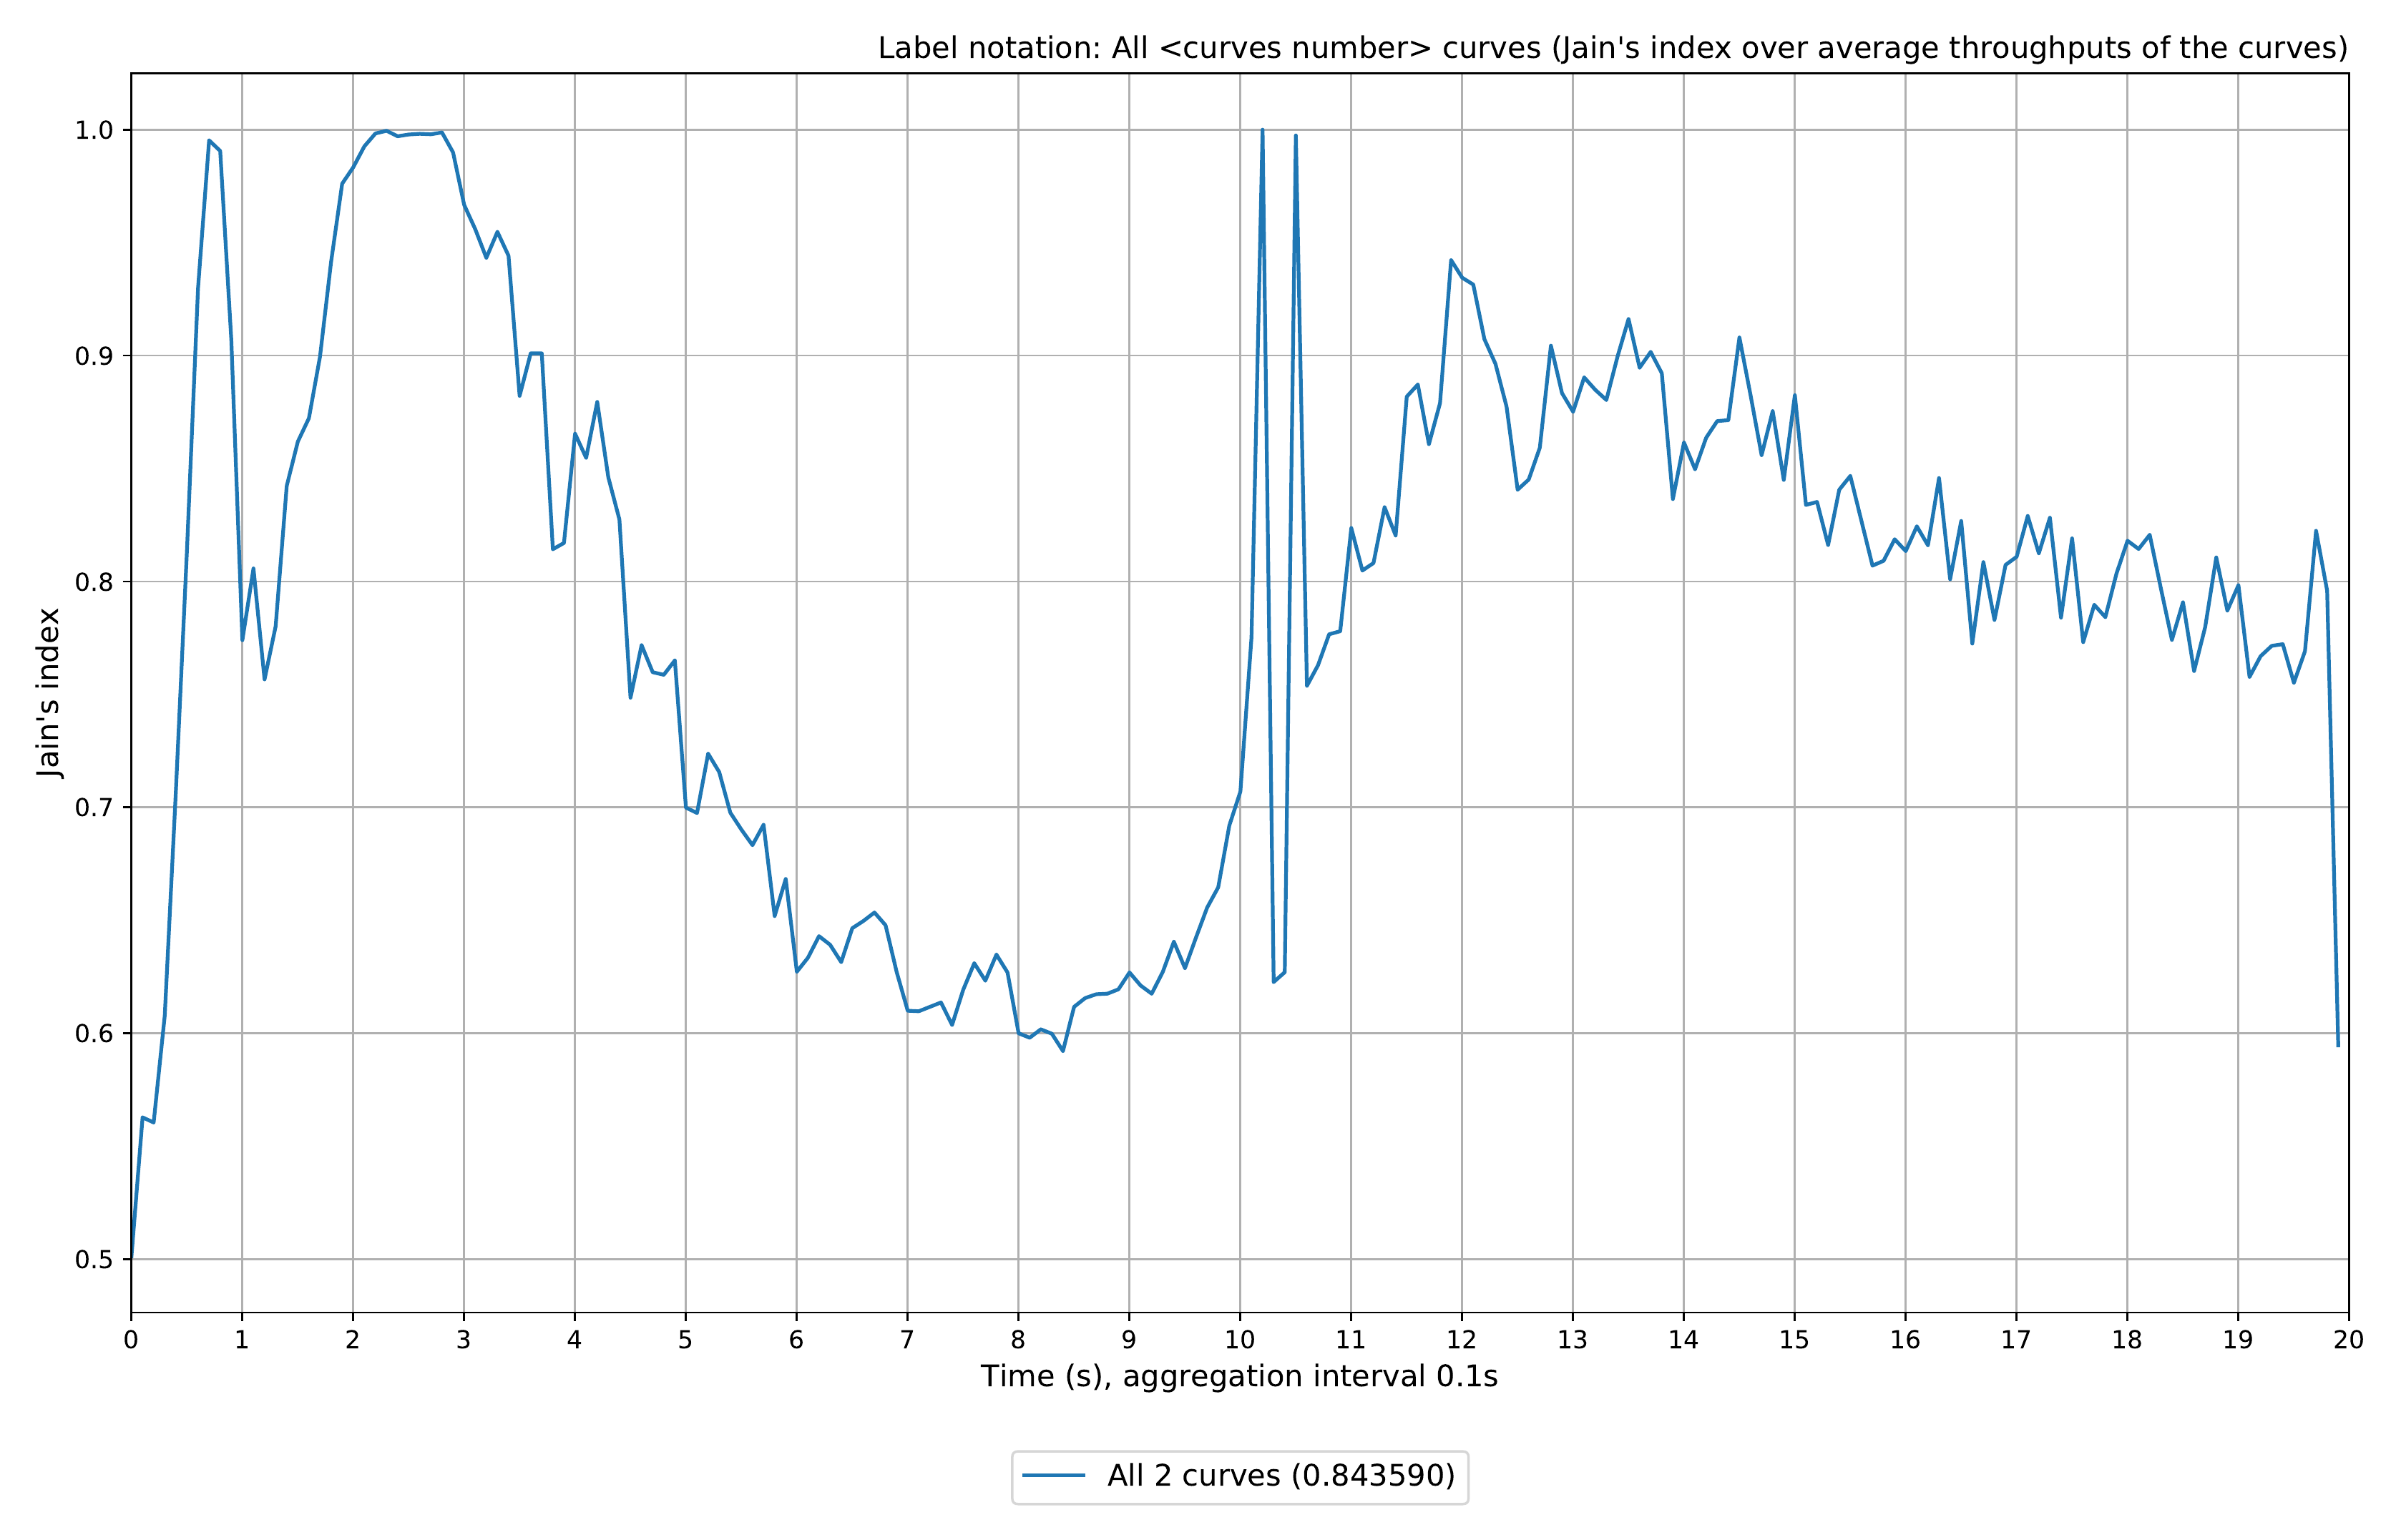}
\caption{Per-direction average Jain's index plot.}
\end{figure}

With the smaller aggregation interval, the average one-way delay plot~\ref{fig:pdavgdelay} looks even more similar to the per-packet one-way delay plot~\ref{fig:pdpptdelay}.

\begin{figure}[h!]
\centering
\includegraphics[width=\textwidth]{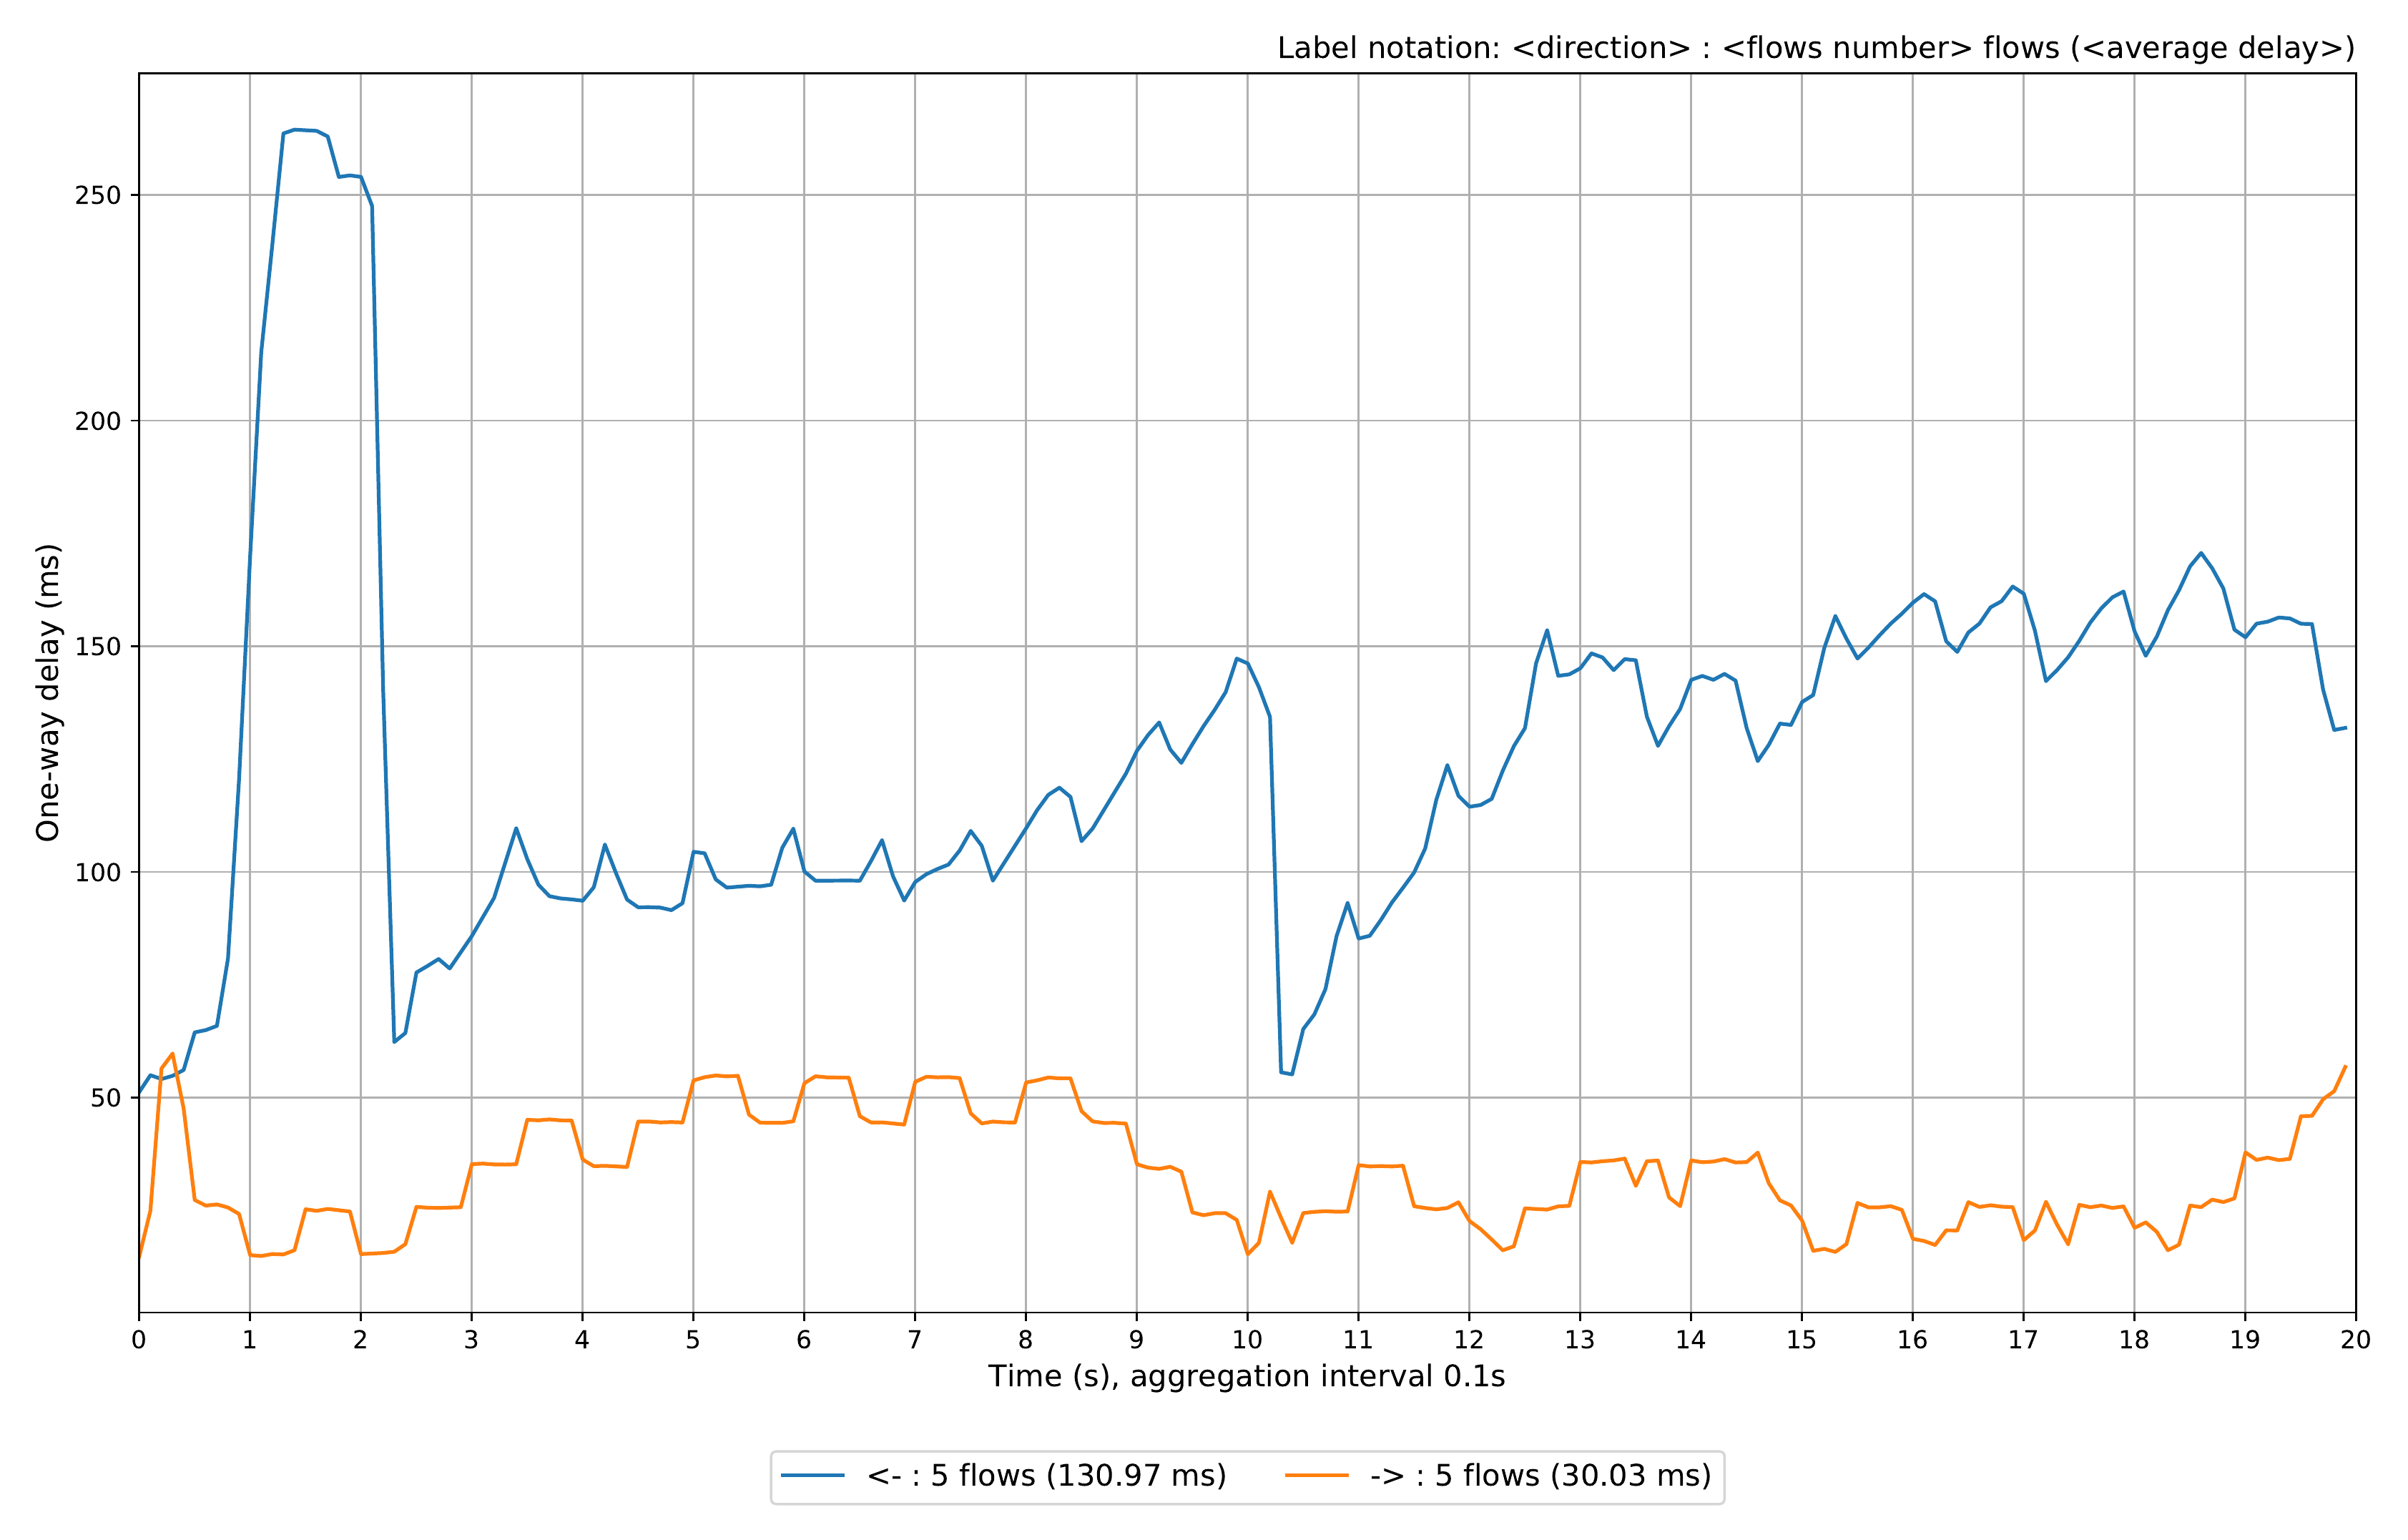}
\caption{Per-direction average one-way delay plot.}
\label{fig:pdavgdelay}
\end{figure}

\textcolor{white}{.}

\begin{figure}[h!]
\centering
\includegraphics[width=\textwidth]{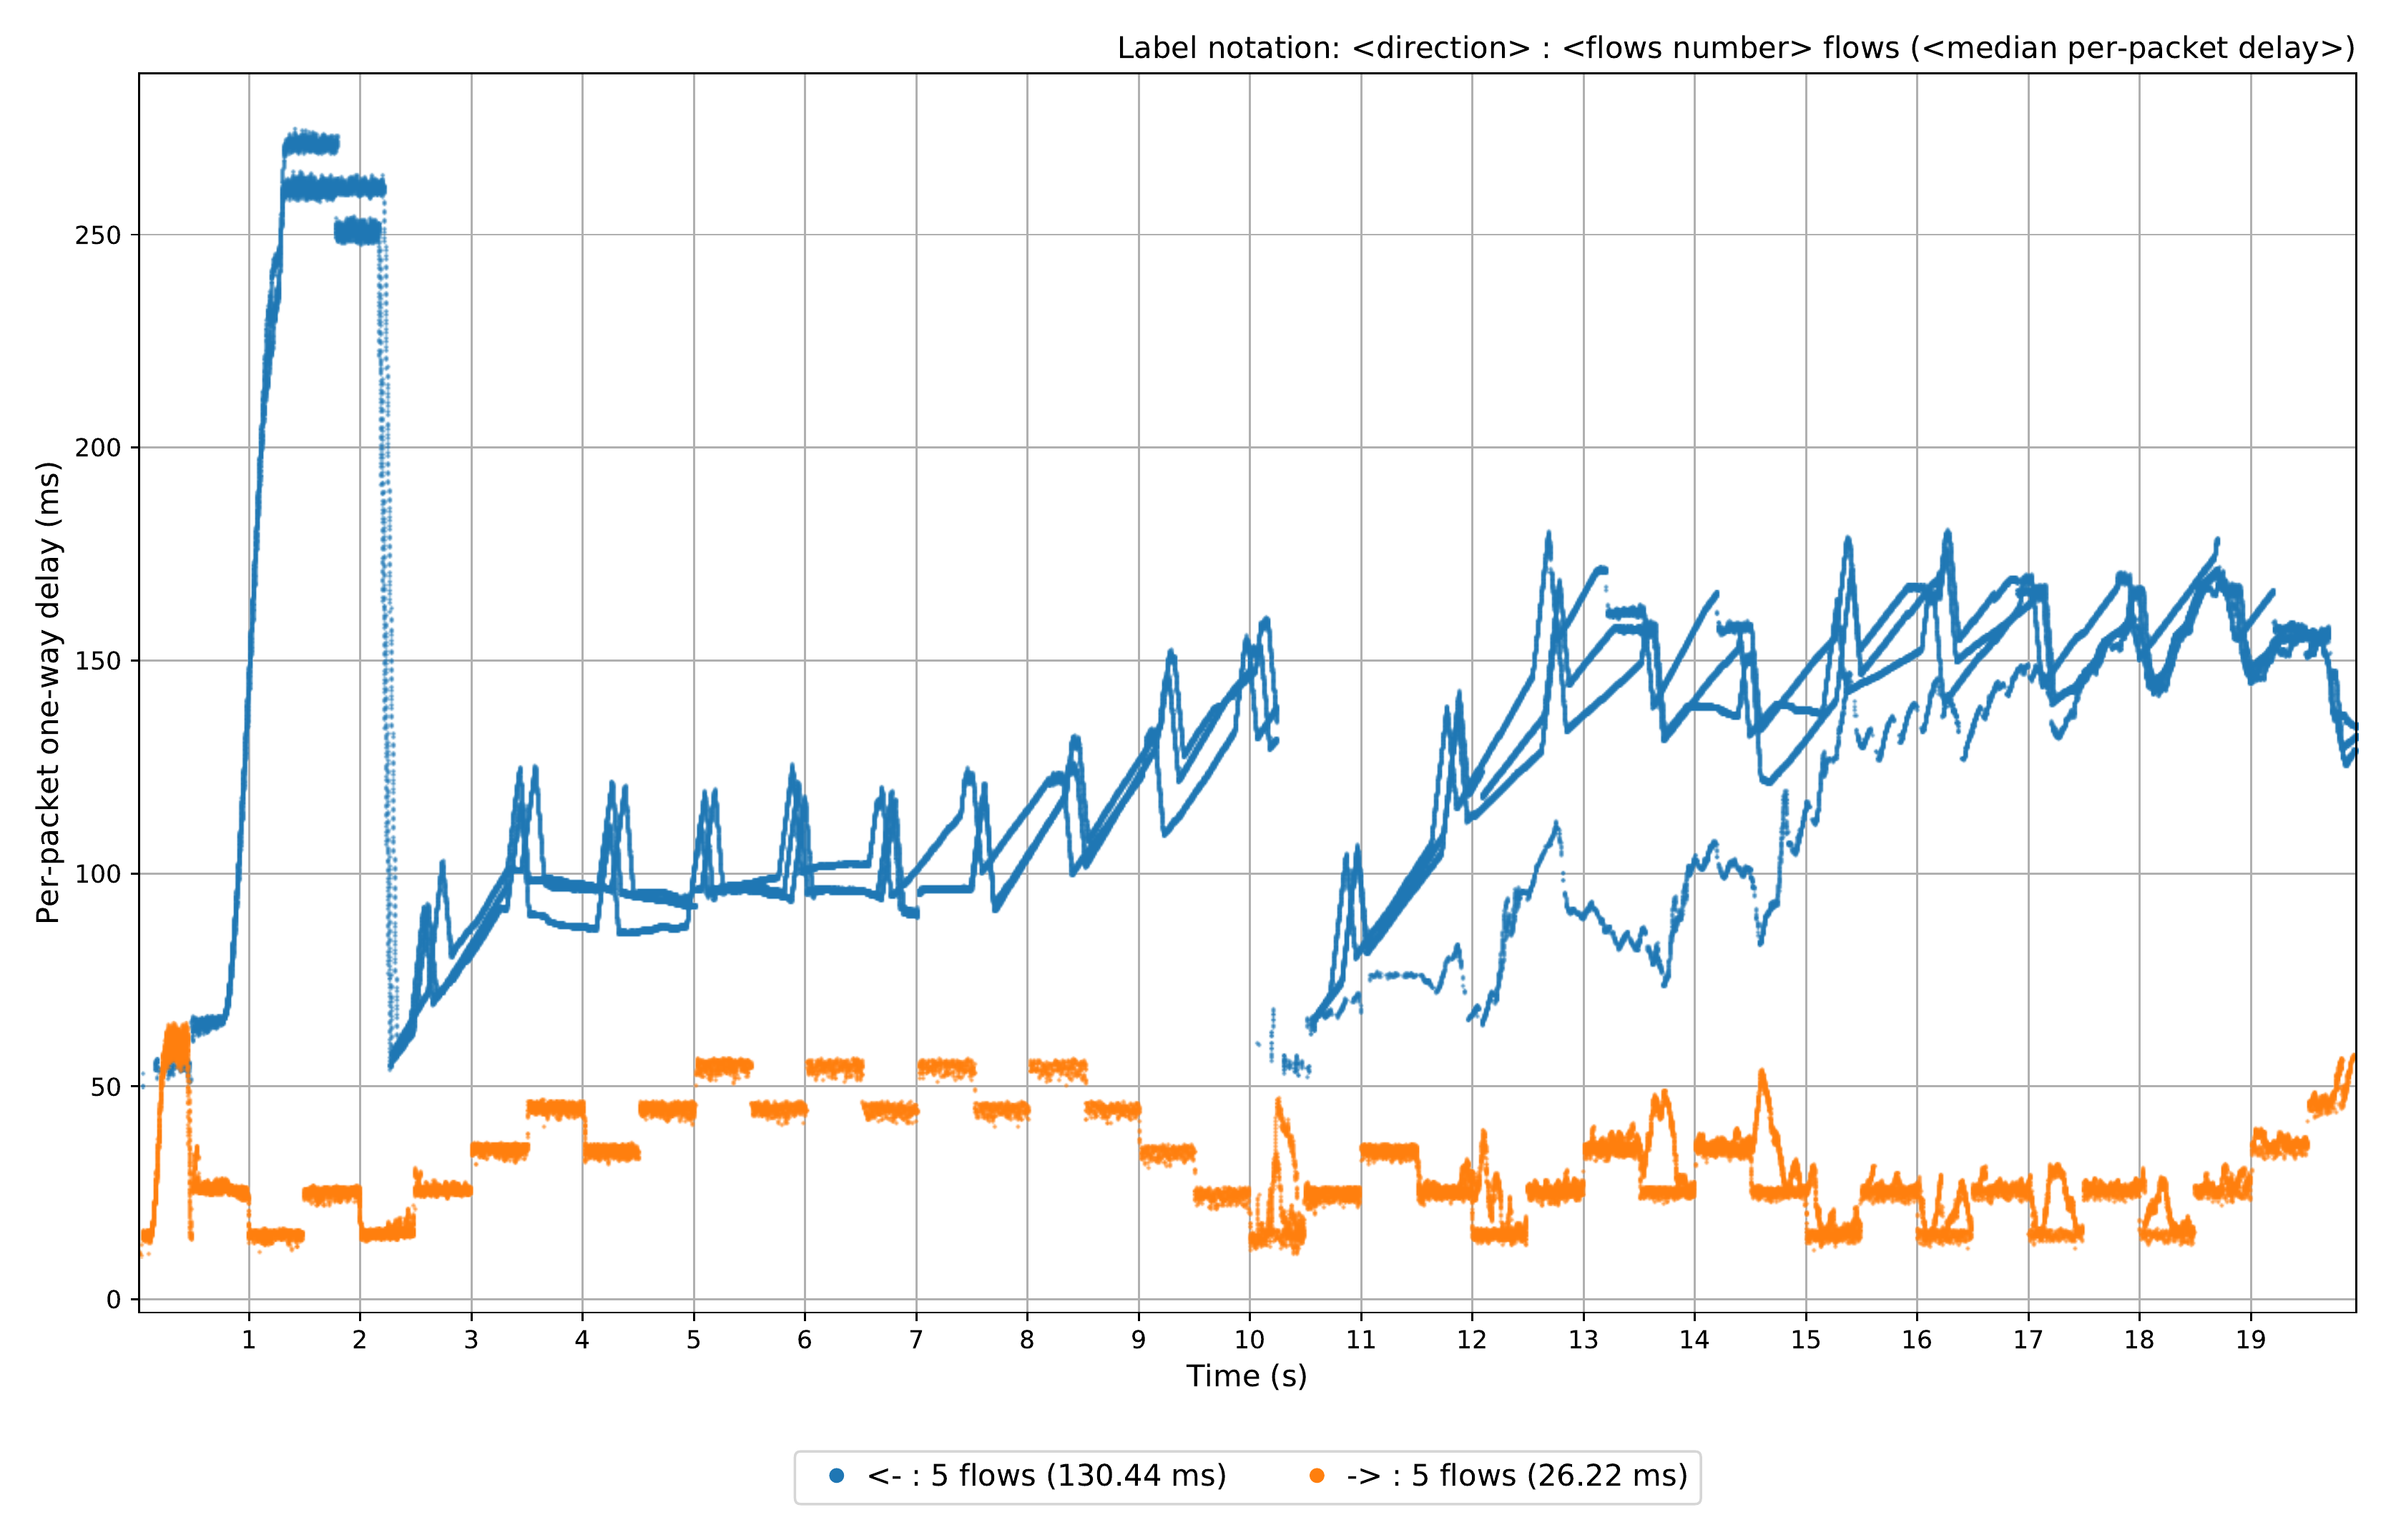}
\caption{Per-direction per-packet one-way delay plot.}
\label{fig:pdpptdelay}
\end{figure}

\newpage

\begin{lstlisting}[frame=single,basicstyle=\linespread{1}\ttfamily\normalsize,caption=Per-direction statistics.]
== Average and loss statistics ==

Average Jain's index  : 0.843590

-- Curve "<- : 5 flows":
Average throughput    : 61.187288 Mbps
Average one-way delay : 130.973213 ms
Loss                  : 0.790351 %

-- Curve "-> : 5 flows":
Average throughput    : 24.353883 Mbps
Average one-way delay : 30.034458 ms
Loss                  : 0.107786 %

===== Per-packet statistics =====

-- Curve "<- : 5 flows":
Median per-packet one-way delay          : 130.439043 ms
Average per-packet one-way delay         : 130.973213 ms
95th percentile per-packet one-way delay : 224.978924 ms

-- Curve "-> : 5 flows":
Median per-packet one-way delay          : 26.221037 ms
Average per-packet one-way delay         : 30.034458 ms
95th percentile per-packet one-way delay : 54.371119 ms
\end{lstlisting}
\bigbreak
\bigbreak

During the first ten seconds of the runtime, two groups of three BBR flows run into both directions. The rate of each group is limited to $3 \cdot 20=60$ Mbit/s. In ten seconds two pairs of two Copa flows are started to run into both directions. Therefore, the  rate of the five flows running into the same direction could be $60 + 2 \cdot 10 = 80$ Mbit/s but is limited by the 70 Mbit/s bandwidth of the central link. In the average rate plot~\ref{fig:pdrate}, the described behavior is better seen for the leftward direction, even though there are some peaks exceeding 70 Mbit/s.

\newpage

\section{Per-Scheme-and-Direction Plots and Statistics}

In this section, the aggregation interval of the average one-way delay plot is 0.01 seconds.

\begin{figure}[h!]
\centering
\includegraphics[width=0.99\textwidth]{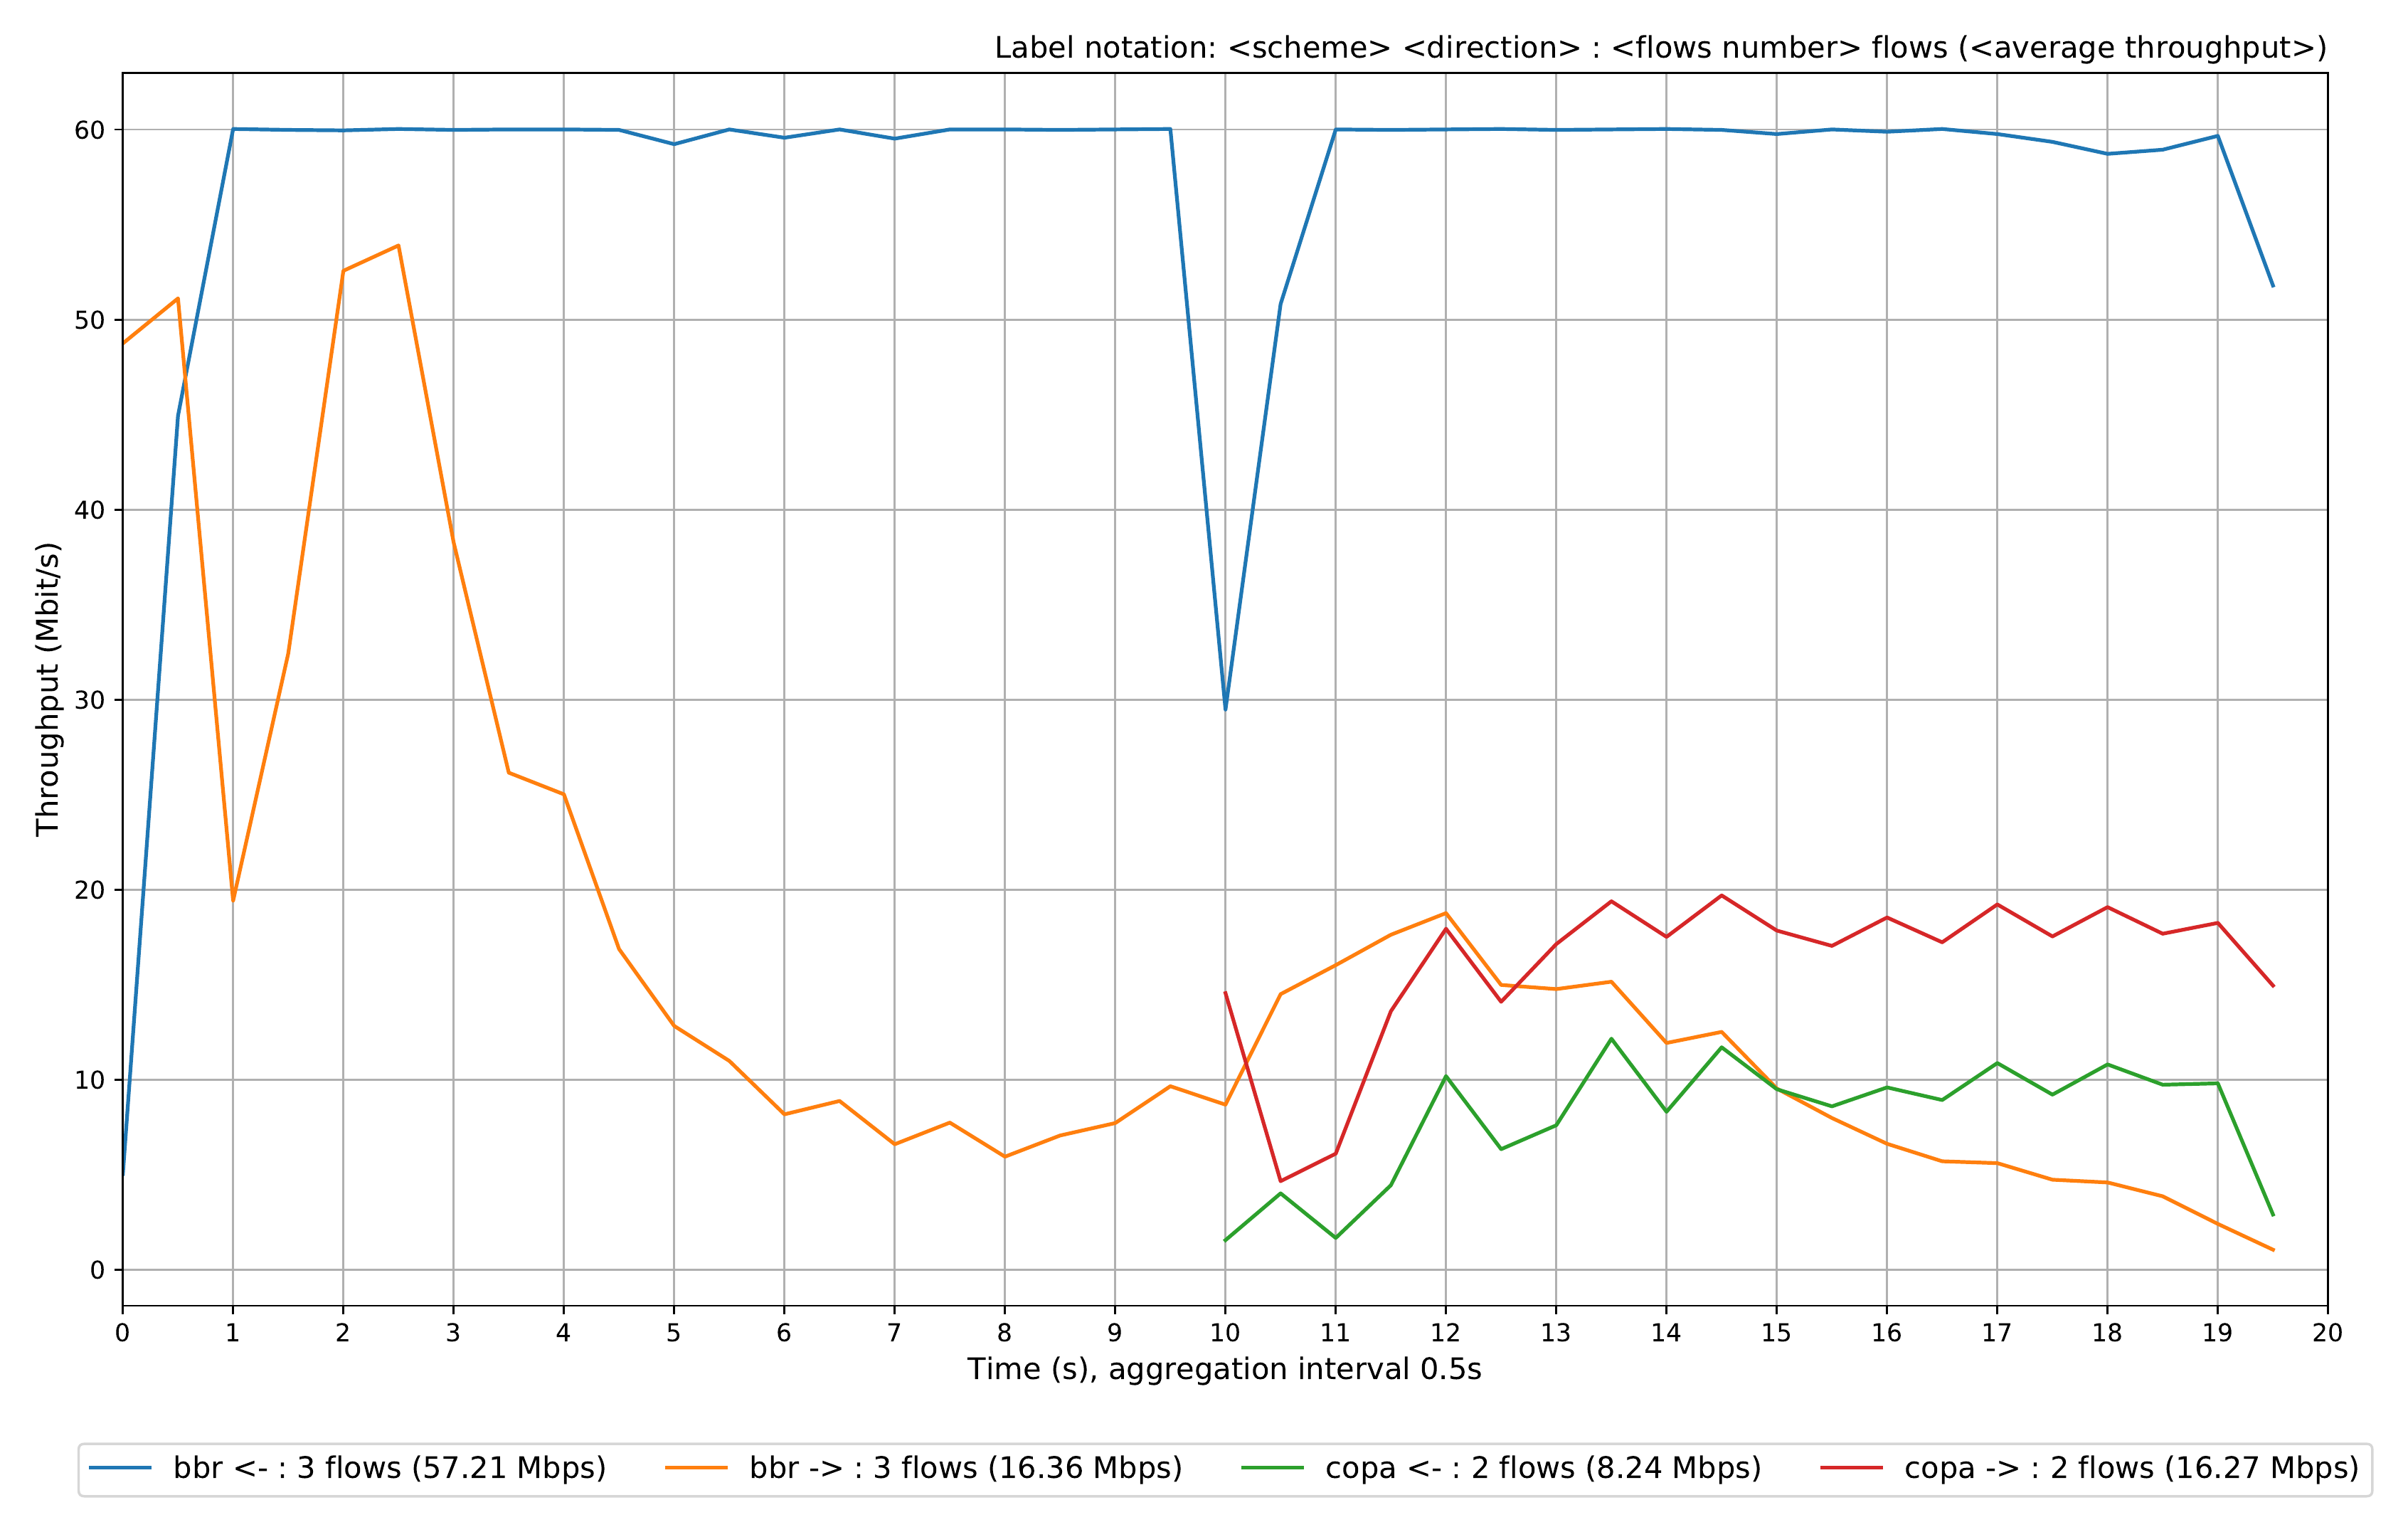}
\caption{Per-scheme-and-direction average throughput plot.}
\end{figure}

\vspace{0.5cm}

\begin{figure}[h!]
\centering
\includegraphics[width=\textwidth]{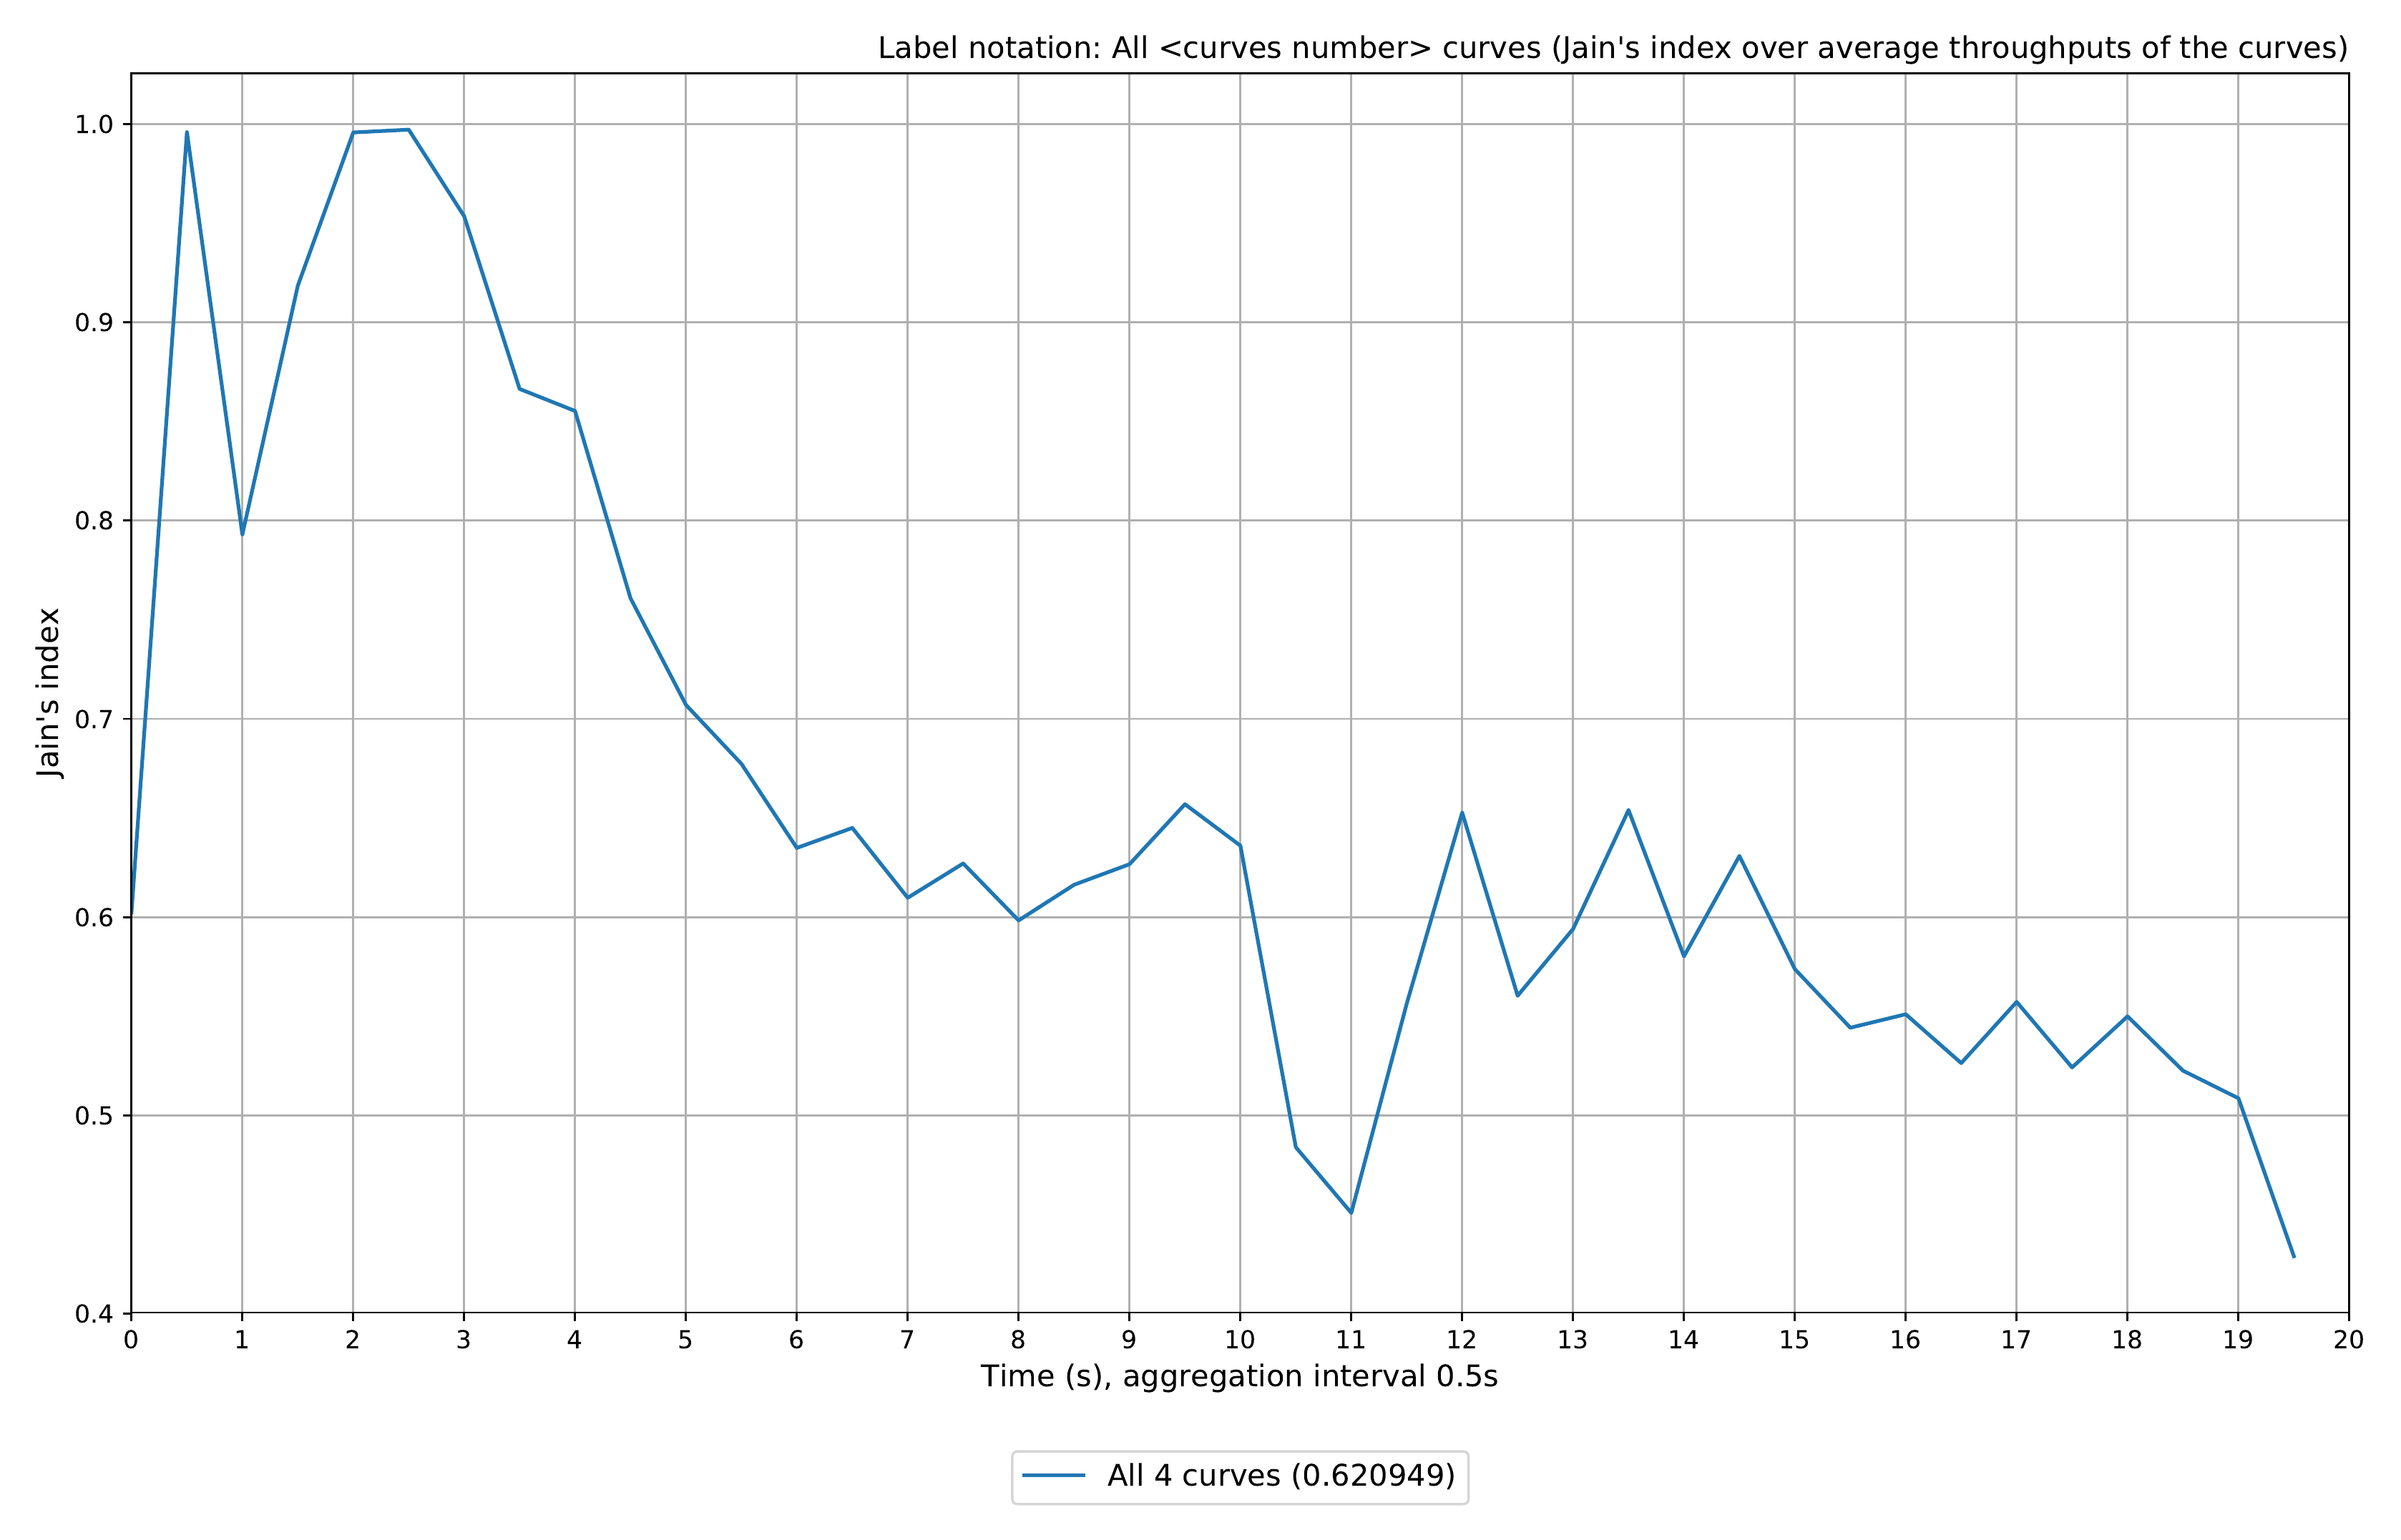}
\caption{Per-scheme-and-direction average Jain's index plot.}
\end{figure}

The small 0.01-second aggregation interval makes the average~\ref{fig:psdavgdelay} and per-packet~\ref{fig:psdpptdelay} one-way delay plots look very much alike.

\begin{figure}[h!]
\centering
\includegraphics[width=\textwidth]{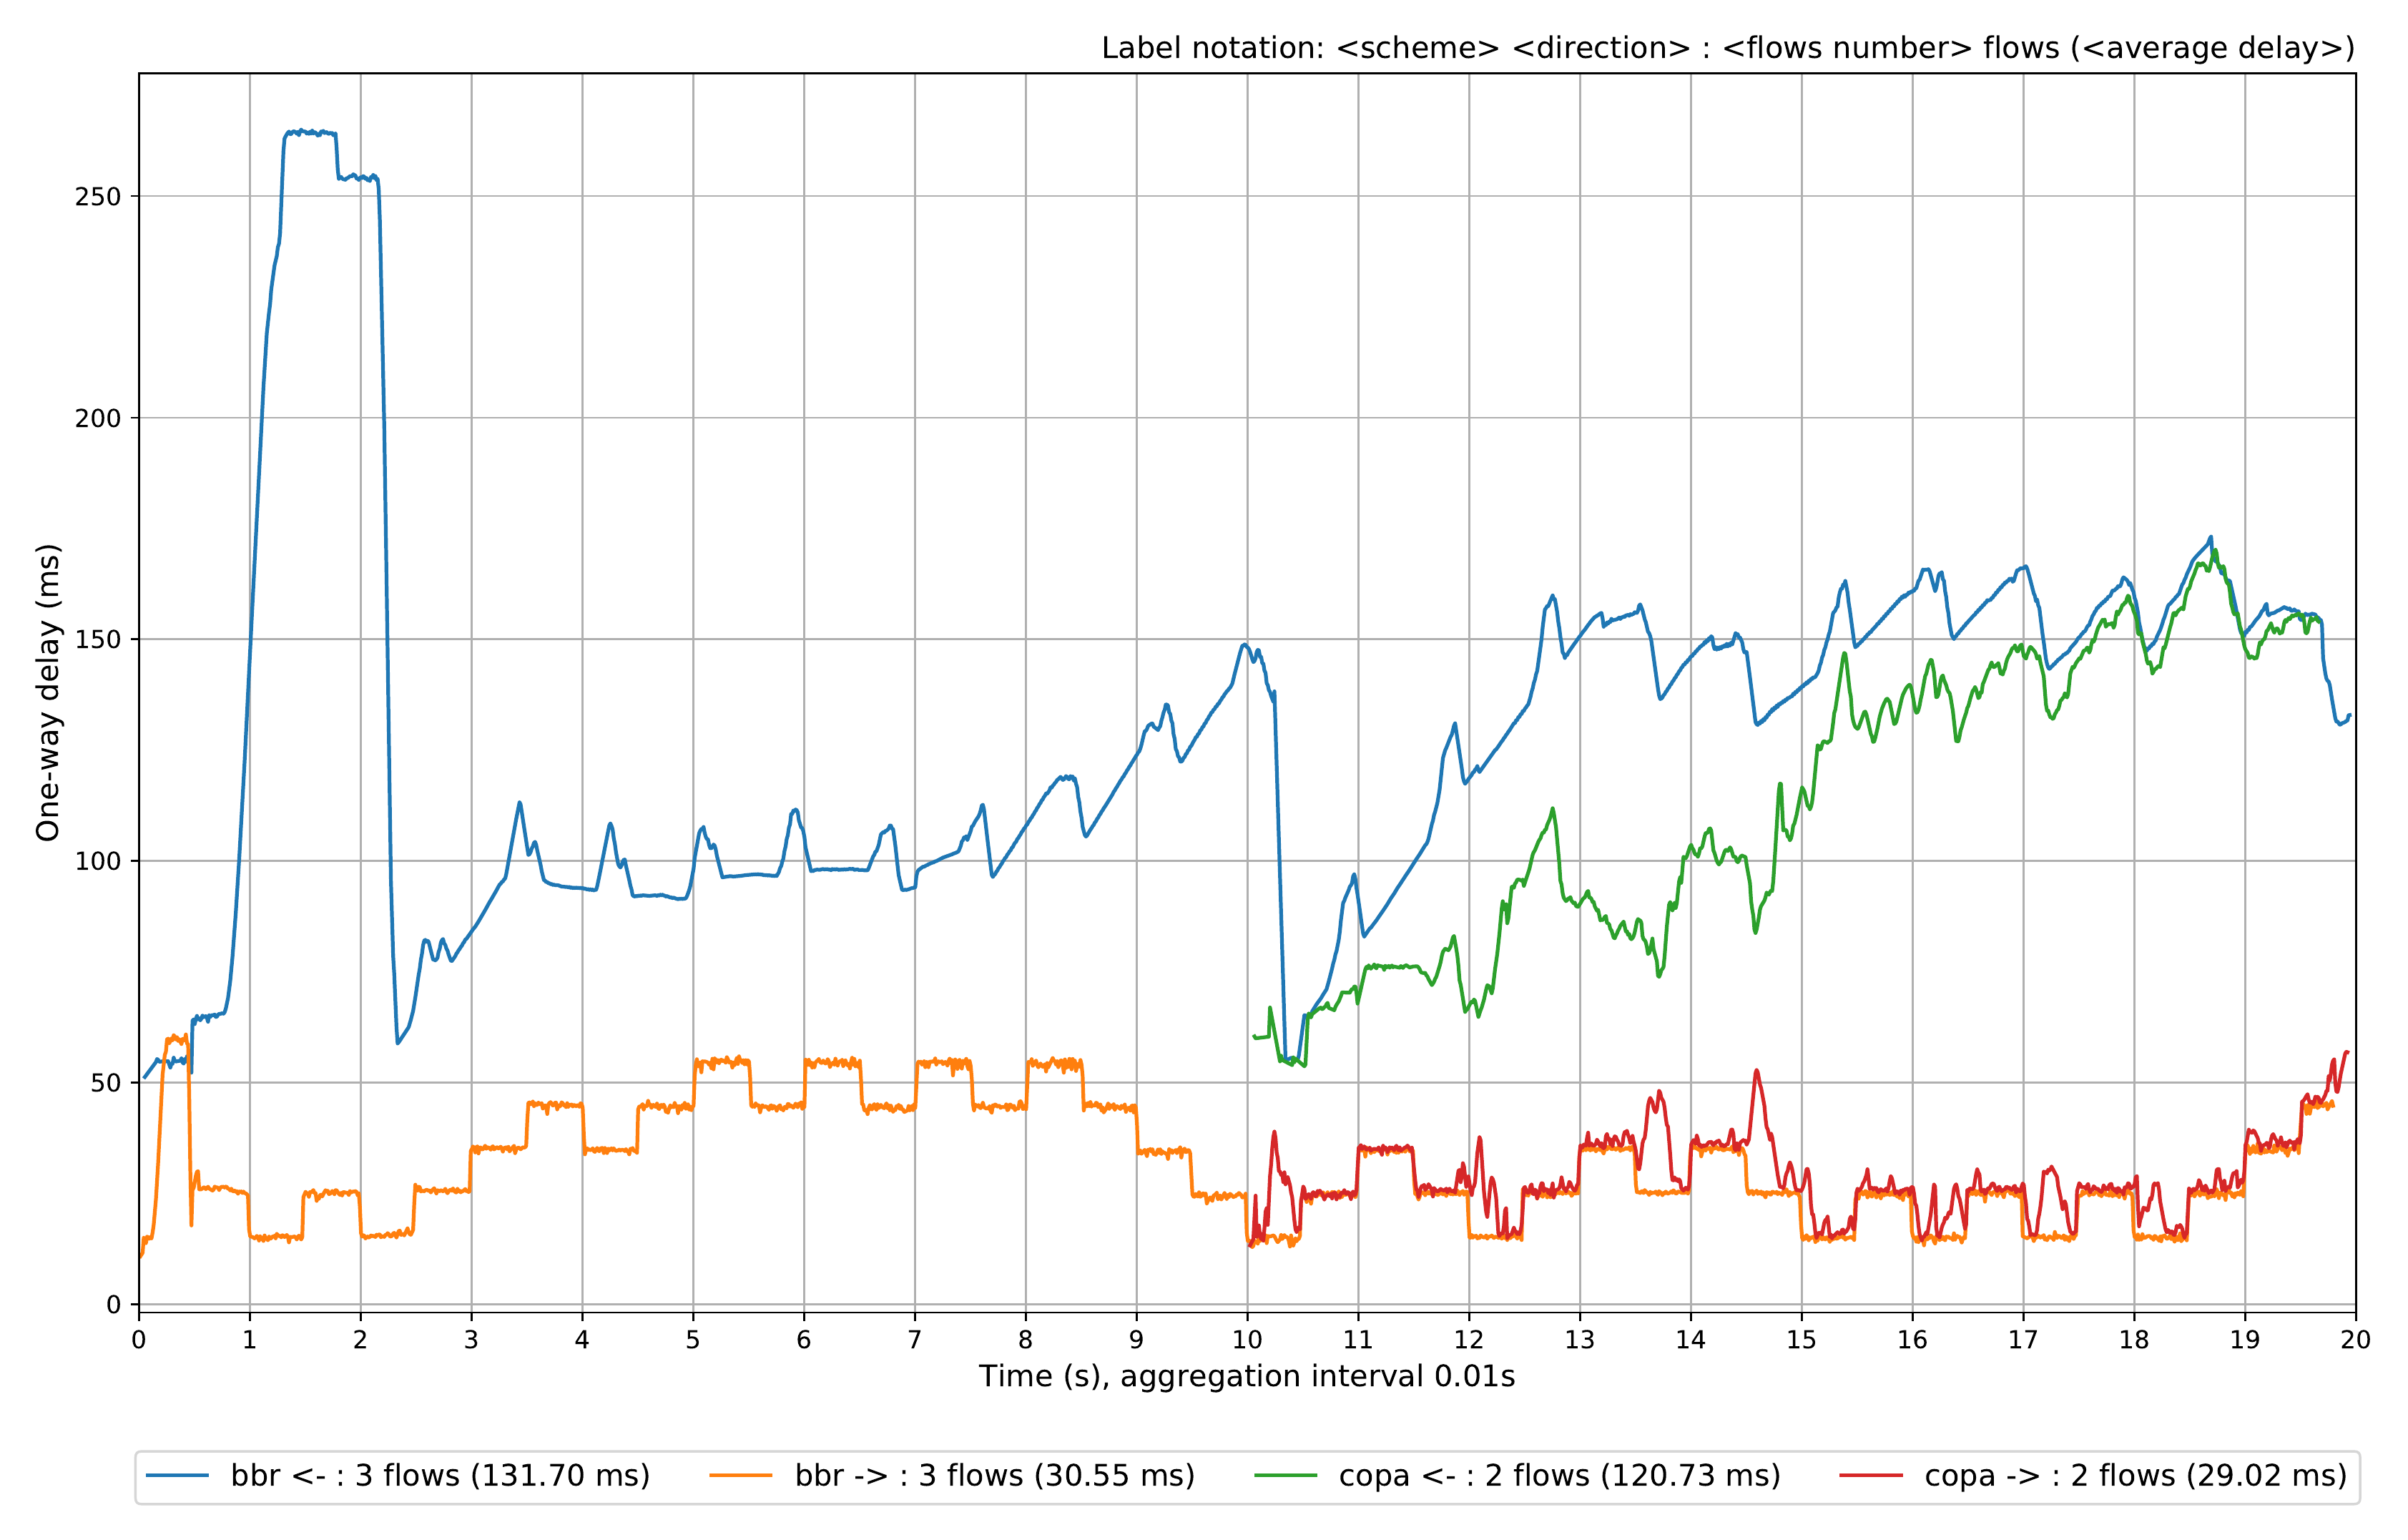}
\caption{Per-scheme-and-direction average one-way delay plot.}
\label{fig:psdavgdelay}
\end{figure}

\textcolor{white}{.}

\begin{figure}[h!]
\centering
\includegraphics[width=\textwidth]{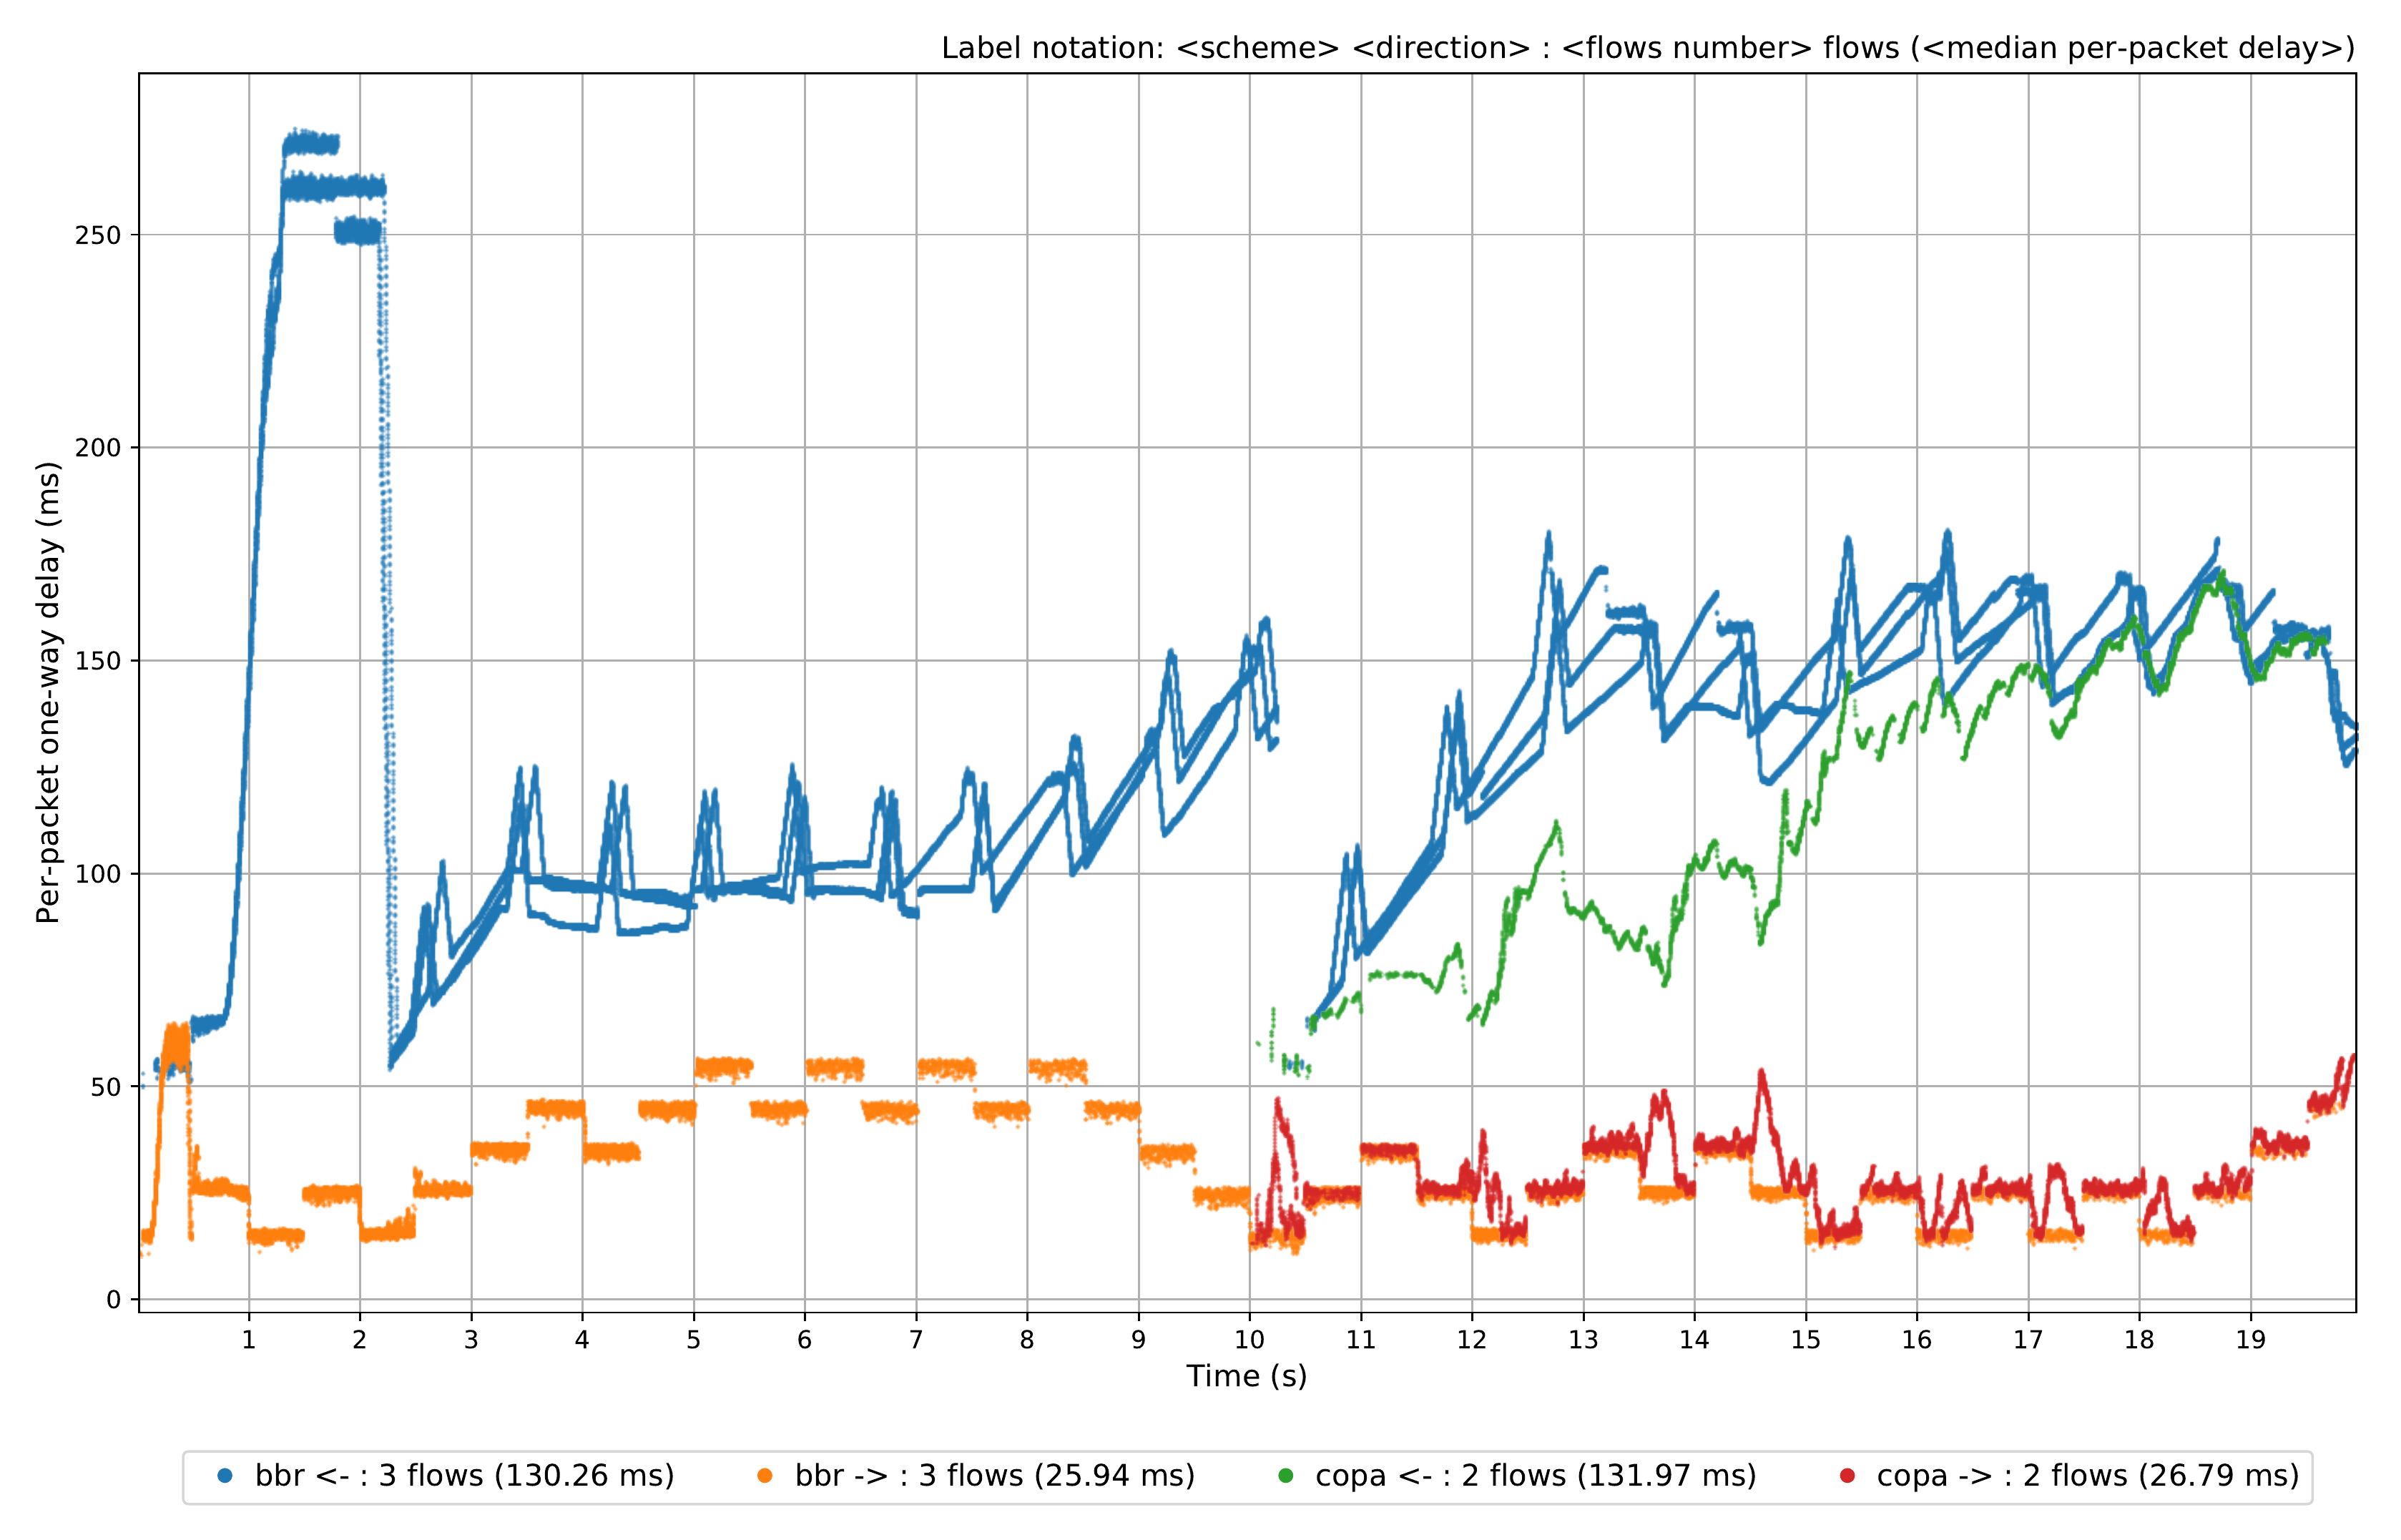}
\caption{Per-scheme-and-direction per-packet one-way delay plot.}
\label{fig:psdpptdelay}
\end{figure}

\newpage

\begin{lstlisting}[frame=single,basicstyle=\linespread{1}\ttfamily\normalsize,caption=Per-scheme-and-direction statistics.]
== Average and loss statistics ==

Average Jain's index  : 0.620949

-- Curve "bbr <- : 3 flows":
Average throughput    : 57.212322 Mbps
Average one-way delay : 131.700397 ms
Loss                  : 0.488160 %

-- Curve "bbr -> : 3 flows":
Average throughput    : 16.364470 Mbps
Average one-way delay : 30.552046 ms
Loss                  : 0.022441 %

-- Curve "copa <- : 2 flows":
Average throughput    : 8.239964 Mbps
Average one-way delay : 120.730178 ms
Loss                  : 4.945032 %

-- Curve "copa -> : 2 flows":
Average throughput    : 16.273102 Mbps
Average one-way delay : 29.016342 ms
Loss                  : 0.278835 %

===== Per-packet statistics =====

-- Curve "bbr <- : 3 flows":
Median per-packet one-way delay          : 130.258083 ms
Average per-packet one-way delay         : 131.700397 ms
95th percentile per-packet one-way delay : 236.953020 ms

-- Curve "bbr -> : 3 flows":
Median per-packet one-way delay          : 25.939941 ms
Average per-packet one-way delay         : 30.552046 ms
95th percentile per-packet one-way delay : 55.520773 ms

-- Curve "copa <- : 2 flows":
Median per-packet one-way delay          : 131.968975 ms
Average per-packet one-way delay         : 120.730178 ms
95th percentile per-packet one-way delay : 159.483910 ms

-- Curve "copa -> : 2 flows":
Median per-packet one-way delay          : 26.786089 ms
Average per-packet one-way delay         : 29.016342 ms
95th percentile per-packet one-way delay : 46.359062 ms
\end{lstlisting}

\newpage

\section{Total Plots and Statistics}

The Jain's index in plot~\ref{fig:tjain} is strictly $1.0$ in this section, as there is only one curve in the average rate plot~\ref{fig:trate}. The curve includes the data of all the ten flows.

\begin{figure}[h!]
\centering
\includegraphics[width=0.99\textwidth]{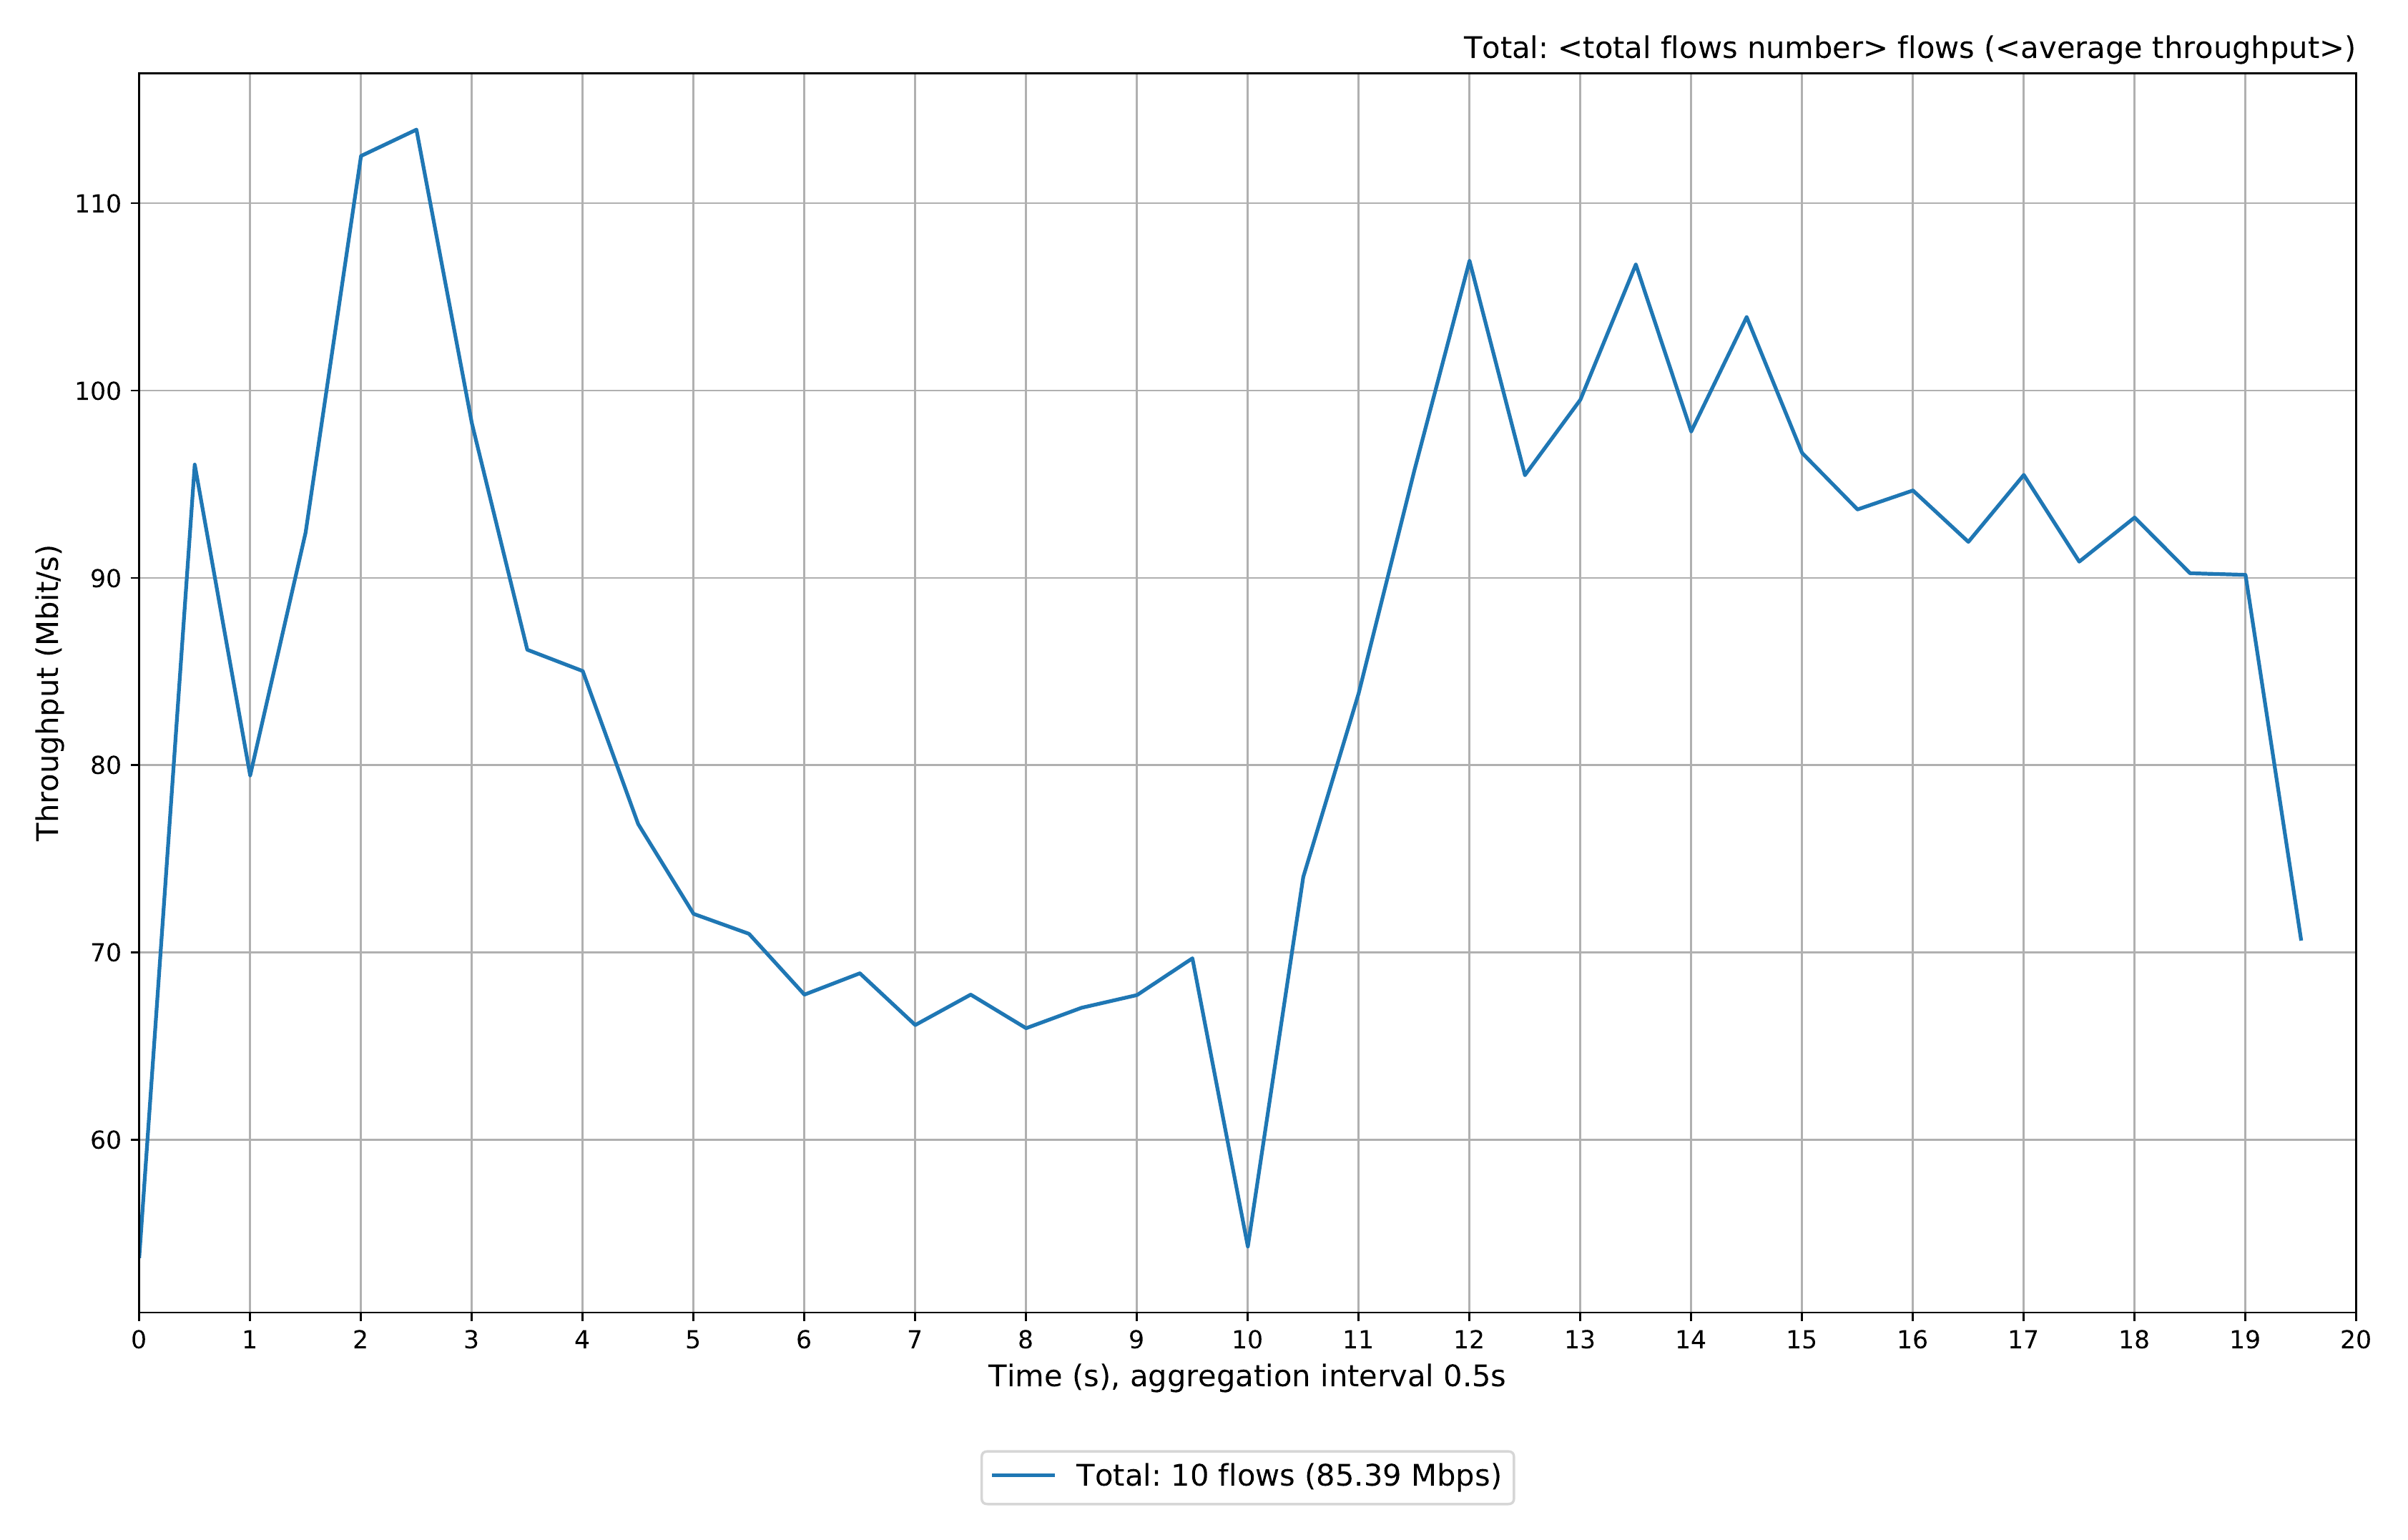}
\caption{Total average throughput plot.}
\label{fig:trate}
\end{figure}

\vspace{0.5cm}

\begin{figure}[h!]
\centering
\includegraphics[width=\textwidth]{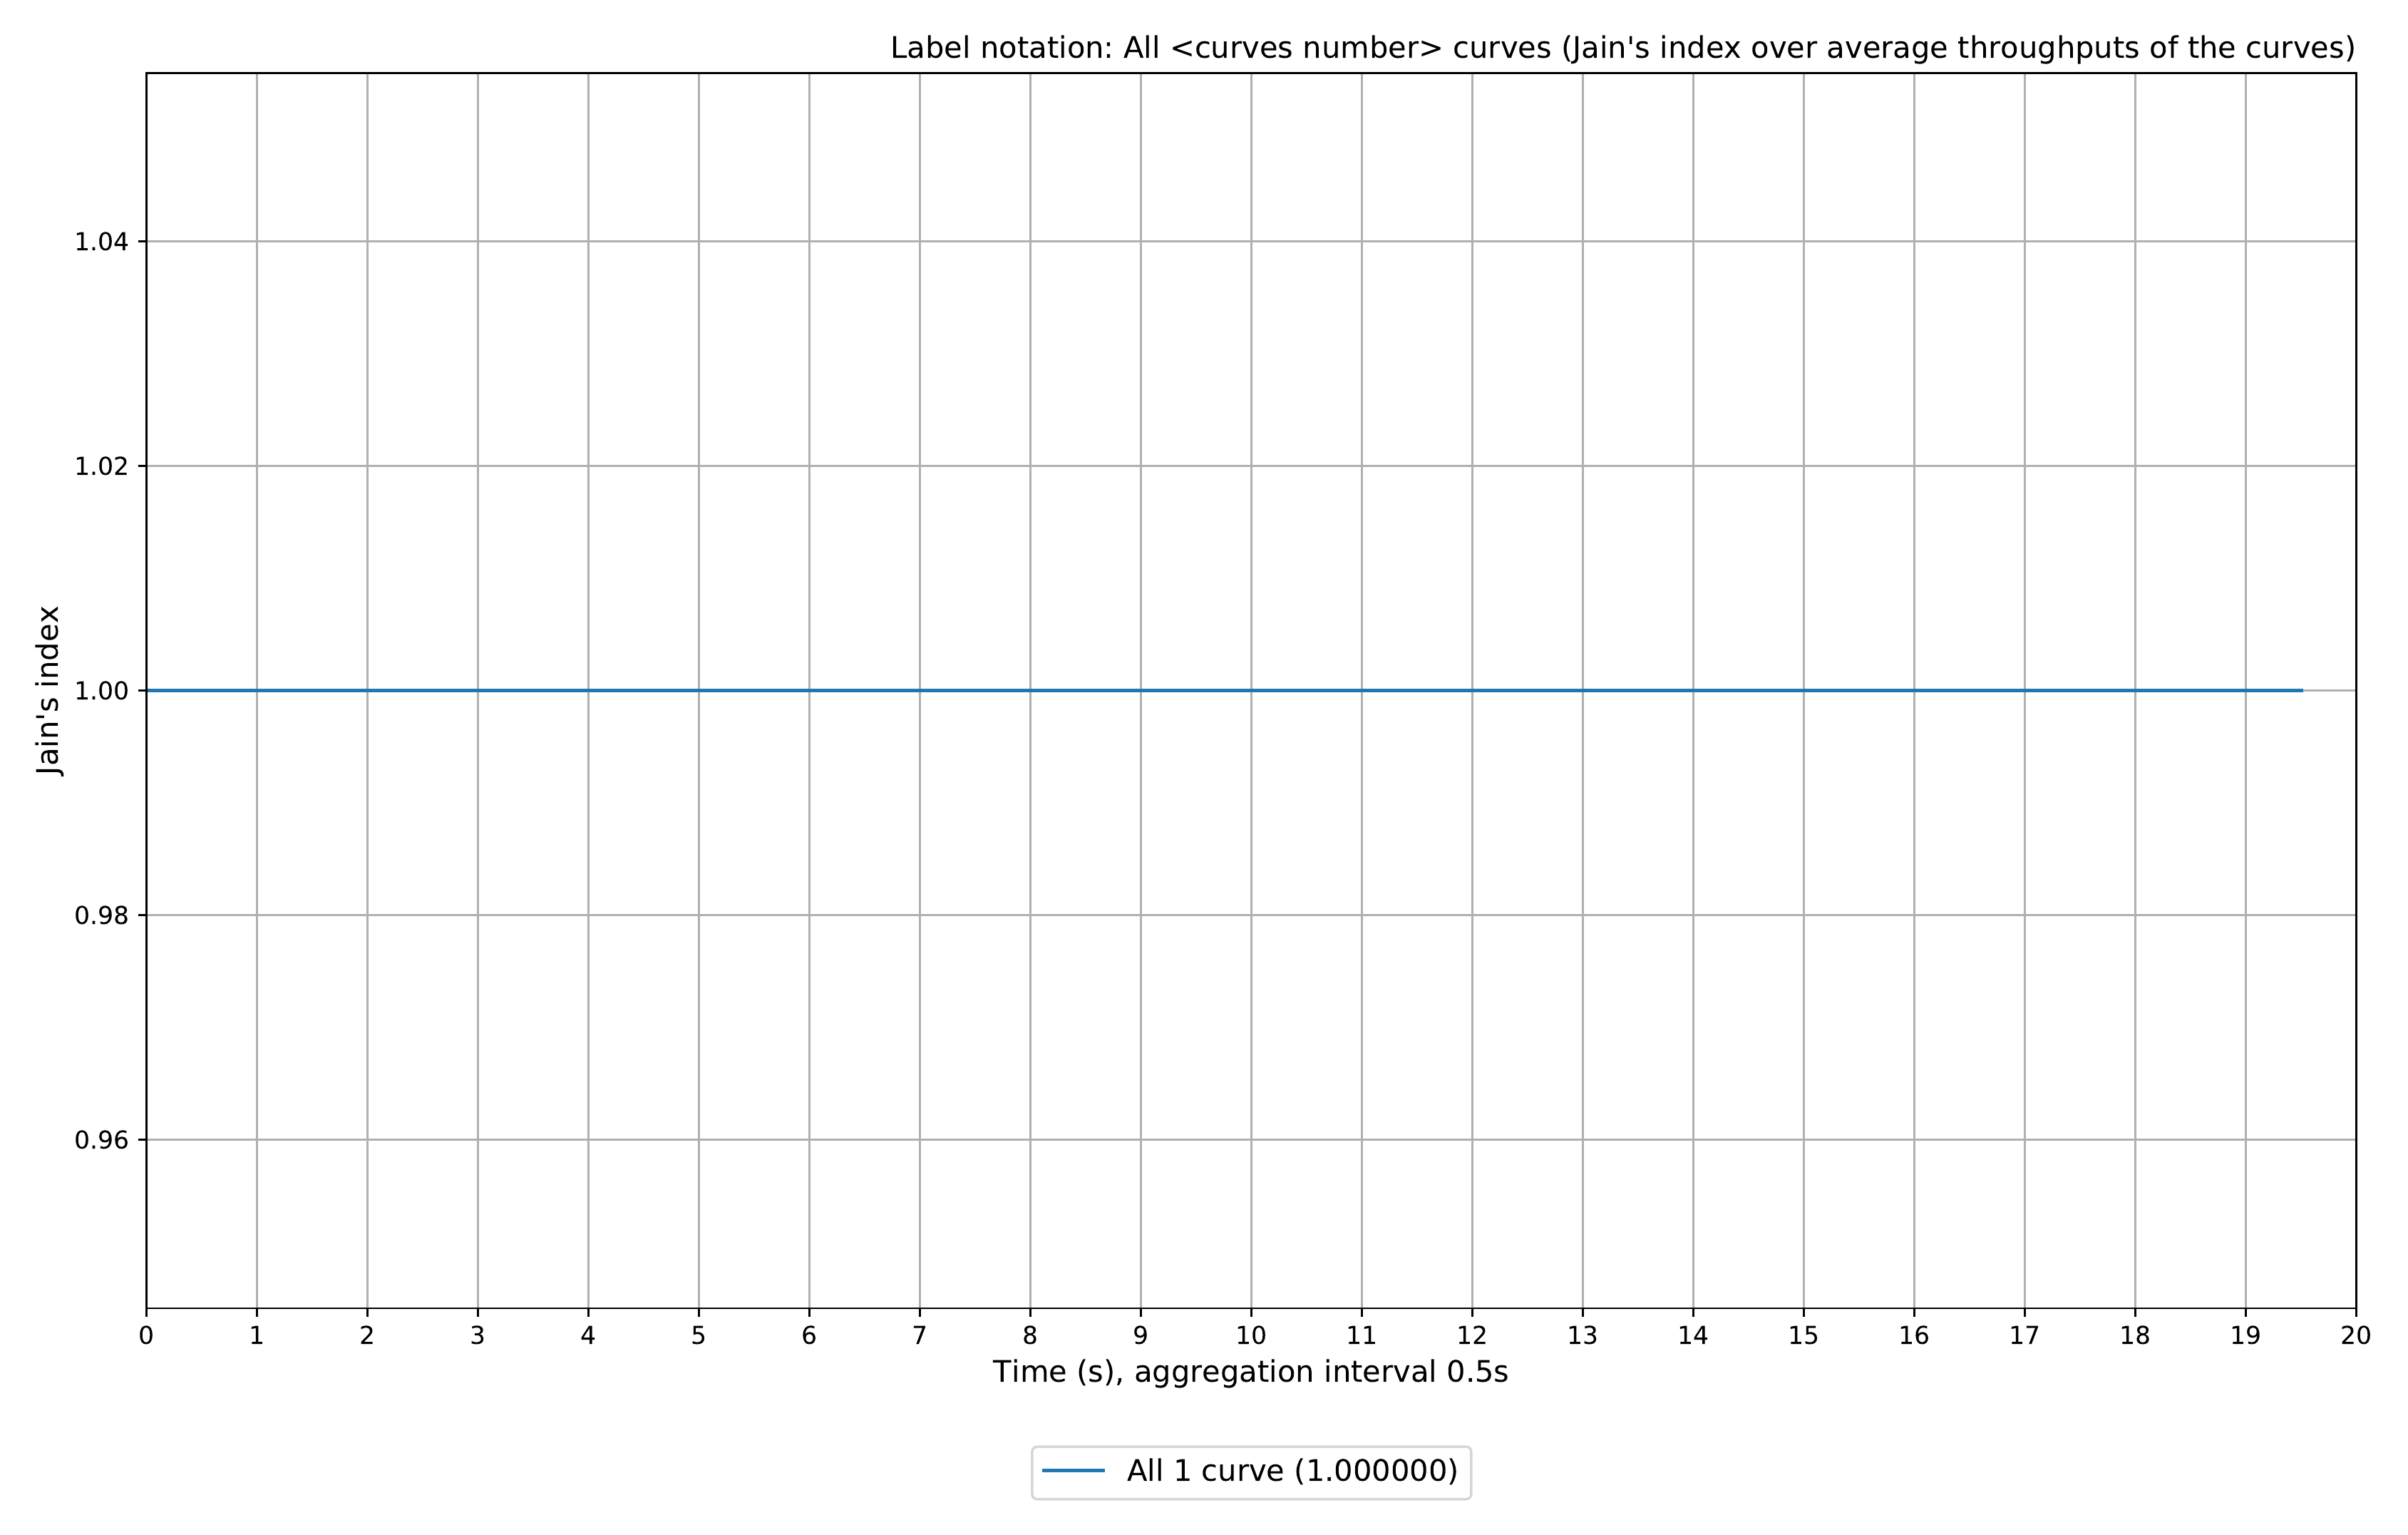}
\caption{Total average Jain's index plot.}
\label{fig:tjain}
\end{figure}

\textcolor{white}{.}\\

\begin{figure}[h!]
\centering
\includegraphics[width=\textwidth]{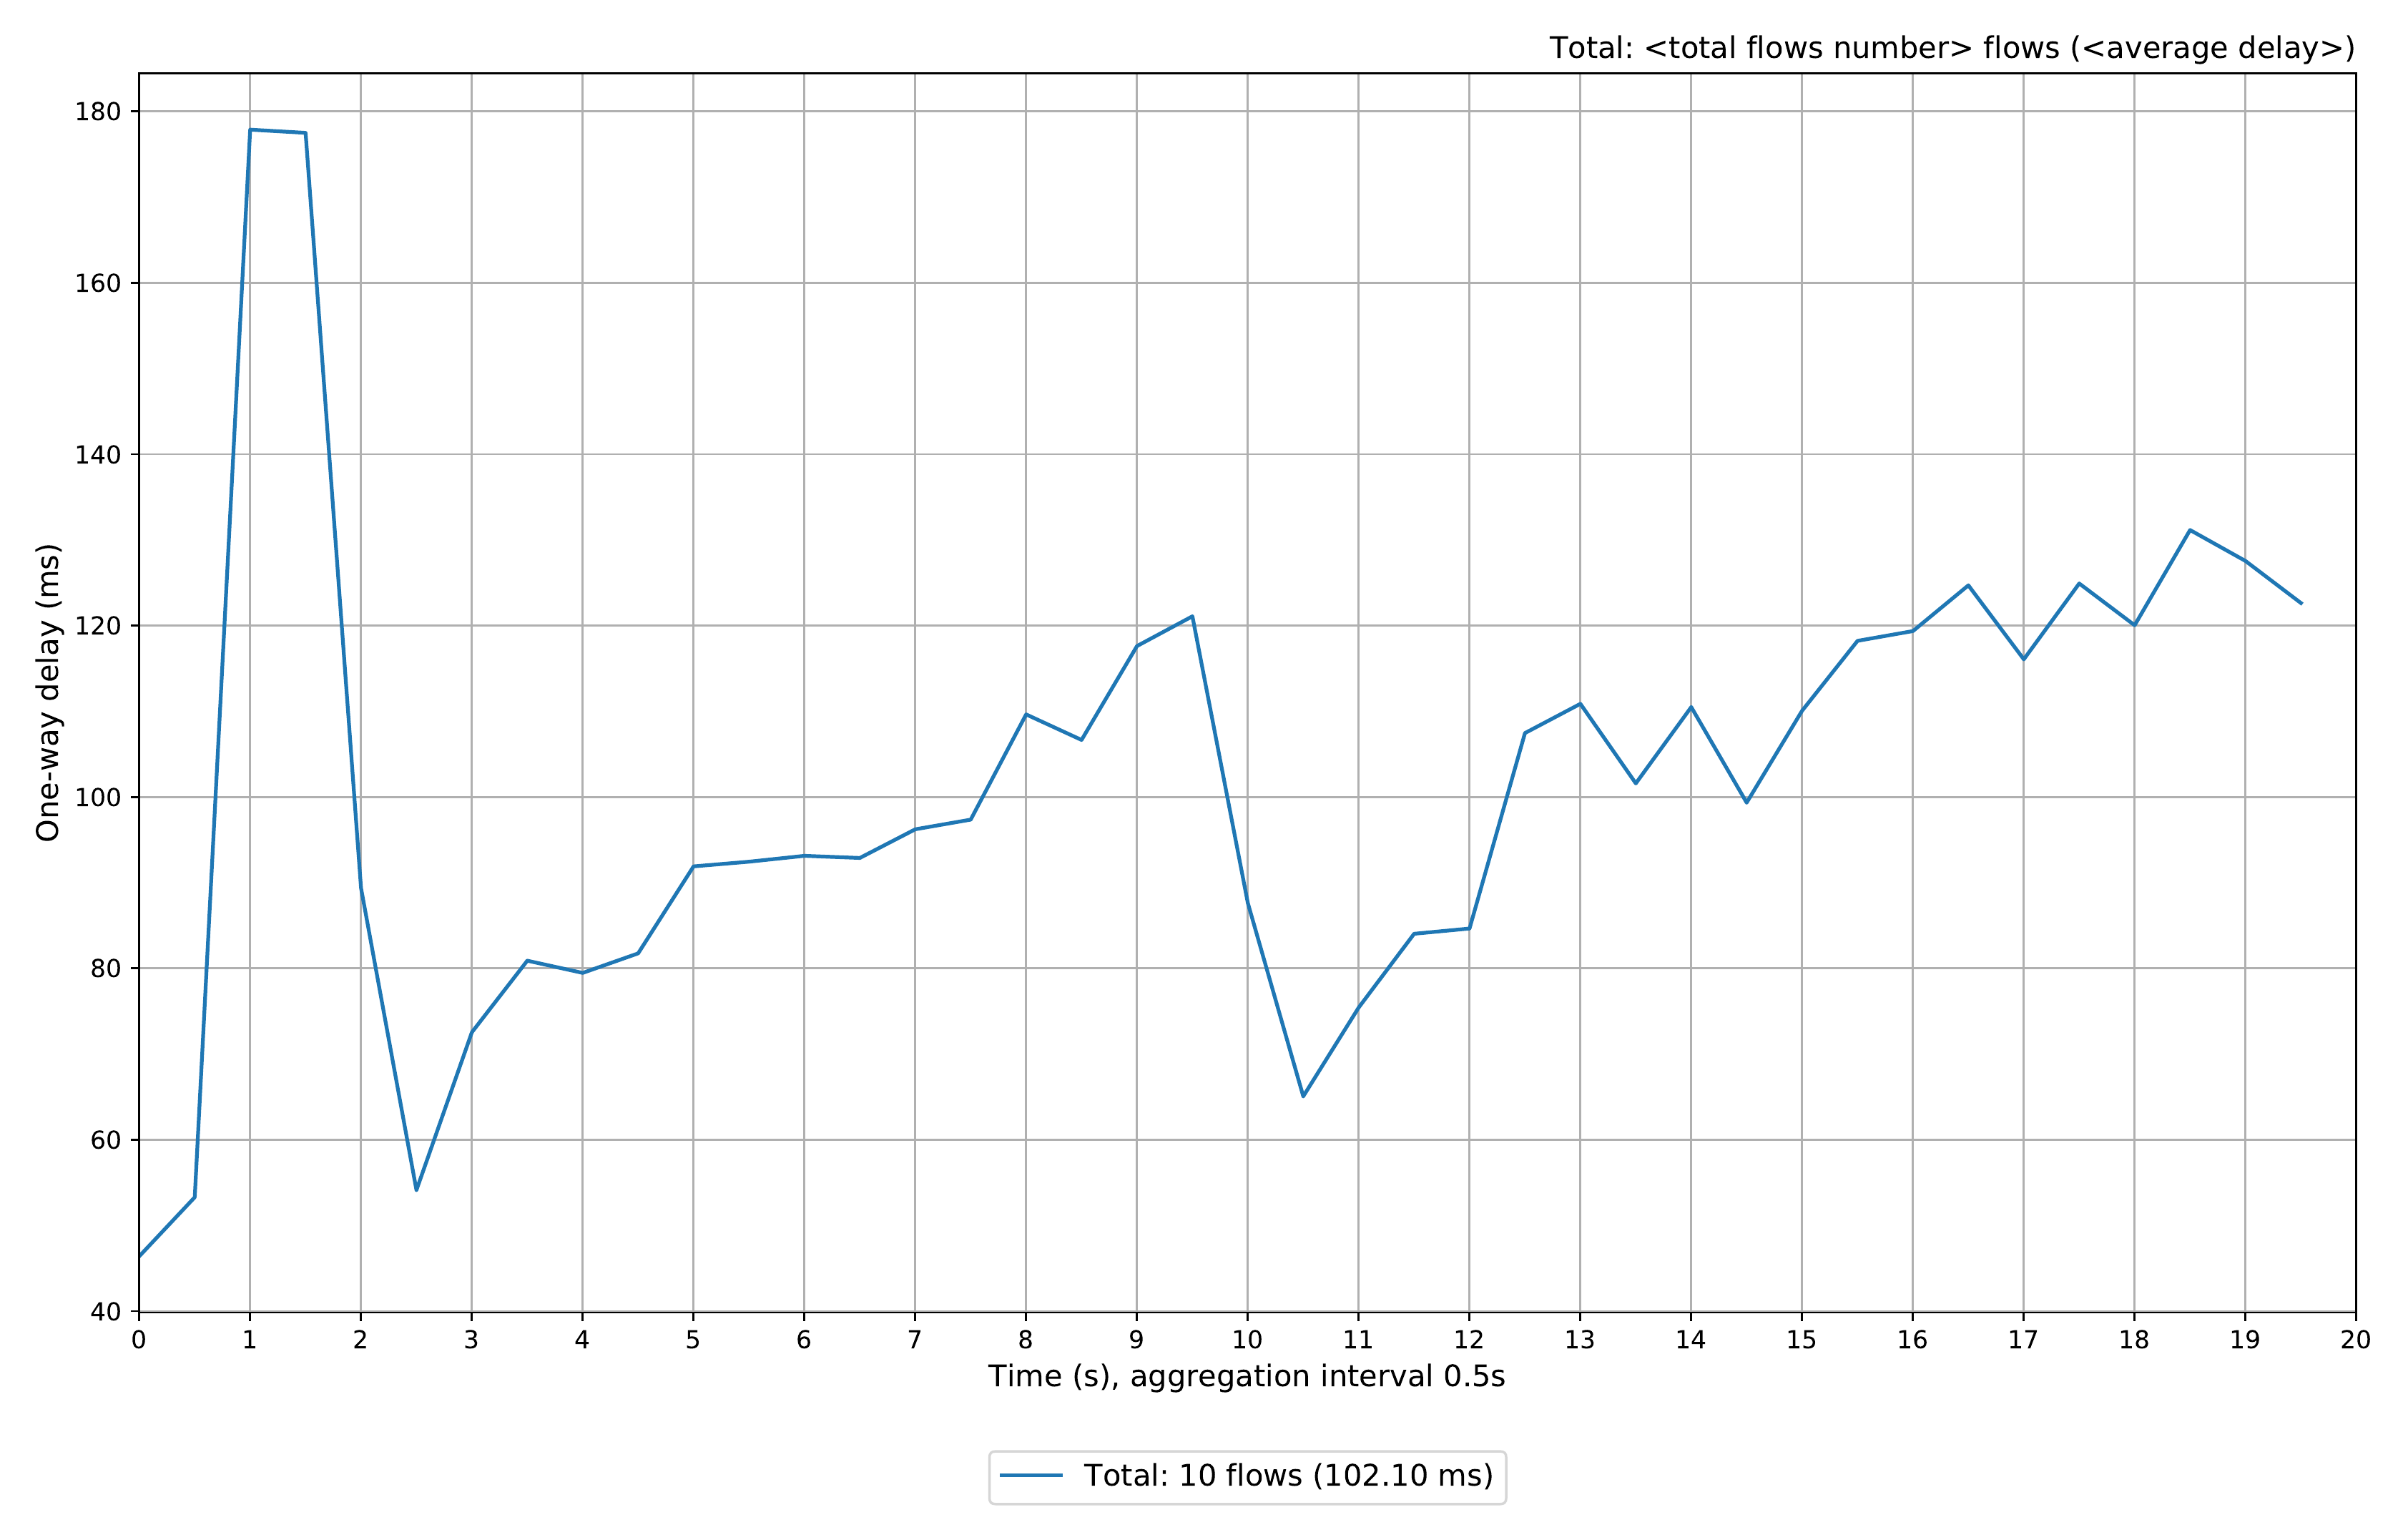}
\caption{Total average one-way delay plot.}
\label{fig:tonedelay}
\end{figure}

\textcolor{white}{.}

\begin{figure}[h!]
\centering
\includegraphics[width=\textwidth]{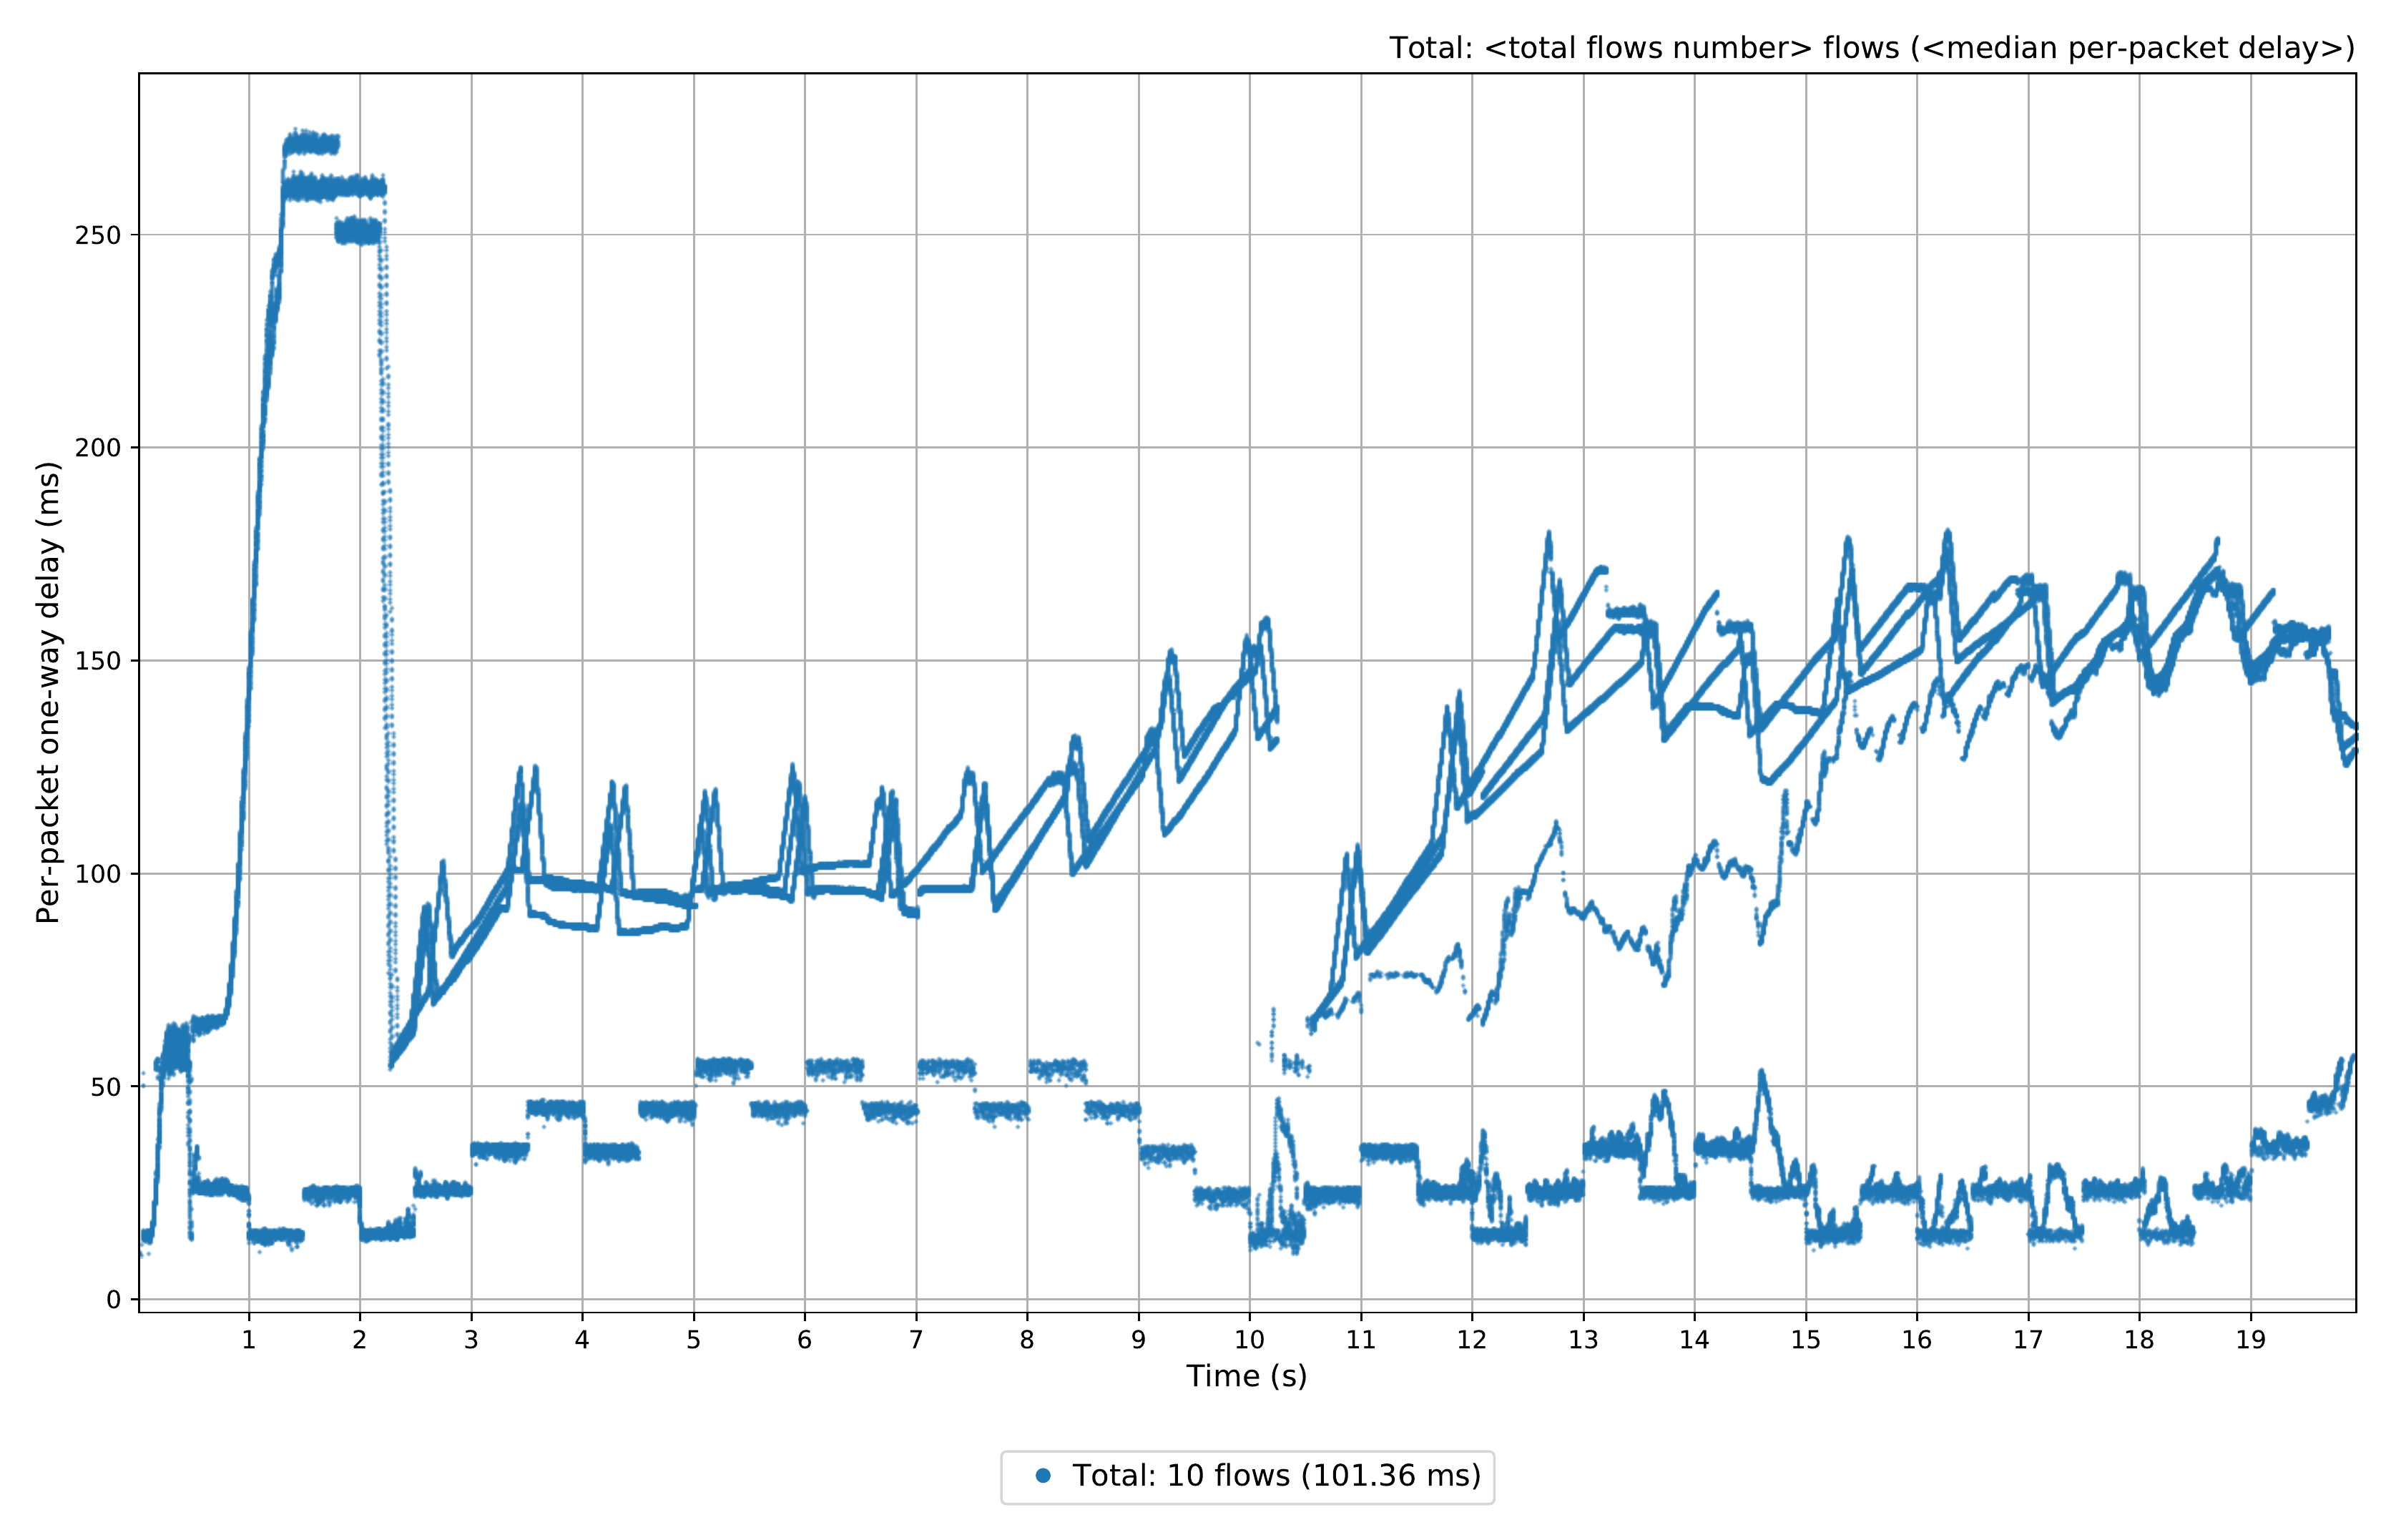}
\caption{Total per-packet one-way delay plot.}
\label{fig:tpptdelay}
\end{figure}

\newpage

\begin{lstlisting}[frame=single,basicstyle=\linespread{1}\ttfamily\normalsize,caption=Total statistics.]
== Average and loss statistics ==

Average Jain's index  : 1.000000

-- Curve "Total: 10 flows":
Average throughput    : 85.390422 Mbps
Average one-way delay : 102.099407 ms
Loss                  : 0.596869 %

===== Per-packet statistics =====

-- Curve "Total: 10 flows":
Median per-packet one-way delay          : 101.356030 ms
Average per-packet one-way delay         : 102.099407 ms
95th percentile per-packet one-way delay : 169.993877 ms
\end{lstlisting}
