# Supplementary material for: The CoCo-Beholder: Enabling Comprehensive Evaluation of Congestion Control Algorithms
Source: arXiv:1912.10531 source file (2019-12-22)
Supplement: Supplementary file 3 [file AppendixC.tex]

\vspace{-0.4cm}
\begin{table}[!h]
\caption{\mbox{The schemes present (on the left) and not present (on the right) in Pantheon.}\\ \textcolor{white}{.....}No papers or source code were found for FillP and FillP-Sheep.}
\label{tab:schemes}
\small

\resizebox{\textwidth}{!}{\begin{tabular}{|>{\centering\arraybackslash}p{1.5cm}|>{\centering\arraybackslash}p{2.5cm}|>{\centering\arraybackslash}p{1.1cm}|>{\centering\arraybackslash}p{0.5cm}|>{\centering\arraybackslash}p{1.5cm}|>{\centering\arraybackslash}p{2.5cm}|>{\centering\arraybackslash}p{1.1cm}|} \cline{1-3}\cline{5-7}

\textbf{Scheme} & \textbf{Full Name} & \textbf{Type} & & \textbf{Scheme} & \textbf{Full Name} & \textbf{Type} \\ [0.1cm]\cline{1-3}\cline{5-7}

bbr & TCP BBR~\cite{bbr} & hybrid & & bic & BIC TCP~\cite{bic} & loss\\ [0.1cm]\cline{1-3}\cline{5-7}

copa & Copa~\cite{copa} & delay & & cdg & TCP CDG~\cite{cdg} & hybrid\\ [0.1cm]\cline{1-3}\cline{5-7}

cubic & TCP Cubic~\cite{cubic} & loss & & highspeed & \makecell{HighSpeed\\TCP}~\cite{hstcp} & loss\\ [0.1cm]\cline{1-3}\cline{5-7}

fillp & FillP & ? & & htcp & H-TCP~\cite{htcp0, htcp} & loss\\ [0.1cm]\cline{1-3}\cline{5-7}

fillp\_sheep & FillP-Sheep & ? & & hybla & TCP Hybla~\cite{hybla} & loss\\ [0.1cm]\cline{1-3}\cline{5-7}

indigo & Indigo~\cite{pantheon} & learned & & illinois & \makecell{TCP\\Illinois}~\cite{illinois} & hybrid \\ [0.1cm]\cline{1-3}\cline{5-7}

ledbat & LEDBAT~\cite{ledbat} & delay && lp & TCP-LP~\cite{lp} & delay\\ [0.1cm]\cline{1-3}\cline{5-7}

pcc & \makecell{PCC\\Allegro}~\cite{pcc} & learned && nv & \makecell{TCP\\New Vegas}~\cite{nv} & delay\\ [0.1cm]\cline{1-3}\cline{5-7}

pcc\_exp & \makecell{PCC-UDT}~\cite{pcc} & learned && reno & \makecell{TCP Reno}~\cite{rfc5681} & loss\\ [0.1cm]\cline{1-3}\cline{5-7}

quic & \makecell{QUIC\\Cubic}~\cite{quic} & loss && scalable & \makecell{Scalable\\TCP}~\cite{scalable} & loss  \\ [0.1cm]\cline{1-3}\cline{5-7}

scream & SCReAM~\cite{scream} & hybrid && veno & TCP Veno~\cite{veno} & hybrid \\[0.1cm] \cline{1-3}\cline{5-7}

sprout & Sprout~\cite{sprout} & delay && westwood & \mbox{\makecell{TCP\\Westwood+}\cite{westwood-plus}} & hybrid\\[0.1cm] \cline{1-3}\cline{5-7}

taova & Tao 100x~\cite{taova} & learned  && yeah & YeAH-TCP~\cite{yeah}  & hybrid\\ [0.1cm]\cline{1-3}\cline{5-7}

vegas & TCP Vegas~\cite{vegas} & delay \\ [0.1cm]\cline{1-3}

verus & Verus~\cite{verus} & delay \\ [0.1cm]\cline{1-3}

vivace & \makecell{PCC\\Vivace}~\cite{vivace} & learned \\ [0.1cm]\cline{1-3}
\end{tabular}}
\end{table}
