# Supplementary material for: The CoCo-Beholder: Enabling Comprehensive Evaluation of Congestion Control Algorithms
Source: arXiv:1912.10531 source file (2019-12-22)
Supplement: Supplementary file 4 [file AppendixD.tex]

This appendix has more of the results of the testing experiments described in Section~\ref{sec:tfirst}. Let us remind the setup of the experiments here.

The topology used in Pantheon is point-to-point. The single link was set up to have the rate 100 Mbit/s, the delay $X$ ms, and the queue size 1000 packets. 

The topology used in CoCo-Beholder is a dumbbell of size one. All the three links were set up to have the rate 100 Mbit/s and the queue size 1000 packets. The left and the right links had 1 ms delay, while the central link had $(X - 2)$ ms delay.

One flow of a tested scheme was run for ten seconds, and the resulting overall rate, $95^{\text{th}}$ percentile one-way delay, and loss statistics were learned. This was repeated ten times for each of the two tools. Tables~\ref{tab:tab2},~\ref{tab:tab3},~\ref{tab:tab4} in this appendix contain the results for the delays $X \in \{3, 5, 20\}$ ms for the schemes present in Pantheon. Tables~\ref{tab:tab6},~\ref{tab:tab7},~\ref{tab:tab8} contain the results for the delays $X \in \{3, 5, 20\}$ ms for the schemes not present in Pantheon but available as Linux kernel modules and added to the collection locally.

The schemes in the tables are sorted in alphabetical order by their names. The values in the cells are rounded to two decimal points. The symbols $\mu$ and $\sigma$ stand for the mean and the sample standard deviation computed over the ten runs of a scheme. The symbol $d_r$ stands for the relative difference calculated using the formula~\ref{eq:differ}. If the mean rate or delay results by CoCo-Beholder and Pantheon differ more than by 10 percent, then the value of the winner is highlighted with blue color and the value of the opponent is highlighted with red color. The symbol $\Delta$ stands for the absolute difference and is computed between the mean loss results of the two emulators.

\begin{table*}[h!]
\centering
\Large
\caption{Testing results for the delay $X=3$ ms.}
 
\resizebox*{\textwidth}{!}{\begin{tabu}{|c|cV{5}c|c|cV{5}c|c|cV{5}c|c|cV{5}}
\hline
\multirow{2}*{\parbox[c][2.5cm]{2.1cm}{\centering \bf \large Scheme}} &  \multicolumn{1}{c|}{\multirow{2}*{\parbox[c][2.5cm]{0.0cm}{}}} & \multicolumn{3}{c|}{\parbox[c][1cm]{2.7cm}{\bf \large Rate (Mbps)}} & \multicolumn{3}{c|}{\parbox[c][1cm]{2.3cm}{\bf \large Delay (ms)}} & \multicolumn{3}{c|}{\parbox[c][1cm]{1.8cm}{\bf \large Loss (\%)}}\\ 
\cline{3-11}
 & \multicolumn{1}{c|}{} & \parbox[c][1.5cm]{1.8cm}{\centering \bf \normalsize CoCo-Beholder}  & \parbox[1cm]{1.9cm}{\centering \bf \normalsize Pantheon} & \multicolumn{1}{c|}{\parbox{1.8cm}{\centering \pmb{$d_r$}}} & \parbox{1.8cm}{\centering \bf \normalsize CoCo-Beholder} & \parbox{1.8cm}{\centering \bf \normalsize Pantheon} & \multicolumn{1}{c|}{\parbox{1.8cm}{\centering \pmb{$d_r$}}} & \parbox{1.8cm}{\centering \bf \normalsize CoCo-Beholder} & \parbox{1.8cm}{\centering \bf \normalsize Pantheon} &\multicolumn{1}{c|}{ \parbox{1.8cm}{\centering \pmb{$\Delta$}}}\\
\cline{1-2}\tabucline[2pt]{3-11}
\multirow{2}*{\parbox[c][1cm]{2.1cm}{\centering bbr}} & \large \pmb{$\mu$} & 99.79 & 99.67 & 0.13\% &\cellcolor{myg}8.79 & \cellcolor{myr}15.05 & 52.56\% &  0.11 & 0.15 & 0.04\\
\cline{2-11}
& \large \pmb{$\sigma$} & 0.03 & 0.14 & & 0.14 & 0.23 & & 0.09 & 0.06 & \\
\cline{1-2}\tabucline[2pt]{3-11}
\multirow{2}*{\parbox[c][1cm]{2.1cm}{\centering copa}} & \large \pmb{$\mu$} & \cellcolor{myg}99.05 & \cellcolor{myr}58.41 & 51.63\% & \cellcolor{myg}4.01 & \cellcolor{myr}5.45 & 30.27\% & 0.04 & 0.05 & 0.02\\
\cline{2-11}
& \large \pmb{$\sigma$} & 0.39 & 1.52 & & 0.00 & 0.21 & & 0.01 & 0.02 & \\
\cline{1-2}\tabucline[2pt]{3-11}
\multirow{2}*{\parbox[c][1cm]{2.1cm}{\centering cubic}} & \large \pmb{$\mu$} & 99.81 & 99.53 & 0.28\% & 122.77 & 117.21 & 4.63\% & 0.99 & 0.97 & 0.02\\
\cline{2-11}
& \large \pmb{$\sigma$} & 0.00 & 0.25 & & 0.16 & 6.87 & & 0.09 & 0.11 &\\
\cline{1-2}\tabucline[2pt]{3-11}
\multirow{2}*{\parbox[c][1cm]{2.1cm}{\centering fillp}} & \large \pmb{$\mu$} & 97.98 & 98.54 & 0.57\% & \cellcolor{myg}28.13 & \cellcolor{myr}36.47 & 25.81\% & 0.69 & 0.73 & 0.04\\
\cline{2-11}
& \large \pmb{$\sigma$} & 0.29 & 0.13 & & 1.73 & 4.14 & & 0.16 & 0.20 &\\
\cline{1-2}\tabucline[2pt]{3-11}
\multirow{2}*{\parbox[c][1cm]{2.1cm}{\centering fillp\_sheep}} & \large \pmb{$\mu$} & 95.75 & 96.78 & 1.07\% & \cellcolor{myg}17.58 & \cellcolor{myr}19.62 & 11.01\% & 0.14 & 0.13 & 0.01\\
\cline{2-11}
& \large \pmb{$\sigma$} & 0.76 & 0.66 & & 1.02 & 1.08 & & 0.14 & 0.05 &\\
\cline{1-2}\tabucline[2pt]{3-11}
\multirow{2}*{\parbox[c][1cm]{2.1cm}{\centering indigo}} & \large \pmb{$\mu$} & 99.09 & 95.05 & 4.17\% & 9.02 & 8.17 & 9.91\% & 0.07 & 0.06 & 0.01\\
\cline{2-11}
& \large \pmb{$\sigma$} & 0.19 & 7.96 & & 0.37 & 1.40 & & 0.05 & 0.01 &\\
\cline{1-2}\tabucline[2pt]{3-11}
\multirow{2}*{\parbox[c][1cm]{2.1cm}{\centering ledbat}} & \large \pmb{$\mu$} & 98.99 & 94.49 & 4.65\% & 50.76 & 48.22 & 5.13\% & 0.55 & 0.48 & 0.07\\
\cline{2-11}
& \large \pmb{$\sigma$} & 0.00 & 5.84 & & 0.00 & 4.07 & & 0.00 & 0.12 &\\
\cline{1-2}\tabucline[2pt]{3-11}
\multirow{2}*{\parbox[c][1cm]{2.1cm}{\centering pcc}} & \large \pmb{$\mu$} & \cellcolor{myg}93.63 & \cellcolor{myr}61.53 & 41.37\% & \cellcolor{myg}4.55 & \cellcolor{myr}5.87 & 25.21\% & 0.06 & 0.04 & 0.02\\
\cline{2-11}
& \large \pmb{$\sigma$} & 0.65 & 17.38 & & 0.35 & 4.01 & & 0.10 & 0.01&\\
\cline{1-2}\tabucline[2pt]{3-11}
\multirow{2}*{\parbox[c][1cm]{2.1cm}{\centering pcc\_exp}} & \large \pmb{$\mu$} & \cellcolor{myg}88.64 & \cellcolor{myr}62.13 & 35.17\% & \cellcolor{myg}21.06 & \cellcolor{myr}28.63 & 30.46\% & 0.08 & 0.84 & 0.76\\
\cline{2-11}
& \large \pmb{$\sigma$} & 1.33 & 29.17 & & 10.68 & 26.43 & & 0.03 & 1.64 & \\
\cline{1-2}\tabucline[2pt]{3-11}
\multirow{2}*{\parbox[c][1cm]{2.1cm}{\centering quic}} & \large \pmb{$\mu$} & 78.74 & 72.16 & 8.72\% & \cellcolor{myg}3.41 & \cellcolor{myr}4.34 & 24.18\% & 0.05 & 0.04 & 0.01\\
\cline{2-11}
& \large \pmb{$\sigma$} & 1.35 & 1.15 & & 0.00 & 0.02 & & 0.10& 0.01 & \\
\cline{1-2}\tabucline[2pt]{3-11}
\multirow{2}*{\parbox[c][1cm]{2.1cm}{\centering scream}} & \large \pmb{$\mu$} & 0.22 & 0.22 & 1.85\% &\cellcolor{myg}3.44 &\cellcolor{myr}4.56 & 27.82\% & 0.16 & 0.00 & 0.16\\
\cline{2-11}
& \large \pmb{$\sigma$} & 0.00 & 0.00 & & 0.03 & 0.06 & & 0.20 & 0.00 &\\
\cline{1-2}\tabucline[2pt]{3-11}
\multirow{2}*{\parbox[c][1cm]{2.1cm}{\centering sprout}} & \large \pmb{$\mu$} & 49.12 & 45.79 & 7.02\% & 12.20 & 12.20 & 0.04\% & 0.08 & 0.07 & 0.02\\
\cline{2-11}
& \large \pmb{$\sigma$} & 0.14 & 0.48 & & 0.03 & 0.03 & & 0.17 & 0.07 &\\
\cline{1-2}\tabucline[2pt]{3-11}
\multirow{2}*{\parbox[c][1cm]{2.1cm}{\centering taova}} & \large \pmb{$\mu$} & 92.95 & 84.32 & 9.74\% &\cellcolor{myg}3.82 & \cellcolor{myr}5.54 & 36.91\% & 0.05 & 0.06 & 0.01\\
\cline{2-11}
& \large \pmb{$\sigma$} & 0.04 & 0.51 & & 0.00 & 0.18 & & 0.04 & 0.08 &\\
\cline{1-2}\tabucline[2pt]{3-11}
\multirow{2}*{\parbox[c][1cm]{2.1cm}{\centering vegas}} & \large \pmb{$\mu$} & \cellcolor{myg}99.66 & \cellcolor{myr}65.76 & 40.99\% & \cellcolor{myg}10.24 & \cellcolor{myr}16.48 & 46.68\% & 0.07 & 0.04 & 0.02\\
\cline{2-11}
& \large \pmb{$\sigma$} & 0.02 & 8.72 &  & 3.39 & 8.61 & & 0.09 & 0.02 & \\
\cline{1-2}\tabucline[2pt]{3-11}
\multirow{2}*{\parbox[c][1cm]{2.1cm}{\centering verus}} & \large \pmb{$\mu$} & 94.46 & 90.50 & 4.28\% & \cellcolor{myg}42.27 & \cellcolor{myr}52.03 & 20.68\% & 3.93 & 4.09 & 0.16\\
\cline{2-11}
& \large \pmb{$\sigma$} & 7.26 & 5.33 & & 10.27 & 9.86 & & 0.25 & 0.16 & \\
\cline{1-2}\tabucline[2pt]{3-11}
%%%%%%%%%%%%%%%%%%%%%%%%%%
\multirow{2}*{\parbox[c][1cm]{2.1cm}{\centering vivace}} & \large \pmb{$\mu$} & \cellcolor{myg}86.13 & \cellcolor{myr}50.23 & 52.66\% & \cellcolor{myg}3.46 & \cellcolor{myr}6.59 & 62.26\% & 0.08 & 0.07 & 0.01\\
\cline{2-11}
& \large \pmb{$\sigma$} & 0.38 & 31.77 & & 0.04 & 2.92 & & 0.04 & 0.04 & \\
\cline{1-2}\tabucline[2pt]{3-11}
%%%%%%%%%%%%%%%%%%%%%%%%%%
\end{tabu}}
\label{tab:tab2}
\end{table*}

\begin{table*}[h!]
\centering
\Large
\caption{Testing results for the delay $X=3$ ms \emph{(continuation)}.}
 
\resizebox*{\textwidth}{!}{\begin{tabu}{|c|cV{5}c|c|cV{5}c|c|cV{5}c|c|cV{5}}
\hline
\multirow{2}*{\parbox[c][2.5cm]{2.1cm}{\centering \bf \large Scheme}} &  \multicolumn{1}{c|}{\multirow{2}*{\parbox[c][2.5cm]{0.0cm}{}}} & \multicolumn{3}{c|}{\parbox[c][1cm]{2.7cm}{\bf \large Rate (Mbps)}} & \multicolumn{3}{c|}{\parbox[c][1cm]{2.3cm}{\bf \large Delay (ms)}} & \multicolumn{3}{c|}{\parbox[c][1cm]{1.8cm}{\bf \large Loss (\%)}}\\ 
\cline{3-11}
 & \multicolumn{1}{c|}{} & \parbox[c][1.5cm]{1.8cm}{\centering \bf \normalsize CoCo-Beholder}  & \parbox[1cm]{1.9cm}{\centering \bf \normalsize Pantheon} & \multicolumn{1}{c|}{\parbox{1.8cm}{\centering \pmb{$d_r$}}} & \parbox{1.8cm}{\centering \bf \normalsize CoCo-Beholder} & \parbox{1.8cm}{\centering \bf \normalsize Pantheon} & \multicolumn{1}{c|}{\parbox{1.8cm}{\centering \pmb{$d_r$}}} & \parbox{1.8cm}{\centering \bf \normalsize CoCo-Beholder} & \parbox{1.8cm}{\centering \bf \normalsize Pantheon} &\multicolumn{1}{c|}{ \parbox{1.8cm}{\centering \pmb{$\Delta$}}}\\
\cline{1-2}\tabucline[2pt]{3-11}
\multirow{2}*{\parbox[c][1cm]{2.1cm}{\centering bic}} & \large \pmb{$\mu$} & 99.80 & 99.57 & 0.23\% & 123.96 & 121.98 & 1.61\% & 3.50 & 3.54 & 0.05\\
\cline{2-11}
& \large \pmb{$\sigma$} & 0.01 & 0.15 & & 0.61 & 0.46 & & 0.15 & 0.29 &\\
\cline{1-2}\tabucline[2pt]{3-11}
\multirow{2}*{\parbox[c][1cm]{2.1cm}{\centering cdg}} & \large \pmb{$\mu$} & 98.61 & 92.80 & 6.06\% & \cellcolor{myr}18.06 & \cellcolor{myg}12.70 & 34.88\% & 0.14 & 0.08 & 0.06\\
\cline{2-11}
& \large \pmb{$\sigma$} & 1.15 & 2.60 & & 3.63 & 3.22 & & 0.10 & 0.03 &\\
\cline{1-2}\tabucline[2pt]{3-11}
\multirow{2}*{\parbox[c][1cm]{2.1cm}{\centering highspeed}} & \large \pmb{$\mu$} & 99.78 & 99.61 & 0.18\% & \cellcolor{myr}118.62 & \cellcolor{myg}102.26 & 14.81\% & 2.39 & 2.25 & 0.15\\
\cline{2-11}
& \large \pmb{$\sigma$} & 0.05 & 0.08 & & 7.37 & 12.07 & & 0.10 & 0.11 & \\
\cline{1-2}\tabucline[2pt]{3-11}
\multirow{2}*{\parbox[c][1cm]{2.1cm}{\centering htcp}} & \large \pmb{$\mu$} & 99.79 & 99.61 & 0.18\% & \cellcolor{myr}112.97 & \cellcolor{myg}86.05 & 27.05\% & 2.42 &  1.97 & 0.45\\
\cline{2-11}
& \large \pmb{$\sigma$} & 0.00 & 0.11 & & 7.91 & 9.64 & & 0.10 & 0.20 & \\
\cline{1-2}\tabucline[2pt]{3-11}
\multirow{2}*{\parbox[c][1cm]{2.1cm}{\centering hybla}} & \large \pmb{$\mu$} & 99.59 & 99.32 & 0.27\% & 116.79 & 108.53 & 7.33\% & 2.22 & 1.80 & 0.42\\
\cline{2-11}
& \large \pmb{$\sigma$} & 0.00 & 0.10 & & 2.55 & 16.89 & & 0.13 & 0.29 & \\
\cline{1-2}\tabucline[2pt]{3-11}
\multirow{2}*{\parbox[c][1cm]{2.1cm}{\centering illinois}} & \large \pmb{$\mu$} & 99.80 & 99.59 & 0.21\% & 94.25 & 88.55 & 6.23\% & 2.12 & 1.90 & 0.22\\
\cline{2-11}
& \large \pmb{$\sigma$} & 0.01 & 0.15 & & 13.59 & 7.76 & & 0.06 & 0.60 & \\
\cline{1-2}\tabucline[2pt]{3-11}
\multirow{2}*{\parbox[c][1cm]{2.1cm}{\centering lp}} & \large \pmb{$\mu$} & 99.79 & 99.55 & 0.24\% & \cellcolor{myr}109.62 & \cellcolor{myg}83.55 & 26.99\% & 2.00 & 1.86 & 0.14\\
\cline{2-11}
& \large \pmb{$\sigma$} & 0.00 & 0.06 & & 20.50 & 2.64 & & 0.09 & 0.14&\\
\cline{1-2}\tabucline[2pt]{3-11}
\multirow{2}*{\parbox[c][1cm]{2.1cm}{\centering nv}} & \large \pmb{$\mu$} & 99.38 & 97.32 & 2.10\% & \cellcolor{myg}5.84 & \cellcolor{myr}6.83 & 15.65\% & 0.02 & 0.06 & 0.04\\
\cline{2-11}
& \large \pmb{$\sigma$} & 0.01 & 0.49 & & 0.09 & 0.07 & & 0.06 & 0.01 & \\
\cline{1-2}\tabucline[2pt]{3-11}
\multirow{2}*{\parbox[c][1cm]{2.1cm}{\centering reno}} & \large \pmb{$\mu$} & 99.79 & 99.64 & 0.15\% & 86.72 & 85.09 & 1.90\% & 2.11 & 1.99 & 0.12
\\
\cline{2-11}
& \large \pmb{$\sigma$} & 0.00 & 0.09 & & 14.01 & 9.75 & & 0.29 & 0.53&\\
\cline{1-2}\tabucline[2pt]{3-11}
\multirow{2}*{\parbox[c][1cm]{2.1cm}{\centering scalable}} & \large \pmb{$\mu$} & 99.80 & 99.61 & 0.19\% & 124.18 & 122.83 & 1.09\% & 4.78 & 4.37 & 0.41\\
\cline{2-11}
& \large \pmb{$\sigma$} & 0.01 &0.12 & & 0.50 & 0.11 & & 0.23 & 0.74 & \\
\cline{1-2}\tabucline[2pt]{3-11}
\multirow{2}*{\parbox[c][1cm]{2.1cm}{\centering veno}} & \large \pmb{$\mu$} & 99.79 & 99.62 & 0.17\% & \cellcolor{myr}105.81 & \cellcolor{myg}79.14 & 28.85\% & 1.91& 1.74 & 0.17\\
\cline{2-11}
& \large \pmb{$\sigma$} & 0.00 & 0.12 & & 21.56 & 9.83 & & 0.17 & 0.51 & \\
\cline{1-2}\tabucline[2pt]{3-11}
%%%%%%%%%%%%%%%%%%%%%%%%%
\multirow{2}*{\parbox[c][1cm]{2.1cm}{\centering westwood}} & \large \pmb{$\mu$} & 99.64& 98.66& 0.99\% & 72.74 & 69.91 & 3.96\% & 1.65 & 1.69 & 0.04\\
\cline{2-11}
& \large \pmb{$\sigma$} & 0.11 & 0.29 & & 7.12 & 9.55 & & 0.10 & 0.08 &\\
\cline{1-2}\tabucline[2pt]{3-11}
%%%%%%%%%%%%%%%%%%%%%%%%%
\multirow{2}*{\parbox[c][1cm]{2.1cm}{\centering yeah}} & \large \pmb{$\mu$} & 99.81 & 99.61 & 0.19\% & \cellcolor{myr}33.72 & \cellcolor{myg}28.48 & 16.85\% & 0.33 & 0.30 & 0.03\\
\cline{2-11}
& \large \pmb{$\sigma$} & 0.00 & 0.12 & & 0.78 & 4.26 & & 0.09 & 0.06& \\
\cline{1-2}\tabucline[2pt]{3-11}
\end{tabu}}
\label{tab:tab6}
\end{table*}

\begin{table*}[h!]
\centering
\Large
\caption{Testing results for the delay $X=5$ ms.}
 
\resizebox*{\textwidth}{!}{\begin{tabu}{|c|cV{5}c|c|cV{5}c|c|cV{5}c|c|cV{5}}
\hline
\multirow{2}*{\parbox[c][2.5cm]{2.1cm}{\centering \bf \large Scheme}} &  \multicolumn{1}{c|}{\multirow{2}*{\parbox[c][2.5cm]{0.0cm}{}}} & \multicolumn{3}{c|}{\parbox[c][1cm]{2.7cm}{\bf \large Rate (Mbps)}} & \multicolumn{3}{c|}{\parbox[c][1cm]{2.3cm}{\bf \large Delay (ms)}} & \multicolumn{3}{c|}{\parbox[c][1cm]{1.8cm}{\bf \large Loss (\%)}}\\ 
\cline{3-11}
 & \multicolumn{1}{c|}{} & \parbox[c][1.5cm]{1.8cm}{\centering \bf \normalsize CoCo-Beholder}  & \parbox[1cm]{1.9cm}{\centering \bf \normalsize Pantheon} & \multicolumn{1}{c|}{\parbox{1.8cm}{\centering \pmb{$d_r$}}} & \parbox{1.8cm}{\centering \bf \normalsize CoCo-Beholder} & \parbox{1.8cm}{\centering \bf \normalsize Pantheon} & \multicolumn{1}{c|}{\parbox{1.8cm}{\centering \pmb{$d_r$}}} & \parbox{1.8cm}{\centering \bf \normalsize CoCo-Beholder} & \parbox{1.8cm}{\centering \bf \normalsize Pantheon} &\multicolumn{1}{c|}{ \parbox{1.8cm}{\centering \pmb{$\Delta$}}}\\
\cline{1-2}\tabucline[2pt]{3-11}
\multirow{2}*{\parbox[c][1cm]{2.1cm}{\centering bbr}} & \large \pmb{$\mu$} & 99.61 & 99.45 & 0.16\% & \cellcolor{myg}11.47 & \cellcolor{myr}21.05 & 58.93\% & 0.16 & 0.19 & 0.02\\
\cline{2-11}
& \large \pmb{$\sigma$} & 0.00 & 0.10 & & 0.11 & 0.19 & & 0.06 & 0.01& \\
\cline{1-2}\tabucline[2pt]{3-11}
\multirow{2}*{\parbox[c][1cm]{2.1cm}{\centering copa}} & \large \pmb{$\mu$} & \cellcolor{myg}84.59 & \cellcolor{myr}63.99 & 27.73\% & \cellcolor{myr}8.67 & \cellcolor{myg}7.44 & 15.29\% & 0.01 & 0.06 & 0.05\\
\cline{2-11}
& \large \pmb{$\sigma$} & 9.95 & 1.32 & & 1.15 & 0.19 & & 0.02 & 0.02 &\\
\cline{1-2}\tabucline[2pt]{3-11}
\multirow{2}*{\parbox[c][1cm]{2.1cm}{\centering cubic}} & \large \pmb{$\mu$} & 99.63 & 99.37 & 0.26\% & 124.84 & 119.13 & 4.68\% & 1.12 & 1.05 & 0.07\\
\cline{2-11}
& \large \pmb{$\sigma$} & 0.00 & 0.12 & & 0.19 & 6.02 & & 0.00& 0.14 & \\
\cline{1-2}\tabucline[2pt]{3-11}
\multirow{2}*{\parbox[c][1cm]{2.1cm}{\centering fillp}} & \large \pmb{$\mu$} & 97.54 & 98.09 & 0.57\% & \cellcolor{myg}26.69 & \cellcolor{myr}36.41 & 30.83\% & 0.71 & 0.83 & 0.12\\
\cline{2-11}
& \large \pmb{$\sigma$} & 0.15 & 0.35 & & 0.61 & 4.75 & & 0.14& 0.13 & \\
\cline{1-2}\tabucline[2pt]{3-11}
\multirow{2}*{\parbox[c][1cm]{2.1cm}{\centering fillp\_sheep}} & \large \pmb{$\mu$} & 95.65 & 90.56 & 5.47\% & \cellcolor{myg}19.52 & \cellcolor{myr}22.52 & 14.31\% & 0.14 & 0.33 & 0.19\\
\cline{2-11}
& \large \pmb{$\sigma$} & 0.28 & 1.63 & & 0.53 & 1.72 & & 0.10& 0.37 & \\
\cline{1-2}\tabucline[2pt]{3-11}
\multirow{2}*{\parbox[c][1cm]{2.1cm}{\centering indigo}} & \large \pmb{$\mu$} & 98.81 & 93.68 & 5.32\% & \cellcolor{myr}12.92 & \cellcolor{myg}9.81 & 27.35\% & 0.07 & 0.07 & 0.00\\
\cline{2-11}
& \large \pmb{$\sigma$} & 0.05 & 1.39 & & 2.60 & 1.95 & & 0.06 & 0.01 &\\
\cline{1-2}\tabucline[2pt]{3-11}
\multirow{2}*{\parbox[c][1cm]{2.1cm}{\centering ledbat}} & \large \pmb{$\mu$} & 97.48 & 92.12 & 5.65\% & 49.69 & 45.40 & 9.02\% & 0.56 & 0.51 & 0.05\\
\cline{2-11}
& \large \pmb{$\sigma$} & 0.00 & 6.70 & & 0.00 & 6.41 & & 0.00& 0.05 & \\
\cline{1-2}\tabucline[2pt]{3-11}
\multirow{2}*{\parbox[c][1cm]{2.1cm}{\centering pcc}} & \large \pmb{$\mu$} & \cellcolor{myg}92.87 & \cellcolor{myr}59.70 & 43.49\% & 7.04 & 6.39 & 9.63\% & 0.04 & 0.06 & 0.02\\
\cline{2-11}
& \large \pmb{$\sigma$} & 0.60 & 18.32 & & 0.61 & 0.39 & & 0.07 & 0.01&\\
\cline{1-2}\tabucline[2pt]{3-11}
\multirow{2}*{\parbox[c][1cm]{2.1cm}{\centering pcc\_exp}} & \large \pmb{$\mu$} & 88.20 & 88.01 & 0.22\% & \cellcolor{myr}81.27 & \cellcolor{myg}28.61 & 95.86\% & 1.09 & 0.34 & 0.75\\
\cline{2-11}
& \large \pmb{$\sigma$} & 3.38 & 2.44 & & 47.22 & 20.00 & & 1.46 & 0.73 & \\
\cline{1-2}\tabucline[2pt]{3-11}
\multirow{2}*{\parbox[c][1cm]{2.1cm}{\centering quic}} & \large \pmb{$\mu$} & 77.55 & 71.77 & 7.73\% & \cellcolor{myg}5.41 & \cellcolor{myr}6.34 & 15.95\% & 0.13 & 0.08 & 0.05\\
\cline{2-11}
& \large \pmb{$\sigma$} & 0.39 & 0.71 & & 0.00 & 0.04 & & 0.13 & 0.05 & \\
\cline{1-2}\tabucline[2pt]{3-11}
\multirow{2}*{\parbox[c][1cm]{2.1cm}{\centering scream}} & \large \pmb{$\mu$} & 0.22 & 0.22 & 2.02\% &\cellcolor{myg}5.41 & \cellcolor{myr}6.58 &  19.55\% & 0.12 & 0.00 &0.12\\
\cline{2-11}
& \large \pmb{$\sigma$} & 0.00 & 0.00 & & 0.05 & 0.05 & & 0.20 & 0.00 & \\
\cline{1-2}\tabucline[2pt]{3-11}
\multirow{2}*{\parbox[c][1cm]{2.1cm}{\centering sprout}} & \large \pmb{$\mu$} & \cellcolor{myg}42.35 & \cellcolor{myr}36.20 & 15.65\% & 13.71 & 14.06 & 2.56\% & 0.15 & 0.09& 0.05\\
\cline{2-11}
& \large \pmb{$\sigma$} & 0.75 & 0.43 & & 0.11 & 0.13 & & 0.22 & 0.10 &\\
\cline{1-2}\tabucline[2pt]{3-11}
\multirow{2}*{\parbox[c][1cm]{2.1cm}{\centering taova}} & \large \pmb{$\mu$} & 92.84 & 84.09 & 9.89\% & \cellcolor{myg}6.10 & \cellcolor{myr}8.68 & 34.97\% & 0.08 & 0.05 & 0.03\\
\cline{2-11}
& \large \pmb{$\sigma$} & 0.04 & 0.62 & & 0.00 & 0.26 & & 0.04& 0.02 & \\
\cline{1-2}\tabucline[2pt]{3-11}
\multirow{2}*{\parbox[c][1cm]{2.1cm}{\centering vegas}} & \large \pmb{$\mu$} & \cellcolor{myg}99.60 & \cellcolor{myr}84.32 & 16.61\% & \cellcolor{myr}30.84 & \cellcolor{myg}24.28 & 23.83\% & 0.08 & 0.06 & 0.2\\
\cline{2-11}
& \large \pmb{$\sigma$} & 0.02 & 11.08 & & 7.85 & 14.23 & & 0.09 & 0.01 & \\
\cline{1-2}\tabucline[2pt]{3-11}
\multirow{2}*{\parbox[c][1cm]{2.1cm}{\centering verus}} & \large \pmb{$\mu$} & 97.17 & 92.52 & 4.91\% & \cellcolor{myg}63.48 &\cellcolor{myr}75.24 & 16.95\% & 4.09 & 4.19 & 0.11\\
\cline{2-11}
& \large \pmb{$\sigma$} & 1.52 & 1.63 & & 0.57 & 2.49 & & 0.14 & 0.14 &\\
\cline{1-2}\tabucline[2pt]{3-11}
%%%%%%%%%%%%%%%%%%%%%%%%%%%
\multirow{2}*{\parbox[c][1cm]{2.1cm}{\centering vivace}} & \large \pmb{$\mu$} & \cellcolor{myg}85.63 & \cellcolor{myr}56.78 & 40.51\% & \cellcolor{myg}8.10 & \cellcolor{myr}12.16 & 40.06\% & 0.06 & 0.12 & 0.06\\
\cline{2-11}
& \large \pmb{$\sigma$} & 0.61 & 26.77 & & 8.11 & 8.15 & & 0.06 & 0.06 & \\
\cline{1-2}\tabucline[2pt]{3-11}
%%%%%%%%%%%%%%%%%%%%%%%%%
\end{tabu}}
\label{tab:tab3}
\end{table*}

\begin{table*}[h!]
\centering
\Large
\caption{Testing results for the delay $X=5$ ms \emph{(continuation)}.}
 
\resizebox*{\textwidth}{!}{\begin{tabu}{|c|cV{5}c|c|cV{5}c|c|cV{5}c|c|cV{5}}
\hline
\multirow{2}*{\parbox[c][2.5cm]{2.1cm}{\centering \bf \large Scheme}} &  \multicolumn{1}{c|}{\multirow{2}*{\parbox[c][2.5cm]{0.0cm}{}}} & \multicolumn{3}{c|}{\parbox[c][1cm]{2.7cm}{\bf \large Rate (Mbps)}} & \multicolumn{3}{c|}{\parbox[c][1cm]{2.3cm}{\bf \large Delay (ms)}} & \multicolumn{3}{c|}{\parbox[c][1cm]{1.8cm}{\bf \large Loss (\%)}}\\ 
\cline{3-11}
 & \multicolumn{1}{c|}{} & \parbox[c][1.5cm]{1.8cm}{\centering \bf \normalsize CoCo-Beholder}  & \parbox[1cm]{1.9cm}{\centering \bf \normalsize Pantheon} & \multicolumn{1}{c|}{\parbox{1.8cm}{\centering \pmb{$d_r$}}} & \parbox{1.8cm}{\centering \bf \normalsize CoCo-Beholder} & \parbox{1.8cm}{\centering \bf \normalsize Pantheon} & \multicolumn{1}{c|}{\parbox{1.8cm}{\centering \pmb{$d_r$}}} & \parbox{1.8cm}{\centering \bf \normalsize CoCo-Beholder} & \parbox{1.8cm}{\centering \bf \normalsize Pantheon} &\multicolumn{1}{c|}{ \parbox{1.8cm}{\centering \pmb{$\Delta$}}}\\
\cline{1-2}\tabucline[2pt]{3-11}
\multirow{2}*{\parbox[c][1cm]{2.1cm}{\centering bic}} & \large \pmb{$\mu$} & 99.63 & 99.44 & 0.19\% & 125.79 & 124.19 & 1.28\% & 3.63 & 3.35 & 0.28\\
\cline{2-11}
& \large \pmb{$\sigma$} & 0.01 & 0.13 & & 0.24 & 0.53 & & 0.14 & 0.85 & \\
\cline{1-2}\tabucline[2pt]{3-11}
\multirow{2}*{\parbox[c][1cm]{2.1cm}{\centering cdg}} & \large \pmb{$\mu$} & 95.95 \cellcolor{myg}& \cellcolor{myr}85.84 & 11.12\% & 13.85 & 12.55 & 9.89\% & 0.08 & 0.09 & 0.01\\
\cline{2-11}
& \large \pmb{$\sigma$} & 1.96 & 4.69 & & 2.42 & 3.26 & & 0.09 & 0.03 & \\
\cline{1-2}\tabucline[2pt]{3-11}
\multirow{2}*{\parbox[c][1cm]{2.1cm}{\centering highspeed}} & \large \pmb{$\mu$} & 99.62 & 99.42 & 0.21\% &\cellcolor{myr}121.12 & \cellcolor{myg}109.55 & 10.03\% & 2.50 & 2.40 & 0.09\\
\cline{2-11}
& \large \pmb{$\sigma$} & 0.00 & 0.09 & & 4.83 & 9.12 & & 0.14 & 0.17 &\\
\cline{1-2}\tabucline[2pt]{3-11}
\multirow{2}*{\parbox[c][1cm]{2.1cm}{\centering htcp}} & \large \pmb{$\mu$} & 99.62 & 99.40 & 0.22\% & \cellcolor{myr}117.69 & \cellcolor{myg}84.60 & 32.72\% & 2.58 & 1.89 & 0.69\\
\cline{2-11}
& \large \pmb{$\sigma$} & 0.00 & 0.09 & & 0.14 & 12.29 && 0.10 & 0.47 &\\
\cline{1-2}\tabucline[2pt]{3-11}
\multirow{2}*{\parbox[c][1cm]{2.1cm}{\centering hybla}} & \large \pmb{$\mu$} & 99.28 & 98.97 & 0.31\% & 117.24 & 110.13 & 6.25\% & 2.25 & 1.71 & 0.53\\
\cline{2-11}
& \large \pmb{$\sigma$} & 0.00 & 0.10 & & 2.06 & 14.42 & & 0.10 & 0.18 & \\
\cline{1-2}\tabucline[2pt]{3-11}
\multirow{2}*{\parbox[c][1cm]{2.1cm}{\centering illinois}} & \large \pmb{$\mu$} & 99.62 & 99.47& 0.15\%  & 91.38 & 91.06 & 0.35\% & 2.18 & 2.16 & 0.02\\
\cline{2-11}
& \large \pmb{$\sigma$} & 0.00 & 0.06 & & 6.31 & 4.01 & & 0.08 & 0.14 &\\
\cline{1-2}\tabucline[2pt]{3-11}
\multirow{2}*{\parbox[c][1cm]{2.1cm}{\centering lp}} & \large \pmb{$\mu$} & 99.62 & 99.46 & 0.16\% & \cellcolor{myr}92.04 & \cellcolor{myg}81.65 & 11.96\% & 2.10 & 1.81 & 0.29\\
\cline{2-11}
& \large \pmb{$\sigma$} & 0.00 & 0.13 & & 15.84 & 12.64 & & 0.08 & 0.59 &\\
\cline{1-2}\tabucline[2pt]{3-11}
\multirow{2}*{\parbox[c][1cm]{2.1cm}{\centering nv}} & \large \pmb{$\mu$} & 97.62 & 95.25 & 2.46\% & \cellcolor{myg}7.95 & \cellcolor{myr}8.80 & 10.17\% & 0.03 & 0.08 & 0.06\\
\cline{2-11}
& \large \pmb{$\sigma$} & 0.04 & 0.30 & & 0.05 & 0.16 & & 0.06 & 0.01 &\\
\cline{1-2}\tabucline[2pt]{3-11}
\multirow{2}*{\parbox[c][1cm]{2.1cm}{\centering reno}} & \large \pmb{$\mu$} & 99.62 & 99.40 & 0.22\% & \cellcolor{myr}91.96 & \cellcolor{myg}79.47 & 14.57\% & 2.09 & 1.82 & 0.27\\
\cline{2-11}
& \large \pmb{$\sigma$} & 0.01 & 0.18 & & 11.73 & 15.52 & & 0.10 & 0.49 & \\
\cline{1-2}\tabucline[2pt]{3-11}
\multirow{2}*{\parbox[c][1cm]{2.1cm}{\centering scalable}} & \large \pmb{$\mu$} & 99.63 & 99.43 & 0.20\% & 125.98 & 124.86 & 0.89\% & 4.85 & 4.41 & 0.44\\
\cline{2-11}
& \large \pmb{$\sigma$} & 0.01 & 0.08 & & 0.26 & 0.12 & & 0.16 & 1.02&\\
\cline{1-2}\tabucline[2pt]{3-11}
\multirow{2}*{\parbox[c][1cm]{2.1cm}{\centering veno    }} & \large \pmb{$\mu$} & 99.62 & 99.41 & 0.21\% & 89.66 & 83.50 & 7.11\% & 1.94 & 1.81 & 0.12\\
\cline{2-11}
& \large \pmb{$\sigma$} & 0.01 & 0.14 & & 10.76 & 2.01 &&0.06 & 0.20 & \\
\cline{1-2}\tabucline[2pt]{3-11}
\multirow{2}*{\parbox[c][1cm]{2.1cm}{\centering westwood}} & \large \pmb{$\mu$} & 98.68 & 95.47 & 3.31\% & 82.29 & 76.31 & 7.54\% & 1.76 & 1.64 & 0.12\\
\cline{2-11}
& \large \pmb{$\sigma$} & 0.17 & 1.38 & & 9.56 & 17.05 & & 0.00 & 0.43 & \\
\cline{1-2}\tabucline[2pt]{3-11}
%%%%%%%%%%%%%%%%%%%%%%%%%
\multirow{2}*{\parbox[c][1cm]{2.1cm}{\centering yeah}} & \large \pmb{$\mu$} & 99.63 & 99.26 & 0.37\% & \cellcolor{myr}34.18 & \cellcolor{myg}28.07 & 19.63\% & 0.26 & 0.36 & 0.10\\
\cline{2-11}
& \large \pmb{$\sigma$} & 0.00 & 0.36 & & 0.38 & 5.27 & & 0.09 & 0.07 &\\
\cline{1-2}\tabucline[2pt]{3-11}
%%%%%%%%%%%%%%%%%%%%%%%%%
\end{tabu}}
\label{tab:tab7}
\end{table*}

\begin{table*}[h!]
\centering
\Large
\caption{Testing results for the delay $X=20$ ms.}
 
\resizebox*{\textwidth}{!}{\begin{tabu}{|c|cV{5}c|c|cV{5}c|c|cV{5}c|c|cV{5}}
\hline
\multirow{2}*{\parbox[c][2.5cm]{2.1cm}{\centering \bf \large Scheme}} &  \multicolumn{1}{c|}{\multirow{2}*{\parbox[c][2.5cm]{0.0cm}{}}} & \multicolumn{3}{c|}{\parbox[c][1cm]{2.7cm}{\bf \large Rate (Mbps)}} & \multicolumn{3}{c|}{\parbox[c][1cm]{2.3cm}{\bf \large Delay (ms)}} & \multicolumn{3}{c|}{\parbox[c][1cm]{1.8cm}{\bf \large Loss (\%)}}\\ 
\cline{3-11}
 & \multicolumn{1}{c|}{} & \parbox[c][1.5cm]{1.8cm}{\centering \bf \normalsize CoCo-Beholder}  & \parbox[1cm]{1.9cm}{\centering \bf \normalsize Pantheon} & \multicolumn{1}{c|}{\parbox{1.8cm}{\centering \pmb{$d_r$}}} & \parbox{1.8cm}{\centering \bf \normalsize CoCo-Beholder} & \parbox{1.8cm}{\centering \bf \normalsize Pantheon} & \multicolumn{1}{c|}{\parbox{1.8cm}{\centering \pmb{$d_r$}}} & \parbox{1.8cm}{\centering \bf \normalsize CoCo-Beholder} & \parbox{1.8cm}{\centering \bf \normalsize Pantheon} &\multicolumn{1}{c|}{ \parbox{1.8cm}{\centering \pmb{$\Delta$}}}\\
\cline{1-2}\tabucline[2pt]{3-11}
\multirow{2}*{\parbox[c][1cm]{2.1cm}{\centering bbr}} & \large \pmb{$\mu$} & 97.76 & 97.59 & 0.18\% & \cellcolor{myg}50.35 &\cellcolor{myr}69.98 & 32.62\% & 0.26 & 0.60 & 0.34\\
\cline{2-11}
& \large \pmb{$\sigma$} & 0.00 & 0.06 & & 28.84 & 2.12 & & 0.09 & 0.06 & \\
\cline{1-2}\tabucline[2pt]{3-11}
\multirow{2}*{\parbox[c][1cm]{2.1cm}{\centering copa}} & \large \pmb{$\mu$} & 83.86 & 82.70 & 1.40\% &\cellcolor{myr}45.42 & \cellcolor{myg}24.35 & 60.39\% & 0.21 & 0.22 & 0.01\\
\cline{2-11}
& \large \pmb{$\sigma$} & 5.38 & 4.07 & & 1.97 & 1.30 & & 0.09 & 0.02 &\\
\cline{1-2}\tabucline[2pt]{3-11}
\multirow{2}*{\parbox[c][1cm]{2.1cm}{\centering cubic}} & \large \pmb{$\mu$} & 97.89 & 97.70 & 0.19\% & 139.87 & 136.26 & 2.62\% & 1.15 & 1.17 & 0.02\\
\cline{2-11}
& \large \pmb{$\sigma$} & 0.00 & 0.08 & & 0.30 & 4.78 & & 0.00 & 0.12 &\\
\cline{1-2}\tabucline[2pt]{3-11}
\multirow{2}*{\parbox[c][1cm]{2.1cm}{\centering fillp}} & \large \pmb{$\mu$} & 94.99 & 96.11 & 1.16\% &\cellcolor{myg}40.19 & \cellcolor{myr}48.80 & 19.36\% & 1.28 & 1.42 & 0.14\\
\cline{2-11}
& \large \pmb{$\sigma$} & 0.70 & 0.70 & &2.09 & 5.67 & & 0.15 & 0.17 & \\
\cline{1-2}\tabucline[2pt]{3-11}
\multirow{2}*{\parbox[c][1cm]{2.1cm}{\centering fillp\_sheep}} & \large \pmb{$\mu$} & 86.97 & 90.29 & 3.75\% & 34.85 & 37.50 & 7.33\% & 0.77 & 0.87 & 0.10\\
\cline{2-11}
& \large \pmb{$\sigma$} & 3.57 & 1.54 & & 0.75 & 0.83 & & 0.15 & 0.18 &\\
\cline{1-2}\tabucline[2pt]{3-11}
\multirow{2}*{\parbox[c][1cm]{2.1cm}{\centering indigo}} & \large \pmb{$\mu$} & 96.47 & 94.84 & 1.70\% & 28.24 & 27.33 & 3.29\% & 0.27 & 0.28 & 0.01\\
\cline{2-11}
& \large \pmb{$\sigma$} & 1.07 & 2.17 & & 4.72 & 4.25 & & 0.09 & 0.05 &\\
\cline{1-2}\tabucline[2pt]{3-11}
\multirow{2}*{\parbox[c][1cm]{2.1cm}{\centering ledbat}} & \large \pmb{$\mu$} & 64.08 & 59.26 & 7.81\% & 31.58 & 29.50 & 6.84\% & 0.44 & 0.43 & 0.01\\
\cline{2-11}
& \large \pmb{$\sigma$} & 2.29 & 4.12 & & 3.61 & 2.33 & & 0.12 & 0.15 &\\
\cline{1-2}\tabucline[2pt]{3-11}
\multirow{2}*{\parbox[c][1cm]{2.1cm}{\centering pcc}} & \large \pmb{$\mu$} & \cellcolor{myg}89.08 & \cellcolor{myr}70.35 & 23.49\% & \cellcolor{myg}31.65 & \cellcolor{myr}42.43 & 29.12\% & 0.25 & 0.36 & 0.11\\
\cline{2-11}
& \large \pmb{$\sigma$} & 0.85 & 8.01 & & 1.41 & 6.55 & & 0.07 & 0.05 &\\
\cline{1-2}\tabucline[2pt]{3-11}
\multirow{2}*{\parbox[c][1cm]{2.1cm}{\centering pcc\_exp}} & \large \pmb{$\mu$} & 90.55 & 85.94 & 5.22\% & \cellcolor{myg}64.16 & \cellcolor{myr}77.44 & 18.75\% &  0.46 &  1.33 & 0.88\\
\cline{2-11}
& \large \pmb{$\sigma$} & 1.97 & 4.05 & & 27.03 & 9.57 & & 0.60 & 0.49 & \\
\cline{1-2}\tabucline[2pt]{3-11}
\multirow{2}*{\parbox[c][1cm]{2.1cm}{\centering quic}} & \large \pmb{$\mu$} & 77.42 & 70.48 & 9.38\% & 20.41 & 21.52 & 5.32\% & 0.27 & 0.30 & 0.03
\\
\cline{2-11}
& \large \pmb{$\sigma$} & 1.12 & 1.00 & & 0.00 & 0.26 & & 0.03 & 0.08 &\\
\cline{1-2}\tabucline[2pt]{3-11}
\multirow{2}*{\parbox[c][1cm]{2.1cm}{\centering scream}} & \large \pmb{$\mu$} & 0.22 & 0.22 & 1.86\% & 20.44 & 21.65 & 5.73\% & 0.28 & 0.35 & 0.07\\
\cline{2-11}
& \large \pmb{$\sigma$} & 0.00 & 0.00 & & 0.00 & 0.09 & & 0.27 & 0.00& \\
\cline{1-2}\tabucline[2pt]{3-11}
\multirow{2}*{\parbox[c][1cm]{2.1cm}{\centering sprout}} & \large \pmb{$\mu$} & 15.69 & 15.80 & 0.71\% & 27.58 & 27.31 & 1.01\% & 0.14 & 0.16 & 0.02\\
\cline{2-11}
& \large \pmb{$\sigma$} & 0.13 & 0.09 & & 0.42 & 0.37 & & 0.40 & 0.09 &  \\
\cline{1-2}\tabucline[2pt]{3-11}
\multirow{2}*{\parbox[c][1cm]{2.1cm}{\centering taova}} & \large \pmb{$\mu$} &\cellcolor{myg}92.05 & \cellcolor{myr}77.28 & 17.45\% & \cellcolor{myg}23.23 & \cellcolor{myr}33.26 & 35.51\% & 0.25 & 0.44 & 0.19\\
\cline{2-11}
& \large \pmb{$\sigma$} & 0.08 & 0.51 & & 0.00 & 0.46 & & 0.08 & 0.12& \\
\cline{1-2}\tabucline[2pt]{3-11}
\multirow{2}*{\parbox[c][1cm]{2.1cm}{\centering vegas}} & \large \pmb{$\mu$} & 97.88 & 88.85 & 9.67\% & \cellcolor{myr}84.73 & \cellcolor{myg}69.09 & 20.34\% & 1.80 & 0.95 & 0.85\\
\cline{2-11}
& \large \pmb{$\sigma$} & 0.01 & 15.28 & & 32.14 & 42.91 & & 0.38 & 0.70 & \\
\cline{1-2}\tabucline[2pt]{3-11}
\multirow{2}*{\parbox[c][1cm]{2.1cm}{\centering verus}} & \large \pmb{$\mu$} & 95.23 & 94.16 & 1.12\% & 133.97 & 137.58 & 2.66\% & 11.09 & 9.67 & 1.42\\
\cline{2-11}
& \large \pmb{$\sigma$} & 1.84 & 1.58 & & 0.48 & 0.56 & & 1.21 & 1.39 & \\
\cline{1-2}\tabucline[2pt]{3-11}
%%%%%%%%%%%%%%%%%%%%%%%%%
\multirow{2}*{\parbox[c][1cm]{2.1cm}{\centering vivace}} & \large \pmb{$\mu$} & 77.77 & 76.00 & 2.31\% & \cellcolor{myg}21.09 & \cellcolor{myr}26.98 & 24.51\% & 0.23 & 0.31 & 0.08\\
\cline{2-11}
& \large \pmb{$\sigma$} & 0.36 & 3.14 & & 0.15 & 7.20 & & 0.12 & 0.06 &\\
\cline{1-2}\tabucline[2pt]{3-11}
%%%%%%%%%%%%%%%%%%%%%%%%%
\end{tabu}}
\label{tab:tab4}
\end{table*}

\textcolor{white}{.}
\begin{table*}[h!]
\centering
\Large
\caption{Testing results for the delay $X=20$ ms \emph{(continuation)}.}
 
\resizebox*{\textwidth}{!}{\begin{tabu}{|c|cV{5}c|c|cV{5}c|c|cV{5}c|c|cV{5}}
\hline
\multirow{2}*{\parbox[c][2.5cm]{2.1cm}{\centering \bf \large Scheme}} &  \multicolumn{1}{c|}{\multirow{2}*{\parbox[c][2.5cm]{0.0cm}{}}} & \multicolumn{3}{c|}{\parbox[c][1cm]{2.7cm}{\bf \large Rate (Mbps)}} & \multicolumn{3}{c|}{\parbox[c][1cm]{2.3cm}{\bf \large Delay (ms)}} & \multicolumn{3}{c|}{\parbox[c][1cm]{1.8cm}{\bf \large Loss (\%)}}\\ 
\cline{3-11}
 & \multicolumn{1}{c|}{} & \parbox[c][1.5cm]{1.8cm}{\centering \bf \normalsize CoCo-Beholder}  & \parbox[1cm]{1.9cm}{\centering \bf \normalsize Pantheon} & \multicolumn{1}{c|}{\parbox{1.8cm}{\centering \pmb{$d_r$}}} & \parbox{1.8cm}{\centering \bf \normalsize CoCo-Beholder} & \parbox{1.8cm}{\centering \bf \normalsize Pantheon} & \multicolumn{1}{c|}{\parbox{1.8cm}{\centering \pmb{$d_r$}}} & \parbox{1.8cm}{\centering \bf \normalsize CoCo-Beholder} & \parbox{1.8cm}{\centering \bf \normalsize Pantheon} &\multicolumn{1}{c|}{ \parbox{1.8cm}{\centering \pmb{$\Delta$}}}\\
\cline{1-2}\tabucline[2pt]{3-11}
\multirow{2}*{\parbox[c][1cm]{2.1cm}{\centering bic}} & \large \pmb{$\mu$} & 97.87 & 97.62&  0.26\% & 140.61 & 139.15 & 1.04\%  & 4.32 & 4.23 & 0.09\\
\cline{2-11}
& \large \pmb{$\sigma$} & 0.02 & 0.05 & & 0.25 & 0.30 & & 0.08 & 0.36 &\\
\cline{1-2}\tabucline[2pt]{3-11}
\multirow{2}*{\parbox[c][1cm]{2.1cm}{\centering cdg}} & \large \pmb{$\mu$} & \cellcolor{myg}79.94 & \cellcolor{myr}34.11 & 80.36\% &\cellcolor{myr} 25.52 &\cellcolor{myg}21.90 & 15.25\% & 0.22 & 0.33 & 0.12\\
\cline{2-11}
& \large \pmb{$\sigma$} & 11.77 & 7.28 & & 4.54 & 0.03 & &0.08 & 0.08&\\
\cline{1-2}\tabucline[2pt]{3-11}
\multirow{2}*{\parbox[c][1cm]{2.1cm}{\centering highspeed}} & \large \pmb{$\mu$} & 97.87 & 97.57 & 0.31\% & 126.52 & 122.46 & 3.26\% & 2.94 & 2.78 & 0.16\\
\cline{2-11}
& \large \pmb{$\sigma$} & 0.00 & 0.15 & & 0.18 & 3.21 & & 0.02 & 0.17 &\\
\cline{1-2}\tabucline[2pt]{3-11}
\multirow{2}*{\parbox[c][1cm]{2.1cm}{\centering htcp}} & \large \pmb{$\mu$} & 97.87 & 97.49 & 0.39\% & 140.38 & 129.11 & 8.36\%  & 2.35 & 2.55 & 0.20\\
\cline{2-11}
& \large \pmb{$\sigma$} & 0.01 & 0.22 &  & 0.14 & 12.17 & & 0.00 & 0.31 &\\
\cline{1-2}\tabucline[2pt]{3-11}
\multirow{2}*{\parbox[c][1cm]{2.1cm}{\centering hybla}} & \large \pmb{$\mu$} & 97.36 & 94.52 & 2.96\% & 139.29 & 138.58 & 0.51\%  & 3.11 & 4.89 & 1.79\\
\cline{2-11}
& \large \pmb{$\sigma$} & 0.00 & 3.73 & & 0.16 & 0.24 & &0.24 &0.39 &\\
\cline{1-2}\tabucline[2pt]{3-11}
\multirow{2}*{\parbox[c][1cm]{2.1cm}{\centering illinois}} & \large \pmb{$\mu$} & 97.87 & 97.53 & 0.35\% & 111.35 & 112.53 & 1.06\% &  2.73 & 2.71 & 0.02\\
\cline{2-11}
& \large \pmb{$\sigma$} & 0.01 & 0.15 & & 0.48 & 5.84 & & 0.08 & 0.22& \\
\cline{1-2}\tabucline[2pt]{3-11}
\multirow{2}*{\parbox[c][1cm]{2.1cm}{\centering lp}} & \large \pmb{$\mu$} & 97.87 & 96.59 & 1.32\% & 111.80 & 113.48 & 1.50\% & 2.33 & 2.16 & 0.16
\\
\cline{2-11}
& \large \pmb{$\sigma$} & 0.00 & 3.34 & & 10.46 & 4.44& & 0.09 & 0.15 &\\
\cline{1-2}\tabucline[2pt]{3-11}
\multirow{2}*{\parbox[c][1cm]{2.1cm}{\centering nv}} & \large \pmb{$\mu$} & \cellcolor{myg}44.88 & \cellcolor{myr}39.53 & 12.68\% & 21.18 & 21.92 & 3.43\% & 0.38 & 0.37 & 0.00\\
\cline{2-11}
& \large \pmb{$\sigma$} & 0.04 & 1.21 & & 0.02 & 0.02 & & 0.13 & 0.03&\\
\cline{1-2}\tabucline[2pt]{3-11}
\multirow{2}*{\parbox[c][1cm]{2.1cm}{\centering reno}} & \large \pmb{$\mu$} & 97.87 & 96.66 & 1.25\% & 111.87 & 111 & 0.78\% & 2.35 & 2.20 & 0.15
\\
\cline{2-11}
& \large \pmb{$\sigma$} & 0.00 & 2.86 & & 10.35 & 6.02 & & 0.08 & 0.15&\\
\cline{1-2}\tabucline[2pt]{3-11}
\multirow{2}*{\parbox[c][1cm]{2.1cm}{\centering scalable}} & \large \pmb{$\mu$} & 97.87 & 97.64 & 0.23\% & 141.96 & 139.94& 1.43\% & 5.75 & 5.40 & 0.35\\
\cline{2-11}
& \large \pmb{$\sigma$} & 0.02 & 0.13 & & 1.64 & 0.18 & & 0.09 & 0.92 &\\
\cline{1-2}\tabucline[2pt]{3-11}
\multirow{2}*{\parbox[c][1cm]{2.1cm}{\centering veno}} & \large \pmb{$\mu$} & 97.87 & 96.65 & 1.26\% & 111.74 & 109.97& 1.60\% & 2.29 & 2.13 & 0.16\\
\cline{2-11}
& \large \pmb{$\sigma$} & 0.00& 0.86 & & 10.55 & 6.83 & & 0.10& 0.12 & \\
\cline{1-2}\tabucline[2pt]{3-11}
\multirow{2}*{\parbox[c][1cm]{2.1cm}{\centering westwood}} & \large \pmb{$\mu$} & 58.45 & 53.02 & 9.75\% & 139.60 & 133.11 & 4.76\% & 2.96 & 3.33 & 0.37\\
\cline{2-11}
& \large \pmb{$\sigma$} &0.84 &2.64 && 0.11 & 9.12 & &0.04 & 0.18 & \\
\cline{1-2}\tabucline[2pt]{3-11}
%%%%%%%%%%%%%%%%%%%%%%%%%
\multirow{2}*{\parbox[c][1cm]{2.1cm}{\centering yeah}} & \large \pmb{$\mu$} & 97.86 & 95.14 & 2.82\% & 60.86 & 60.79 & 0.11\% & 1.80 & 1.60 & 0.20\\
\cline{2-11}
& \large \pmb{$\sigma$} & 0.01 & 2.51 & & 0.52 & 2.45 & & 0.00 & 0.38& \\
\cline{1-2}\tabucline[2pt]{3-11}
%%%%%%%%%%%%%%%%%%%%%%%%%
\end{tabu}}
\label{tab:tab8}
\end{table*}

\newpage

\FloatBarrier

Figure~\ref{fig:compr} shows the example average rate plots by CoCo-Beholder (on the left) and by Pantheon (on the right) for BIC TCP, Scalable TCP, and Sprout in the case of the delay $X=10$ ms. The corresponding per-packet one-way delay plots of the schemes can be found in Figure~\ref{fig:compd} in Section~\ref{sec:tfirst}.\\

\begin{figure}[h!]
    \centering
    \subfloat[BIC TCP by CoCo-Beholder]{{\includegraphics[width=0.5\textwidth]{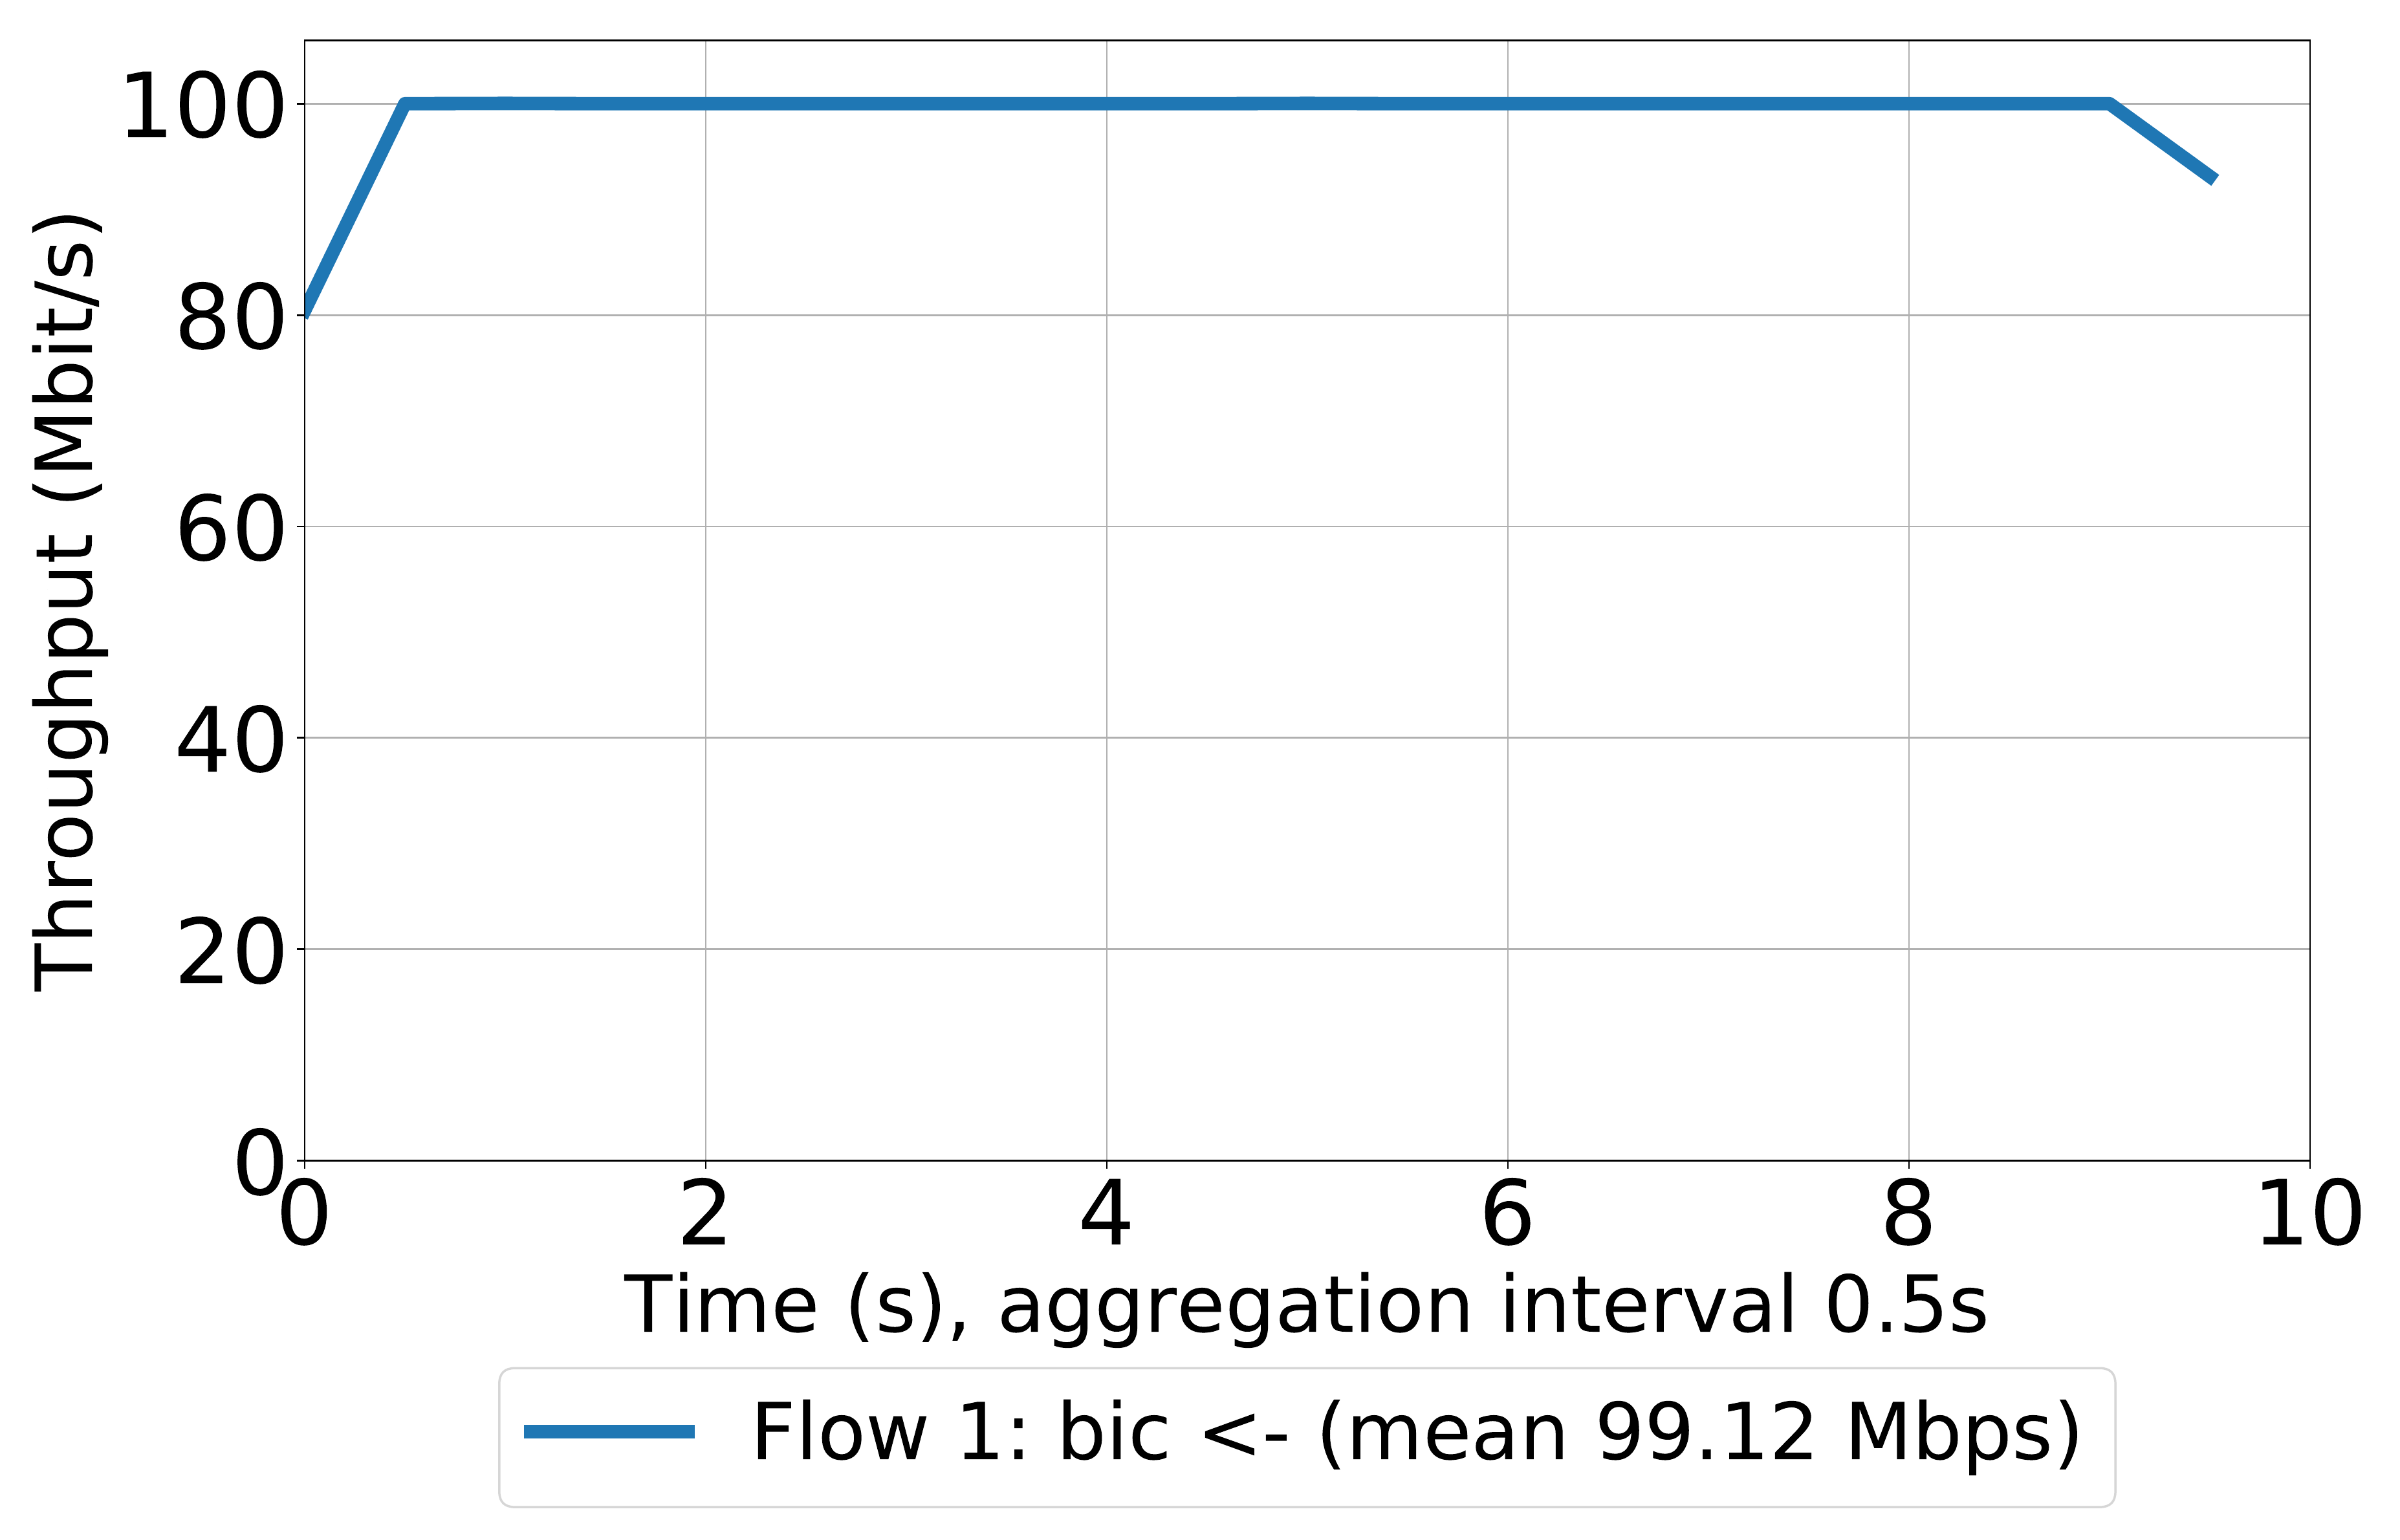} }}%
    \subfloat[BIC TCP by Pantheon]{{\includegraphics[width=0.5\textwidth]{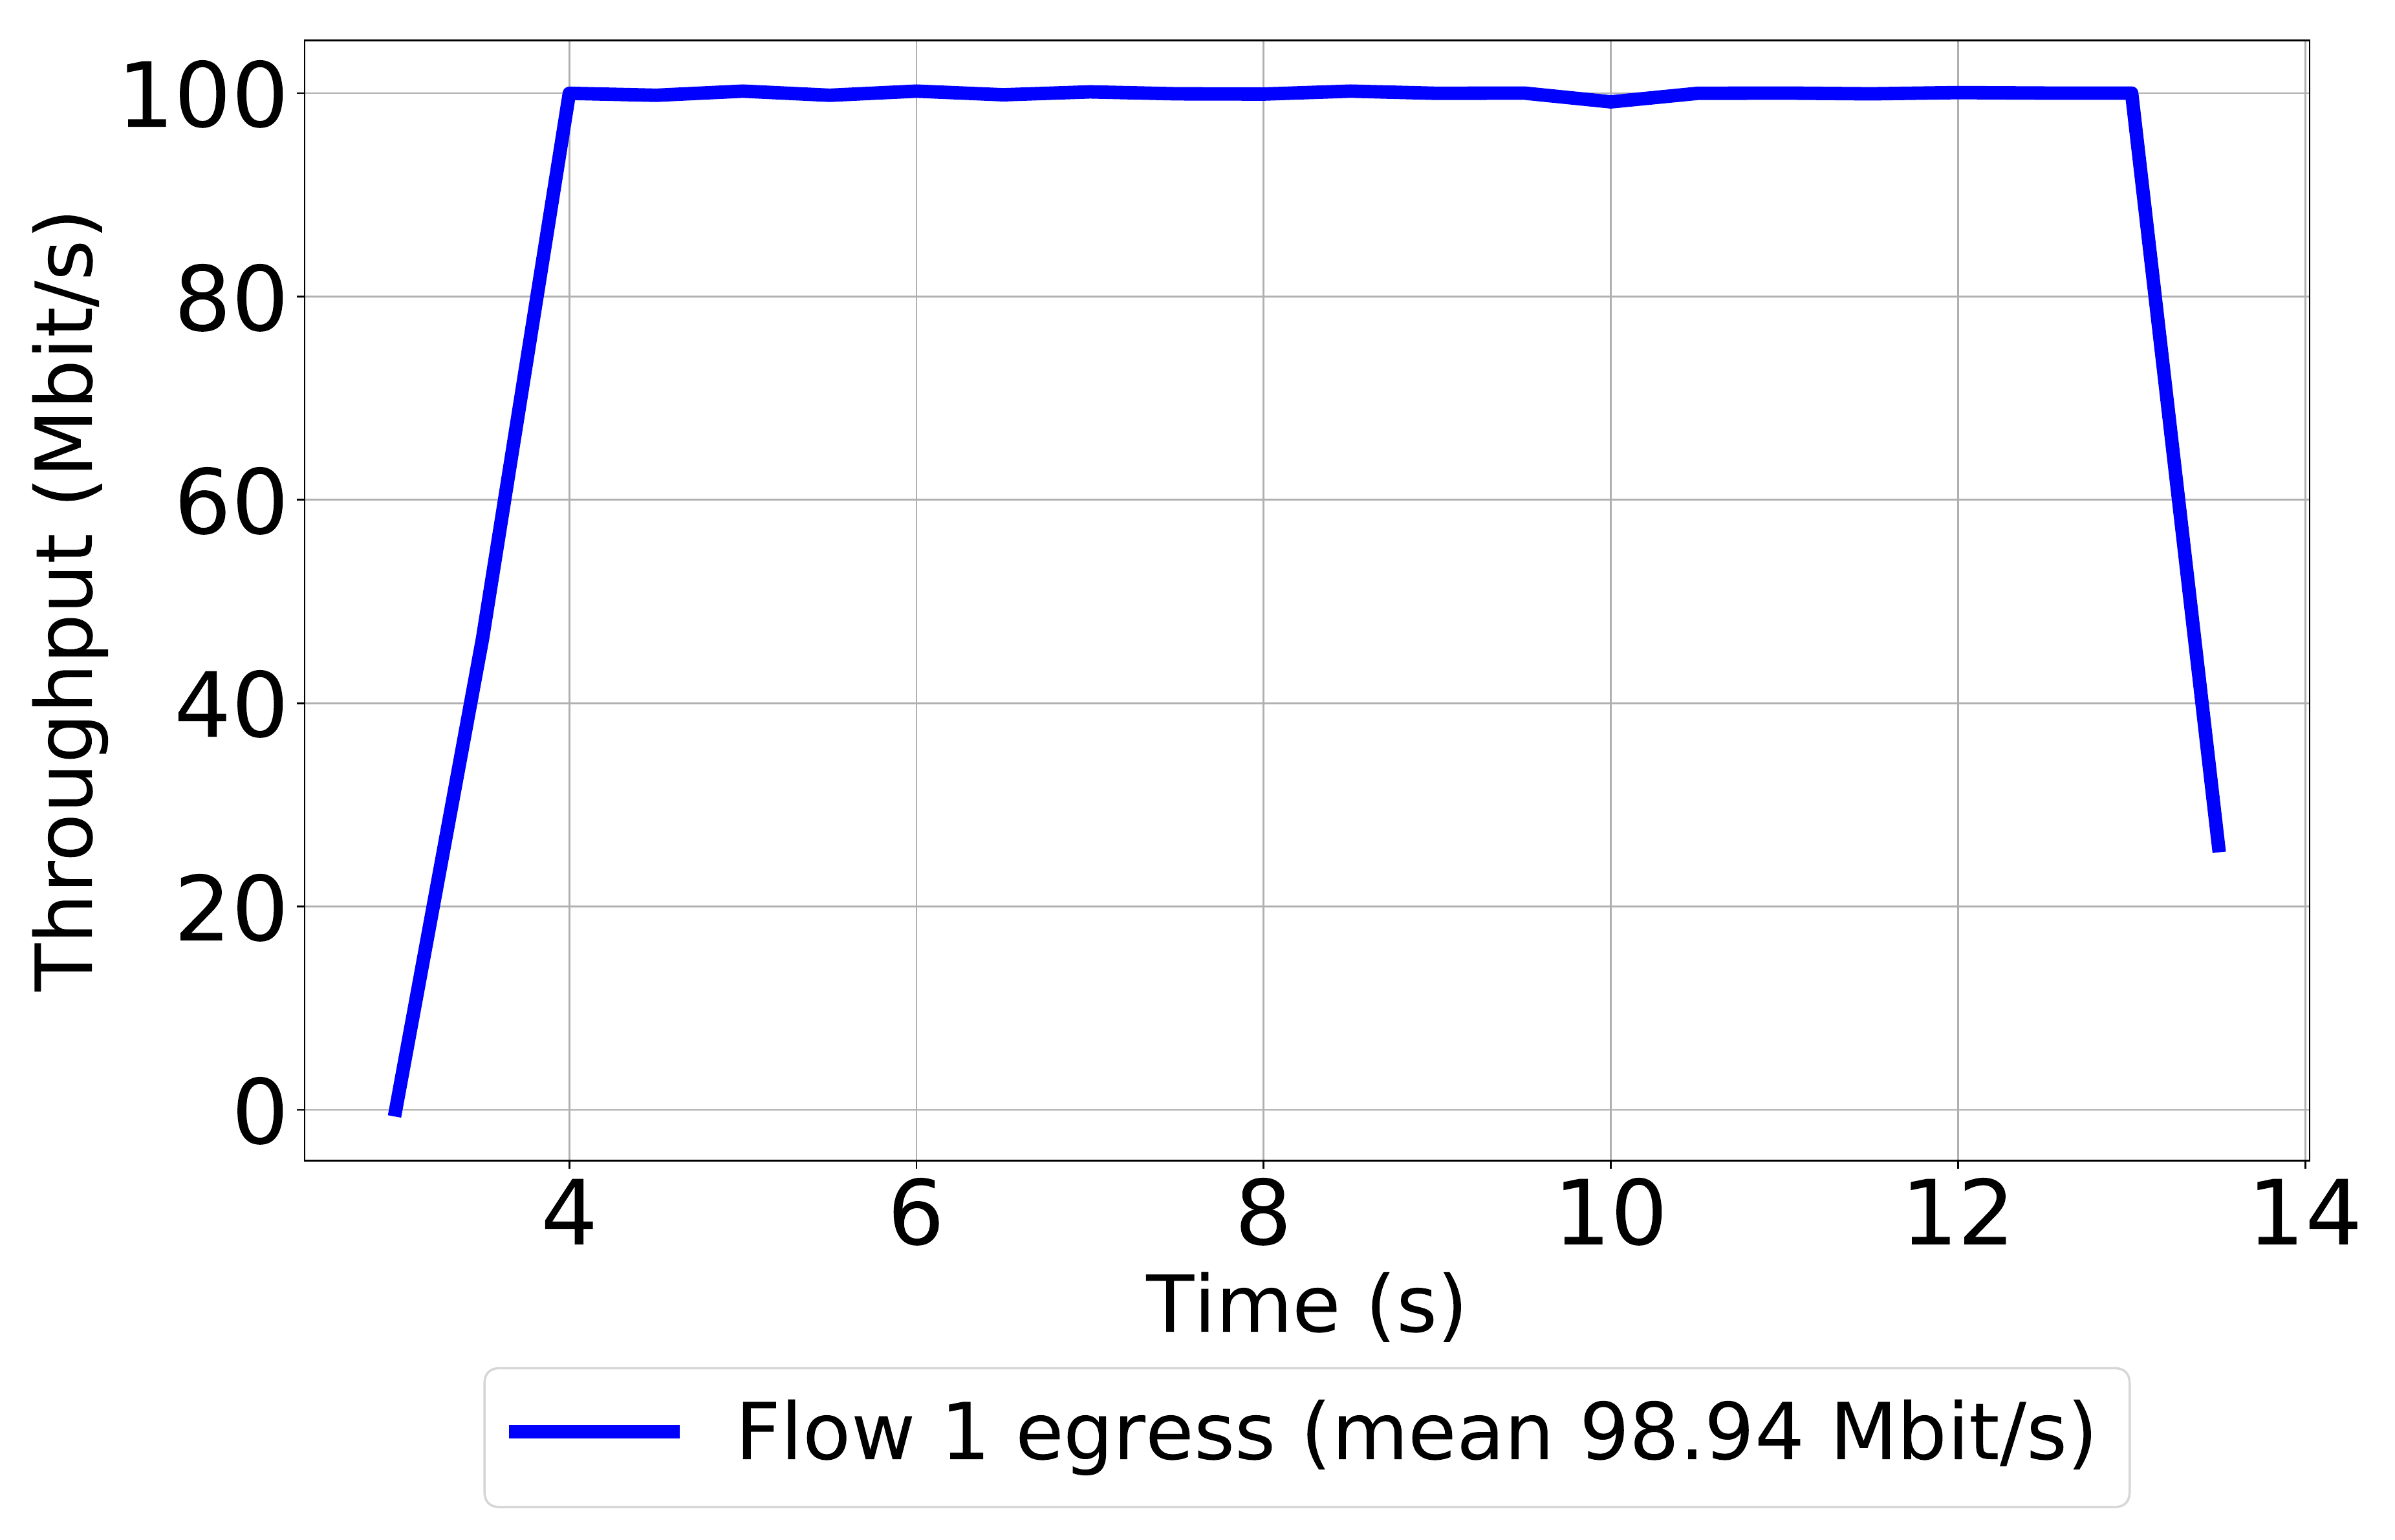} }}\\
    \subfloat[Scalable TCP by CoCo-Beholder]{{\includegraphics[width=0.5\textwidth]{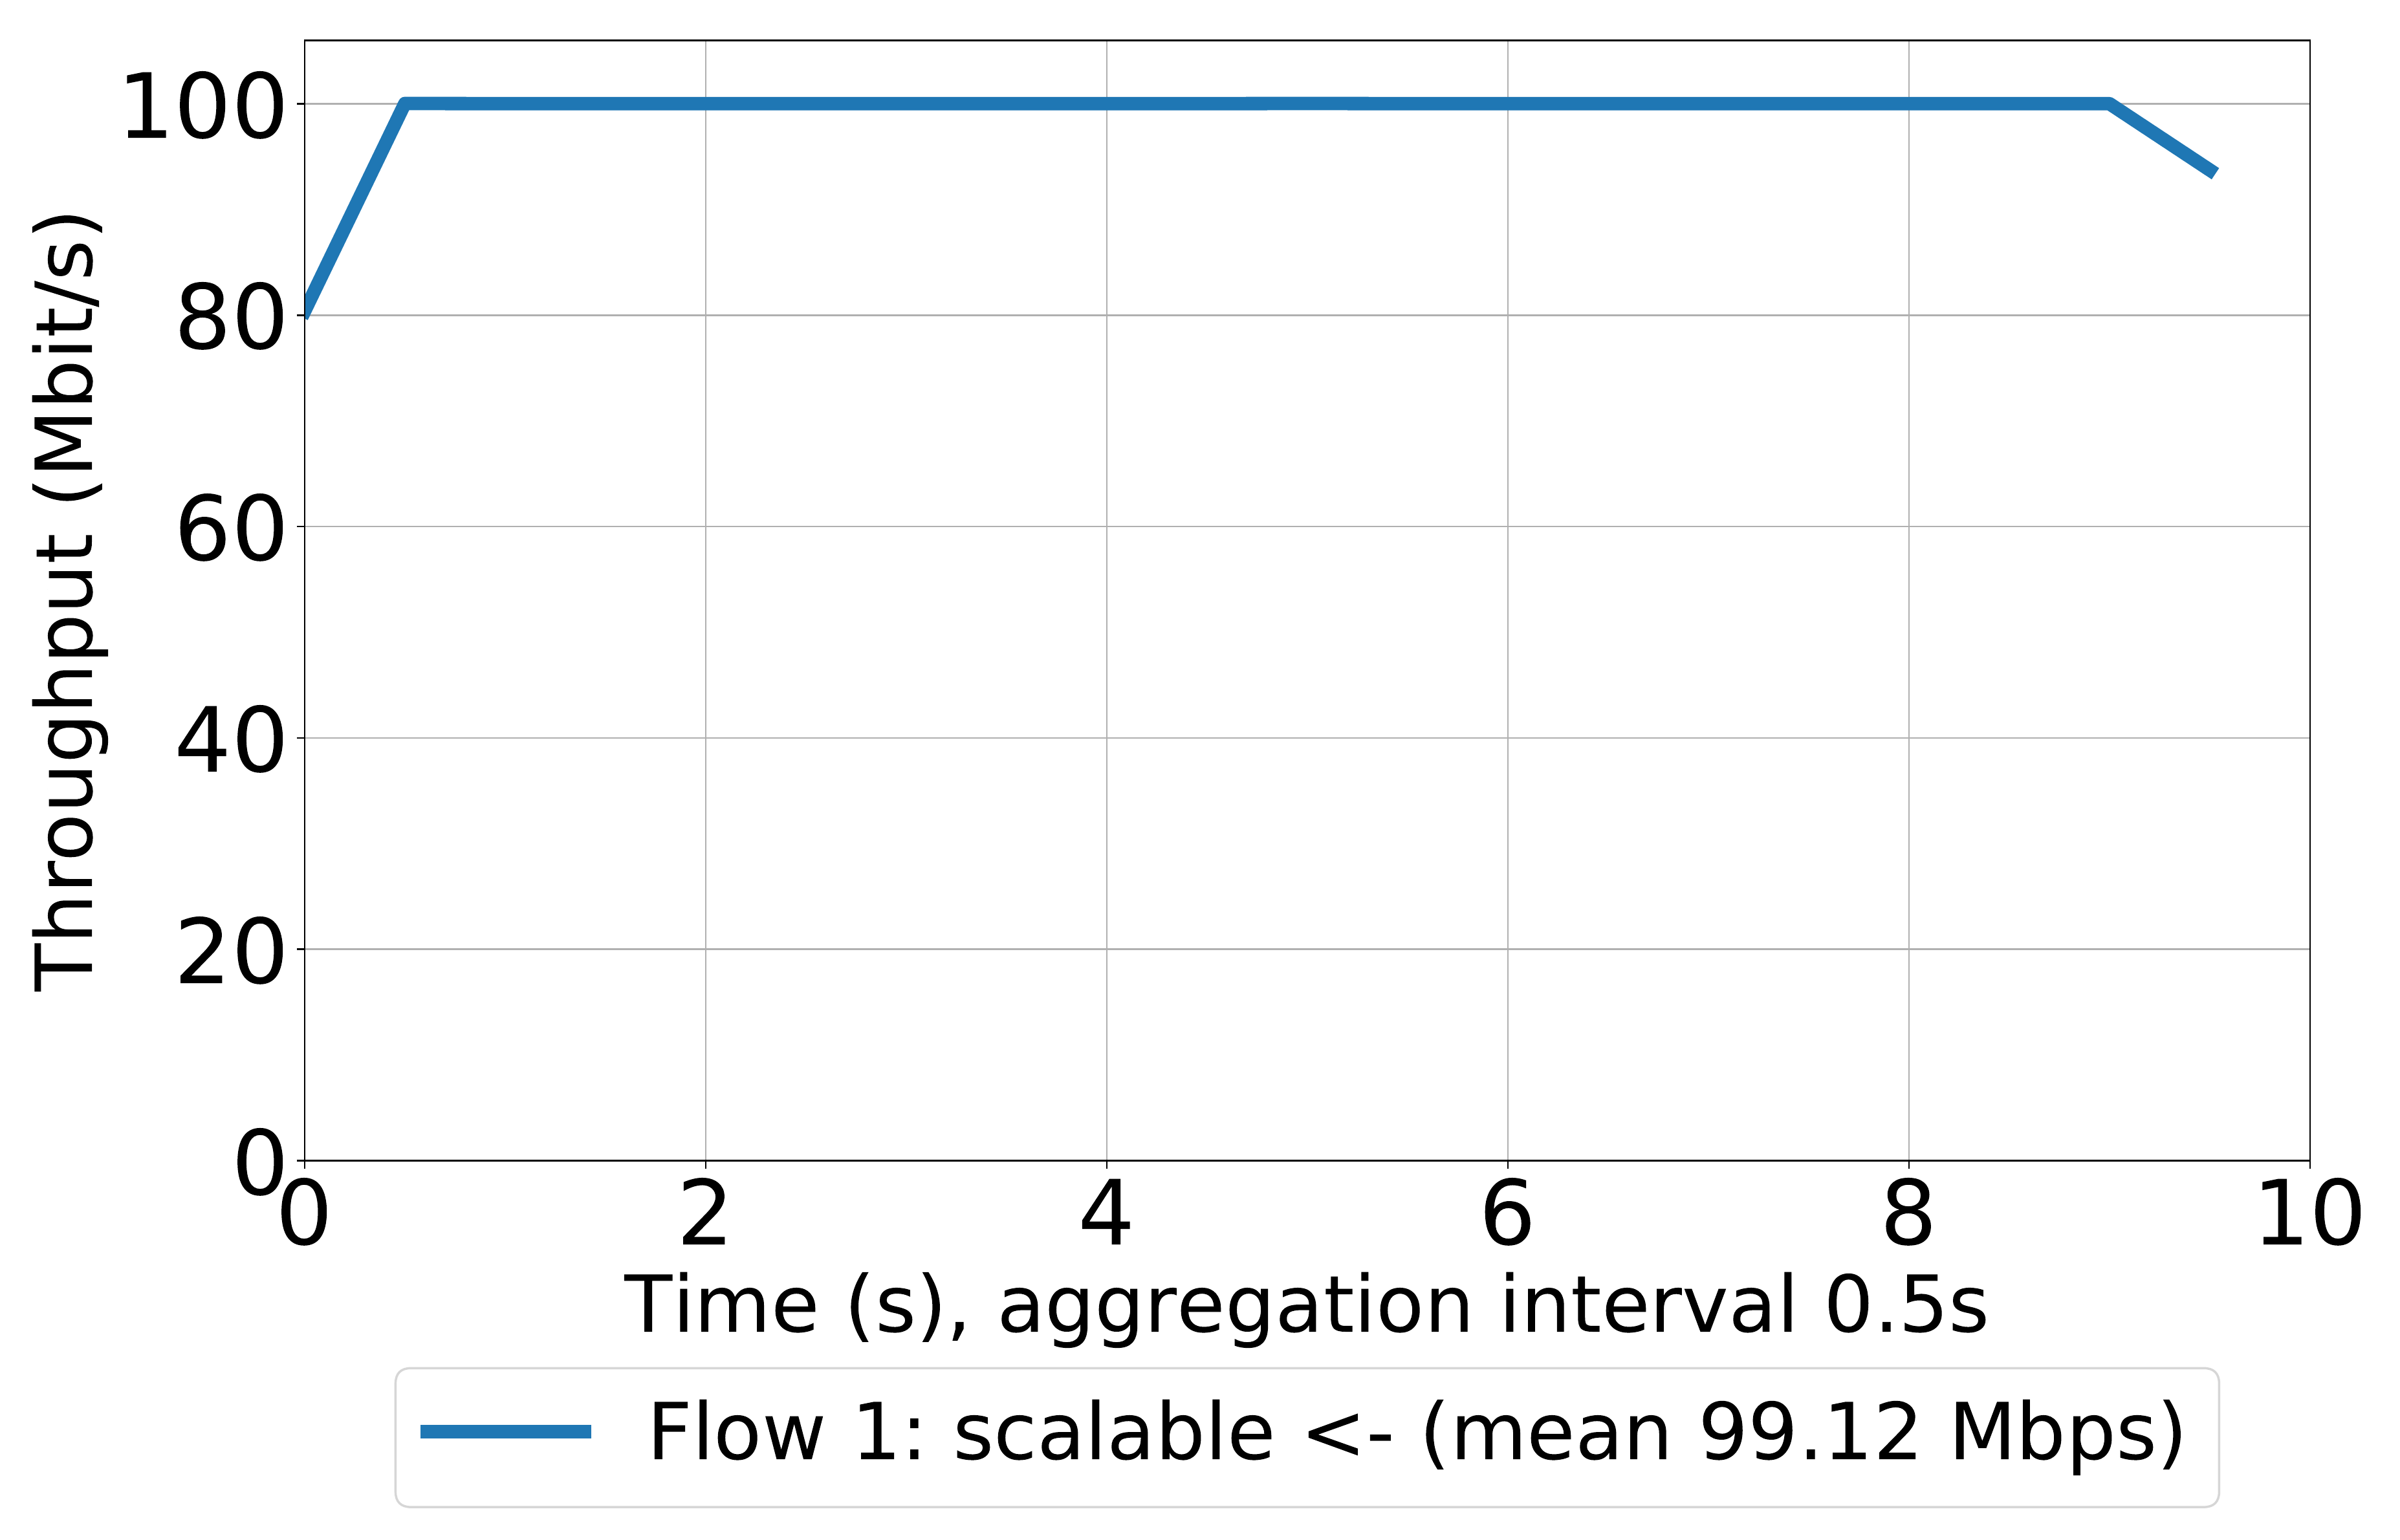} }}%
    \subfloat[Scalable TCP by Pantheon]{{\includegraphics[width=0.5\textwidth]{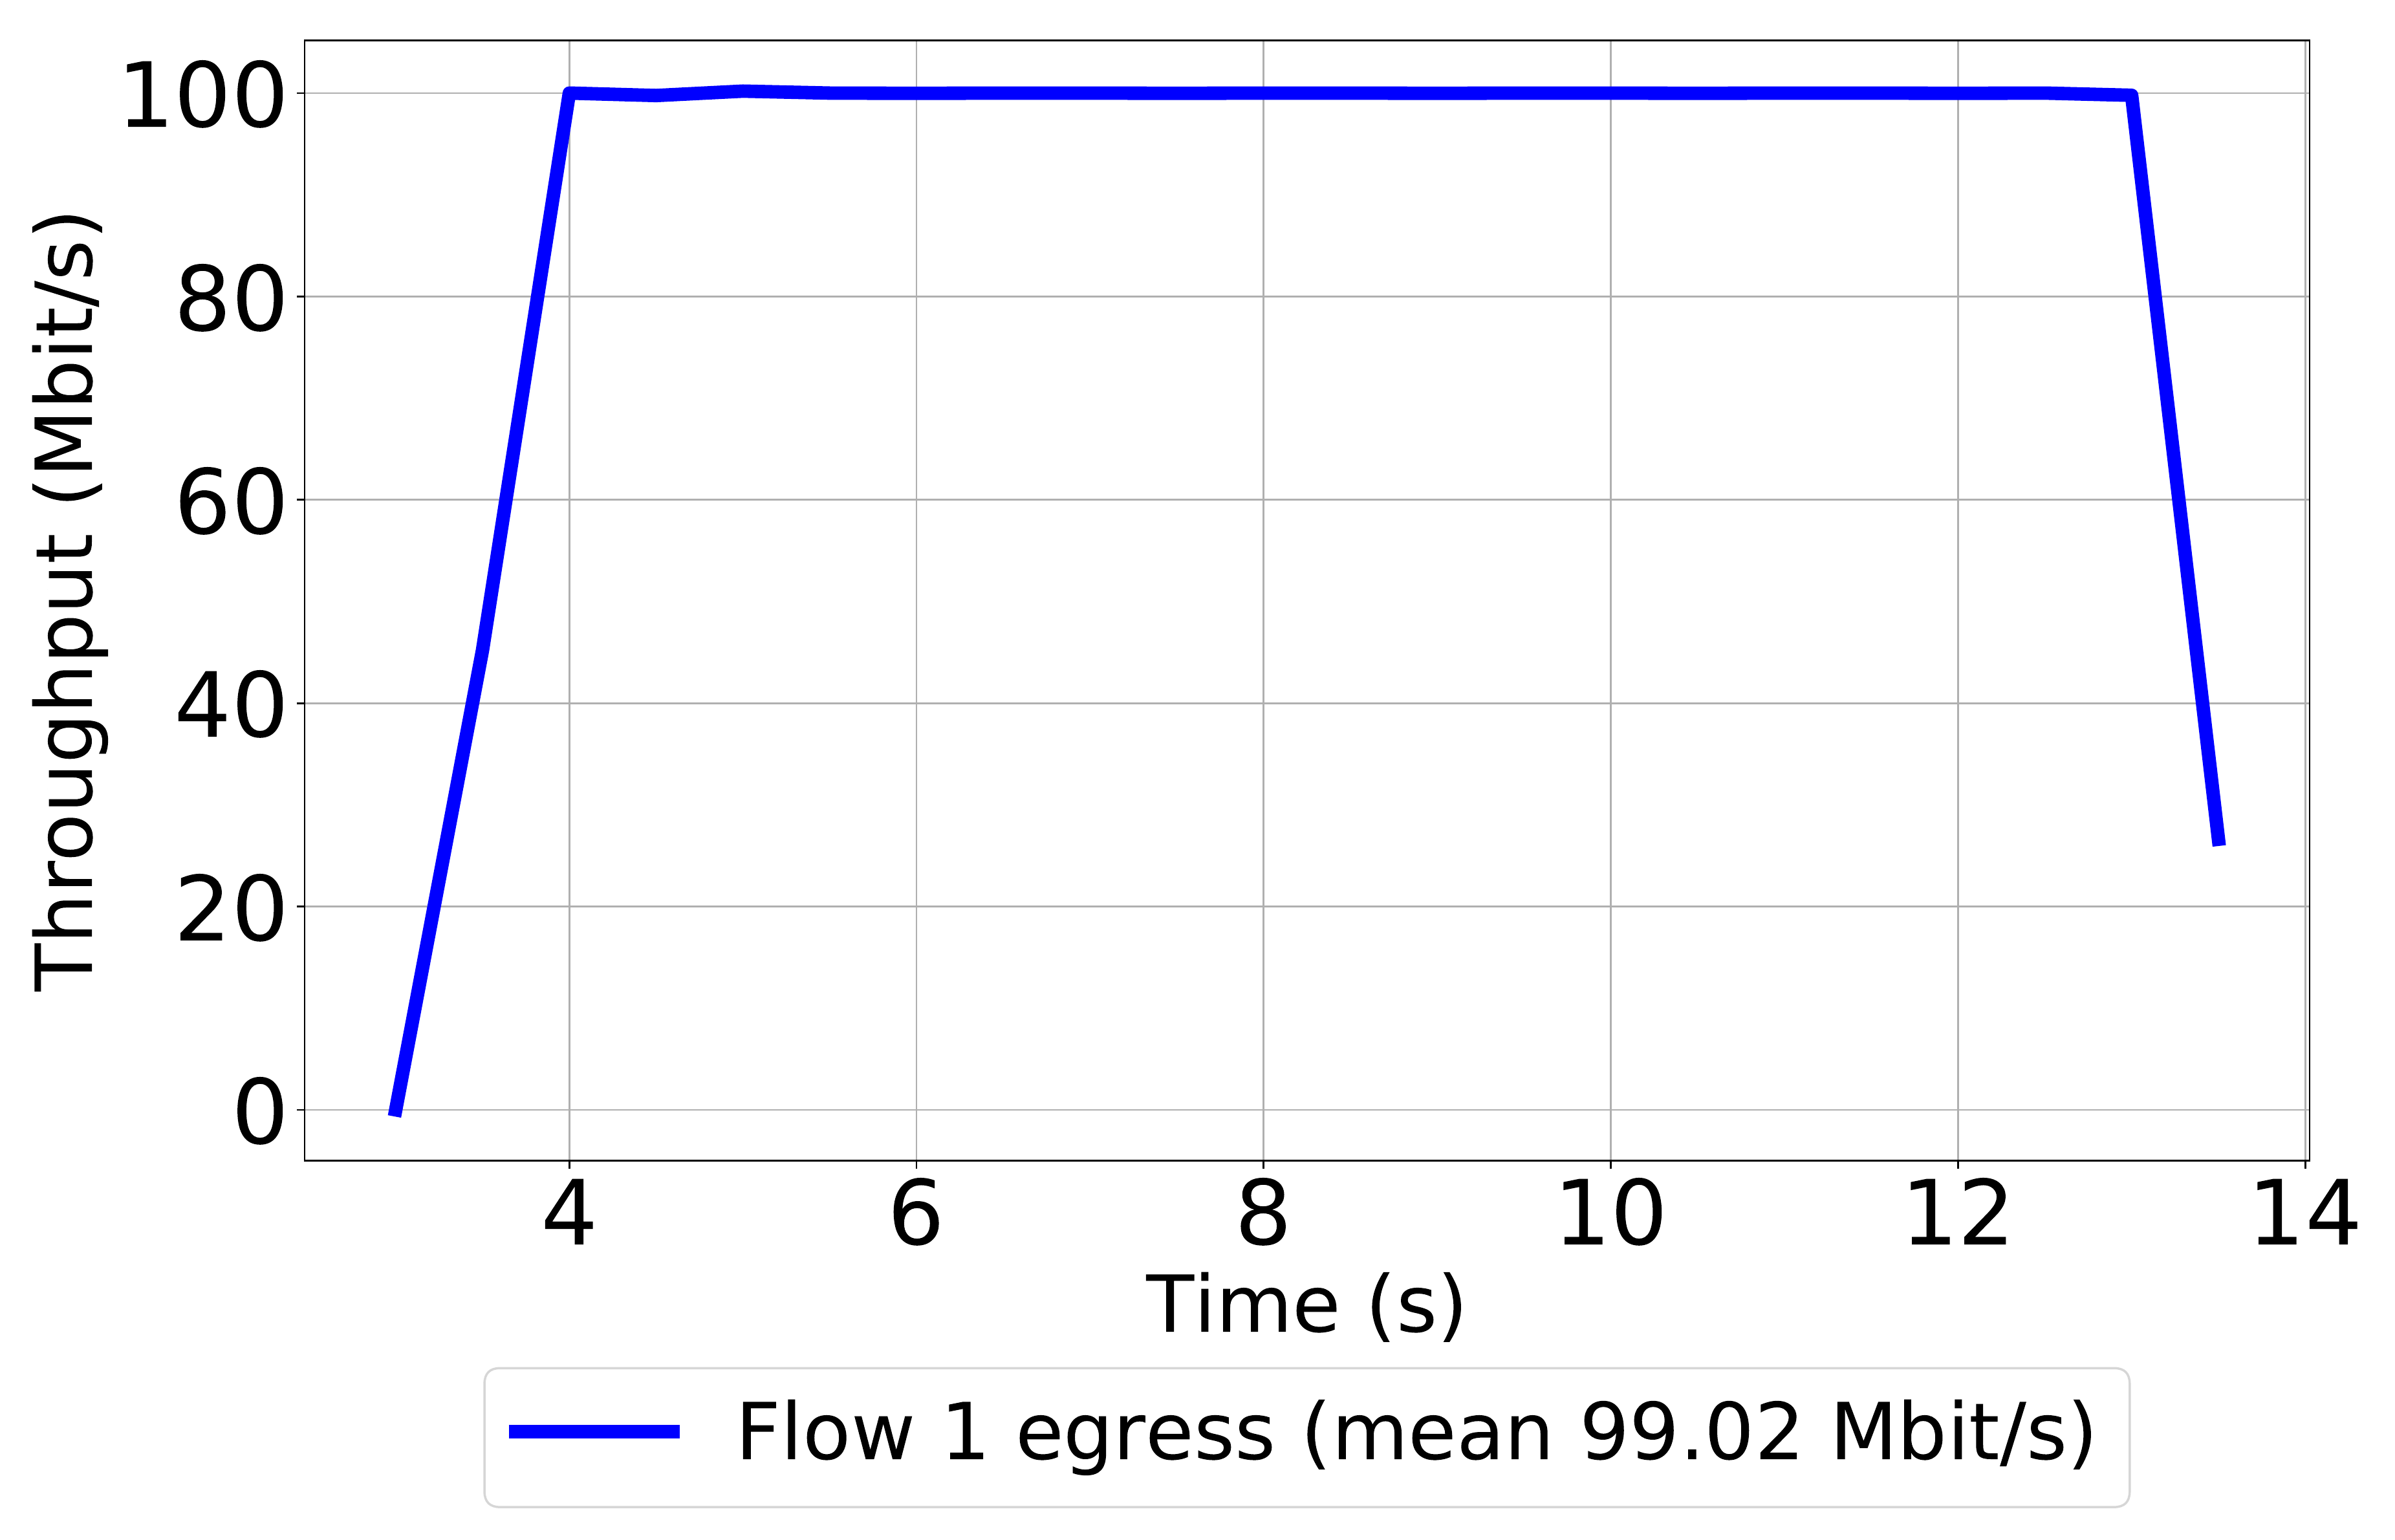} }}\\
    \subfloat[Sprout by CoCo-Beholder]{{\includegraphics[width=0.5\textwidth]{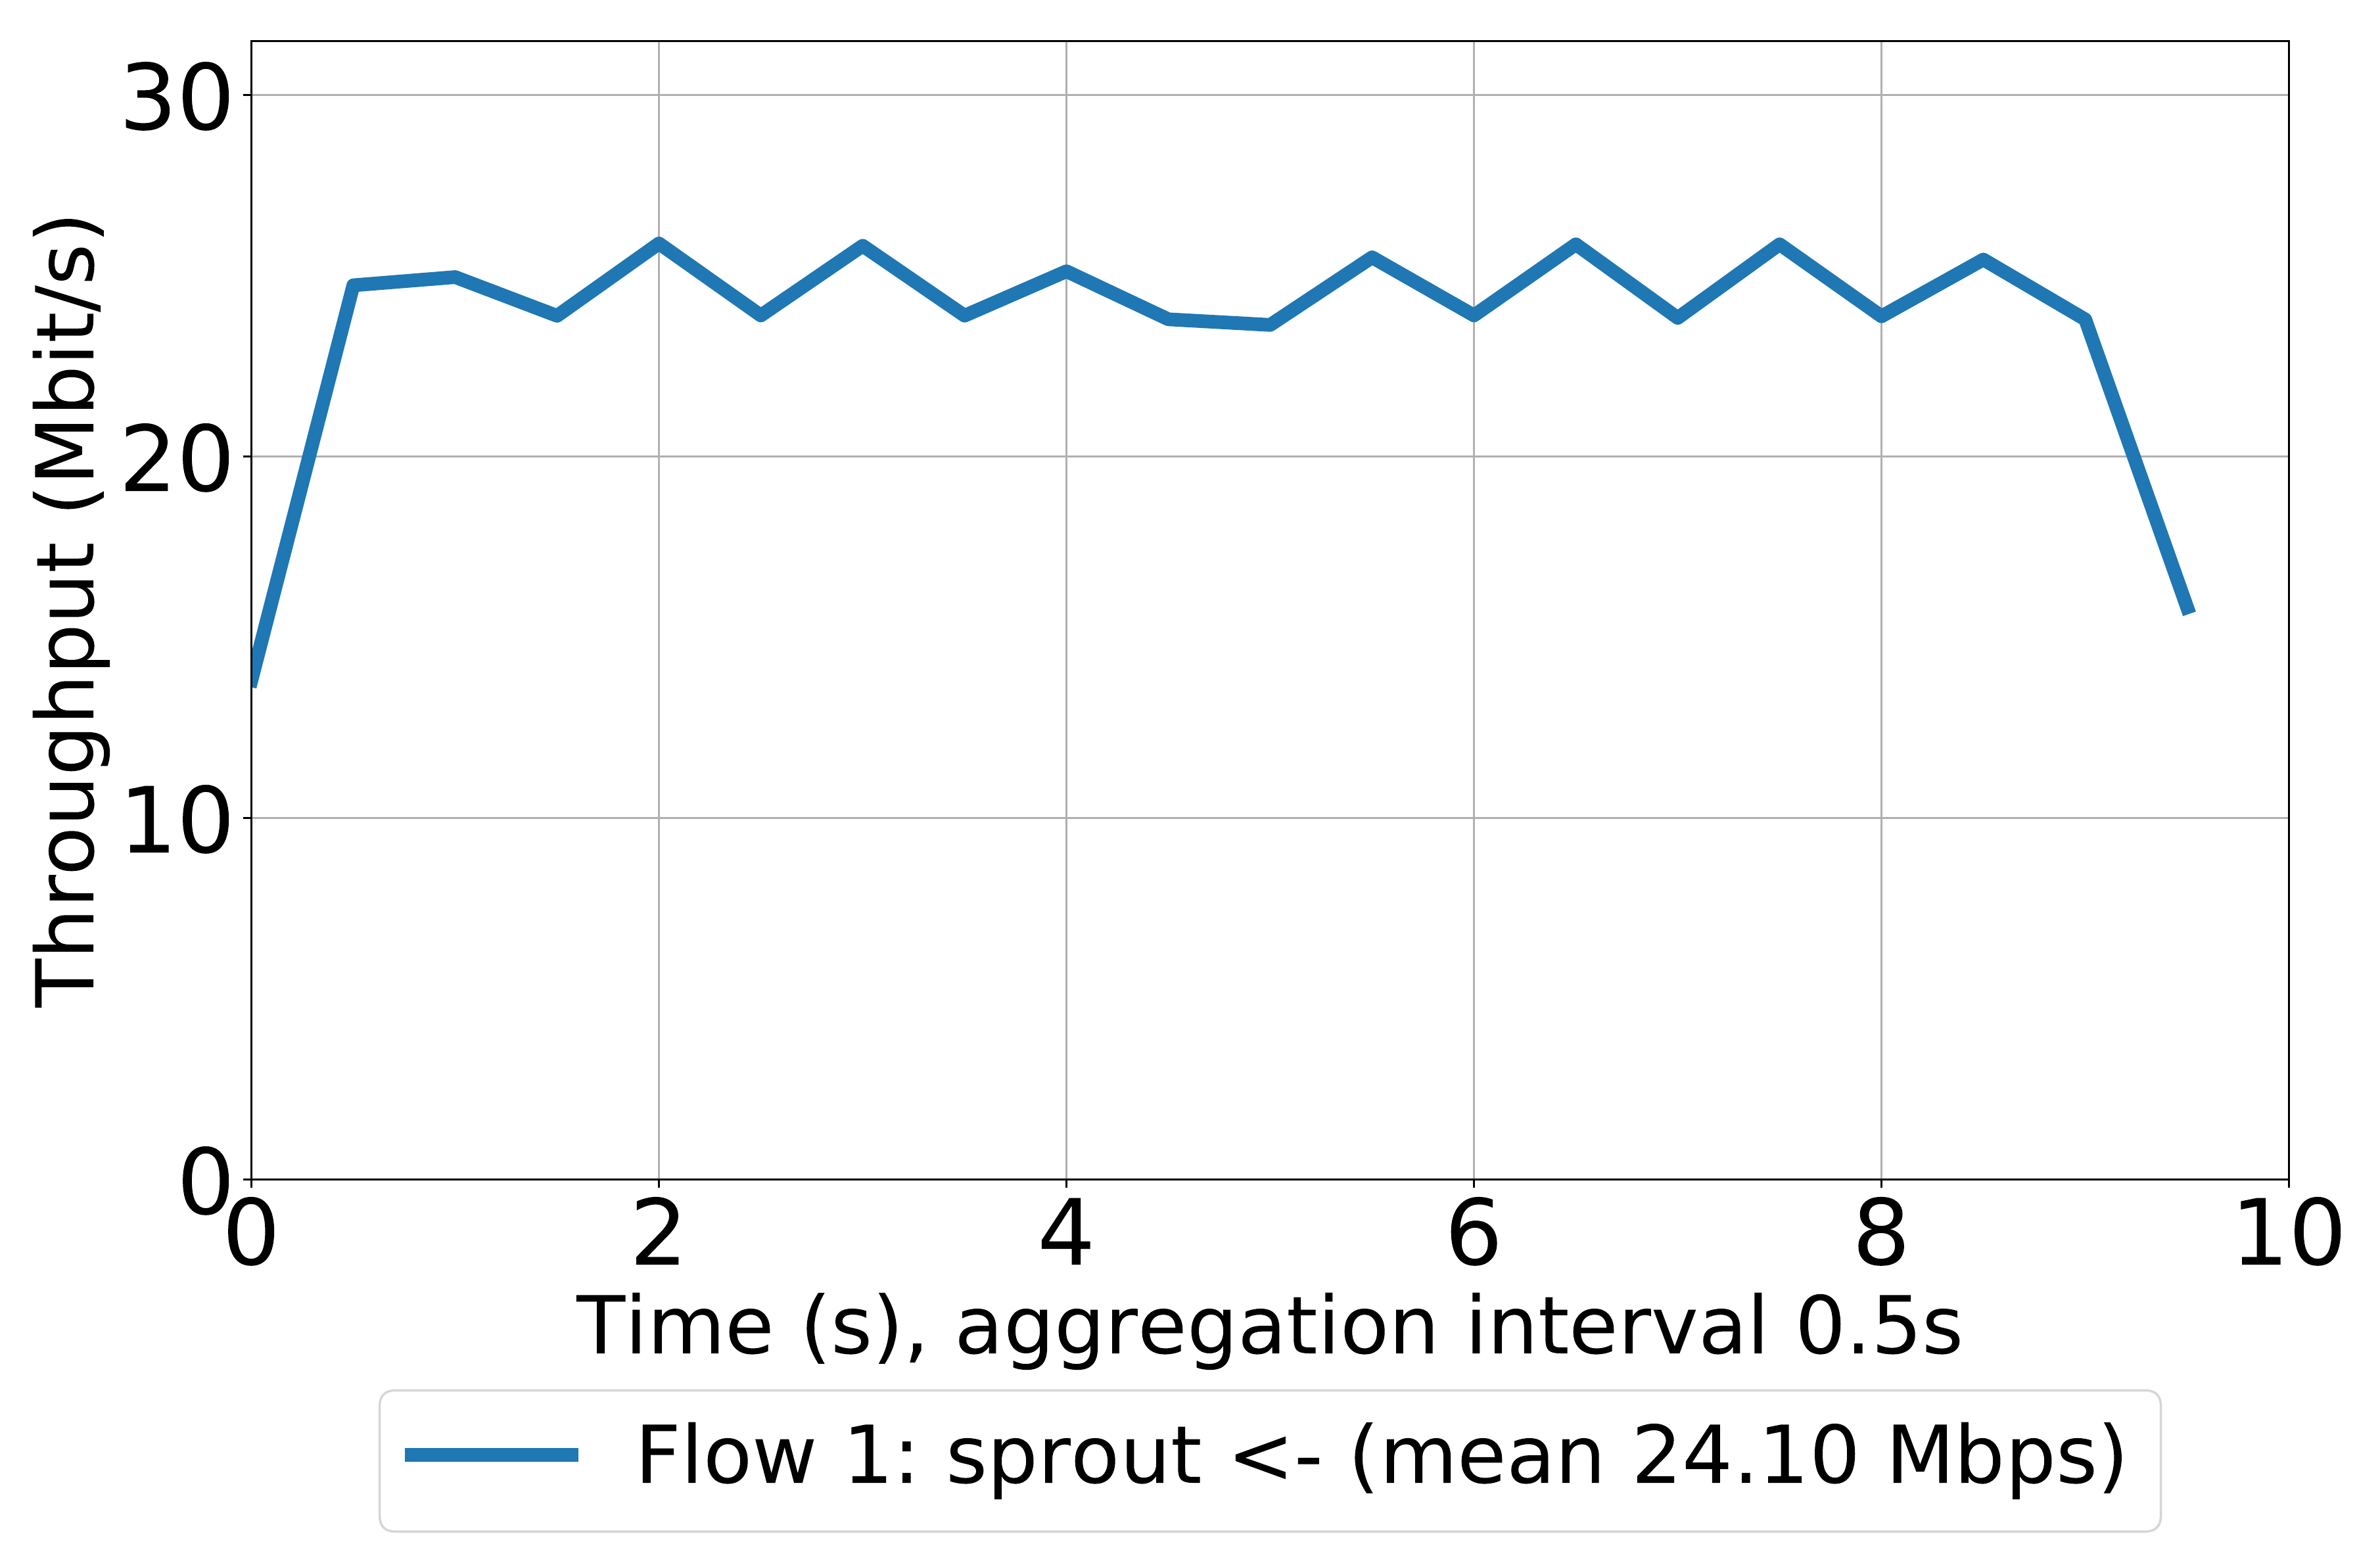} }}%
    \subfloat[Sprout by Pantheon]{{\includegraphics[width=0.5\textwidth]{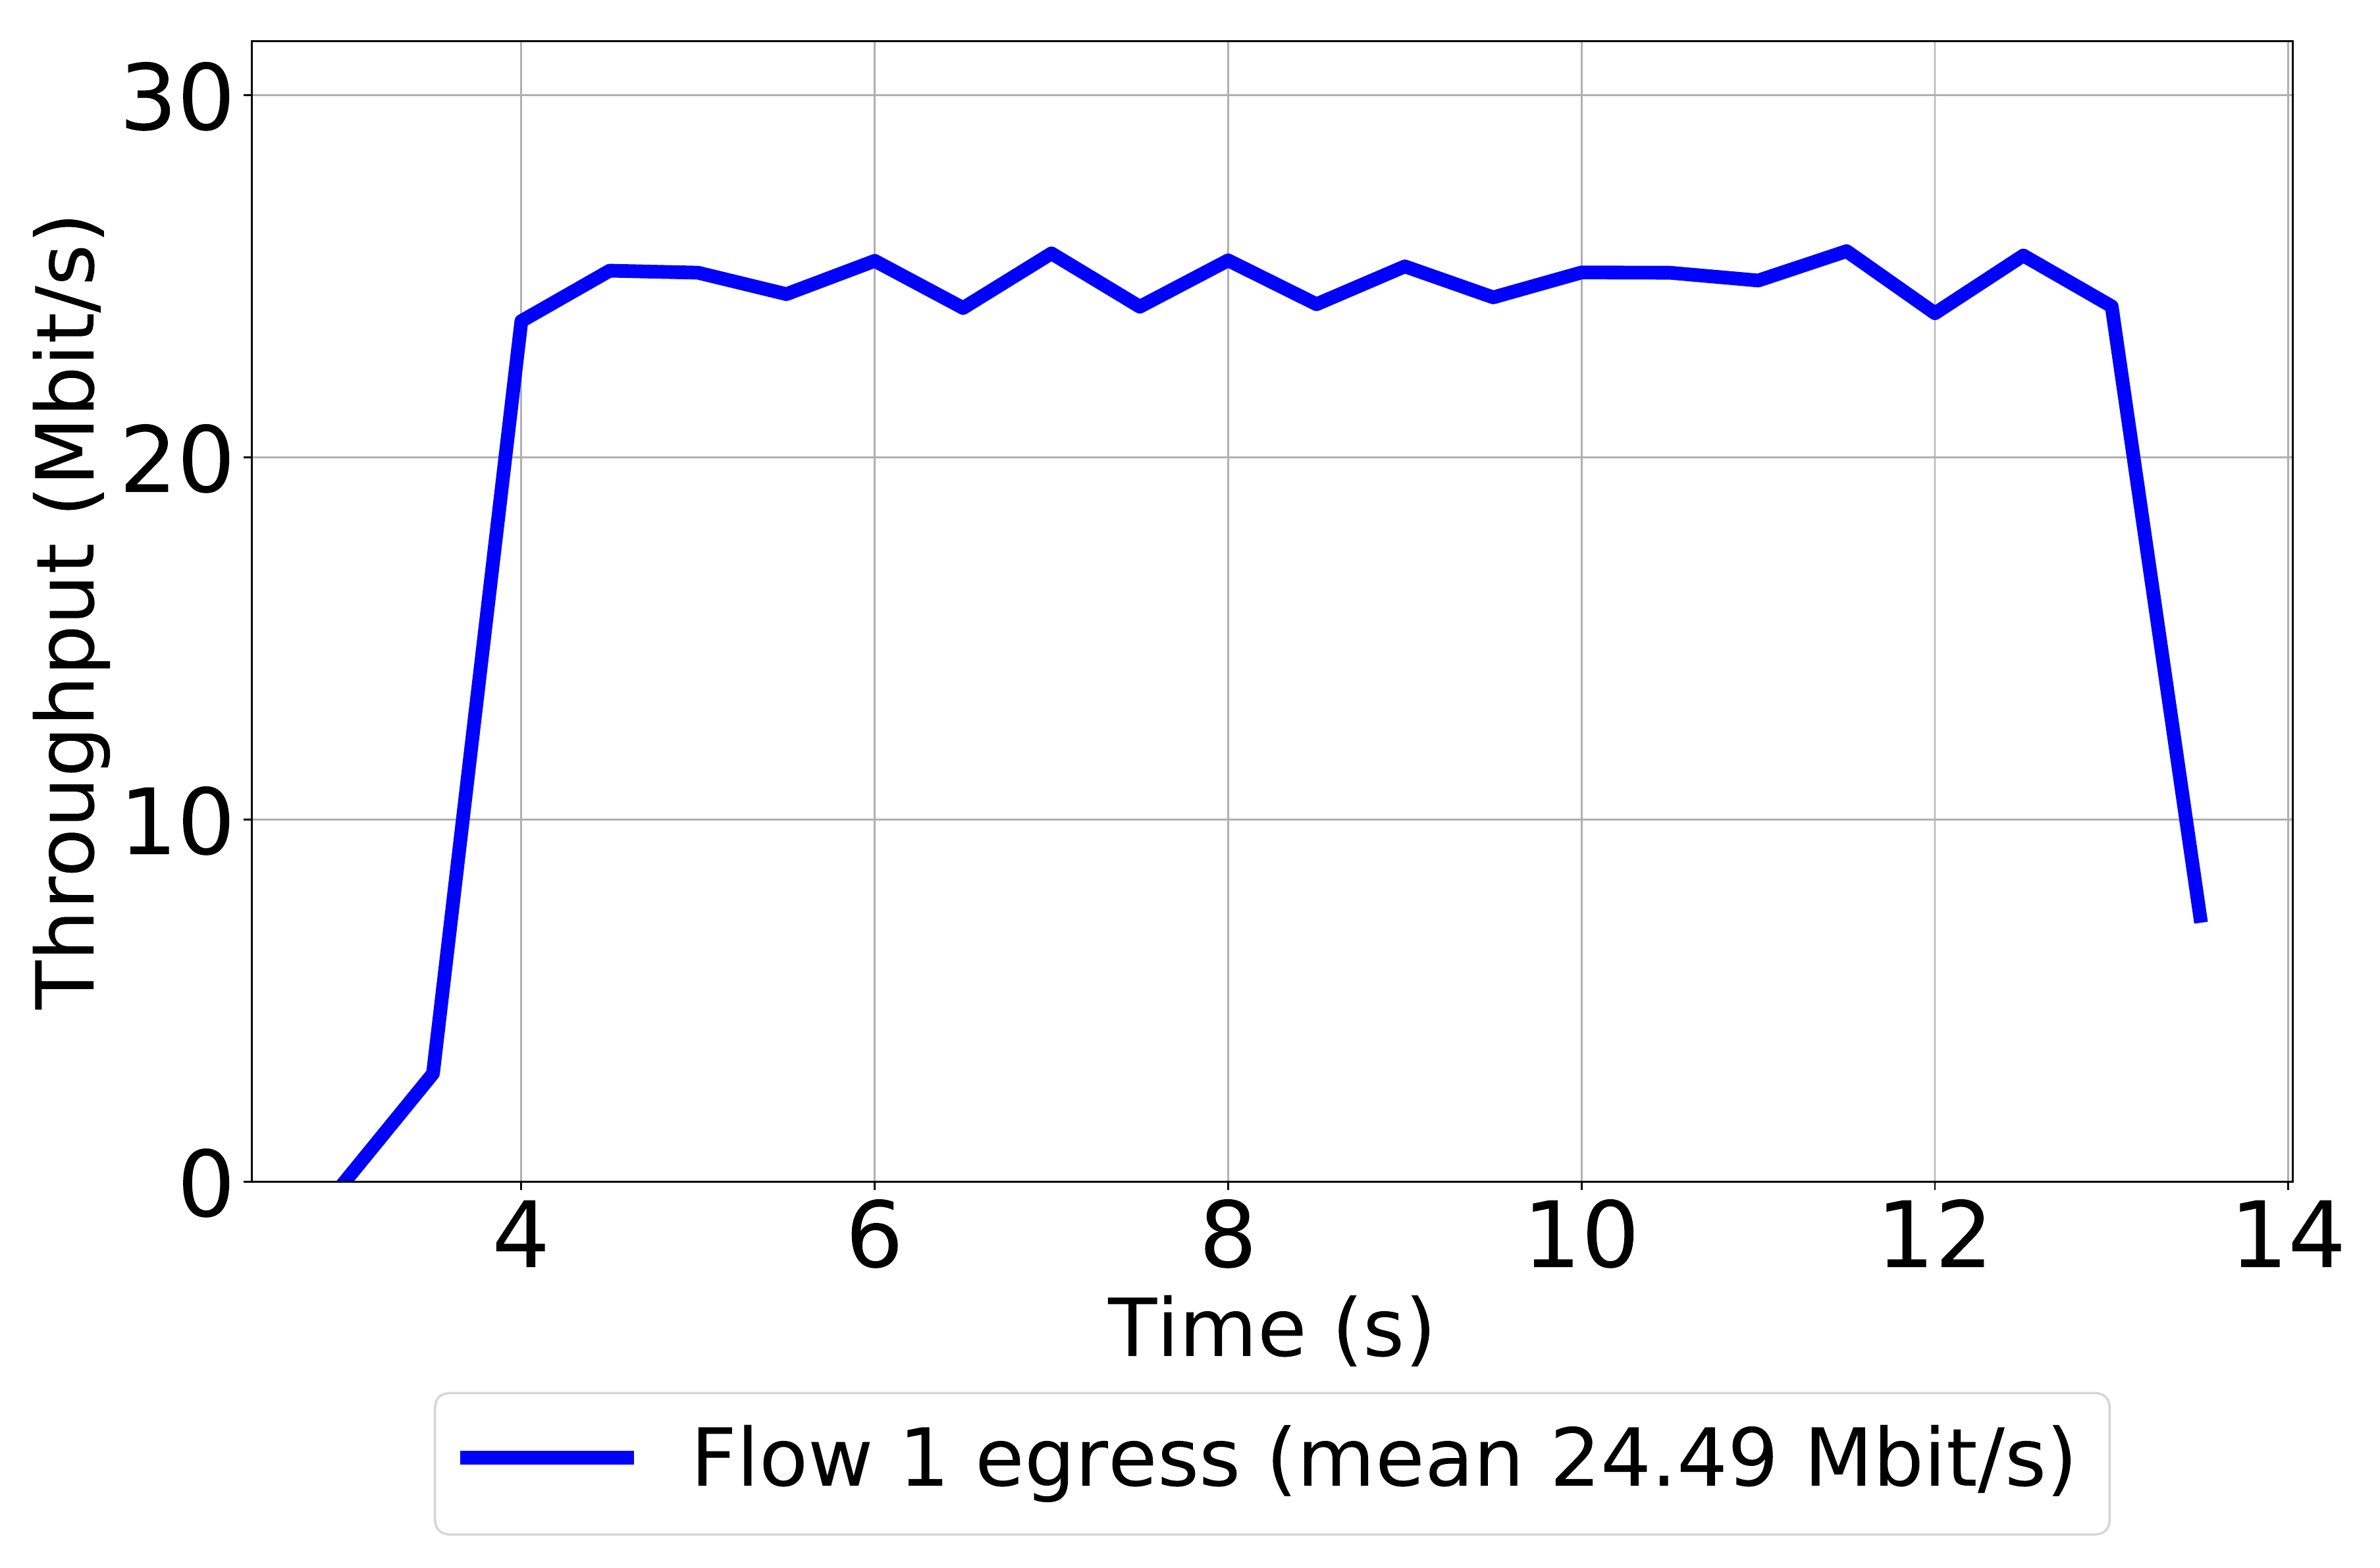} }}%
    \caption{Example average throughput plots, the delay $X=10$ ms.}%
    \label{fig:compr}
\end{figure}
