# Supplementary material for: The CoCo-Beholder: Enabling Comprehensive Evaluation of Congestion Control Algorithms
Source: arXiv:1912.10531 source file (2019-12-22)
Supplement: Supplementary file 5 [file AppendixE.tex]

The appendix provides the results for Cubic run by CoCo-Beholder for ten seconds in the topology of Figure~\ref{fig:vd-dumbbell} under the square-wave variable delay with the base delay\nolinebreak[4] \mbox{0 ms}, the delta 150 ms, and the step in [140, 150, 160] ms.

Section~\ref{sec:tthird} can be consulted for more details on the testing setup. 

Figures \ref{fig:vd-cubic-rate}, \ref{fig:vd-cubic-avgdelay}, \ref{fig:vd-cubic-pptdelay}, \ref{fig:vd-cubic-rtt} on the next pages of the appendix show the average \mbox{throughput}, average one-way delay, per-packet one-way delay, and per-packet RTT  plots for Cubic's data traffic for the steps 140, 150, 160 ms.

All the throughput and delay plots were generated by CoCo-Beholder. The RTT plots were generated using I/O Graph window of Wireshark.

\begin{figure}[h!]
\vspace*{-0.3cm}
\begin{adjustbox}{minipage=\linewidth,totalheight=\textheight}
    \centering
    \subfloat[Step = 140 ms]{{\includegraphics[height=0.3\textheight]{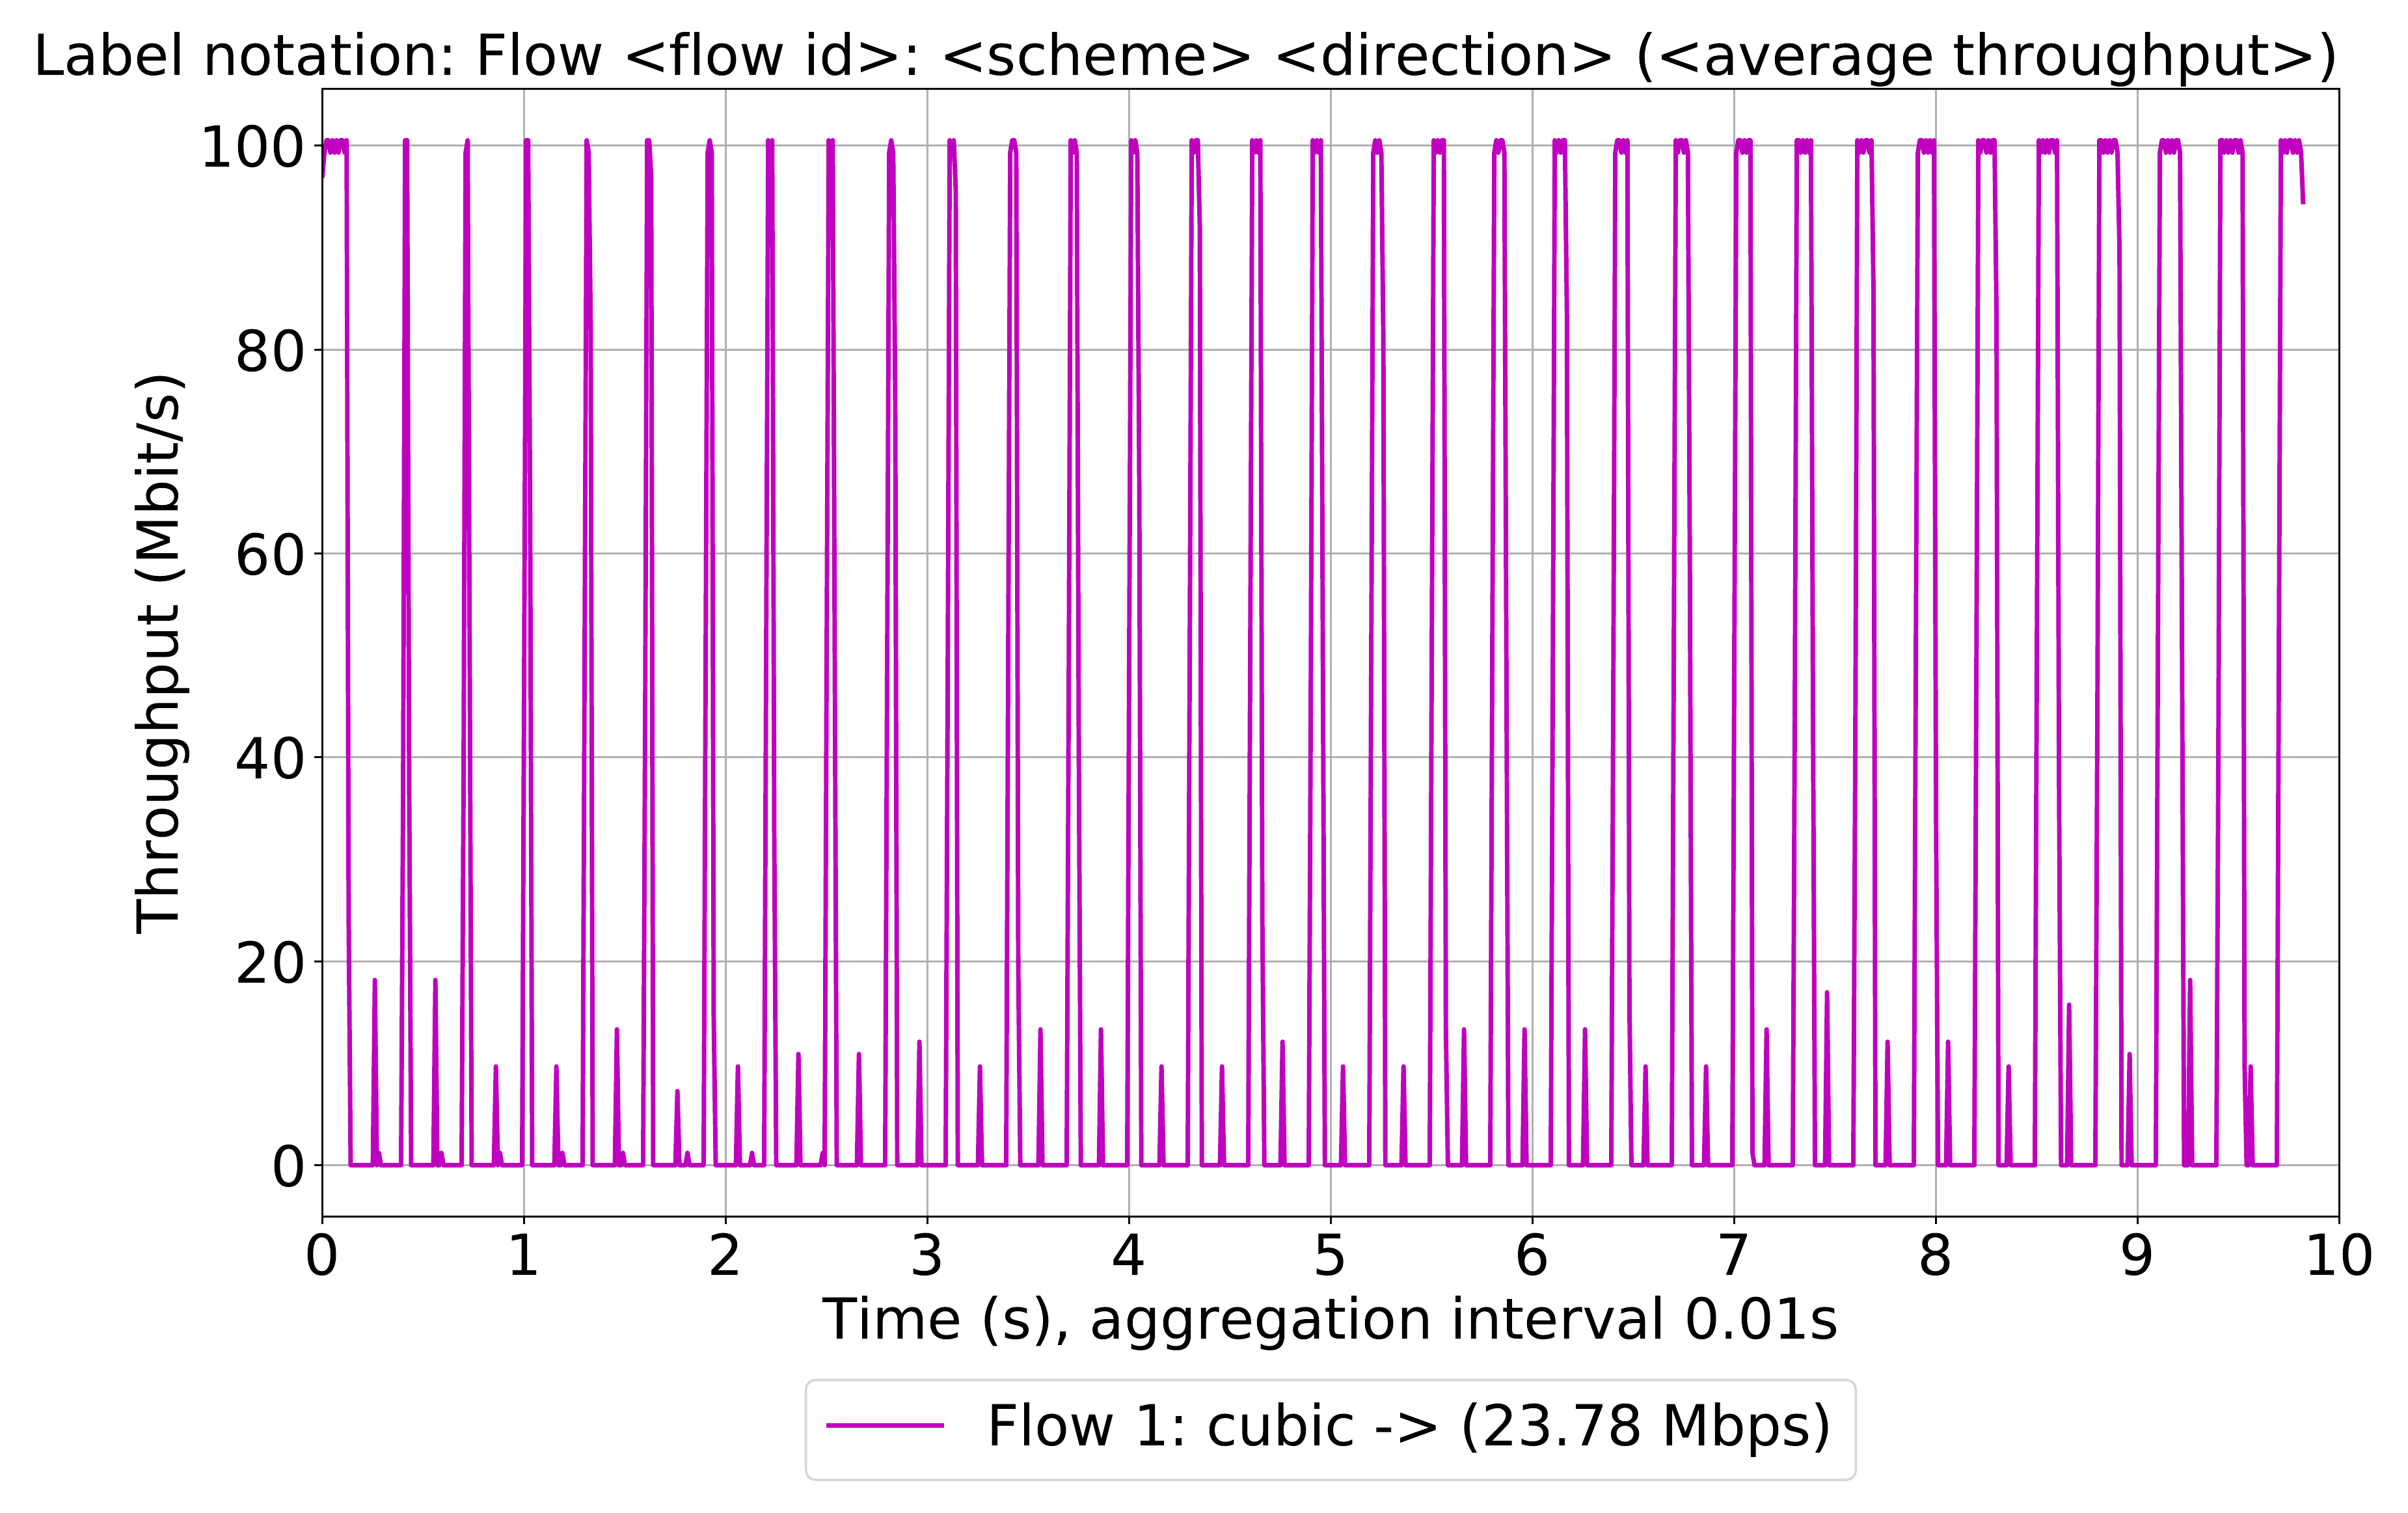} }}\\
    \vspace*{-0.3cm}
    \subfloat[Step = 150 ms]{{\includegraphics[height=0.3\textheight]{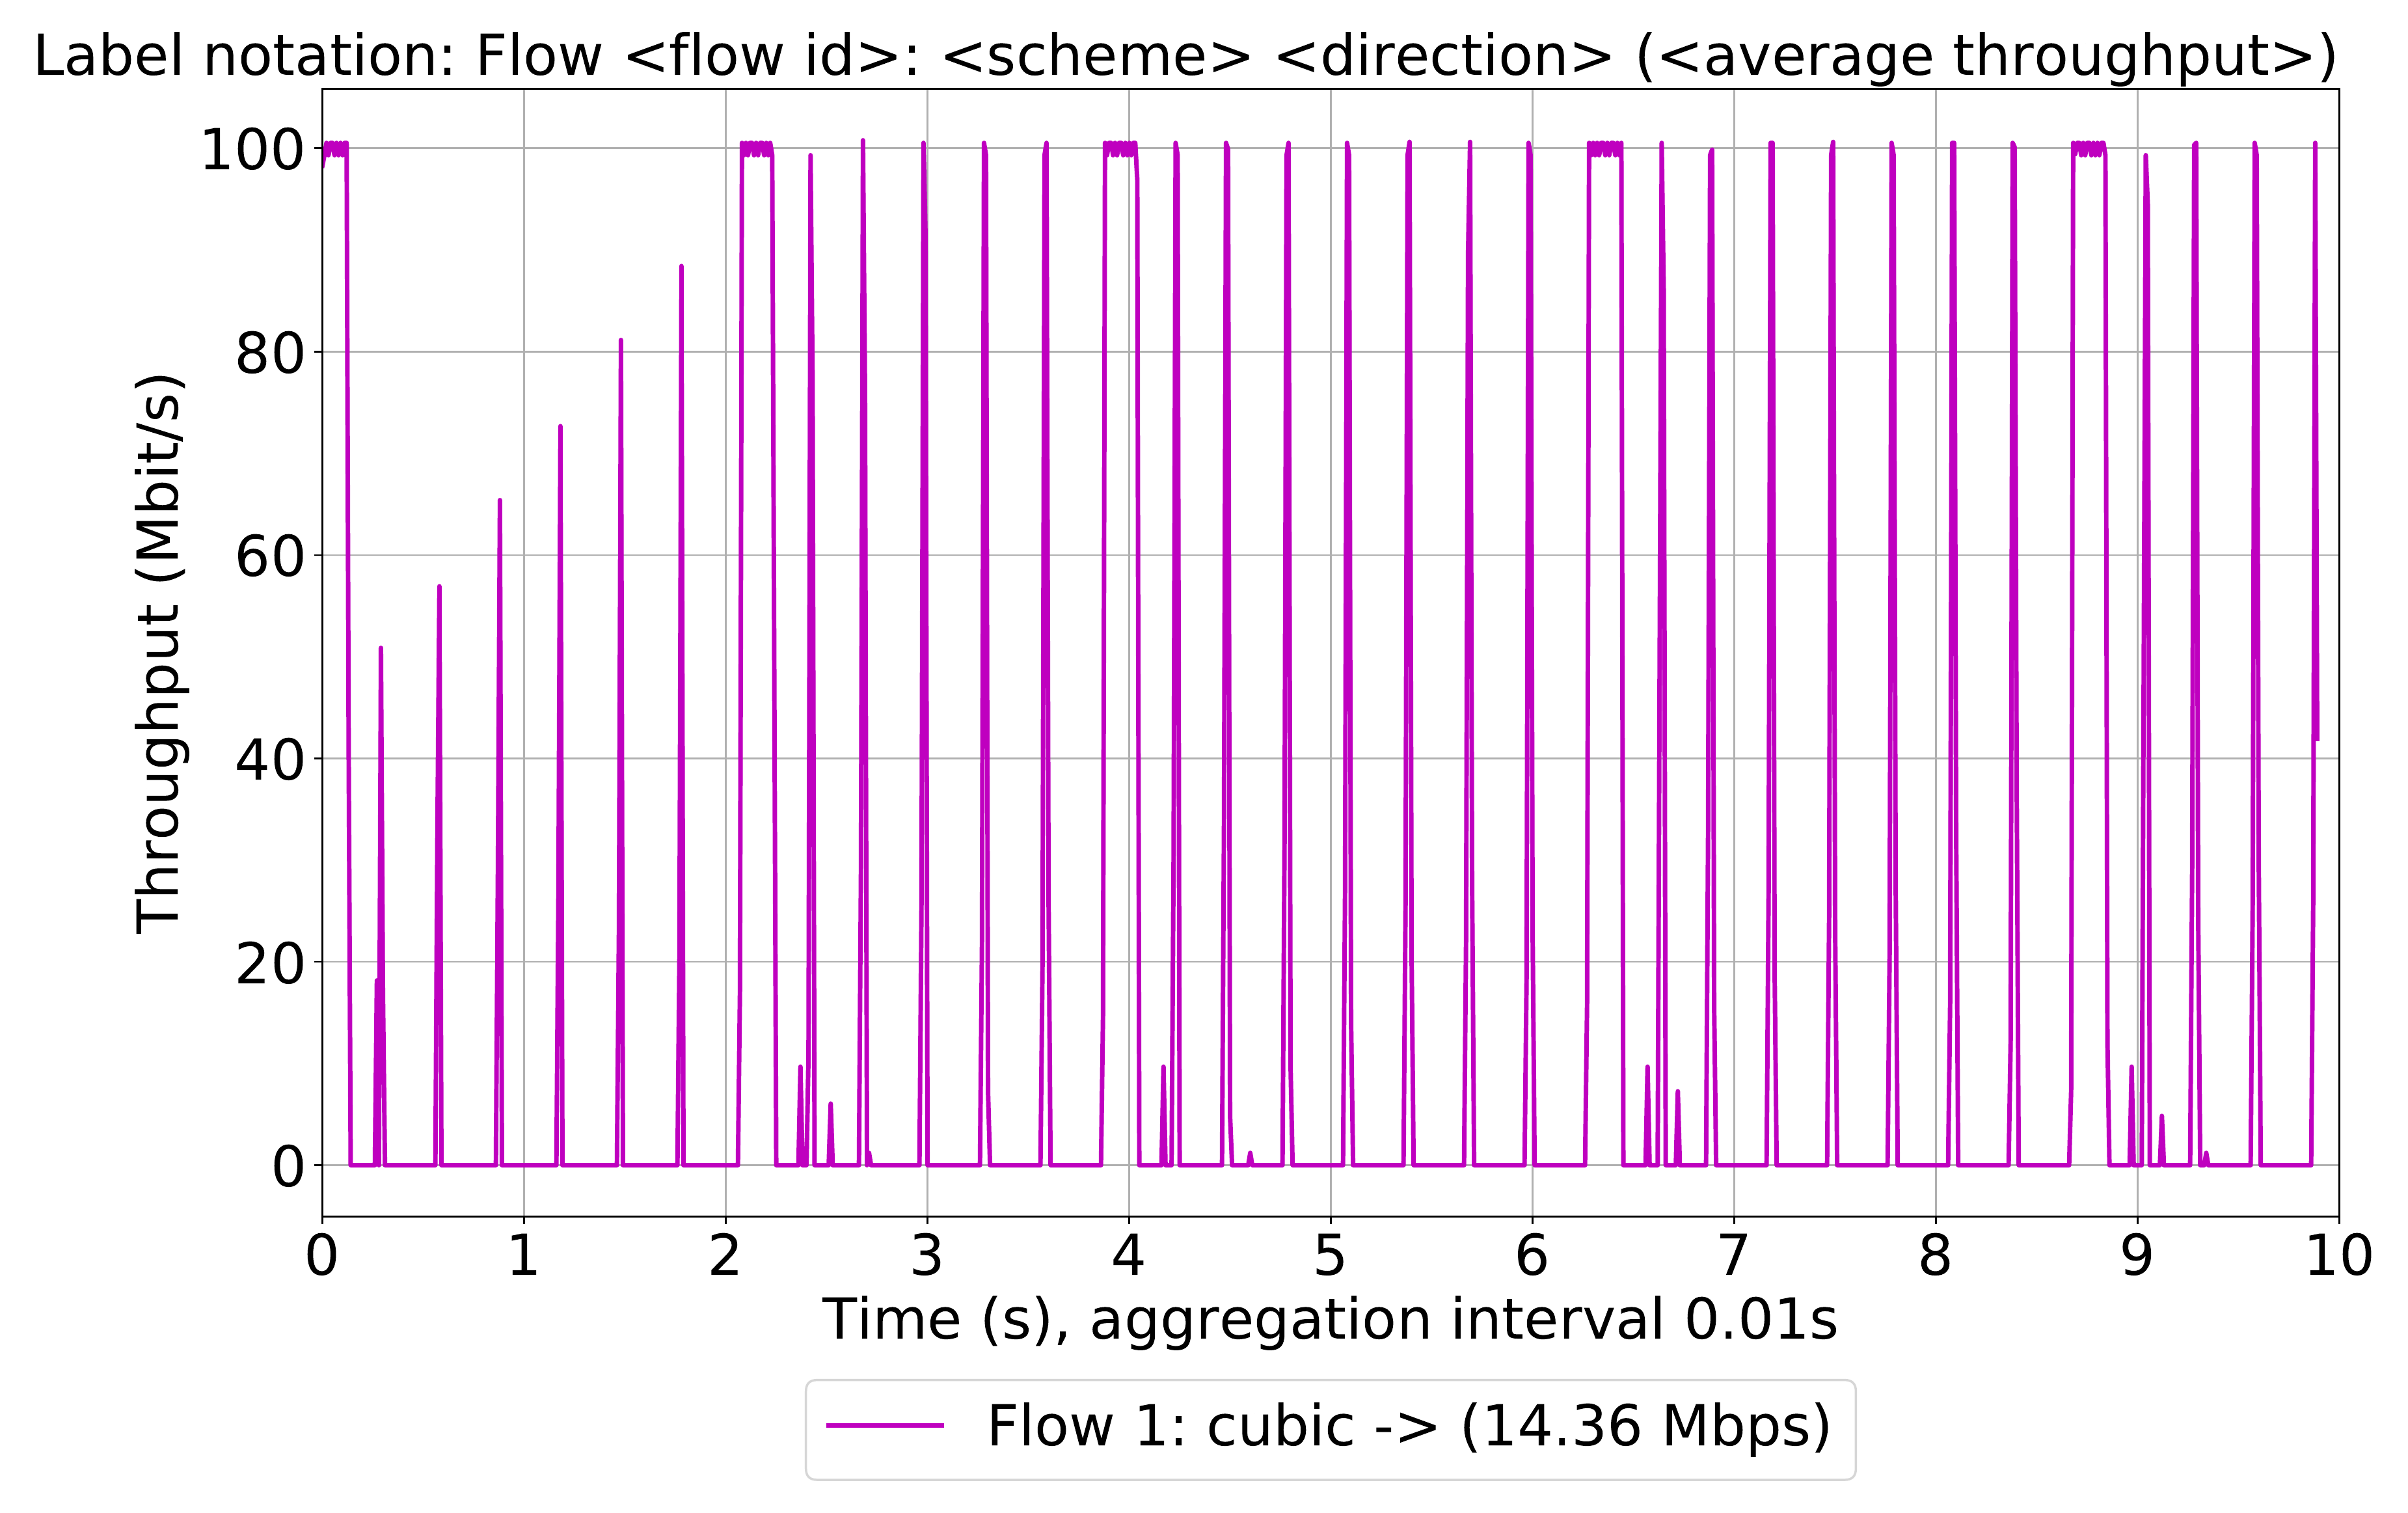} }}\\
    \vspace*{-0.3cm}
    \subfloat[Step = 160 ms]{{\includegraphics[height=0.3\textheight]{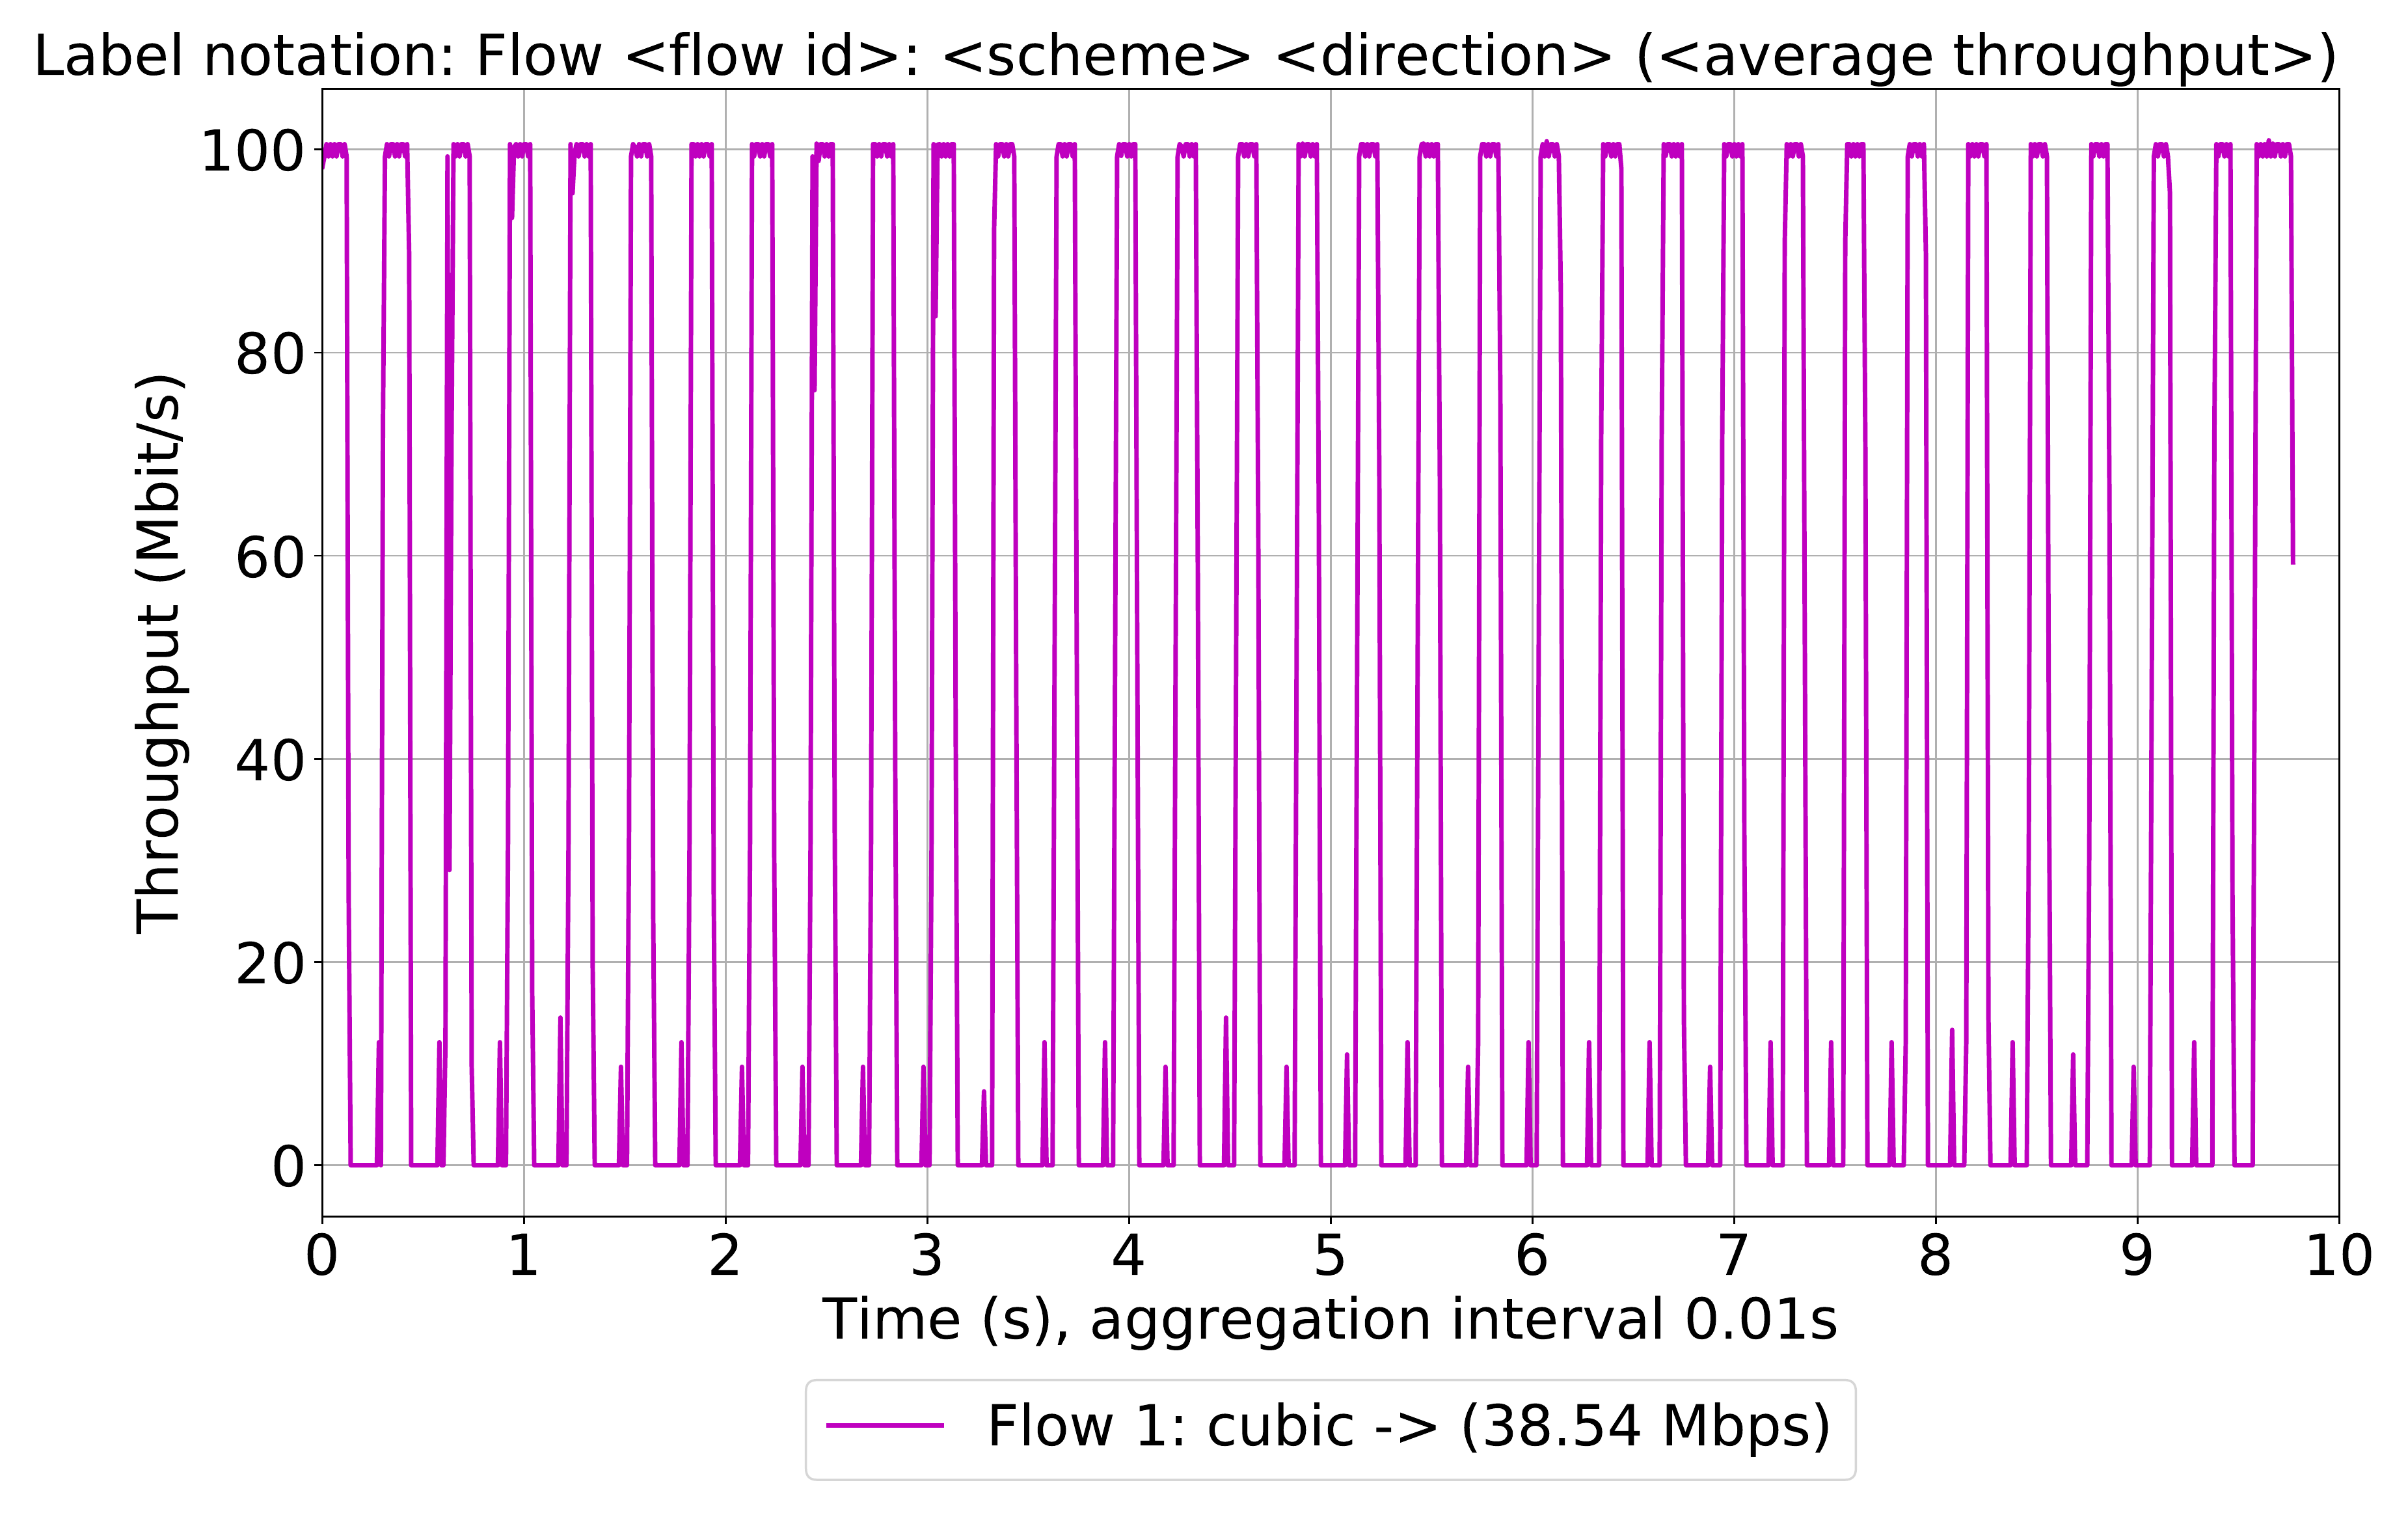} }}%
    \vspace*{-0.1cm}
    \caption{Cubic's average throughput plots for the delta 150 ms.}%
    \label{fig:vd-cubic-rate}
\end{adjustbox}
\end{figure}

\FloatBarrier

\begin{figure}[h!]
\vspace*{-0.3cm}
\begin{adjustbox}{minipage=\linewidth,totalheight=\textheight}
    \centering
    \subfloat[Step = 140 ms]{{\includegraphics[height=0.3\textheight]{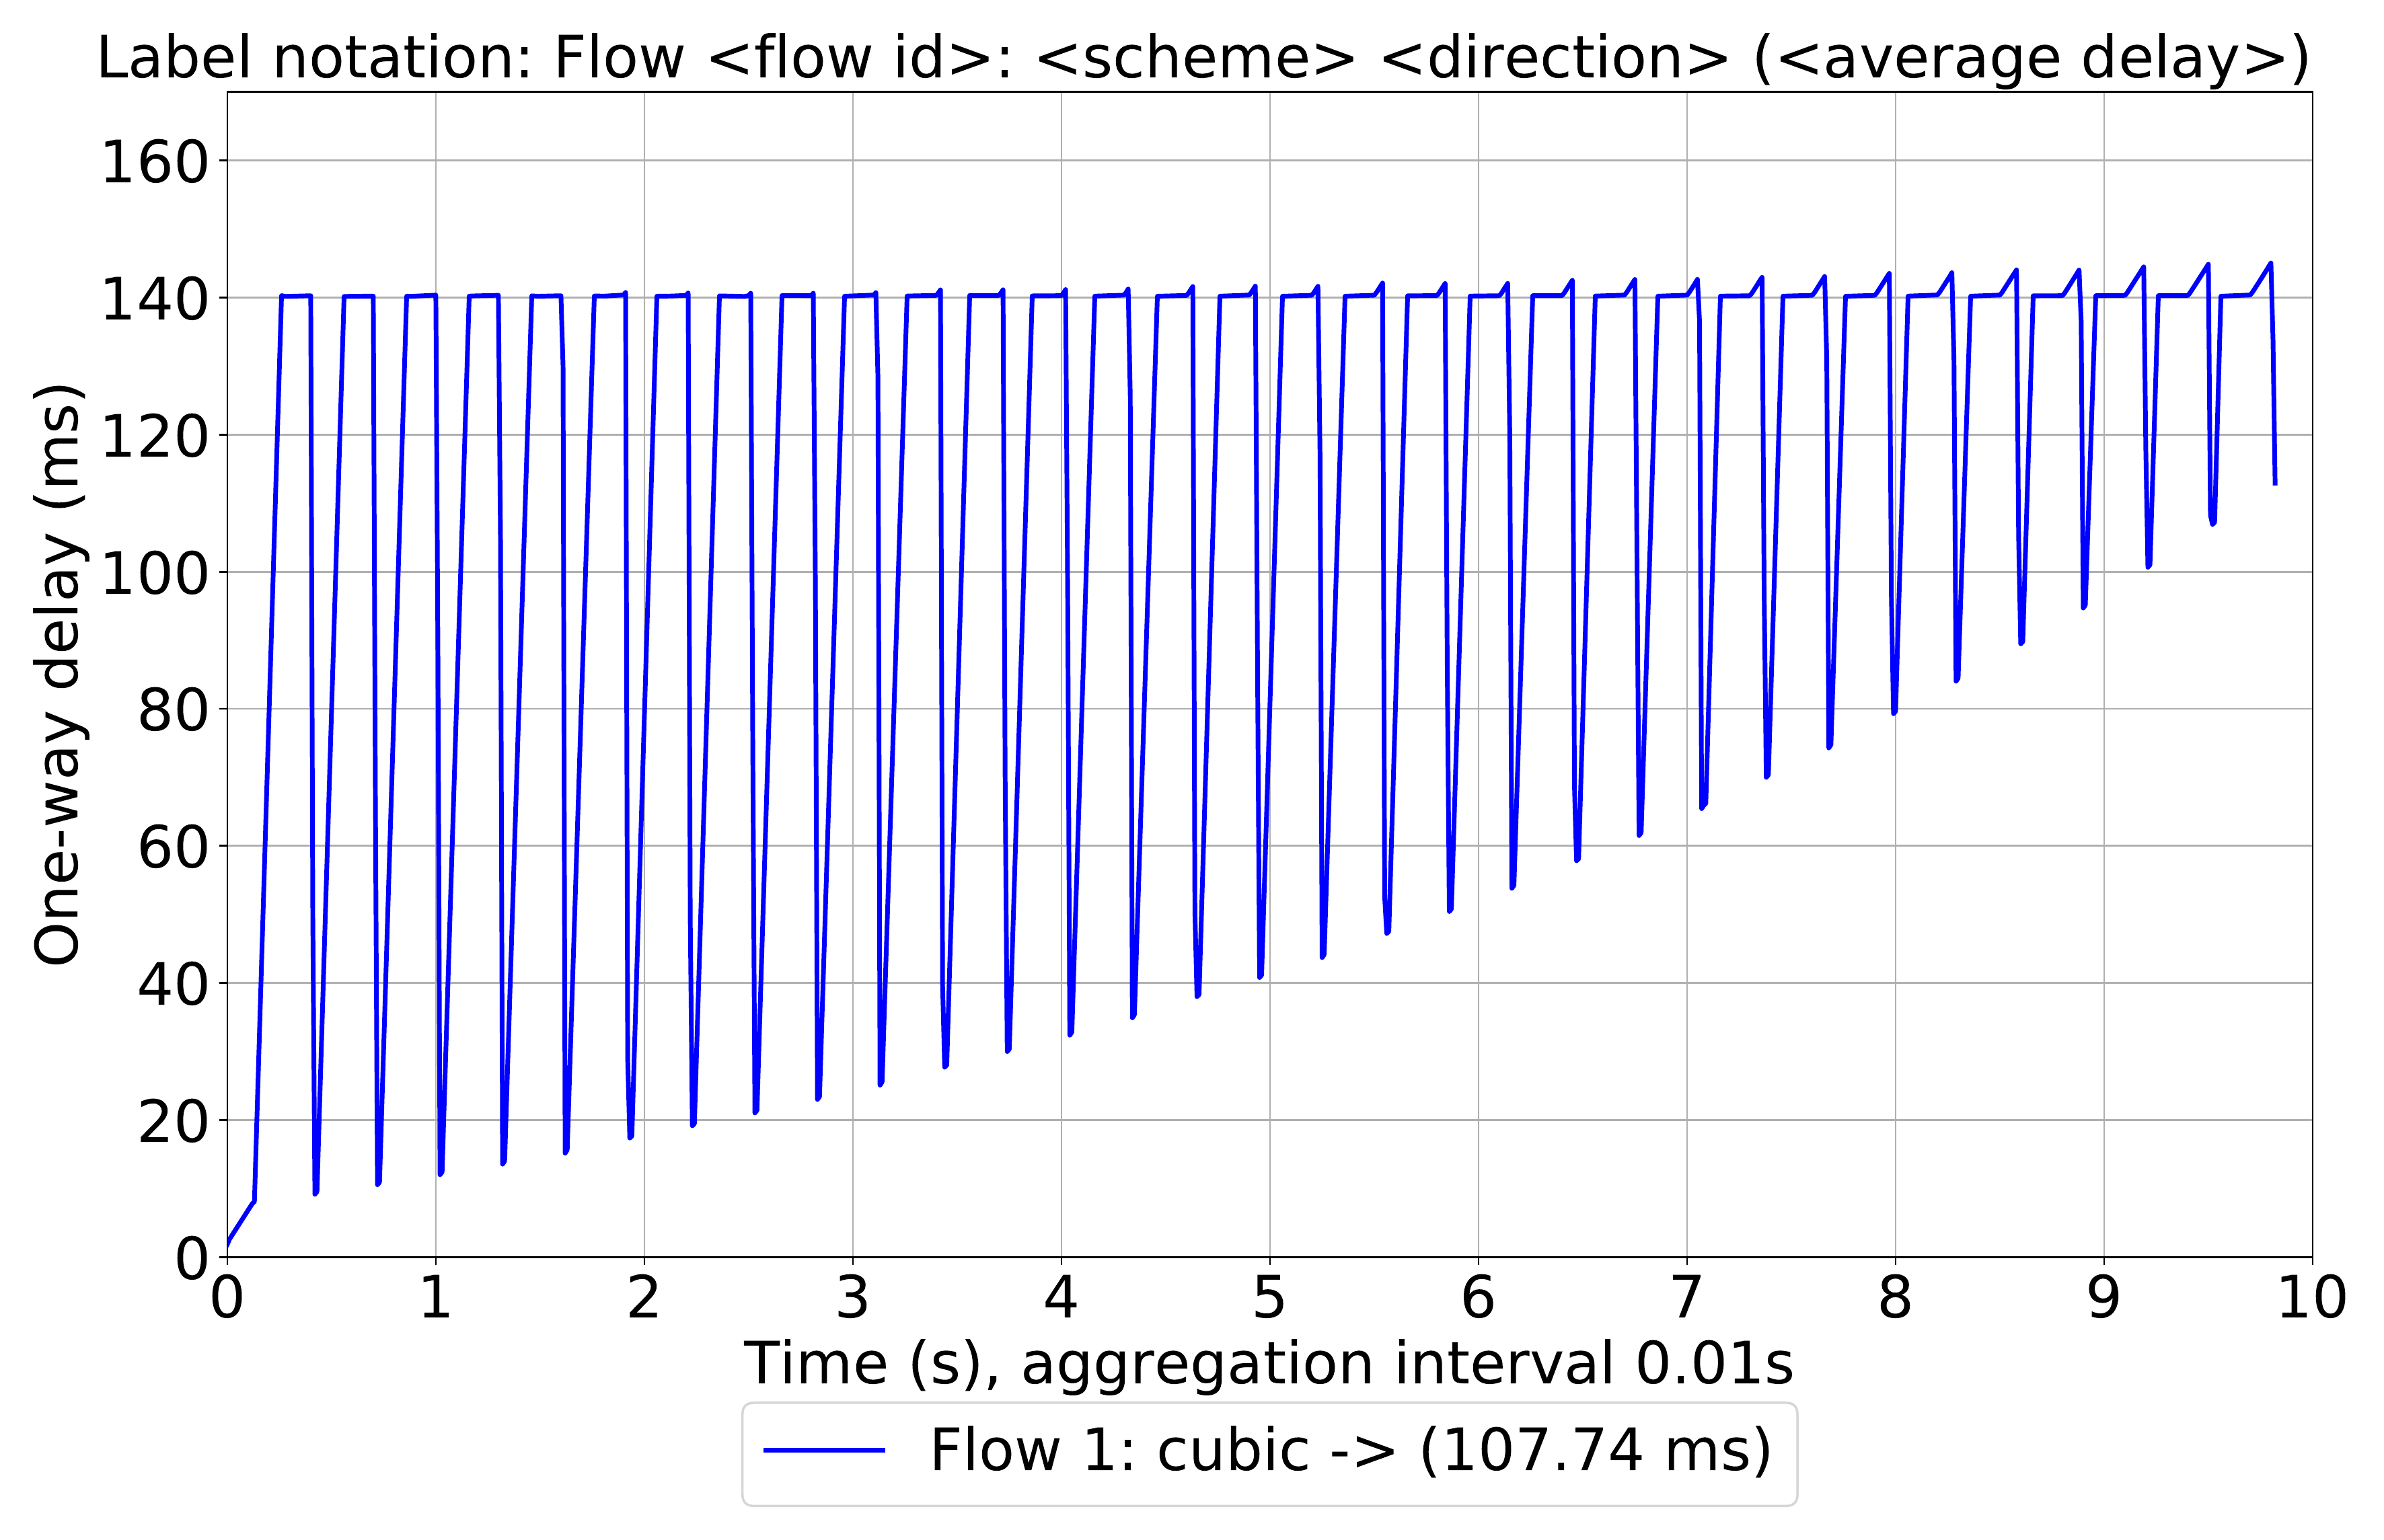} }}\\
    \vspace*{-0.3cm}
    \subfloat[Step = 150 ms]{{\includegraphics[height=0.3\textheight]{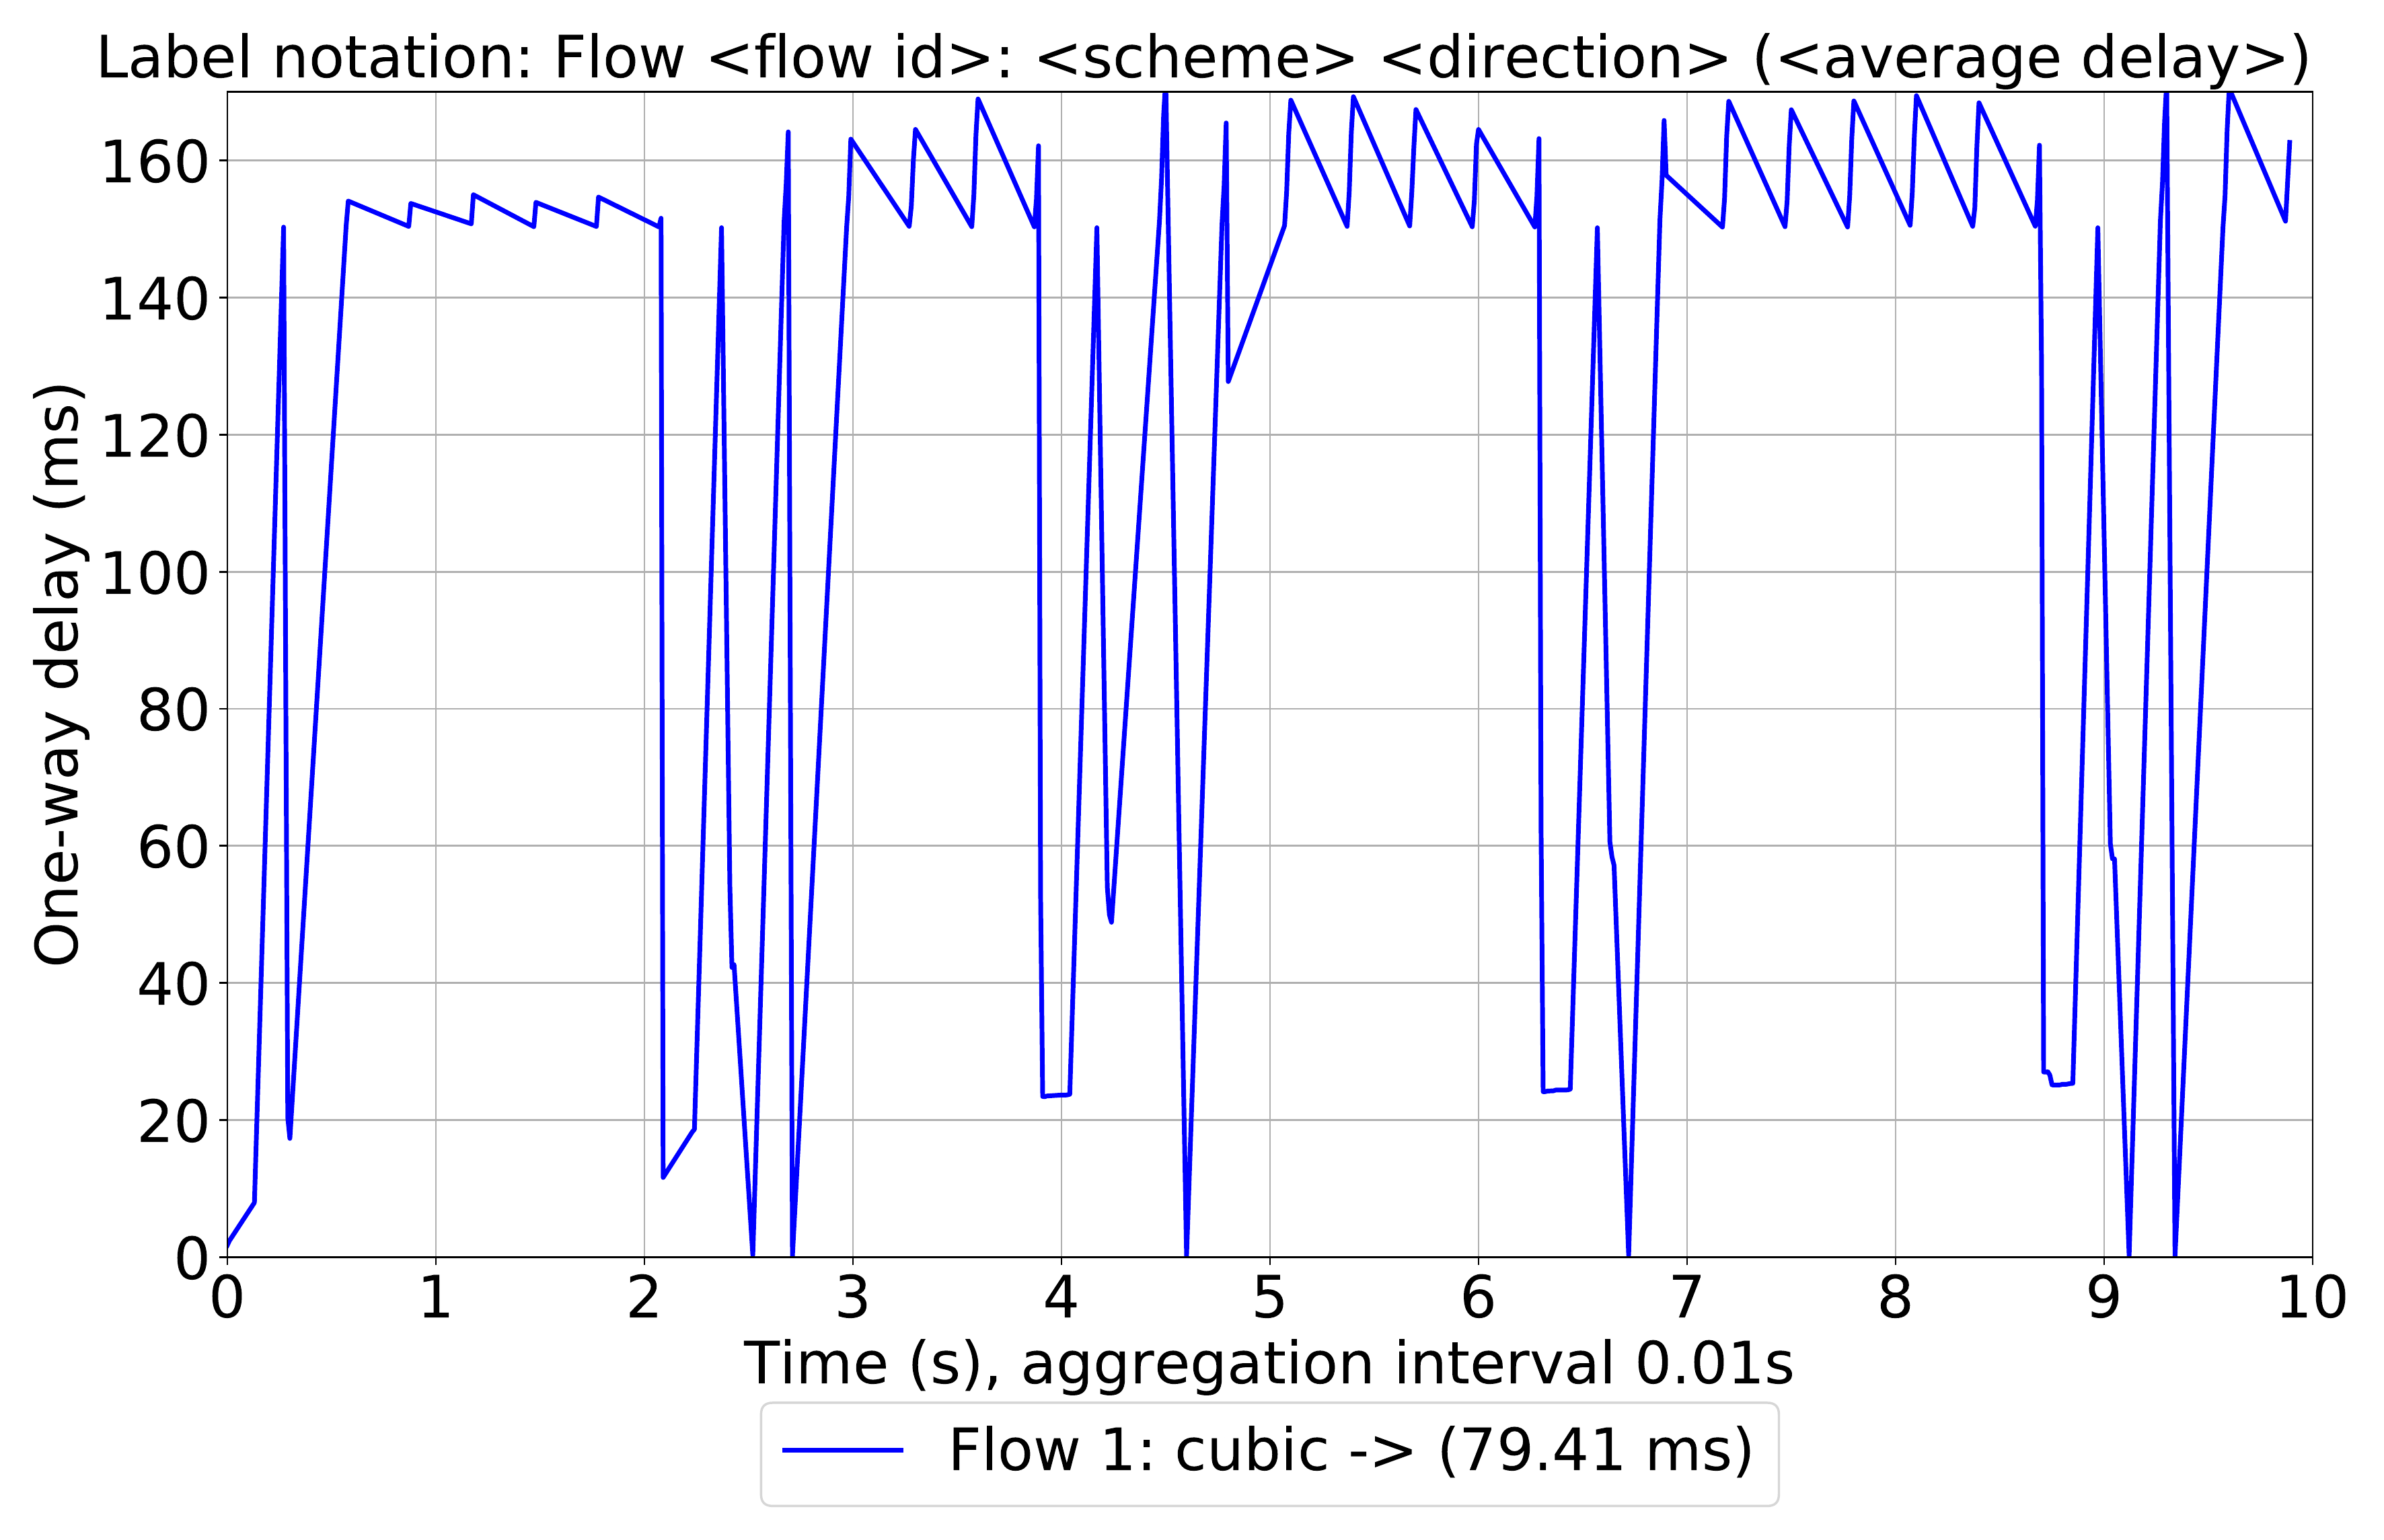} }}\\
    \vspace*{-0.3cm}
    \subfloat[Step = 160 ms]{{\includegraphics[height=0.3\textheight]{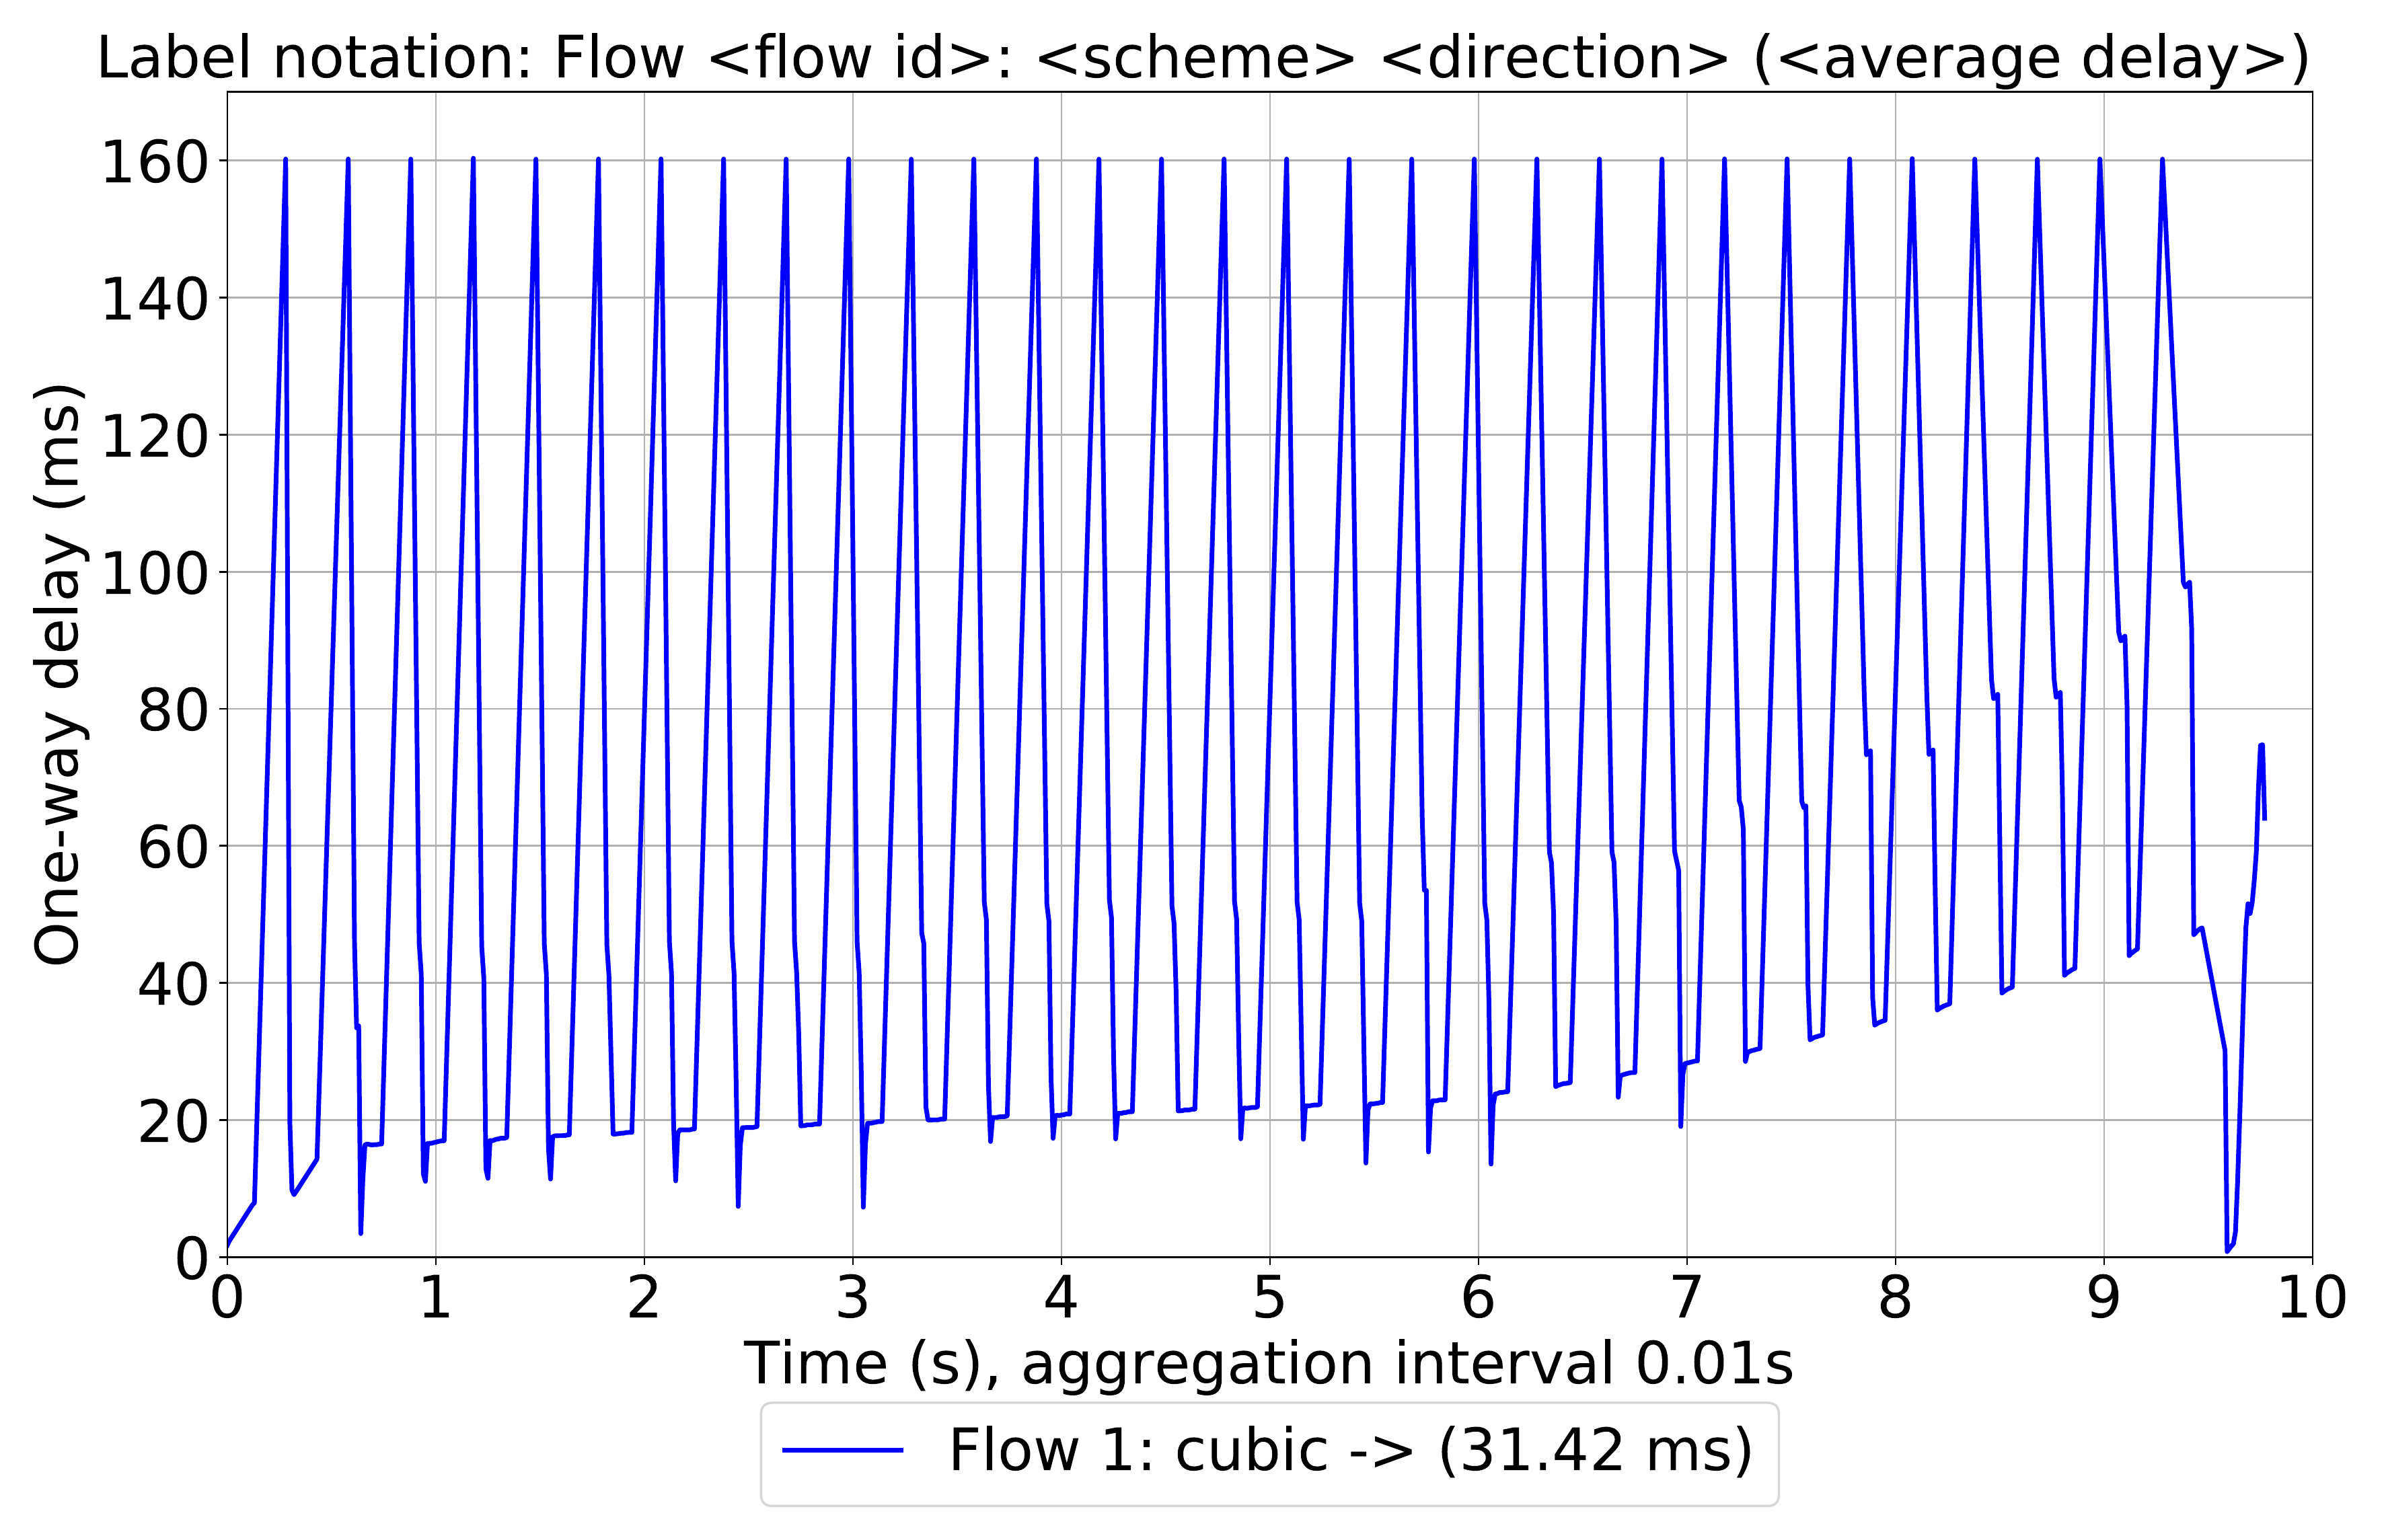} }}%
    \vspace*{-0.1cm}
    \caption{Cubic's average one-way delay plots for the delta 150 ms.}%
    \label{fig:vd-cubic-avgdelay}
\end{adjustbox}
\end{figure}

\FloatBarrier

\begin{figure}[h!]
\vspace*{-0.3cm}
\begin{adjustbox}{minipage=\linewidth,totalheight=\textheight}
    \centering
    \subfloat[Step = 140 ms]{{\includegraphics[height=0.3\textheight]{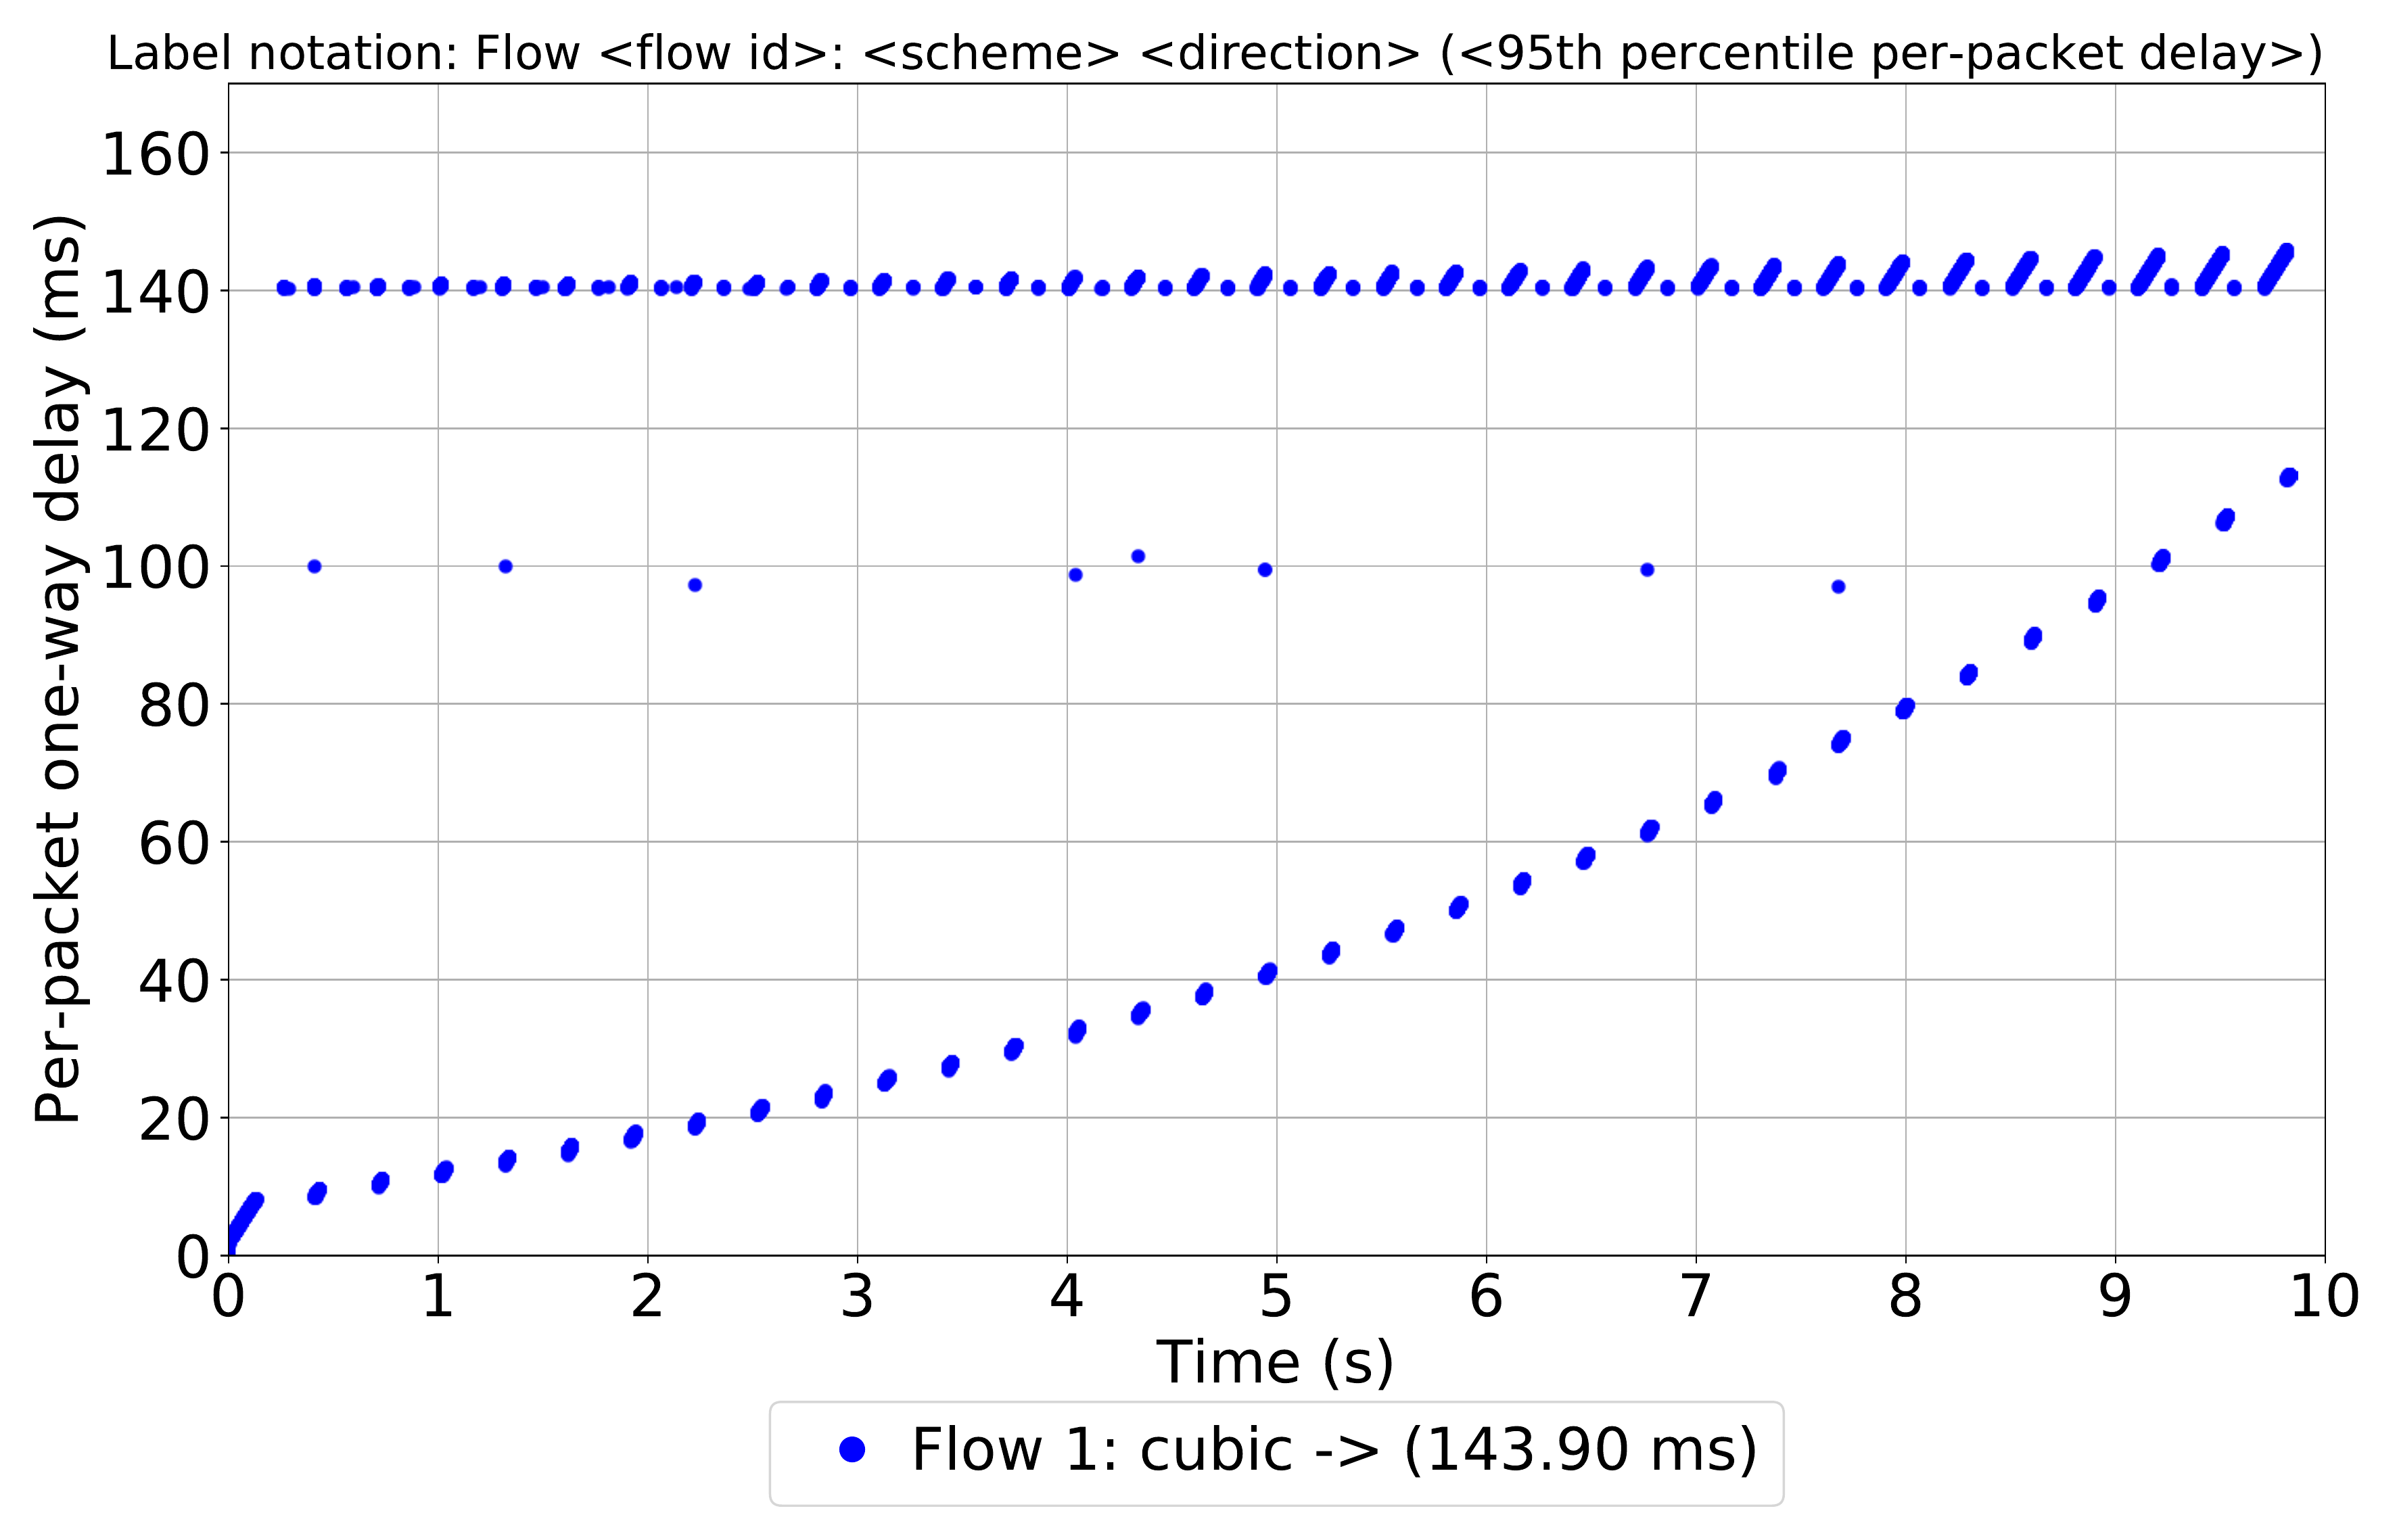} }}\\
    \vspace*{-0.3cm}
    \subfloat[Step = 150 ms]{{\includegraphics[height=0.3\textheight]{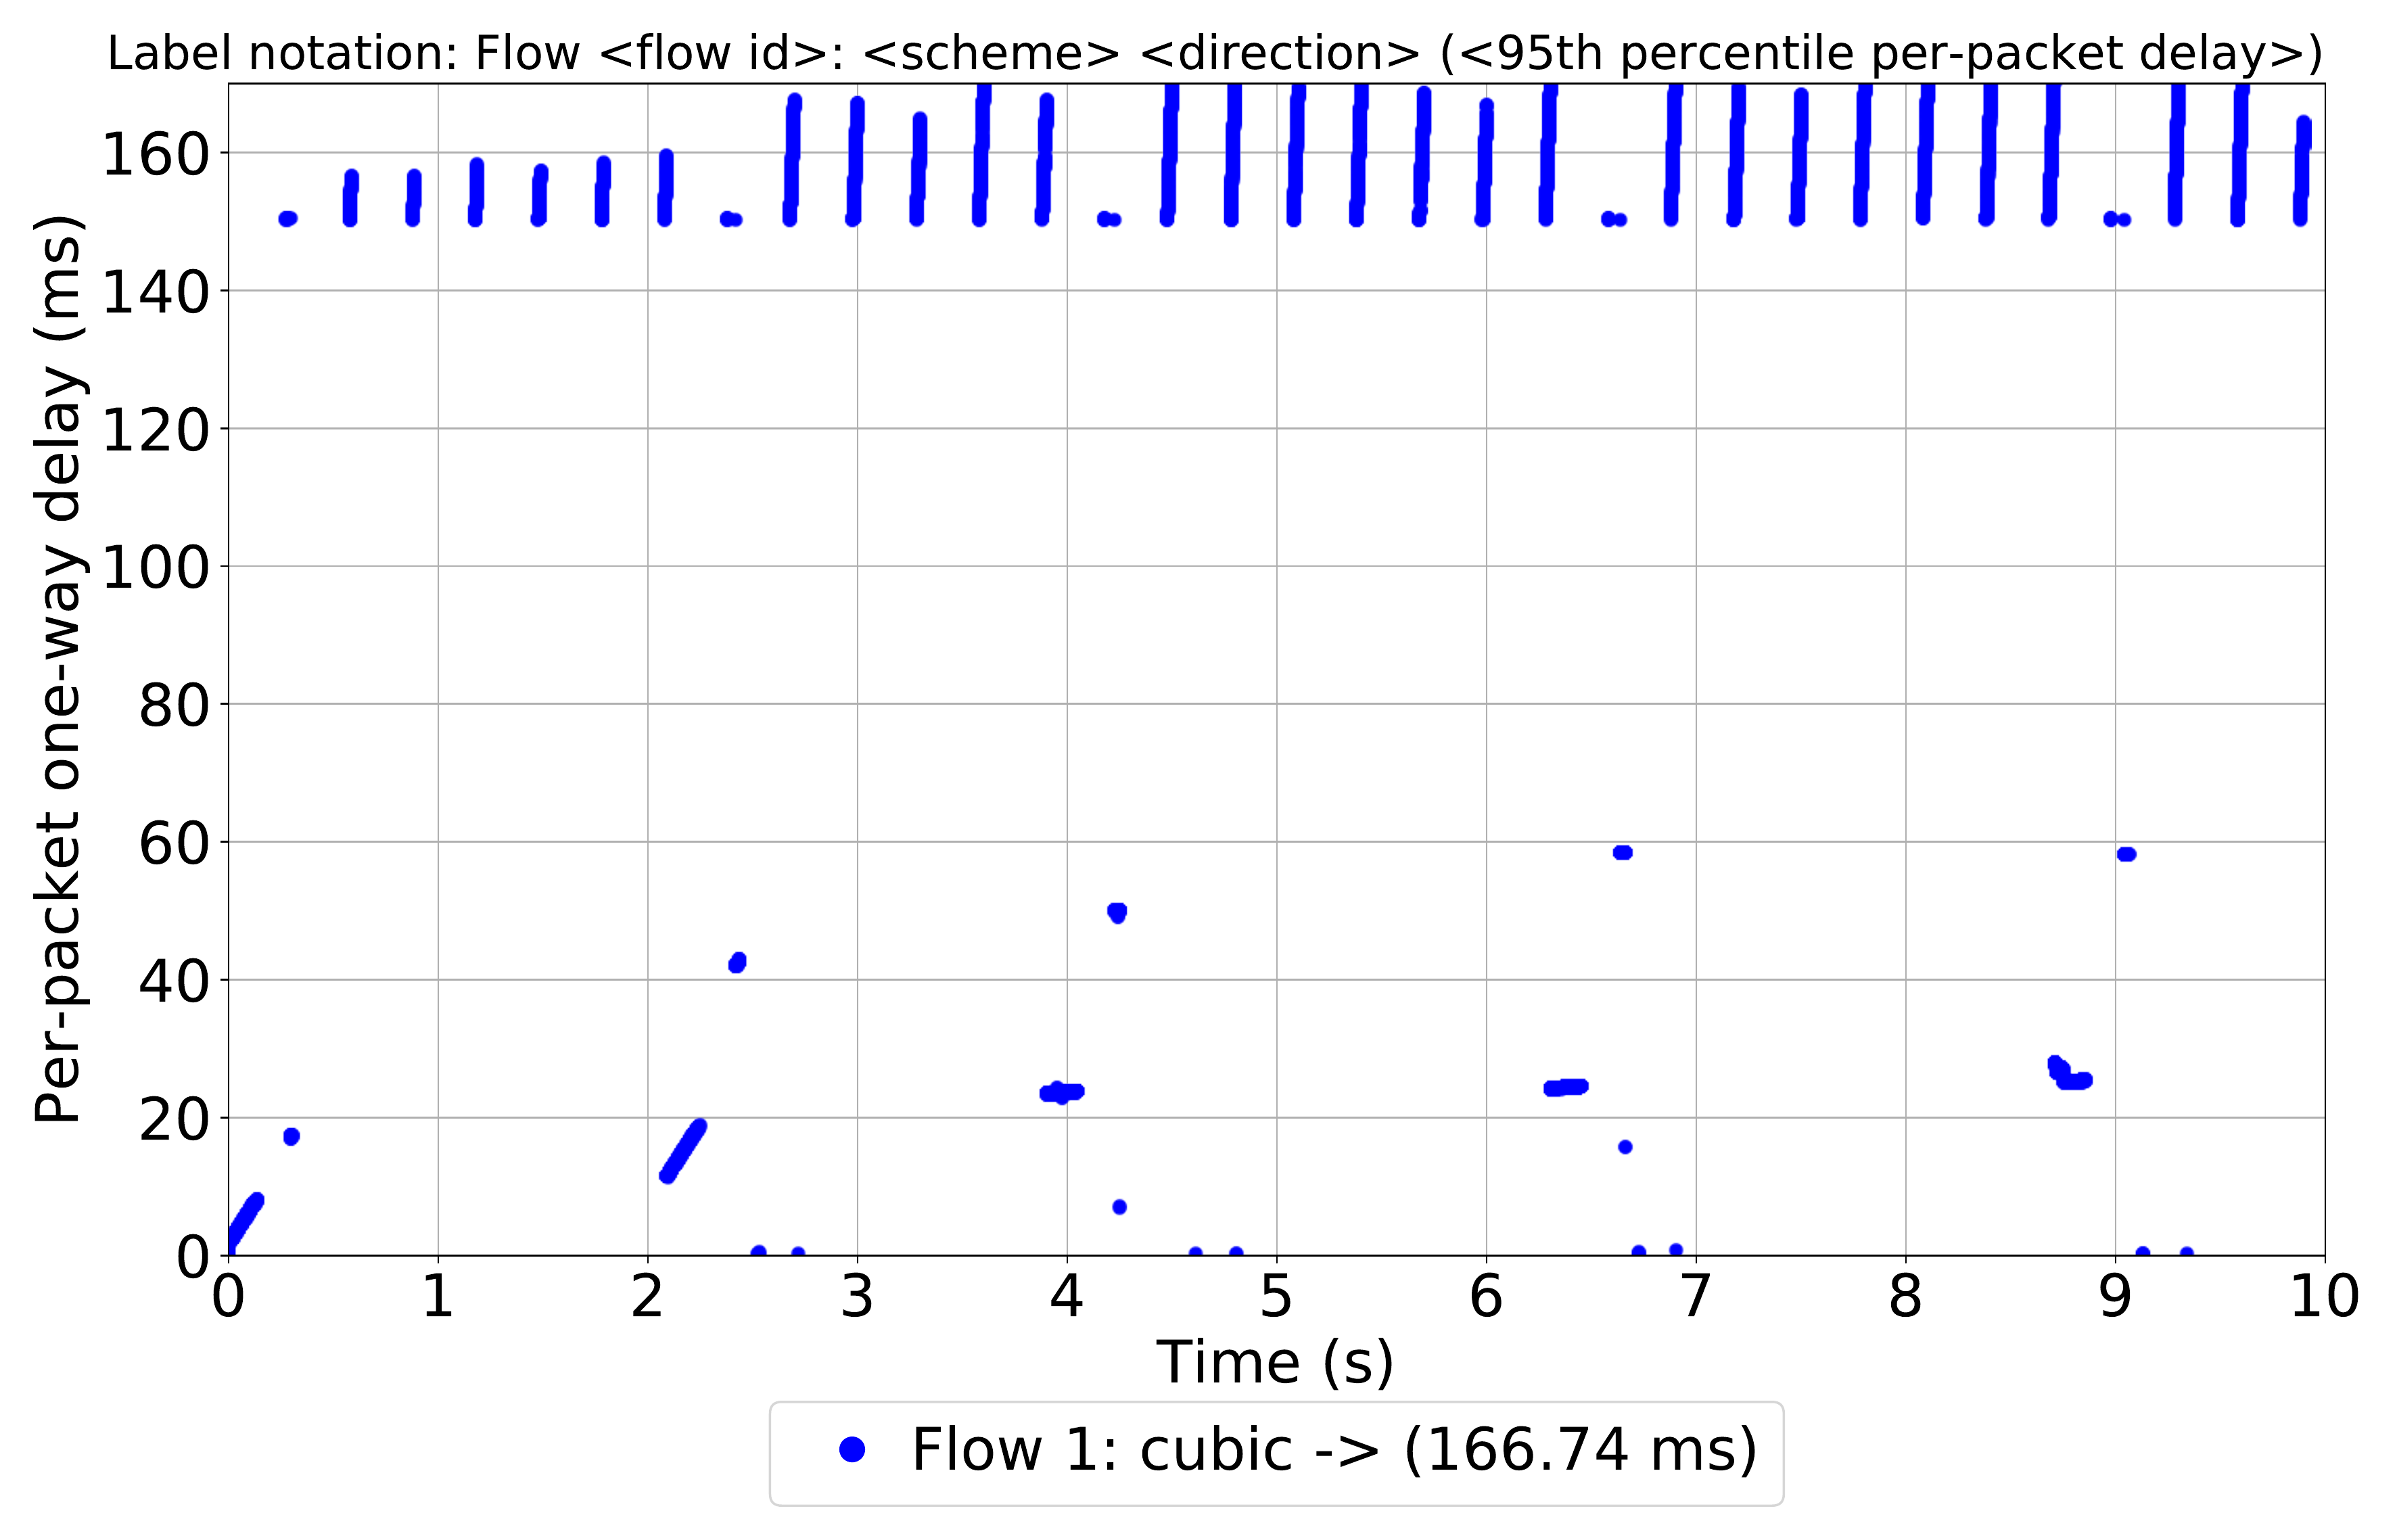} }}\\
    \vspace*{-0.3cm}
    \subfloat[Step = 160 ms]{{\includegraphics[height=0.3\textheight]{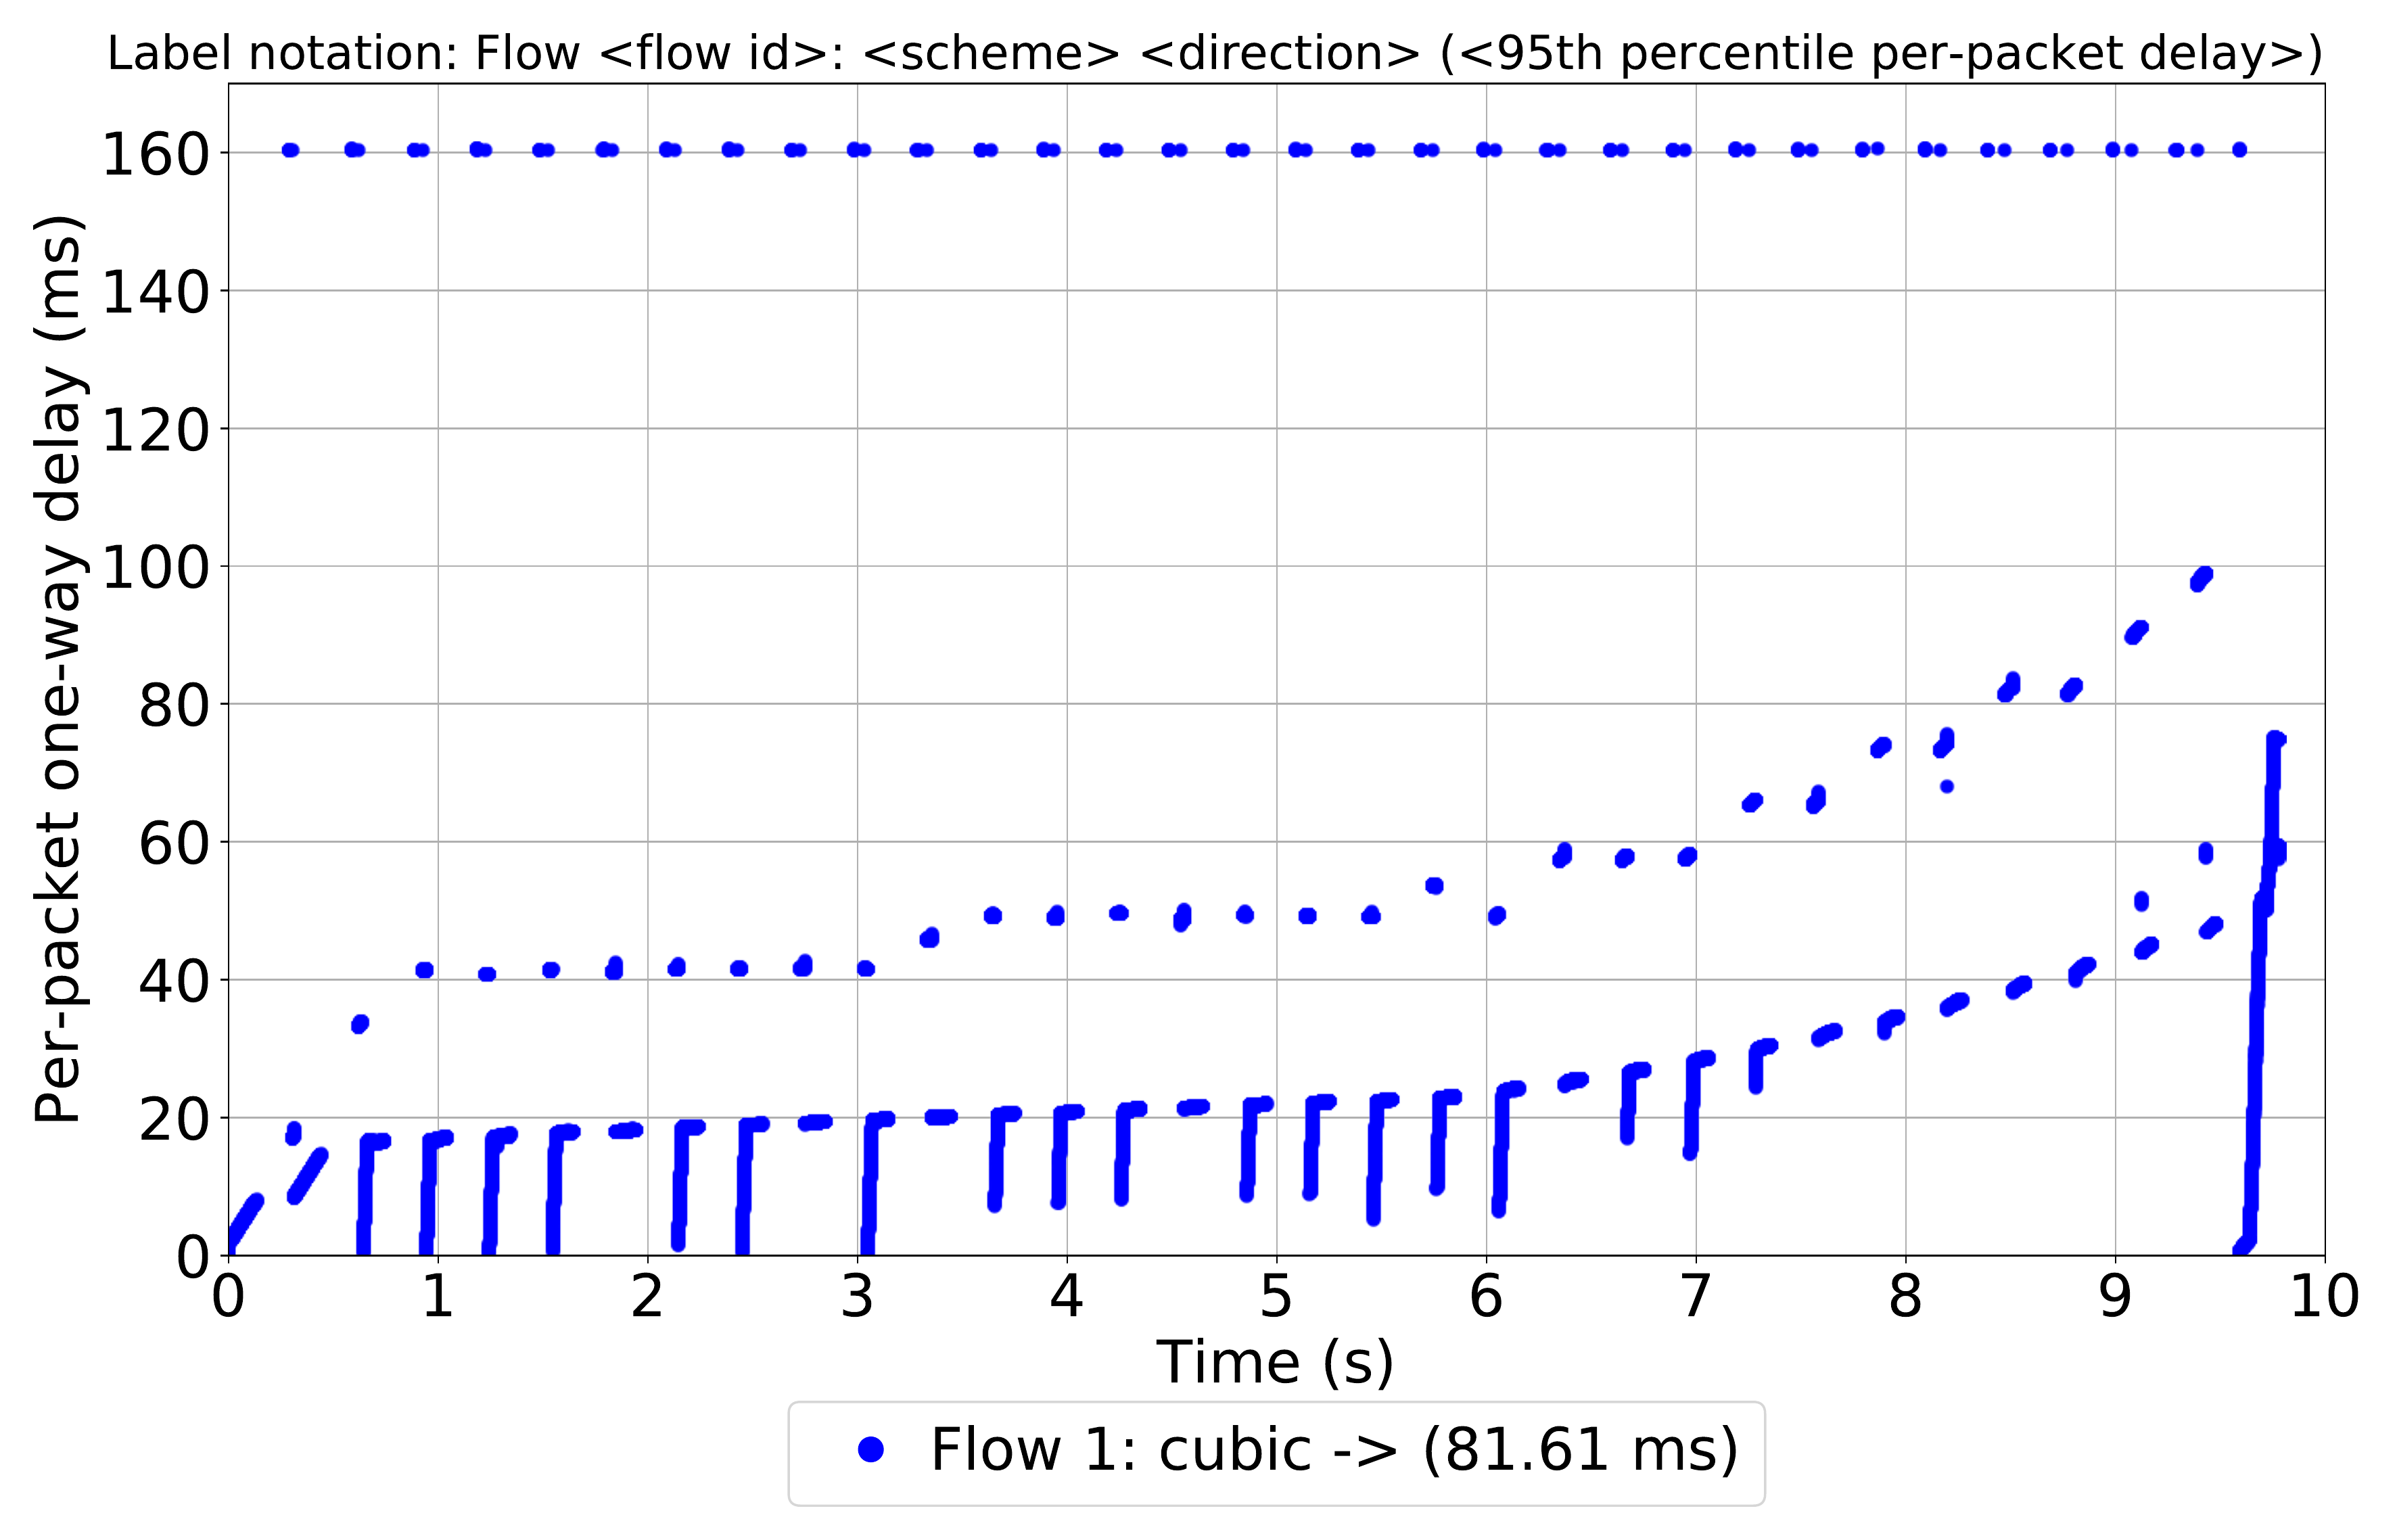} }}%
    \vspace*{-0.1cm}
    \caption{Cubic's per-packet one-way delay plots for the delta 150 ms.}%
    \label{fig:vd-cubic-pptdelay}
\end{adjustbox}
\end{figure}

\FloatBarrier

\begin{figure}[h!]
\vspace*{-0.3cm}
\begin{adjustbox}{minipage=\linewidth,totalheight=\textheight}
    \centering
    \subfloat[Step = 140 ms]{{\includegraphics[height=0.3\textheight]{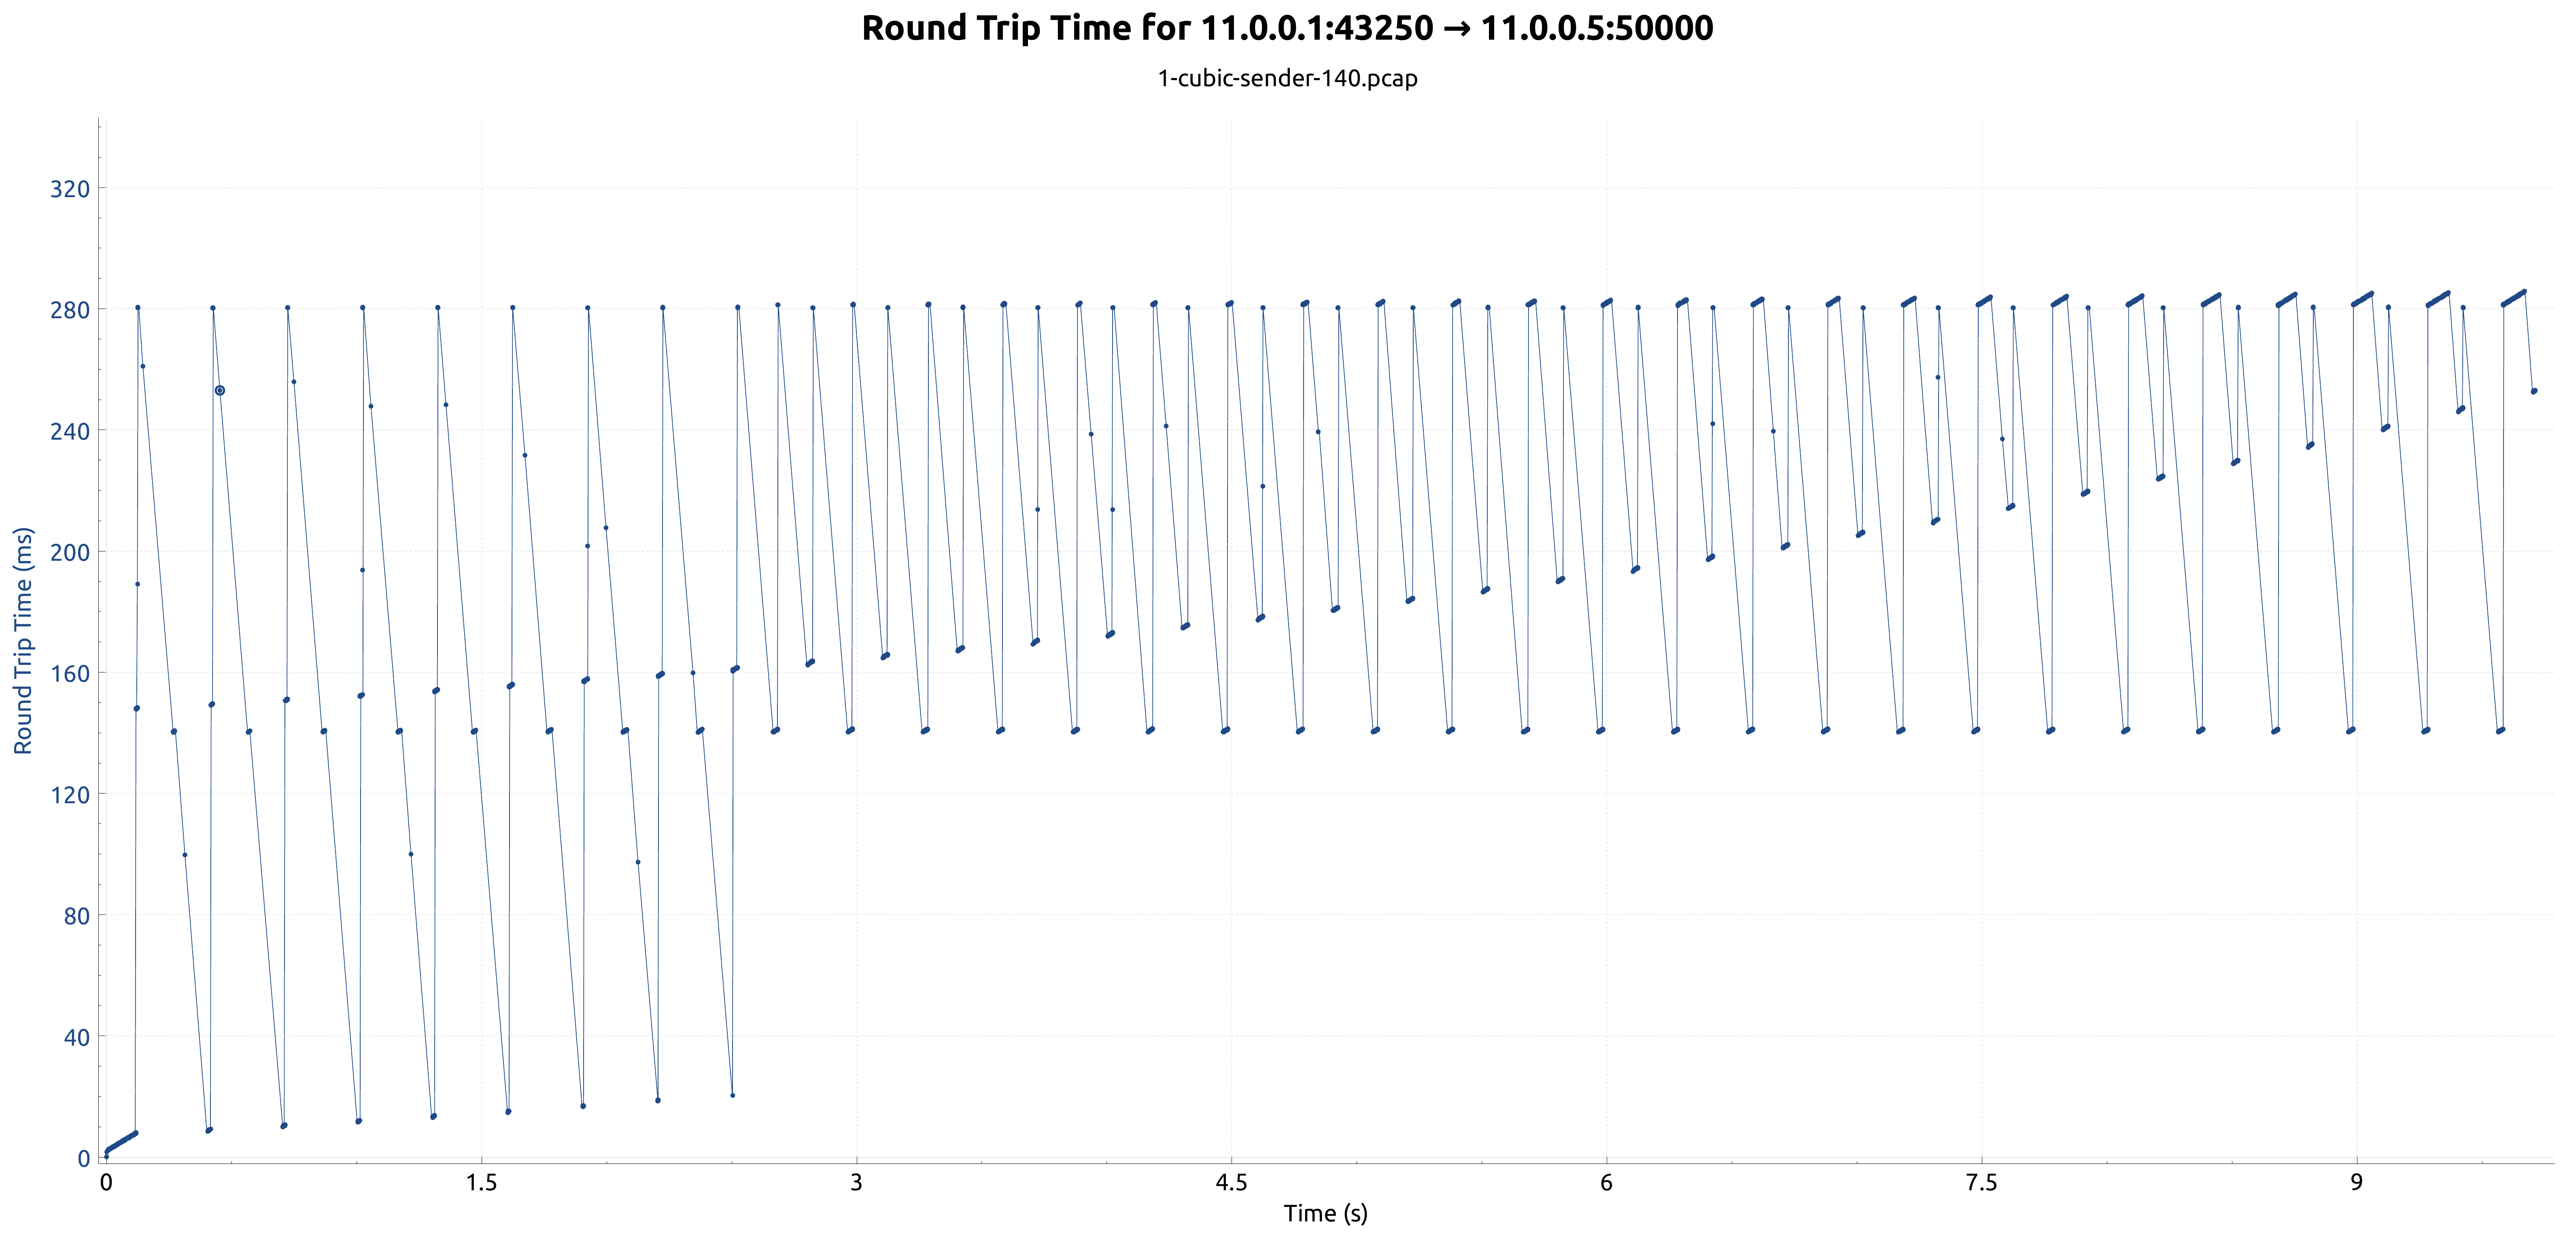} }}\\
    \vspace*{-0.2cm}
    \subfloat[Step = 150 ms]{{\includegraphics[height=0.3\textheight]{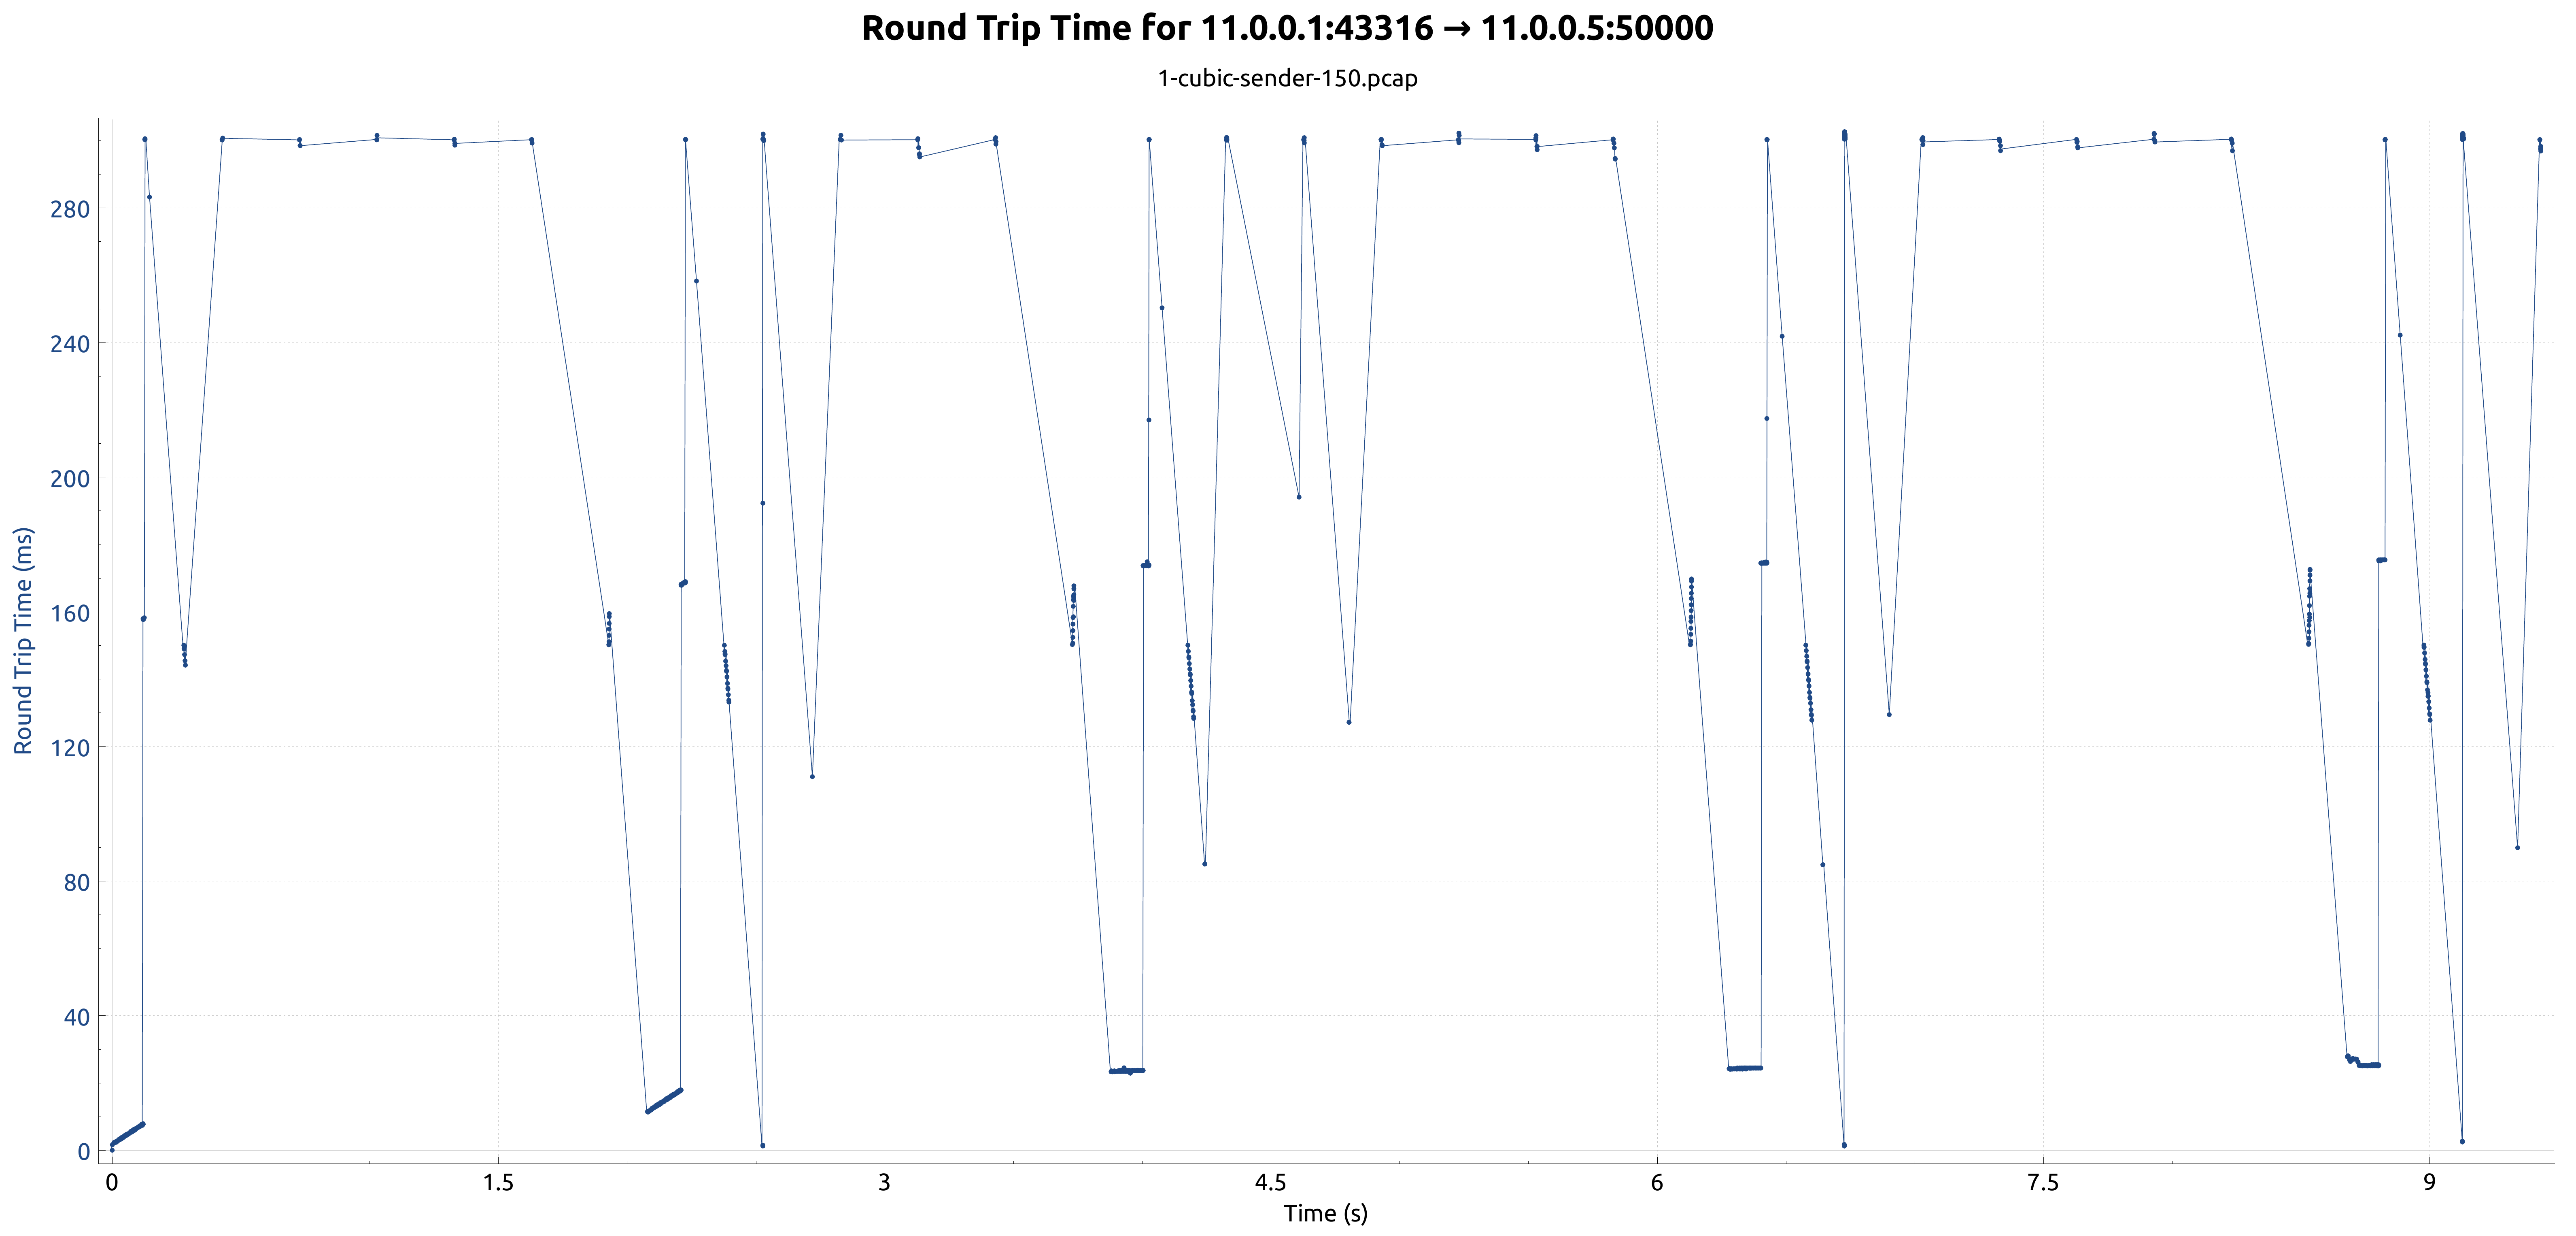} }}\\
    \vspace*{-0.2cm}
    \subfloat[Step = 160 ms]{{\includegraphics[height=0.3\textheight]{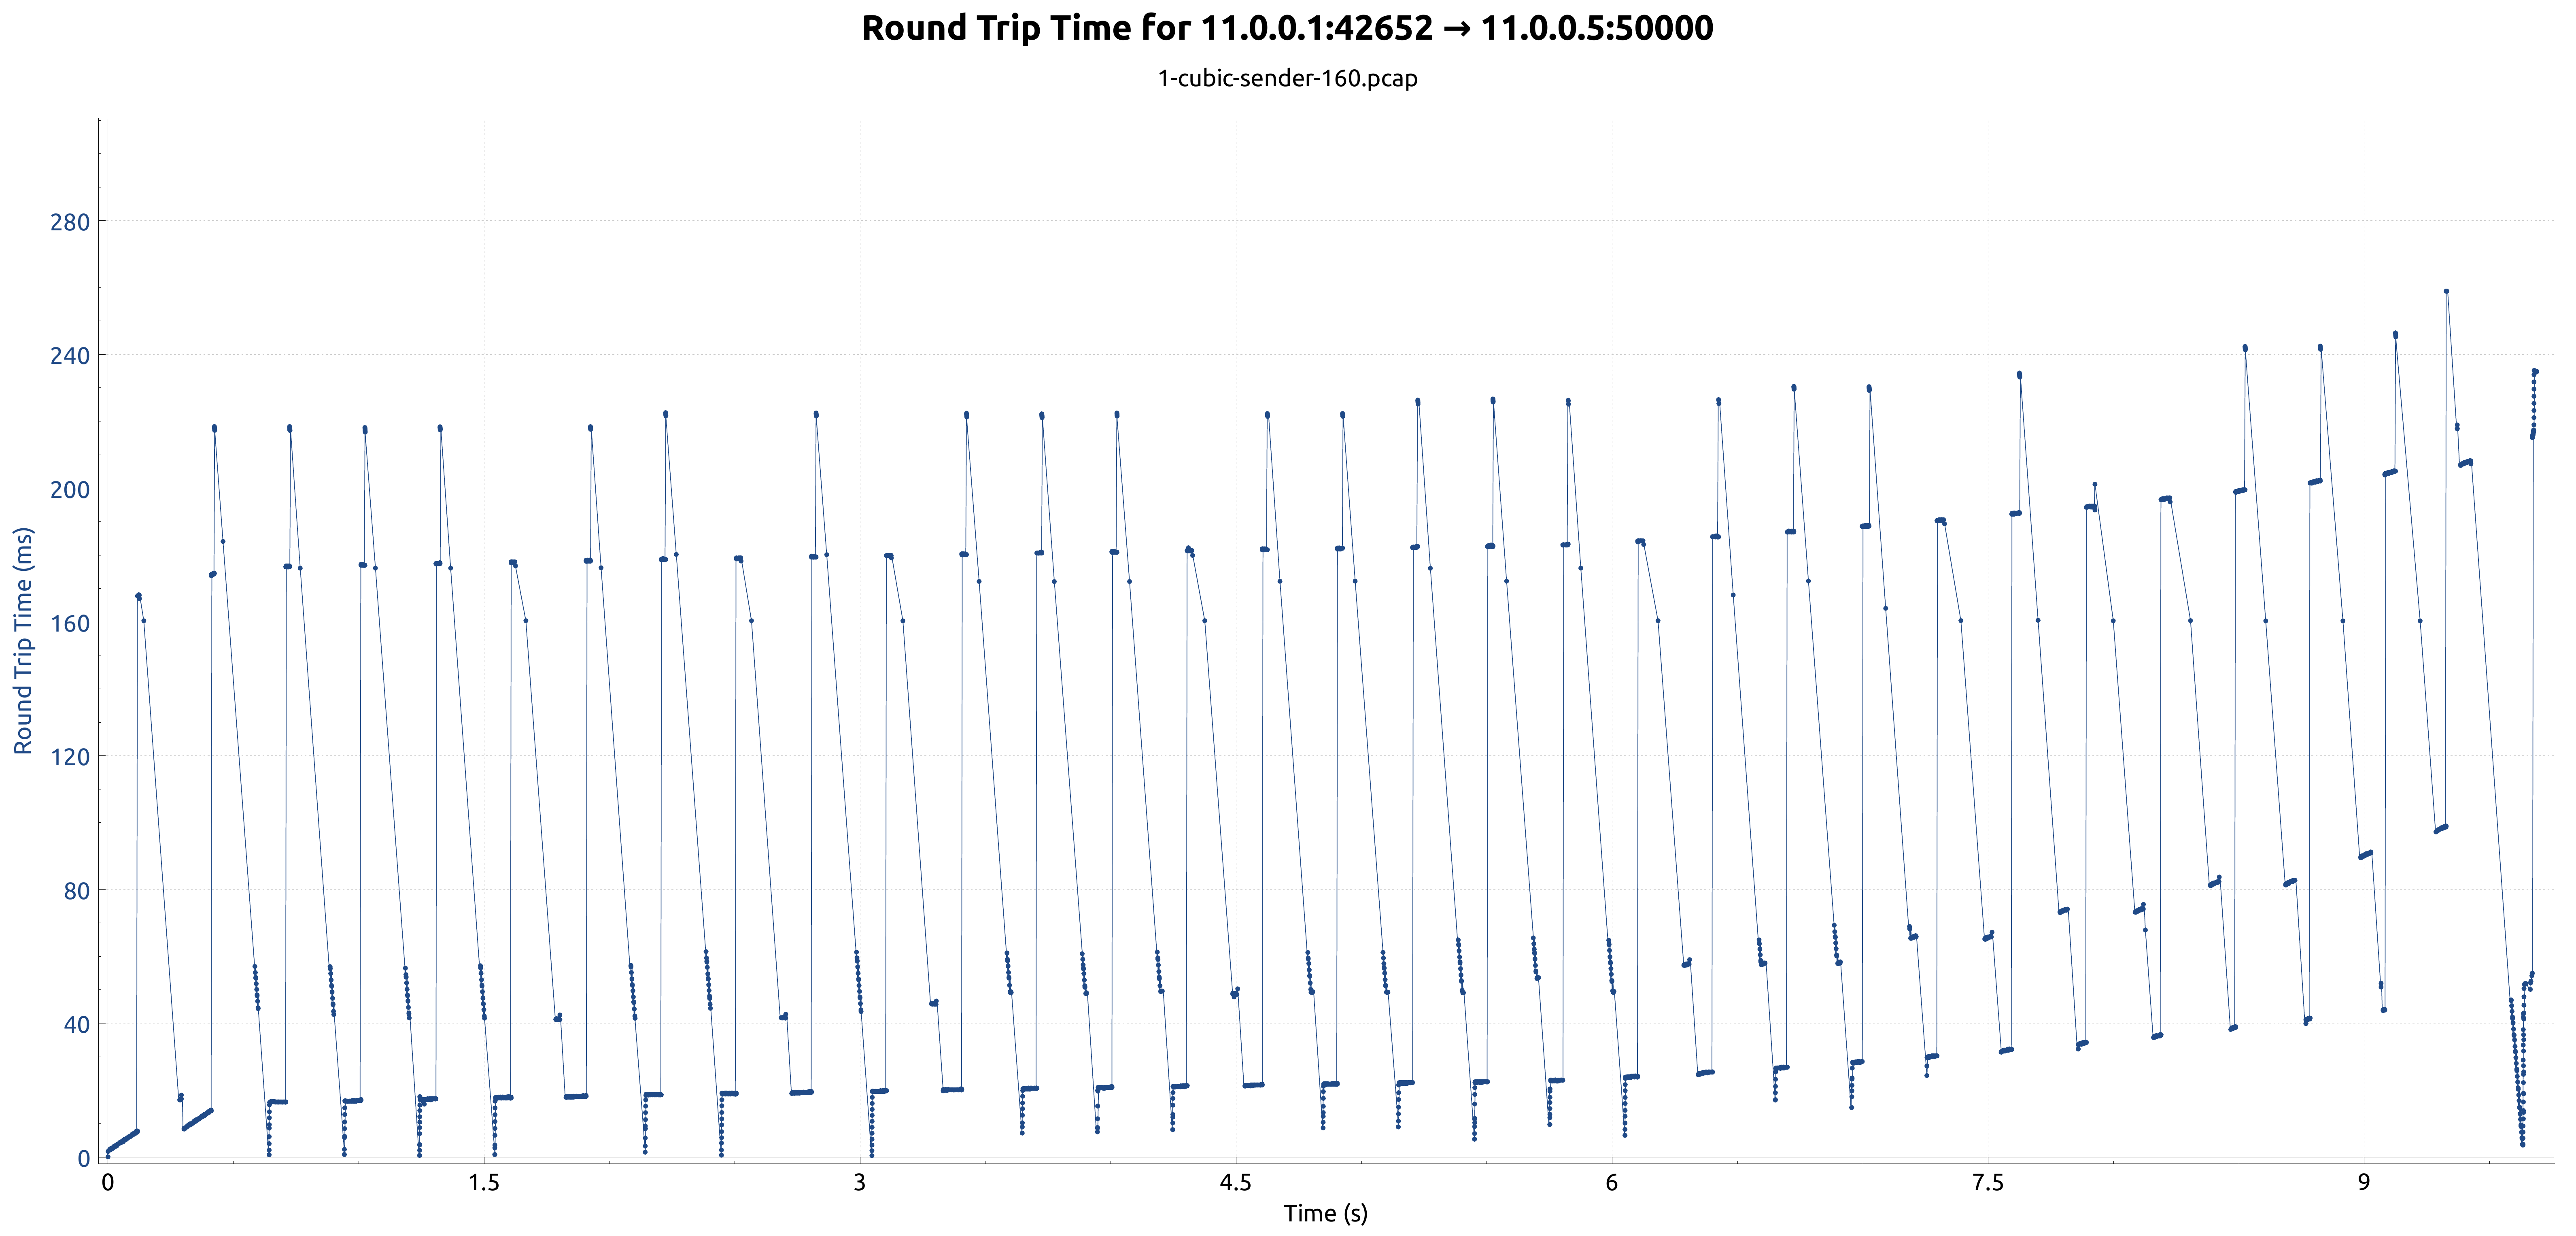} }}%
    \vspace*{-0.1cm}
    \caption{Cubic's per-packet RTT plots for the delta 150 ms.}%
    \label{fig:vd-cubic-rtt}
\end{adjustbox}
\end{figure}

\FloatBarrier
